# Supplementary material for: Aspects of Propagator Sparsening in Lattice QCD
Source: arXiv:2501.05404 source file (2025-03-28)
Supplement: Supplementary file 1 [file Sparsening_Supplementary_Materials.pdf]

# Aspects of Propagator Sparsening in Lattice QCD: Supplementary Material

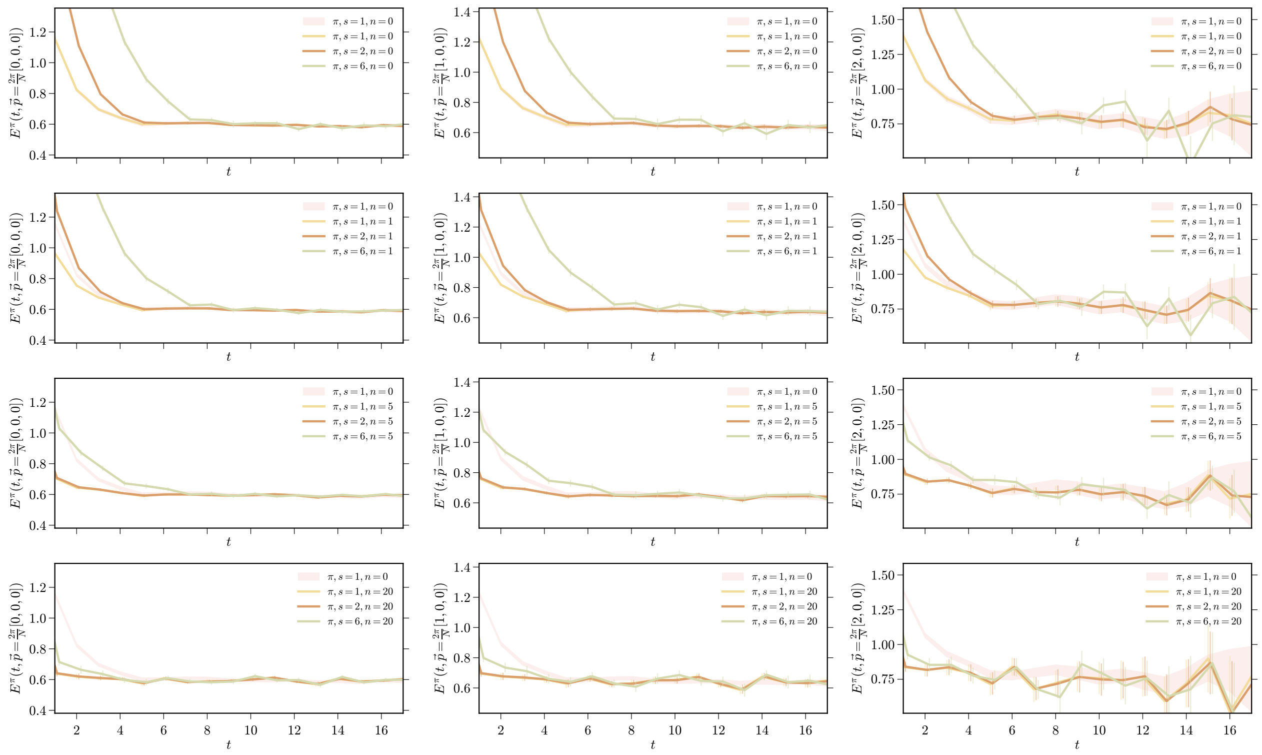


FIG. 1. The pion effective energy as a function of time extent, $E^{\pi}(t, \vec{p})$ (Eq. (18)), for three decimation factors ($s = 1$, $s = 2$, $s = 6$), three blocking factors ($n = 1, n = 5, n = 20$),three different values of momentum, and $\alpha = \beta = 1$. The unsparsened correlation function with $s = 1, n = 0$ is shown as a pink shaded-region.

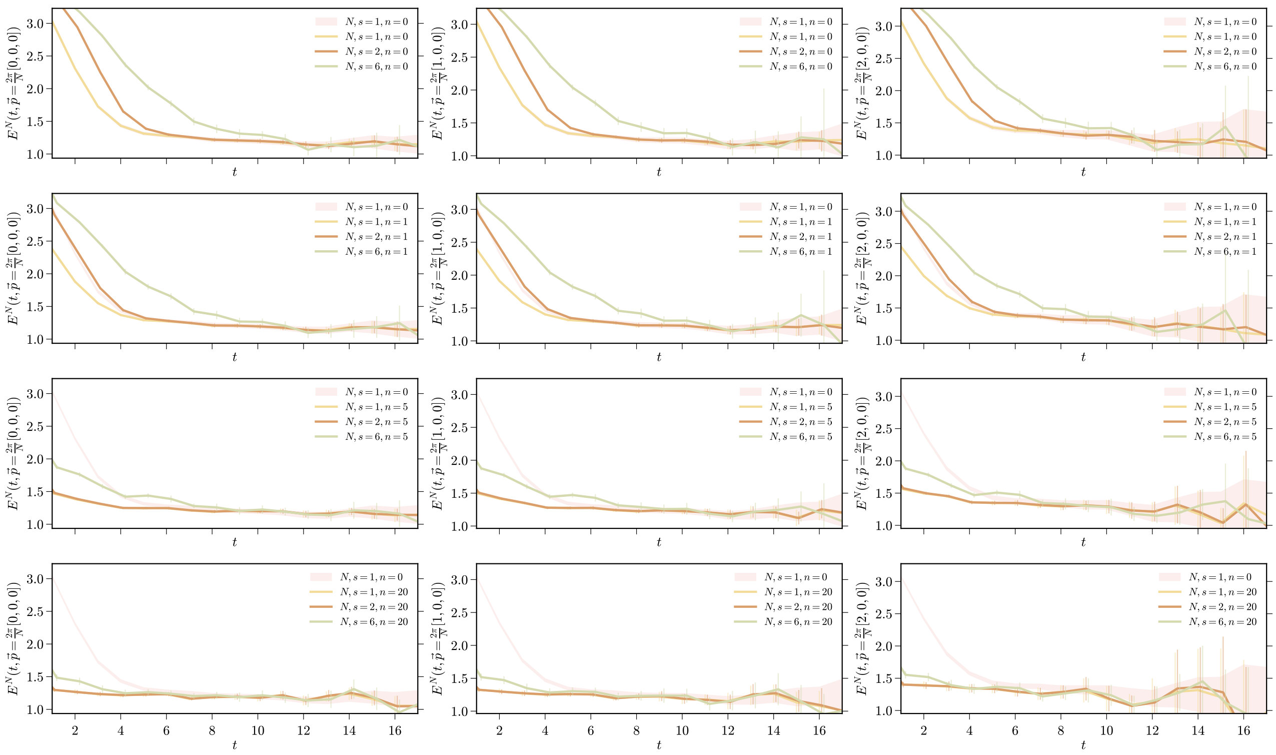


FIG. 2. The proton effective energy as a function of time extent, $E^N(t,\vec{p})$ (Eq. (18)), for three decimation factors ($s=1$, $s=2$, $s=6$), three blocking factors ($n=1, n=5, n=20$),three different values of momentum, and $\alpha=\beta=1$. The unsparsened correlation function with $s=1, n=0$ is shown as a pink shaded-region.

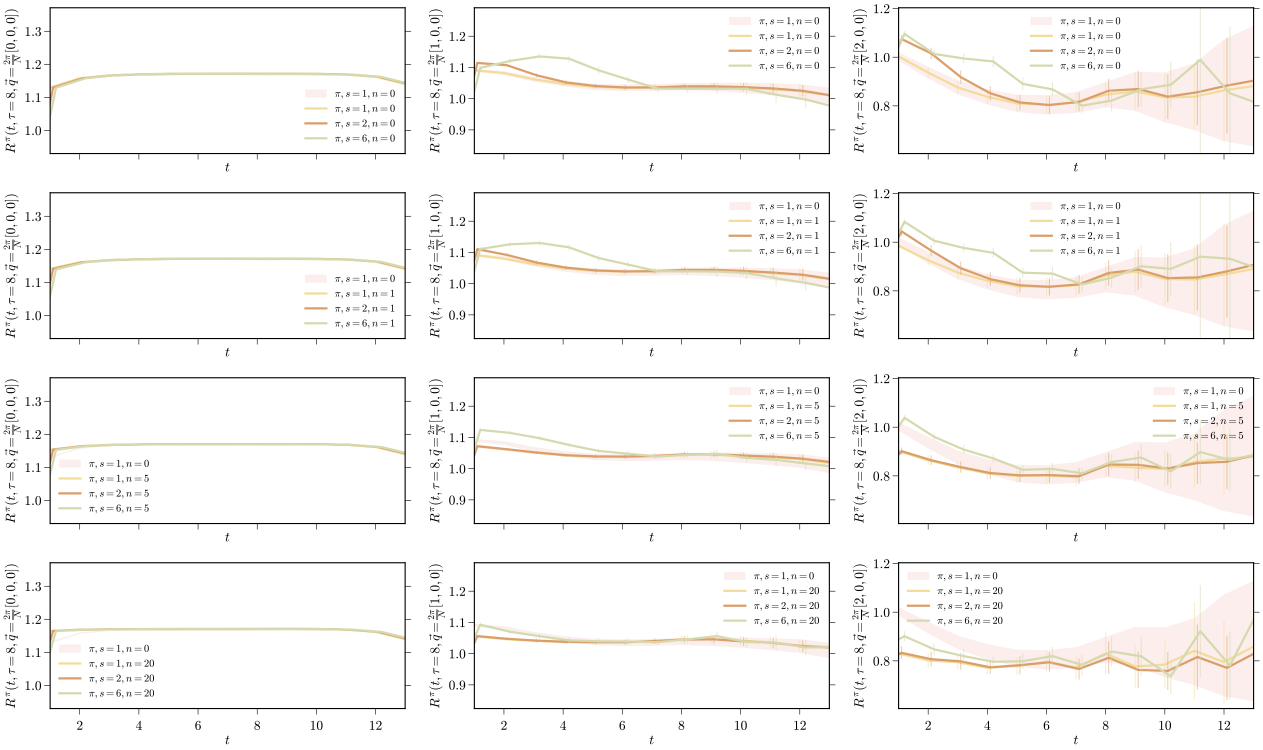

FIG. 3. The pion improved ratio of three- and two-point functions, $R^{\pi}(t, \tau = 8, \vec{q})$ (Eqs. (30) and (33)), for three decimation factors ($s = 1$, $s = 2$, $s = 6$), three blocking factors ($n = 1, n = 5, n = 20$),three different values of momentum, and $\alpha = \beta = 1$. The unsparsened correlation function with $s = 1, n = 0$ is shown as a pink shaded-region.

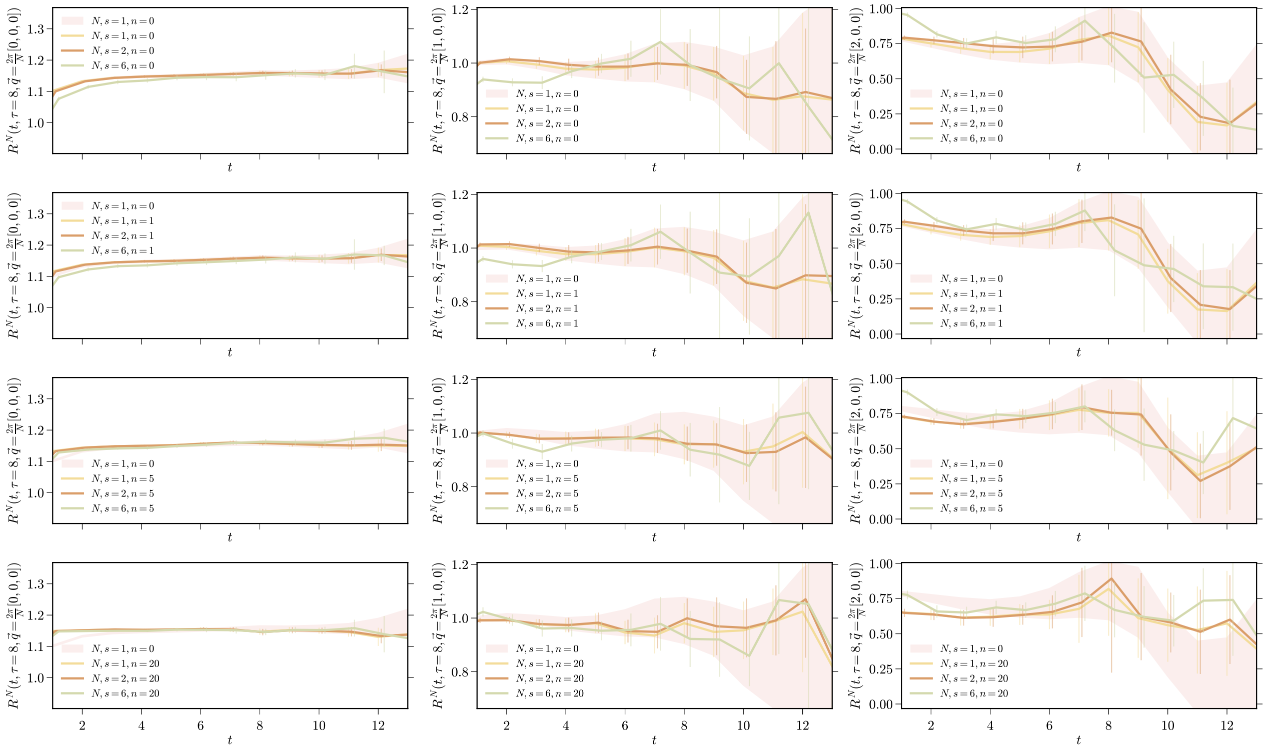


FIG. 4. The proton improved ratio of three- and two-point functions, $R^N(t, \tau = 8, \vec{q})$ (Eqs. (30) and (33)), for three decimation factors ($s = 1$, $s = 2$, $s = 6$), three blocking factors ($n = 1, n = 5, n = 20$),three different values of momentum, and $\alpha = \beta = 1$. The unsparsened correlation function with $s = 1, n = 0$ is shown as a pink shaded-region.

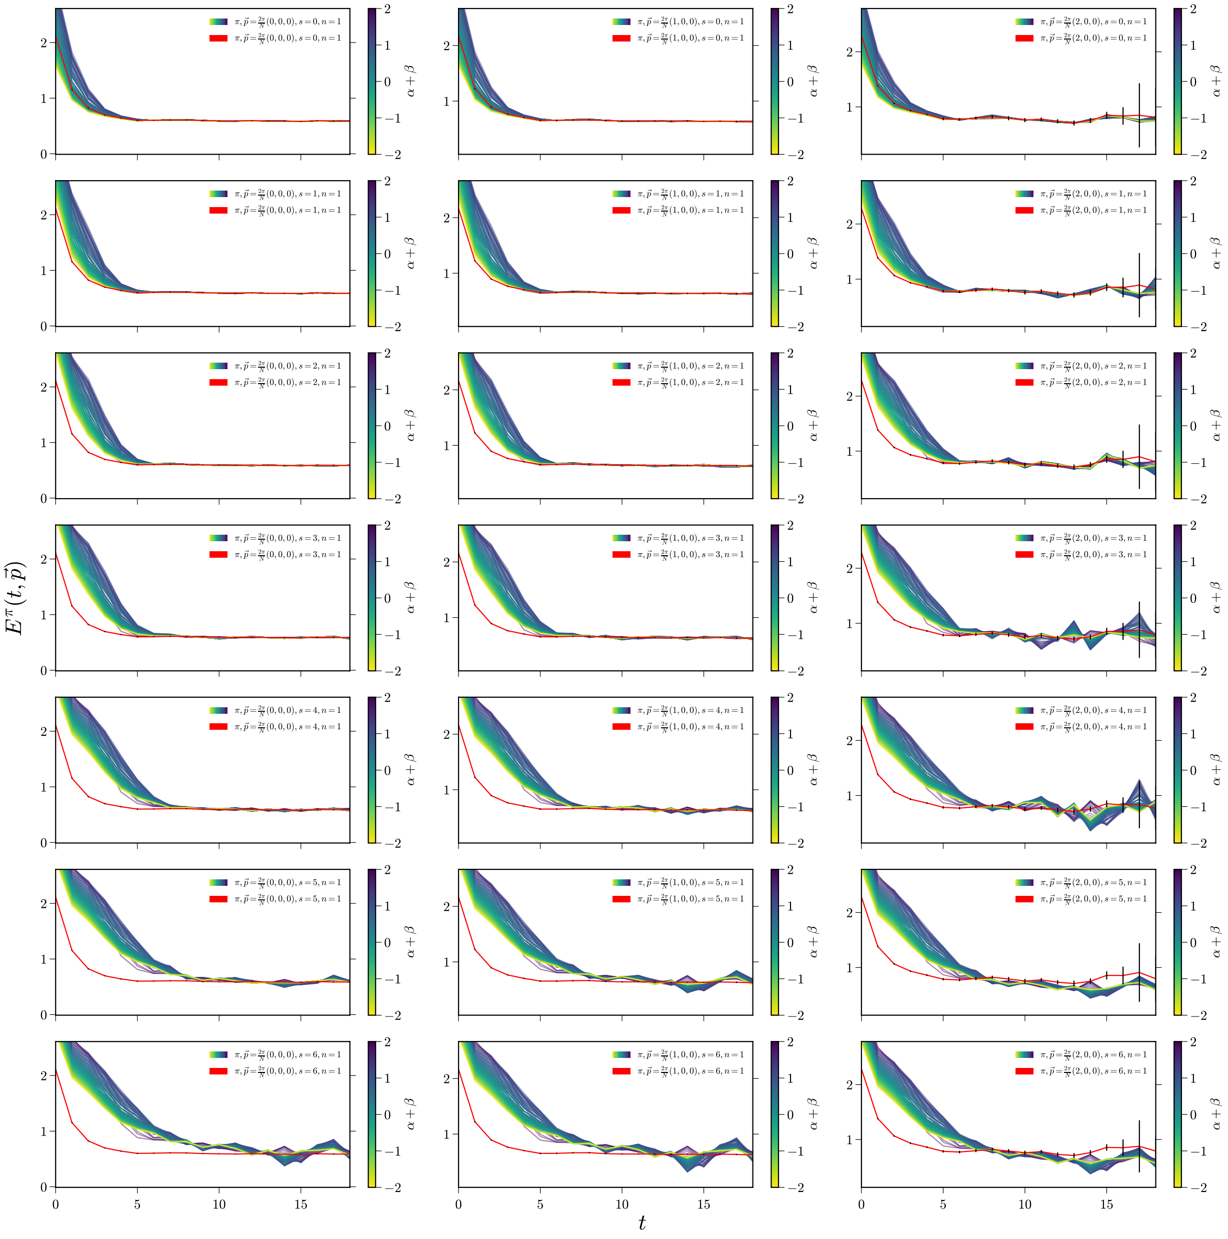


FIG. 5. Effective energy as a function of time, $E^\pi(t, \vec{p})$ (Eq. (18)), for varying $\alpha, \beta$ and momentum. The unsparsened result is shown in red.

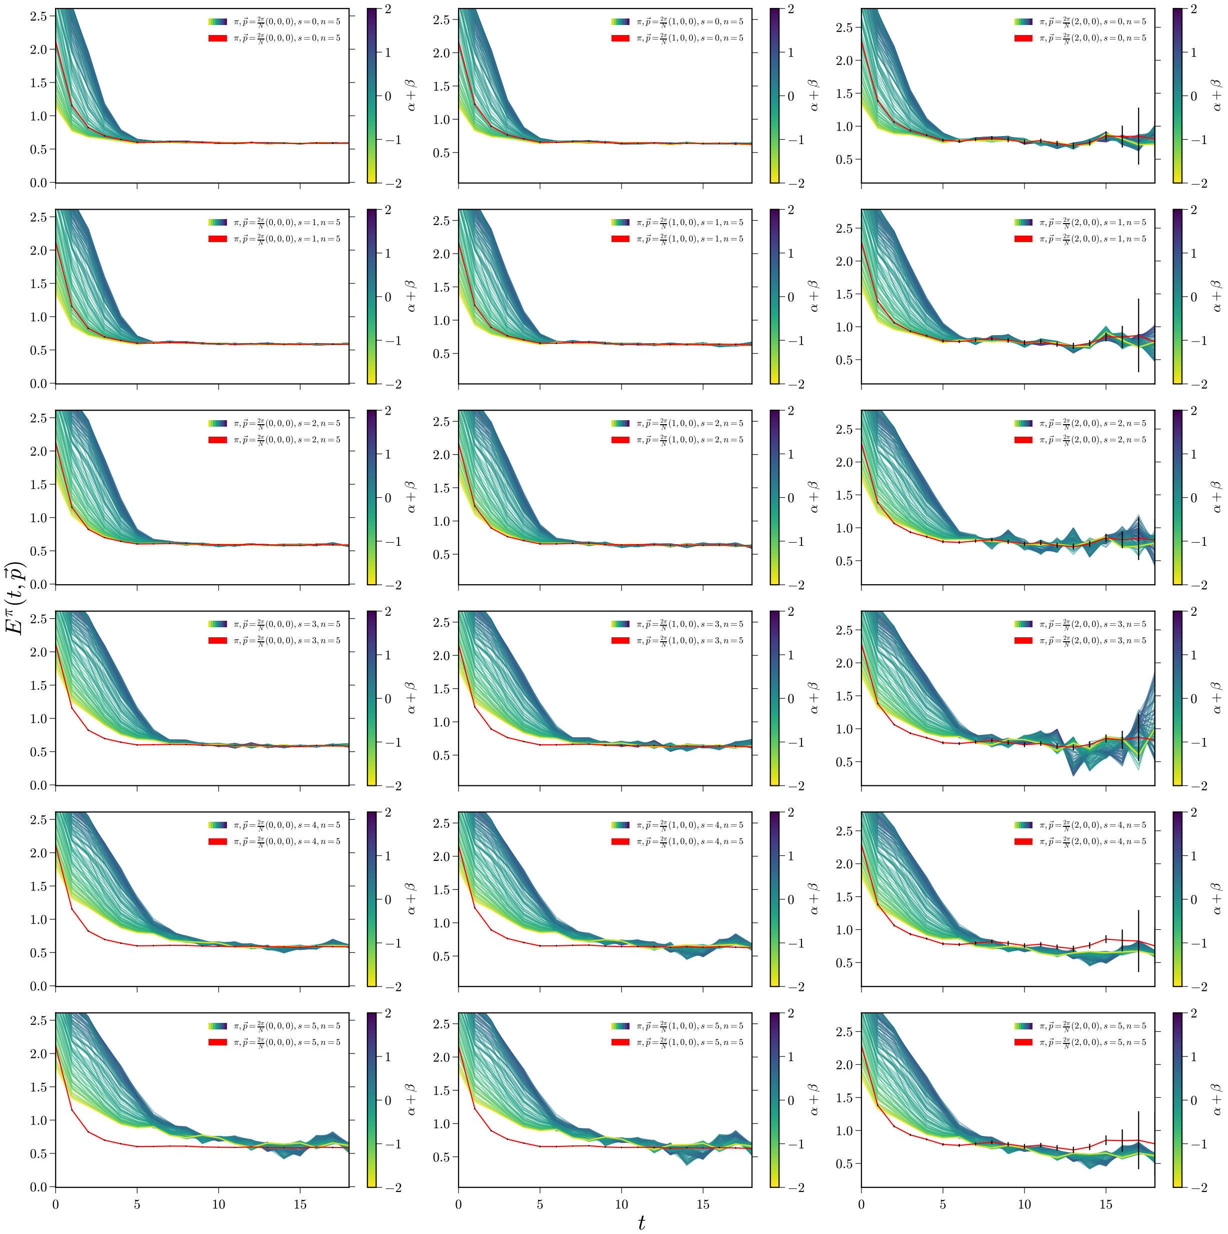

FIG. 6. Effective energy as a function of time, $E^{\pi}(t,\vec{p})$ (Eq. (18)), for varying $\alpha,\beta$ and momentum. The unsparsened result is shown in red.

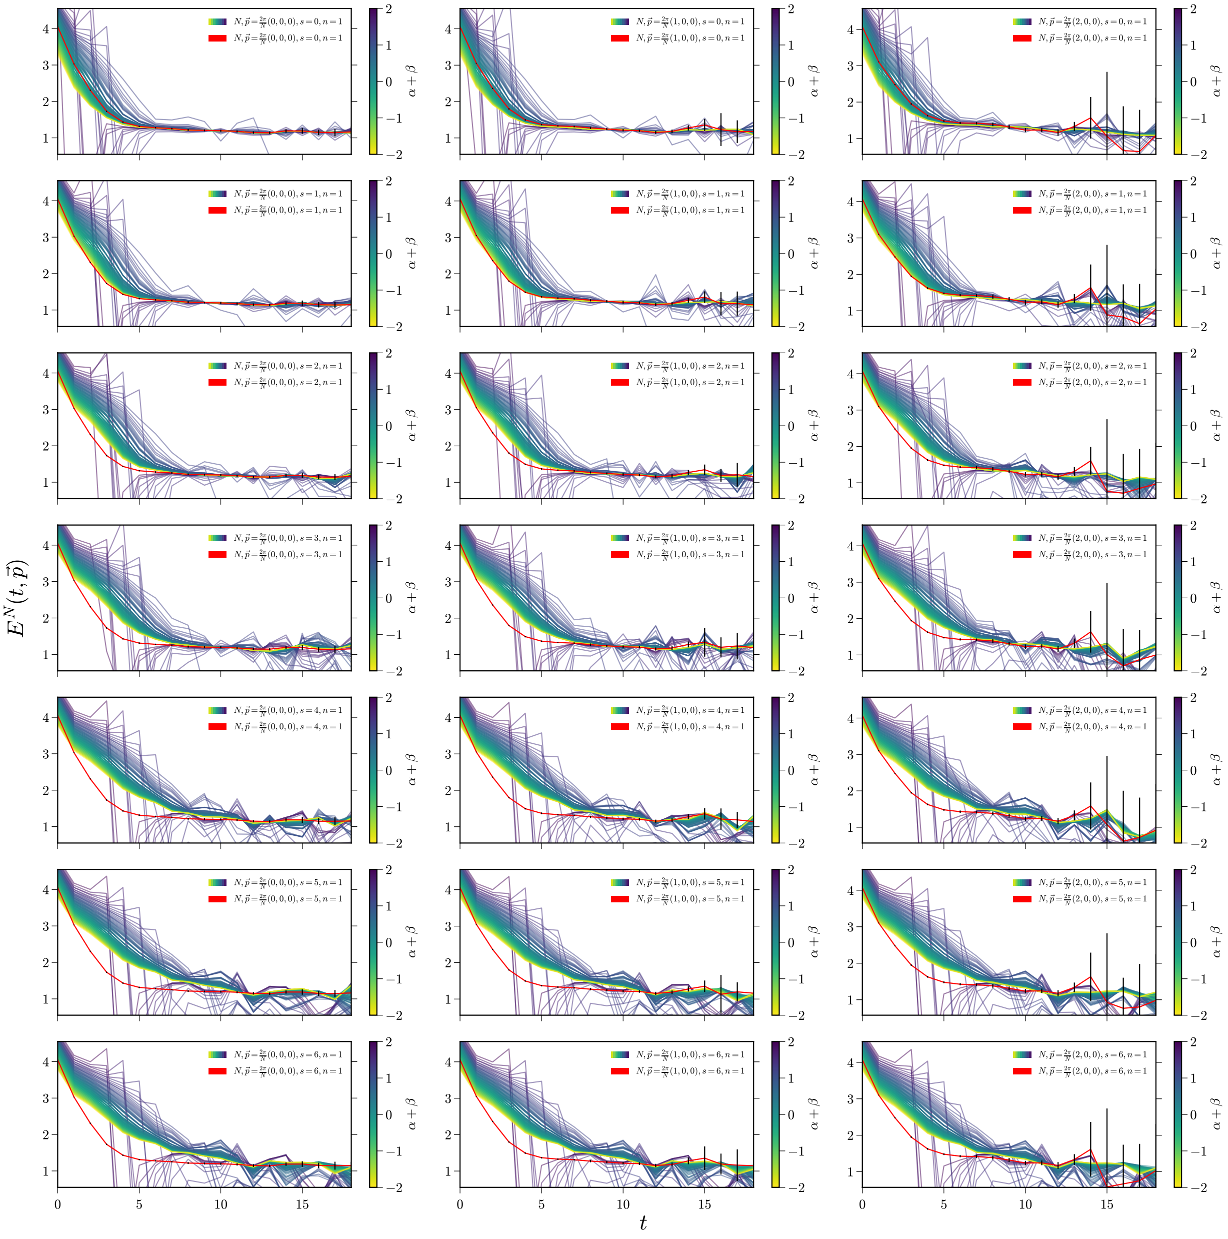

FIG. 7. Effective energy as a function of time, $E^N(t,\vec{p})$ (Eq. (18)), for varying $\alpha, \beta$ and momentum. The unsparsened result is shown in red.

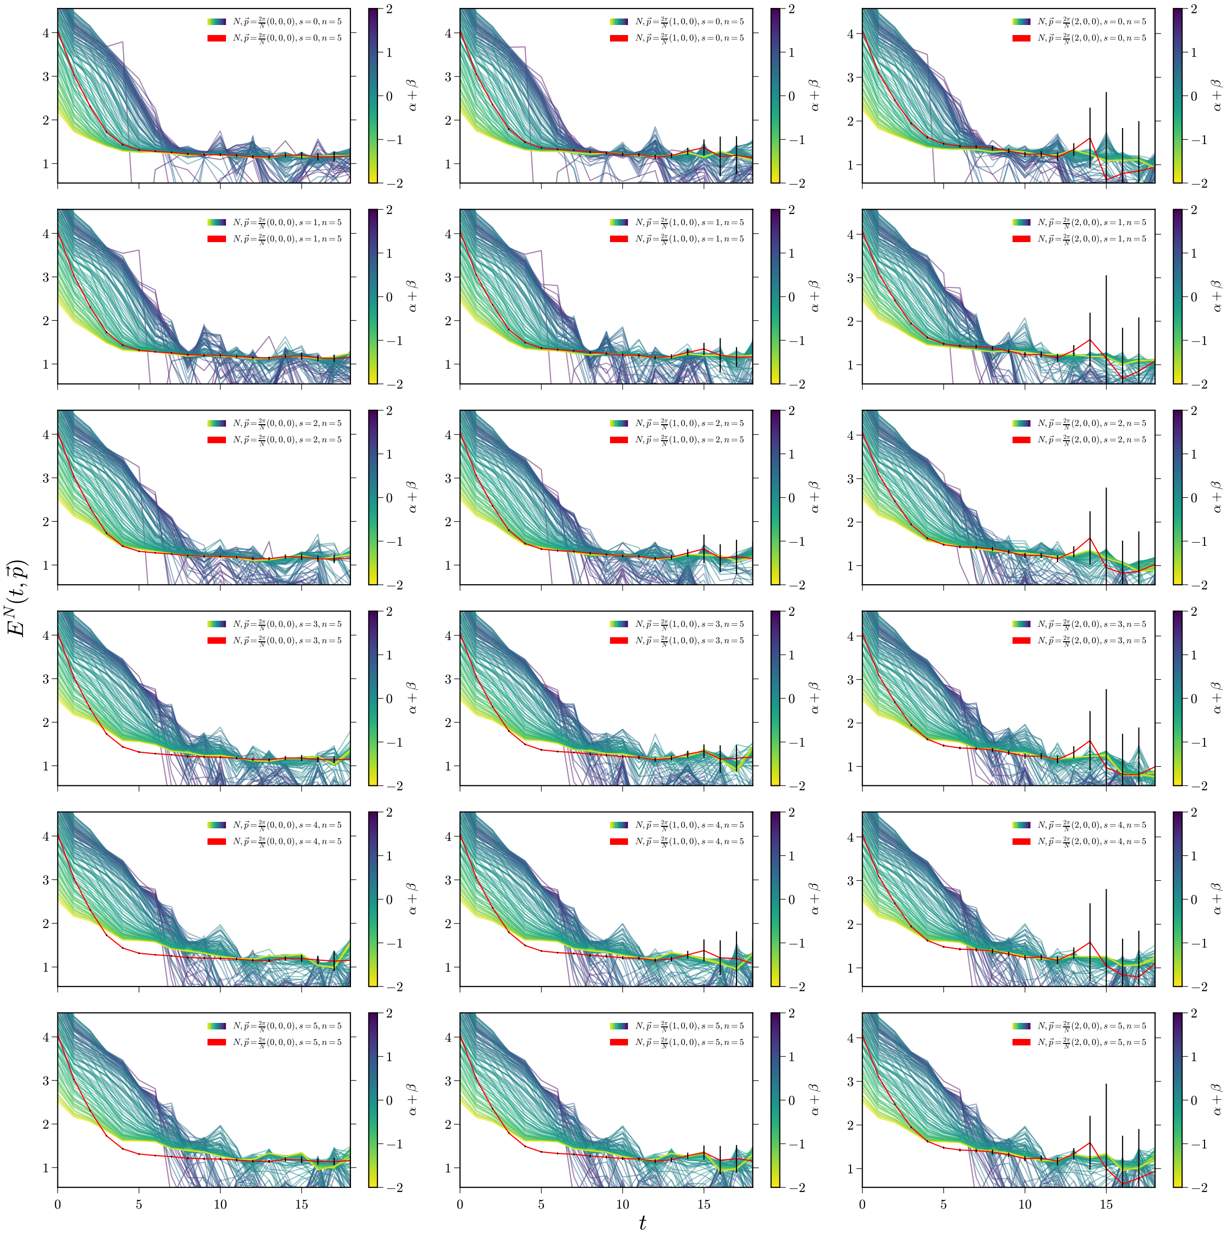


FIG. 8. Effective energy as a function of time, $E^N(t, \vec{p})$ (Eq. (18)), for varying $\alpha, \beta$ and momentum. The unsparsened result is shown in red.

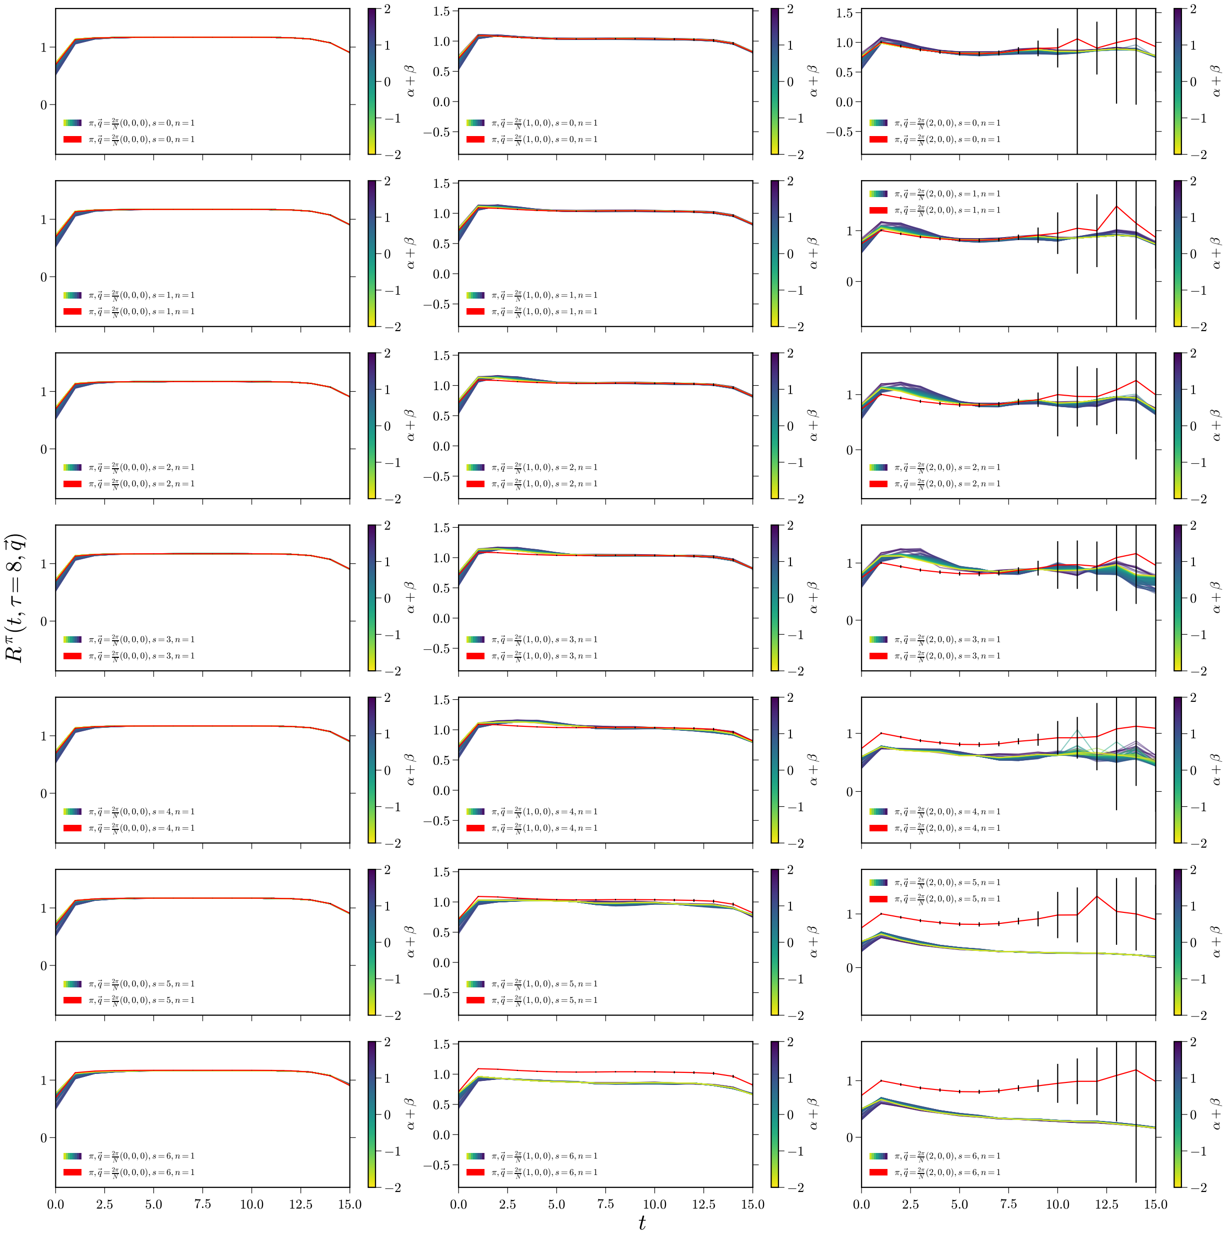

FIG. 9. Improved ratio of three- and two-point functions with $\tau = 8$, $R^{\pi}(t, \tau = 8, \vec{q})$ (Eqs. (30) and (33)), for varying $\alpha, \beta$ and momentum. The unsparsened result is shown in red.

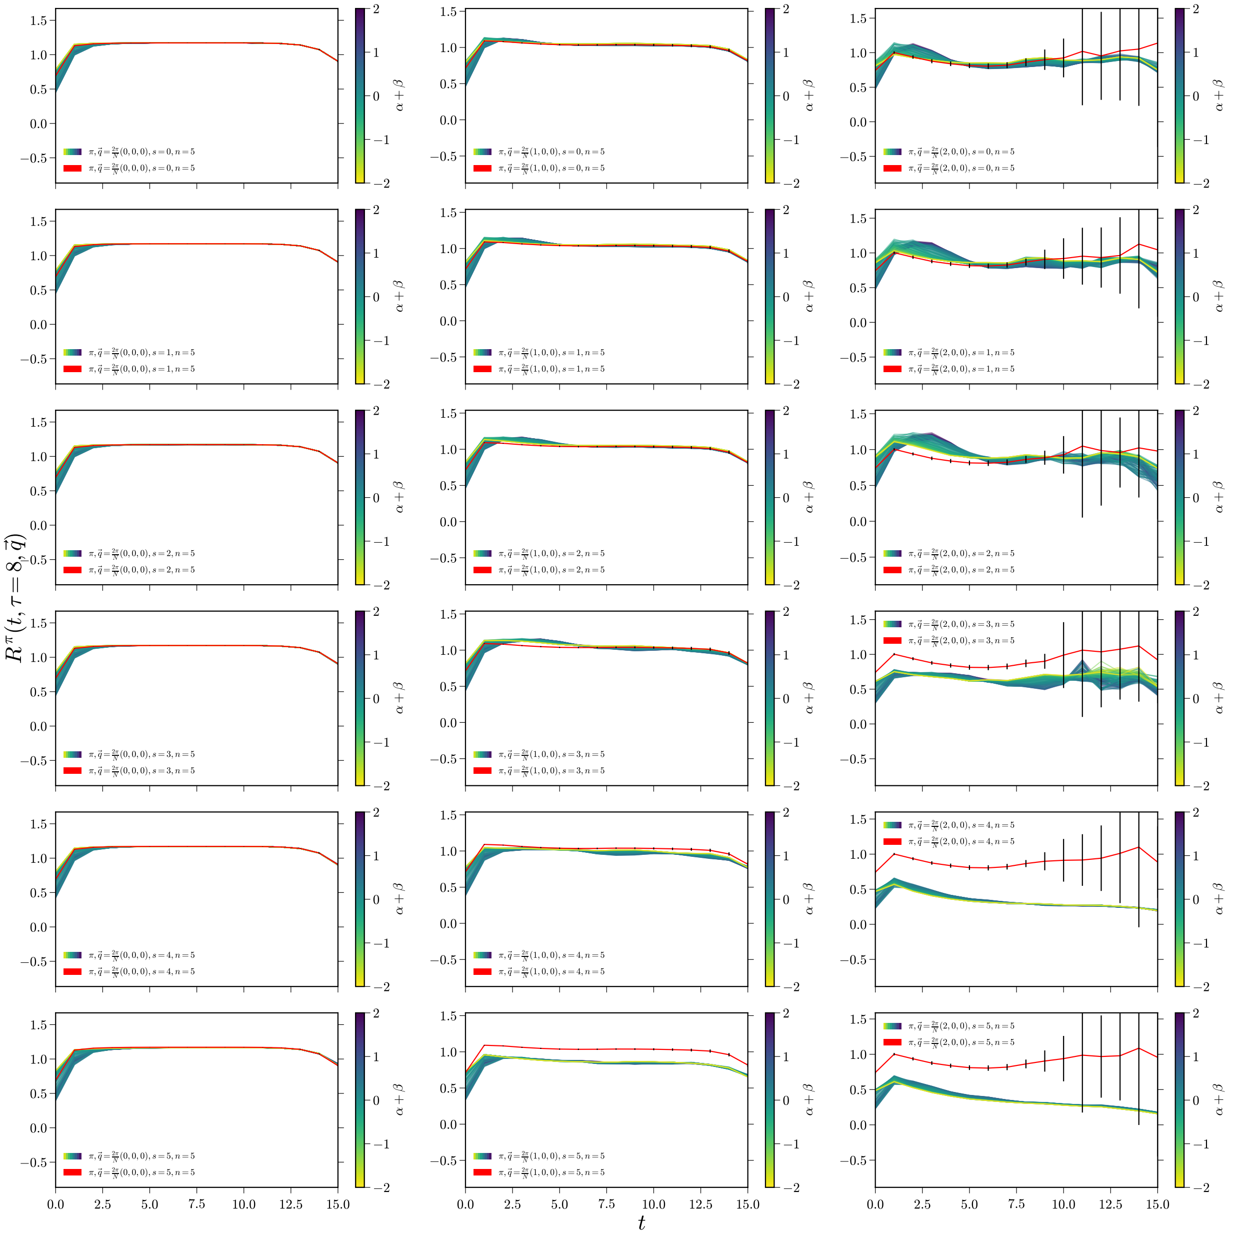

FIG. 10. Improved ratio of three- and two-point functions with $\tau = 8$, $R^{\pi}(t, \tau = 8, \vec{q})$ (Eqs. (30) and (33)), for varying $\alpha, \beta$ and momentum. The unsparsened result is shown in red.

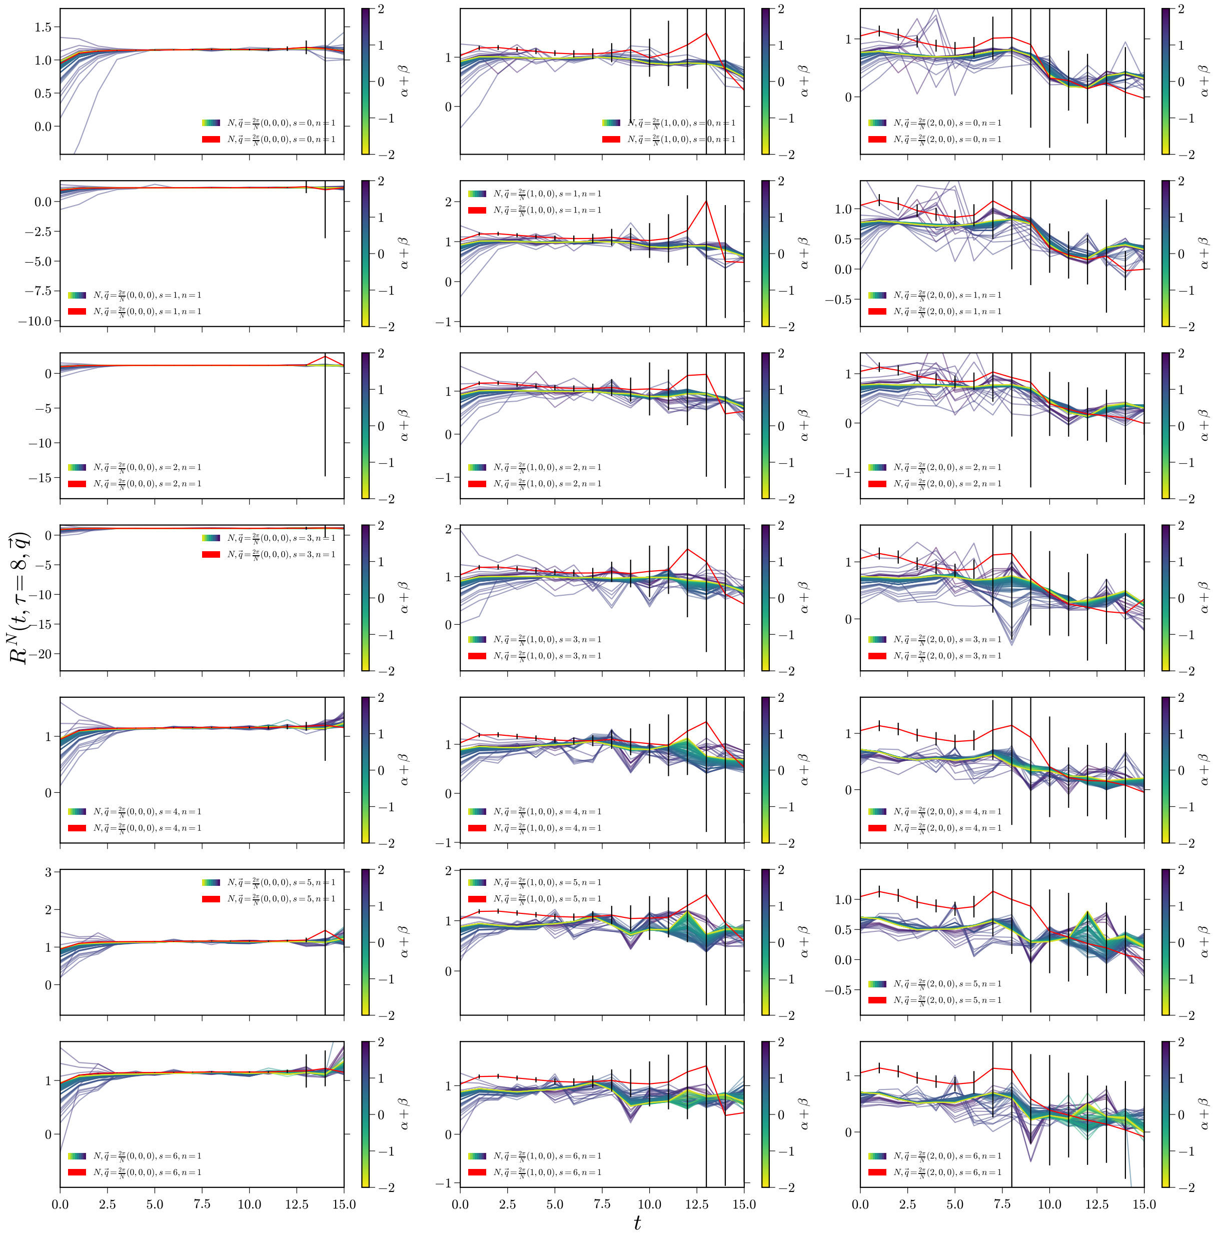


FIG. 11. Improved ratio of three- and two-point functions with $\tau = 8$, $R^N(t, \tau = 8, \vec{q})$ (Eqs. (30) and (33)), for varying $\alpha, \beta$ and momentum. The unsparsened result is shown in red.

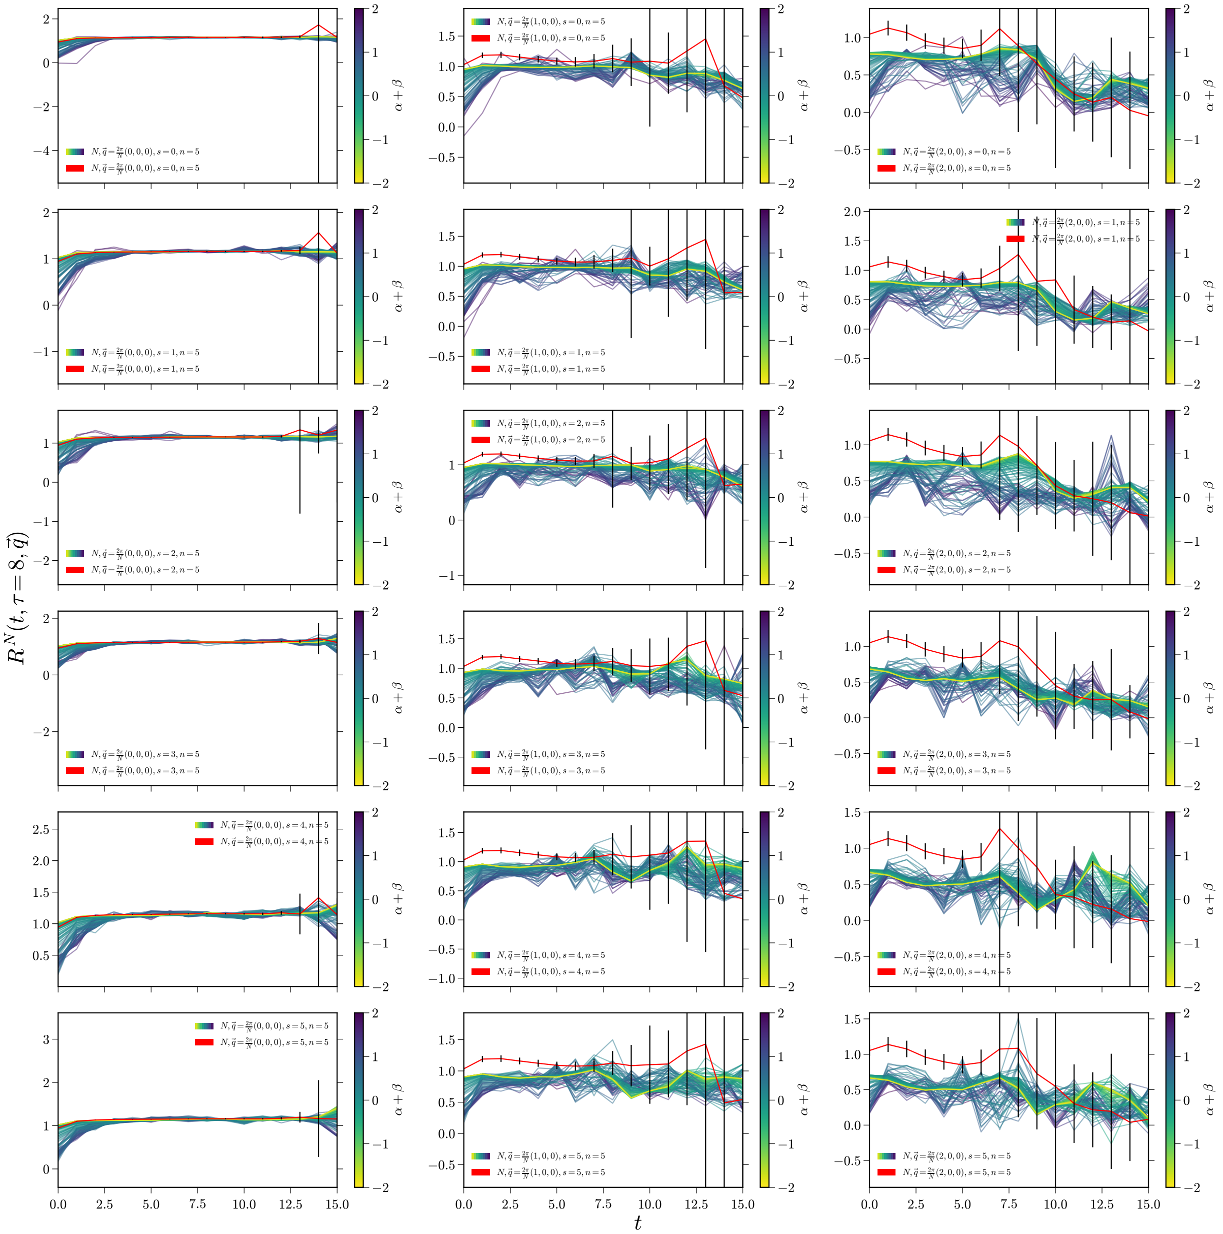

FIG. 12. Improved ratio of three- and two-point functions with $\tau = 8$, $R^N(t, \tau = 8, \vec{q})$ (Eqs. (30) and (33)), for varying $\alpha, \beta$ and momentum. The unsparsened result is shown in red.

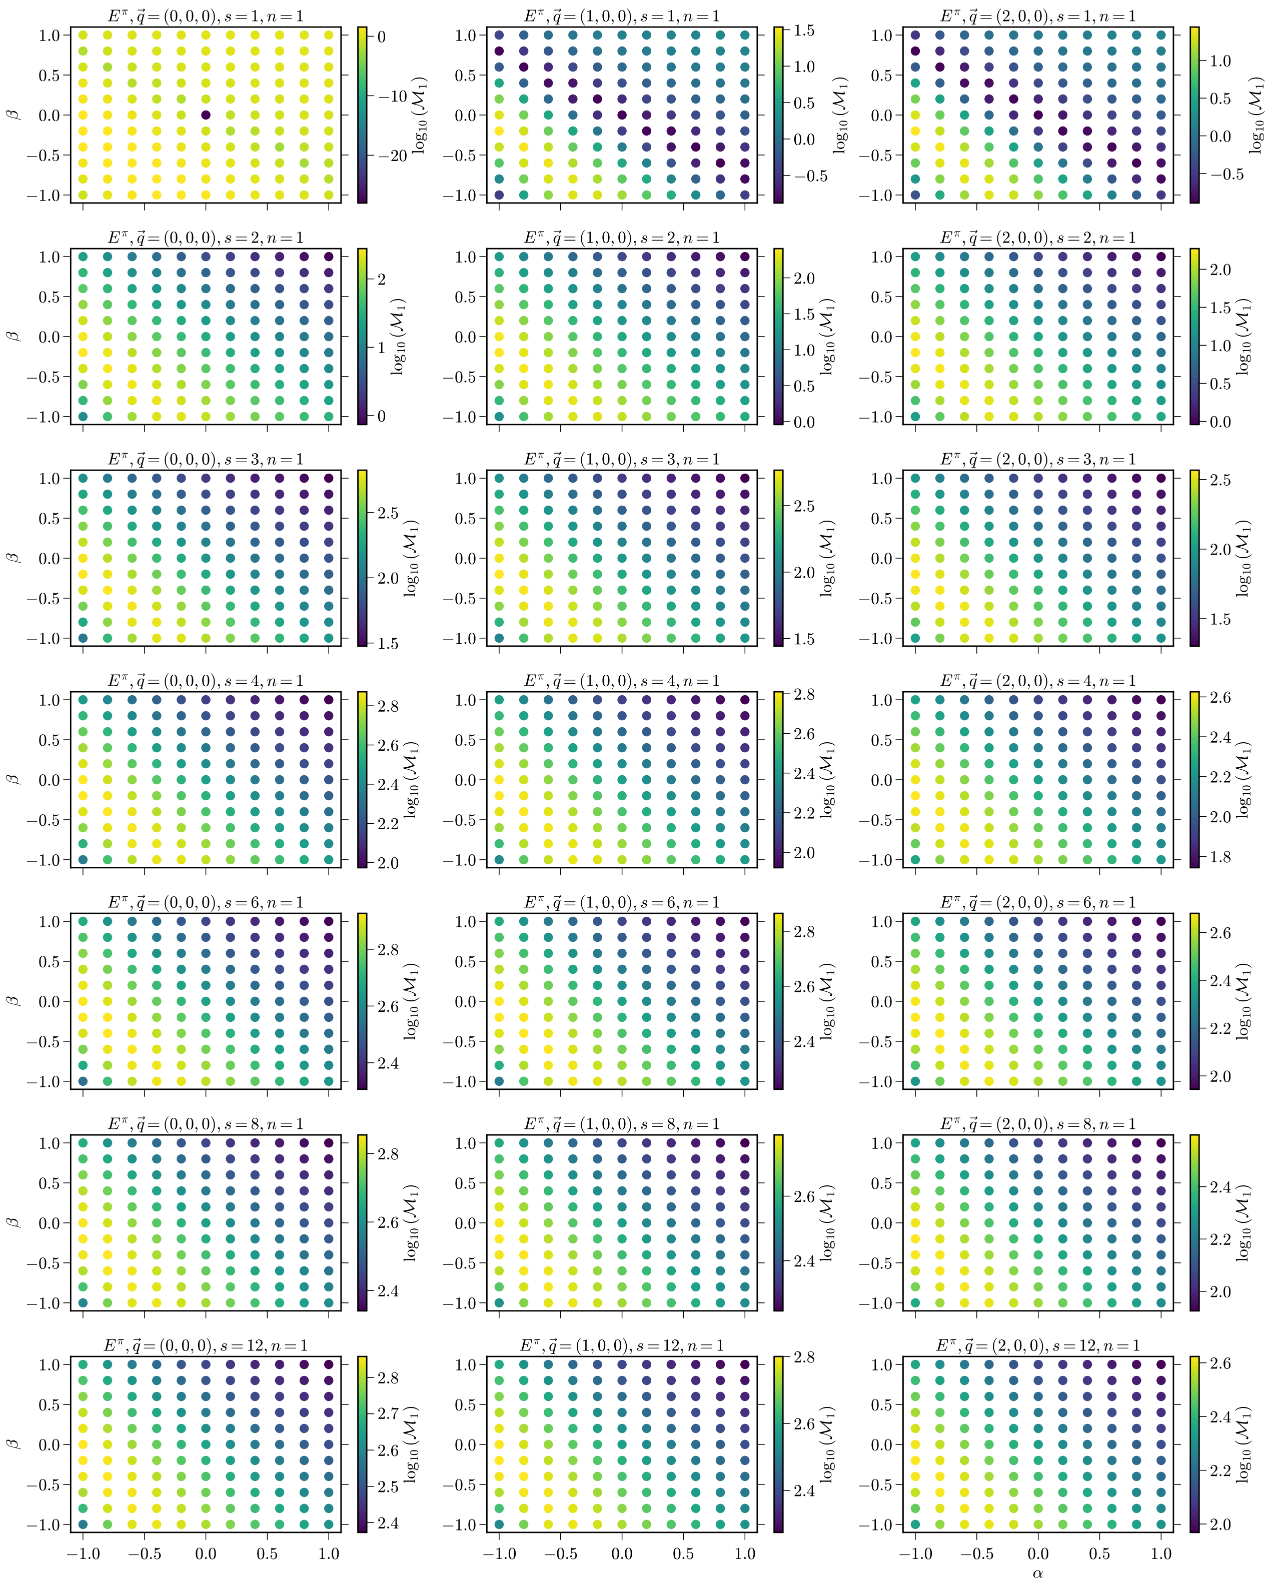


FIG. 13. Metric $\mathcal{M}_1$ (Eq. (25)), for the pion effective energy as a function of $\alpha, \beta$. In this figure, there are $n = 1$ blocking factor, three different values of momentum, and all 7 possible decimation factors.

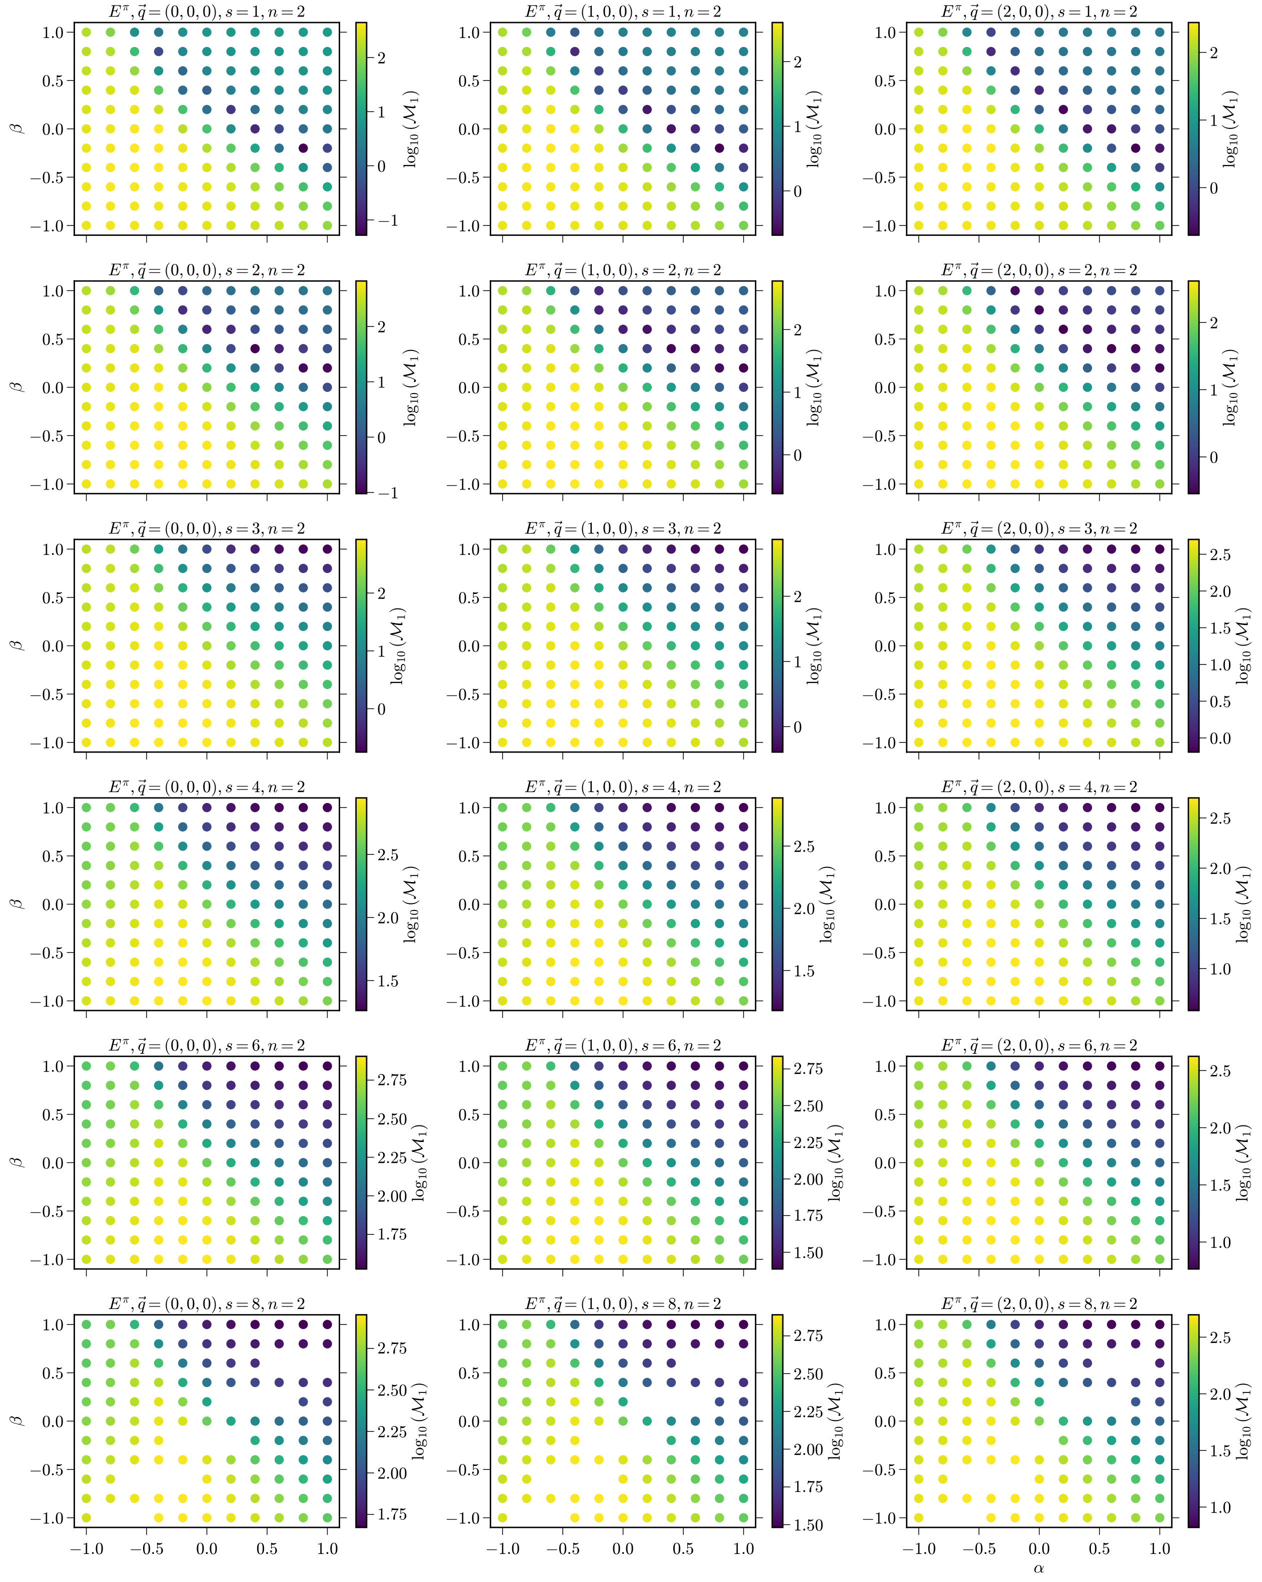

FIG. 14. Metric $\mathcal{M}_1$ (Eq. (25)), for the pion effective energy as a function of $\alpha, \beta$. In this figure, there are $n = 2$ blocking factor, three different values of momentum, and all 7 possible decimation factors.

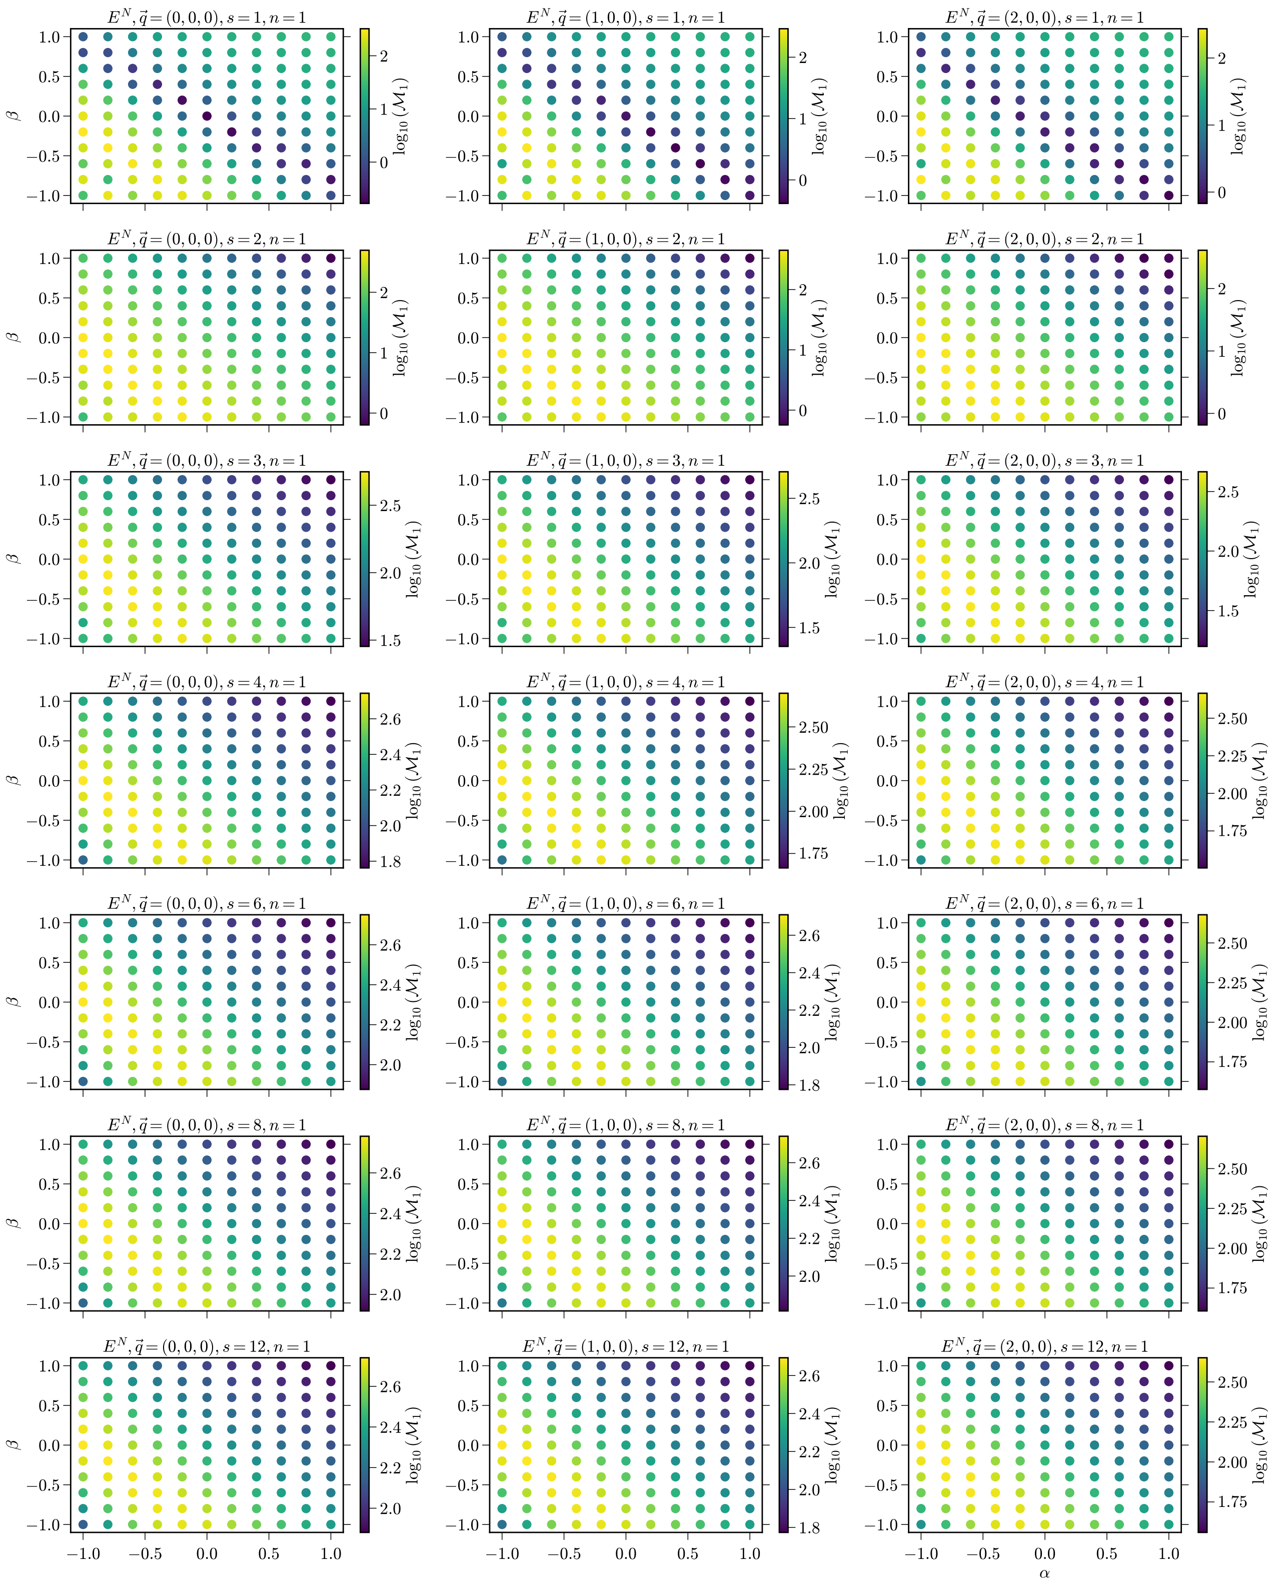


FIG. 15. Metric $\mathcal{M}_1$ (Eq. (25)), for the proton effective energy as a function of $\alpha, \beta$. In this figure, there are $n = 1$ blocking factor, three different values of momentum, and all 7 possible decimation factors.

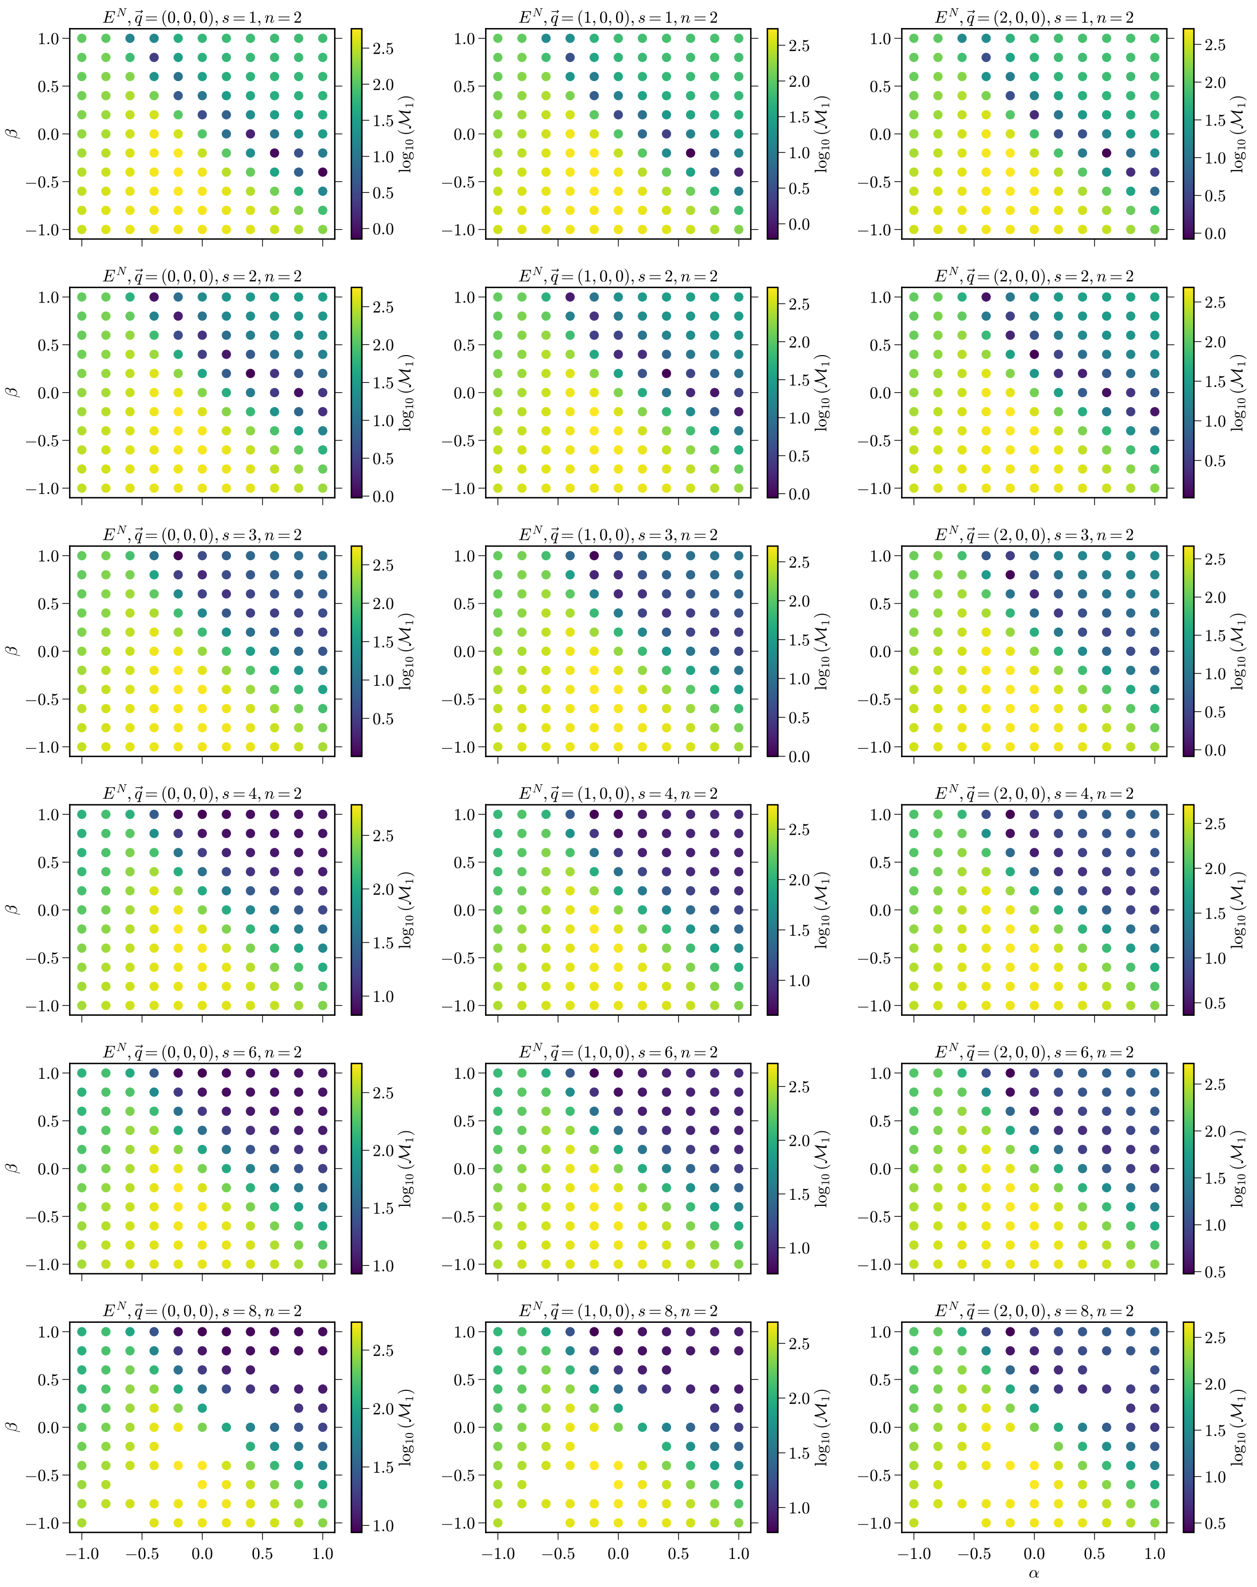


FIG. 16. Metric $\mathcal{M}_1$ (Eq. (25)), for the proton effective energy as a function of $\alpha, \beta$. In this figure, there are $n = 2$ blocking factor, three different values of momentum, and all 7 possible decimation factors.

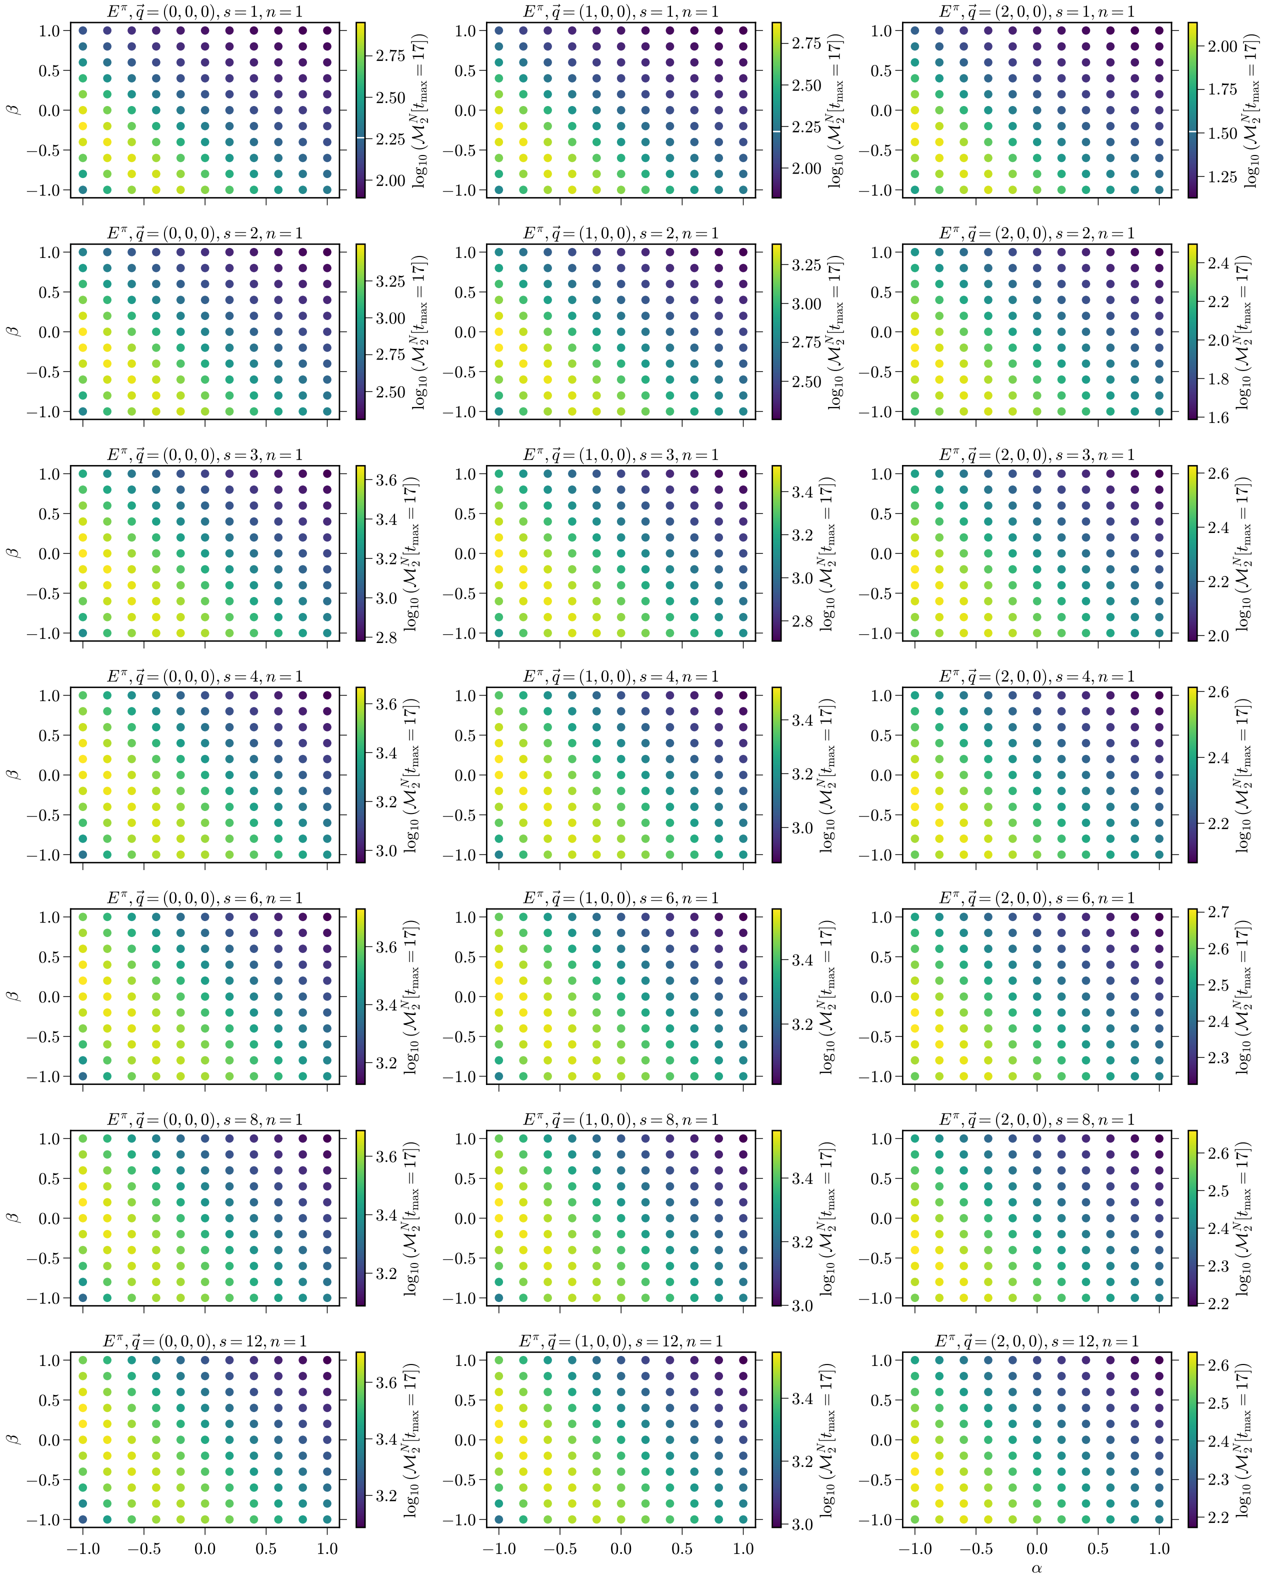

FIG. 17. Metric $\mathcal{M}_2$ (Eq. (26)), for the pion effective energy as a function of $\alpha, \beta$. In this figure, there are $n = 1$ blocking factor, three different values of momentum, and all 7 possible decimation factors.

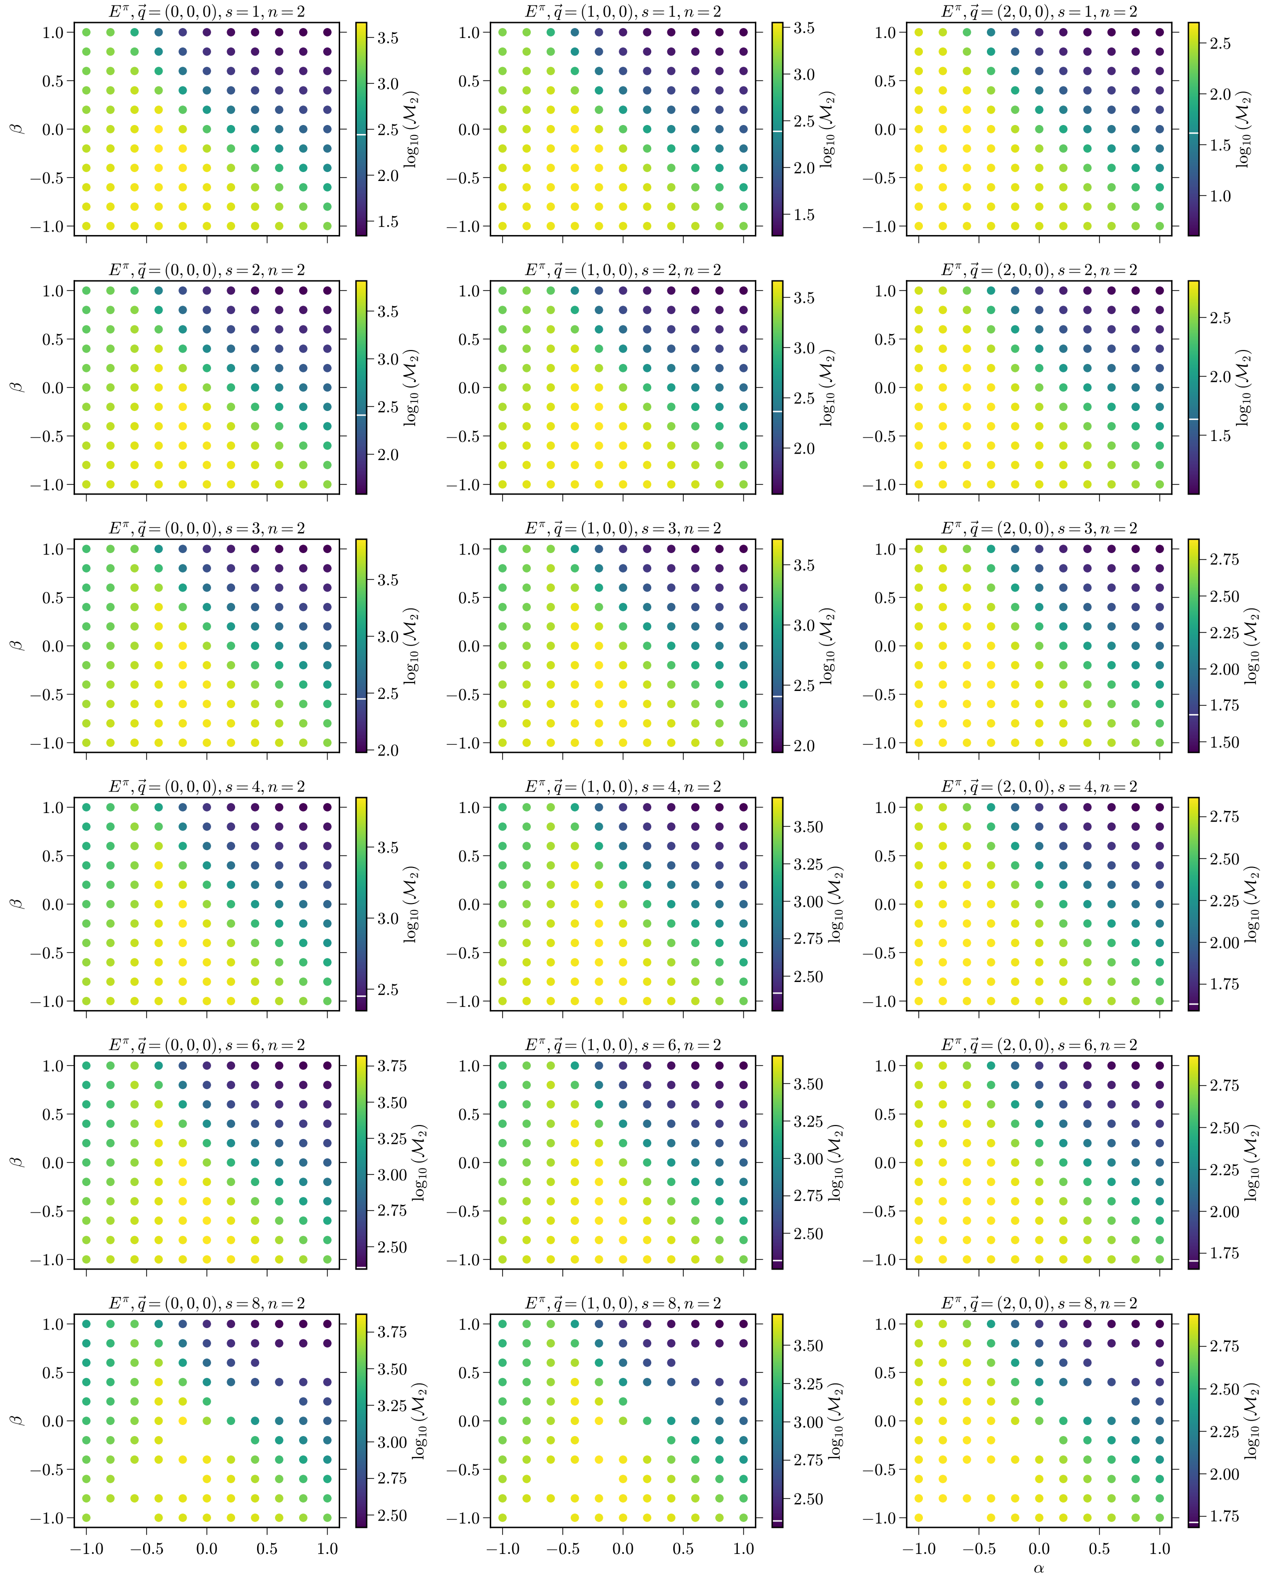


FIG. 18. Metric $\mathcal{M}_2$ (Eq. (26)), for the pion effective energy as a function of $\alpha, \beta$. In this figure, there are $n = 2$ blocking factor, three different values of momentum, and all 7 possible decimation factors.

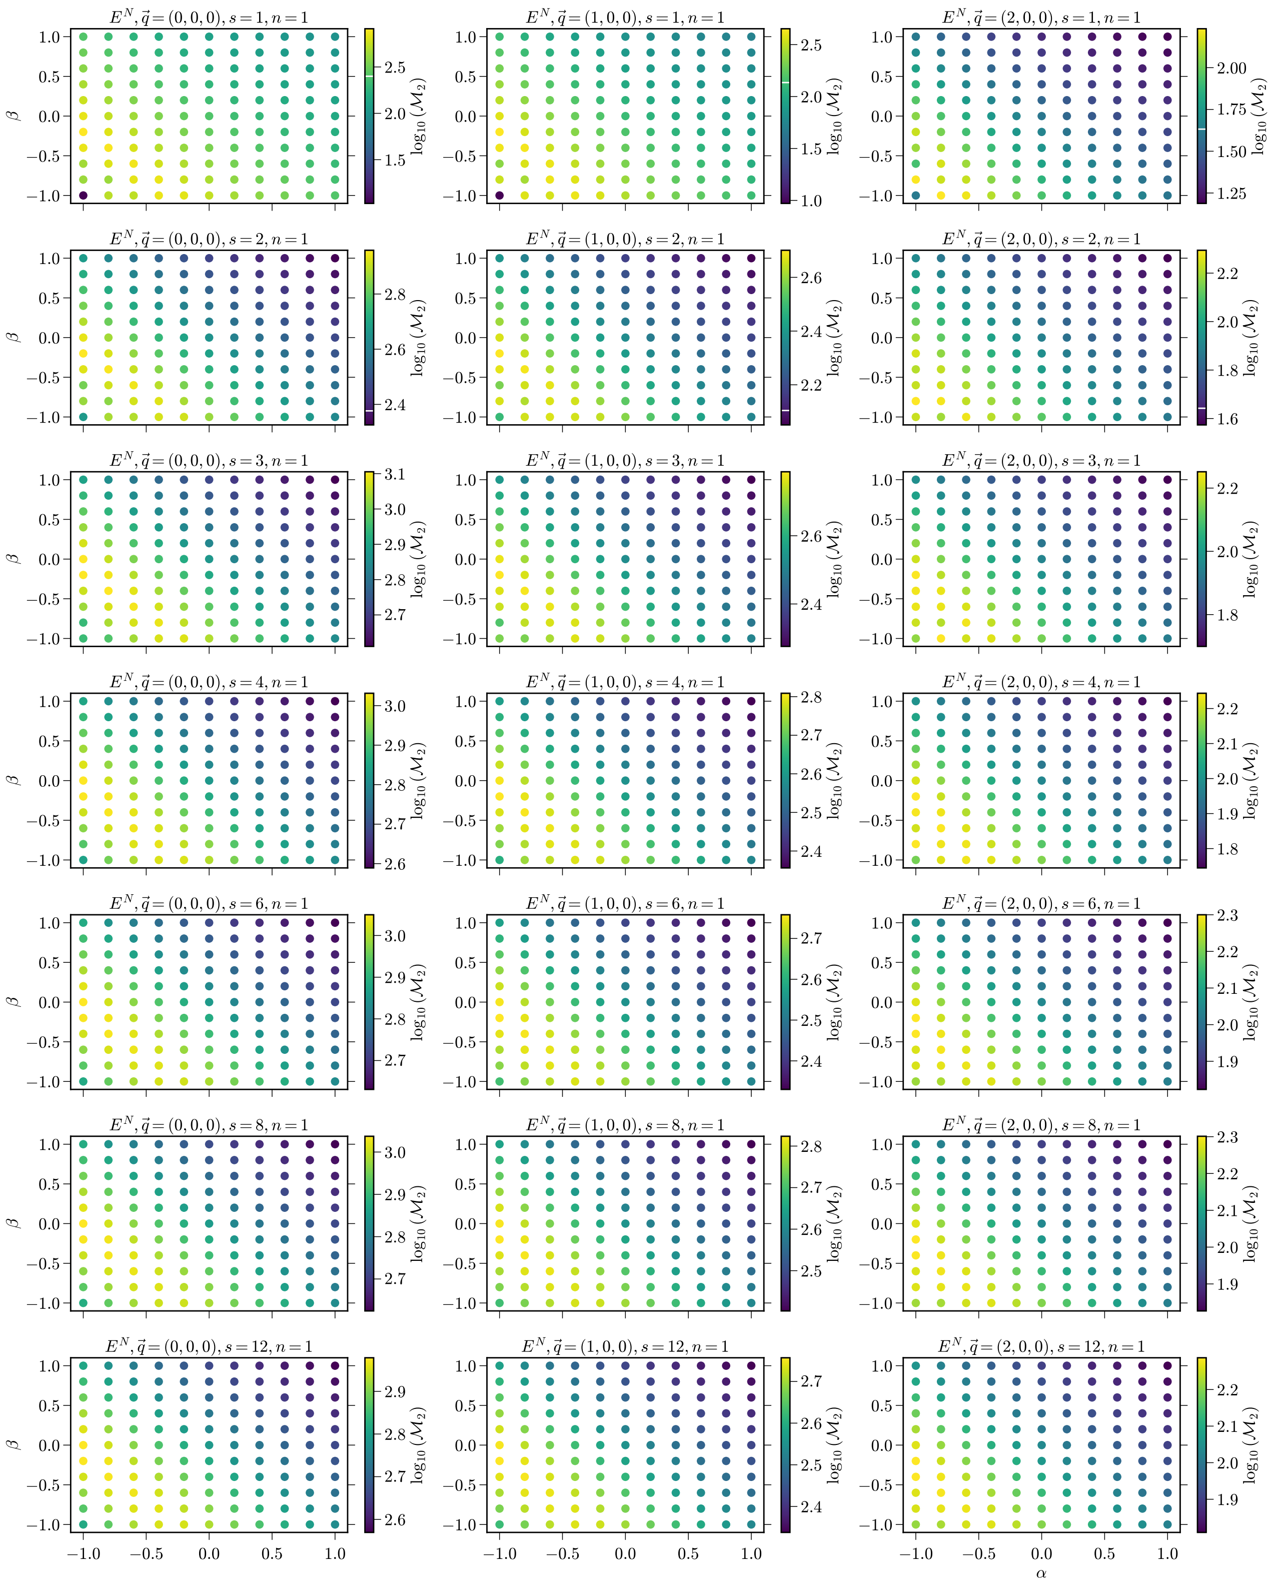


FIG. 19. Metric $\mathcal{M}_2$ (Eq. (26)), for the proton effective energy as a function of $\alpha, \beta$. In this figure, there are $n = 1$ blocking factor, three different values of momentum, and all 7 possible decimation factors.

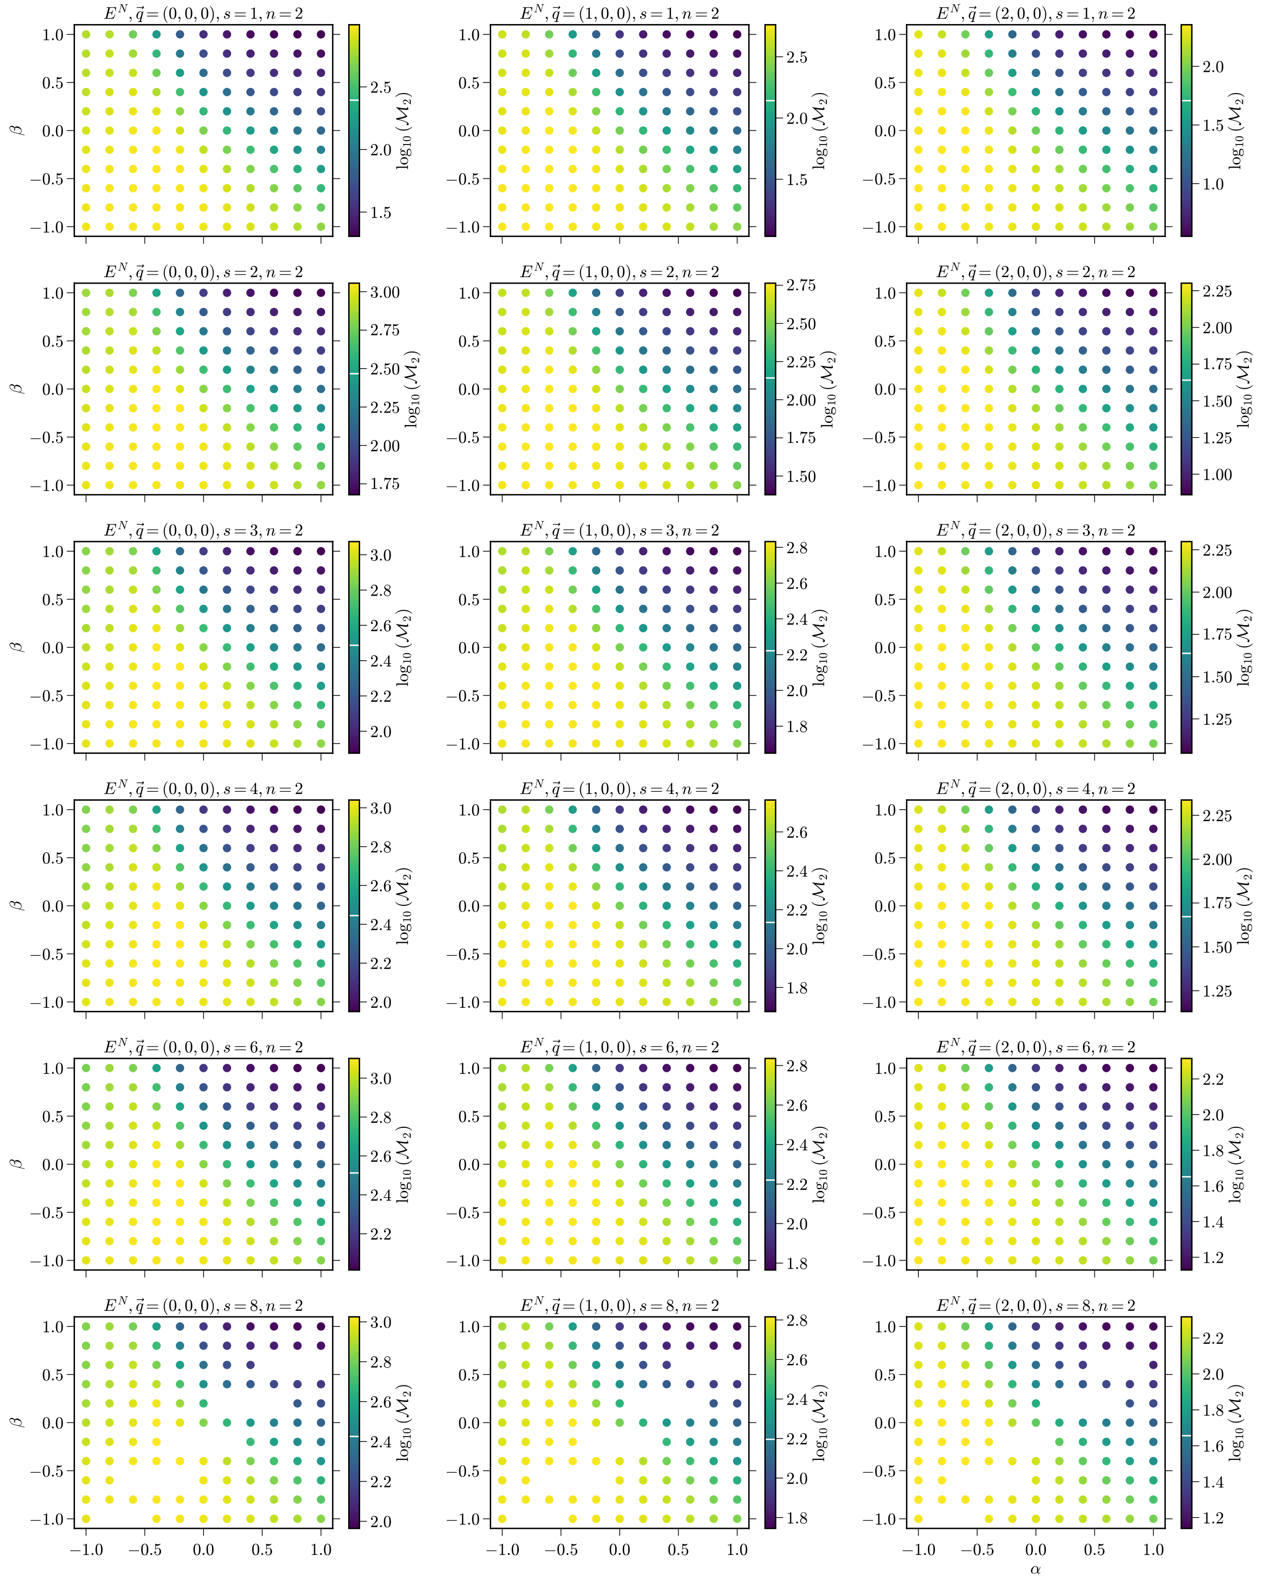


FIG. 20. Metric $\mathcal{M}_2$ (Eq. (26)), for the proton effective energy as a function of $\alpha, \beta$. In this figure, there are $n = 2$ blocking factor, three different values of momentum, and all 7 possible decimation factors.

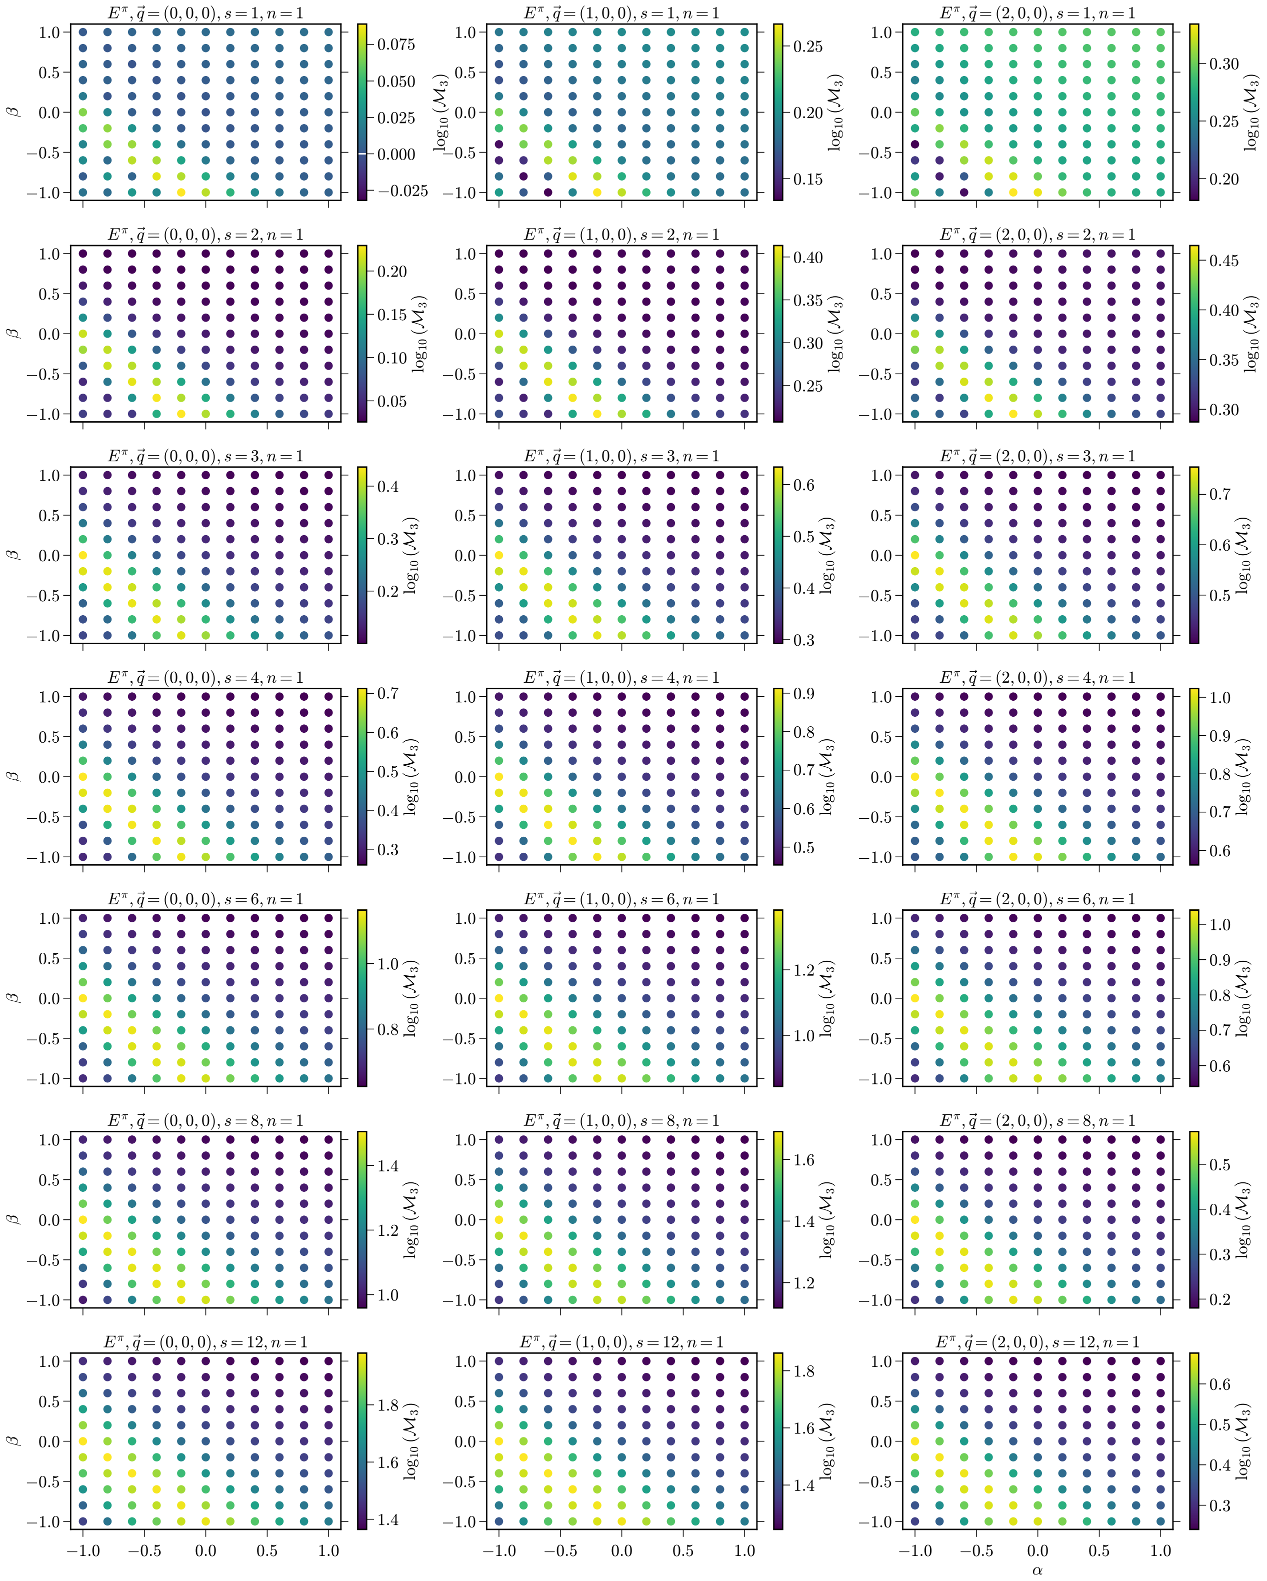


FIG. 21. Metric $\mathcal{M}_3$ (Eq. (27)), for the pion effective energy as a function of $\alpha, \beta$. In this figure, there are $n = 1$ blocking factor, three different values of momentum, and all 7 possible decimation factors.

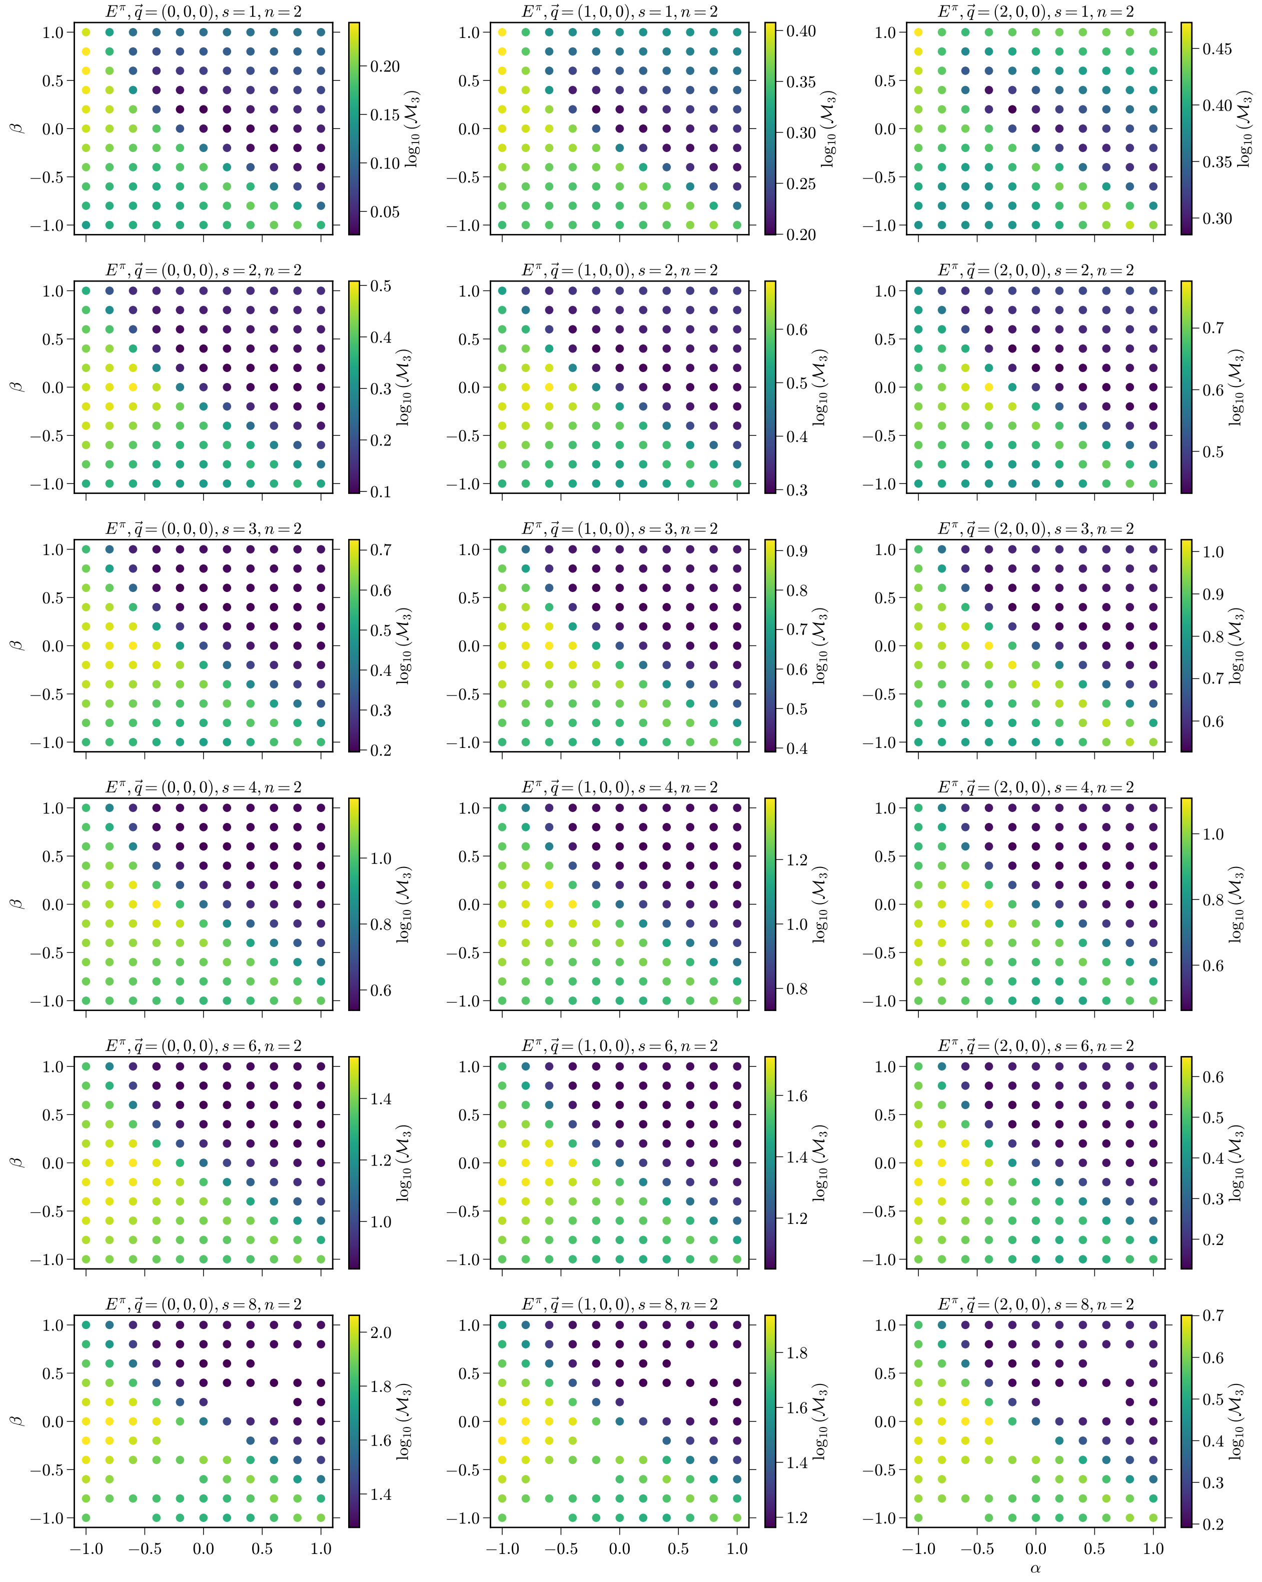

FIG. 22. Metric $\mathcal{M}_3$ (Eq. (27)), for the pion effective energy as a function of $\alpha, \beta$. In this figure, there are $n = 2$ blocking factor, three different values of momentum, and all 7 possible decimation factors.

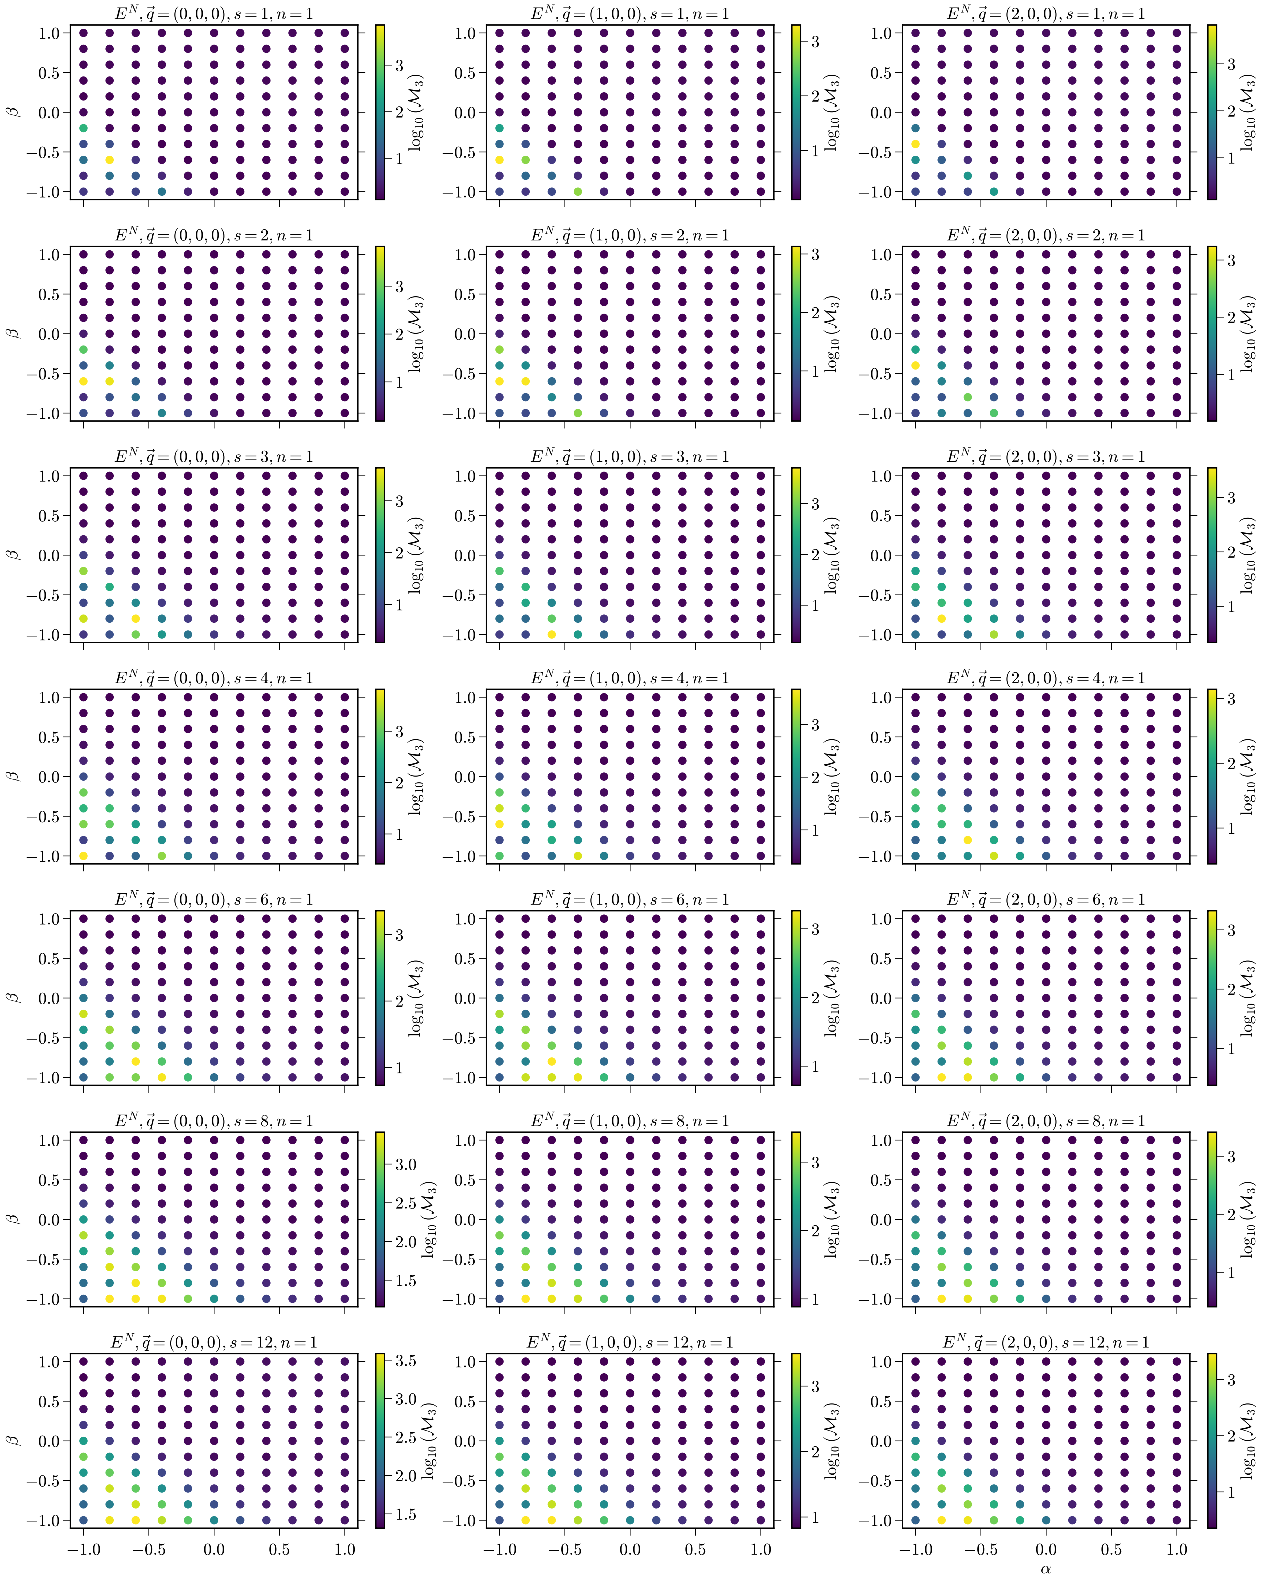


FIG. 23. Metric $\mathcal{M}_3$ (Eq. (27)), for the proton effective energy as a function of $\alpha, \beta$. In this figure, there are $n = 1$ blocking factor, three different values of momentum, and all 7 possible decimation factors.

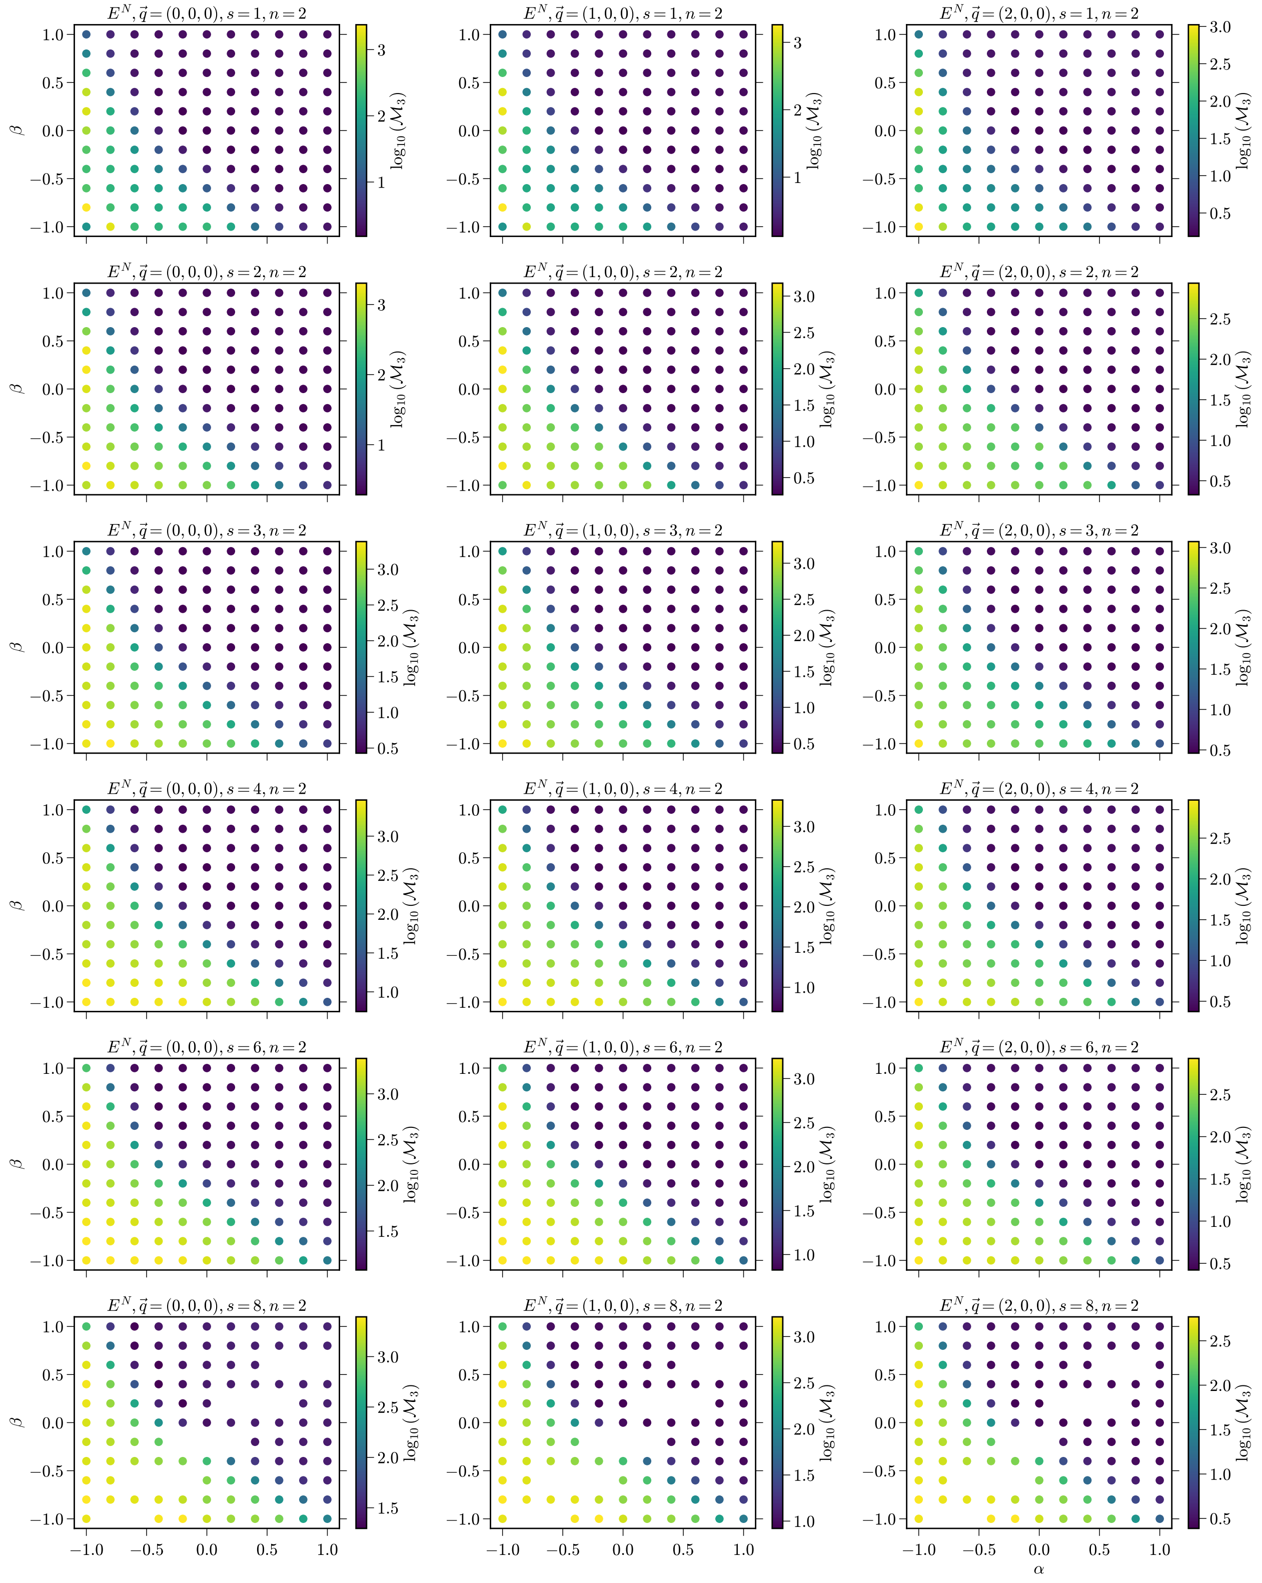


FIG. 24. Metric $\mathcal{M}_3$ (Eq. (27)), for the proton effective energy as a function of $\alpha, \beta$. In this figure, there are $n = 2$ blocking factor, three different values of momentum, and all 7 possible decimation factors.

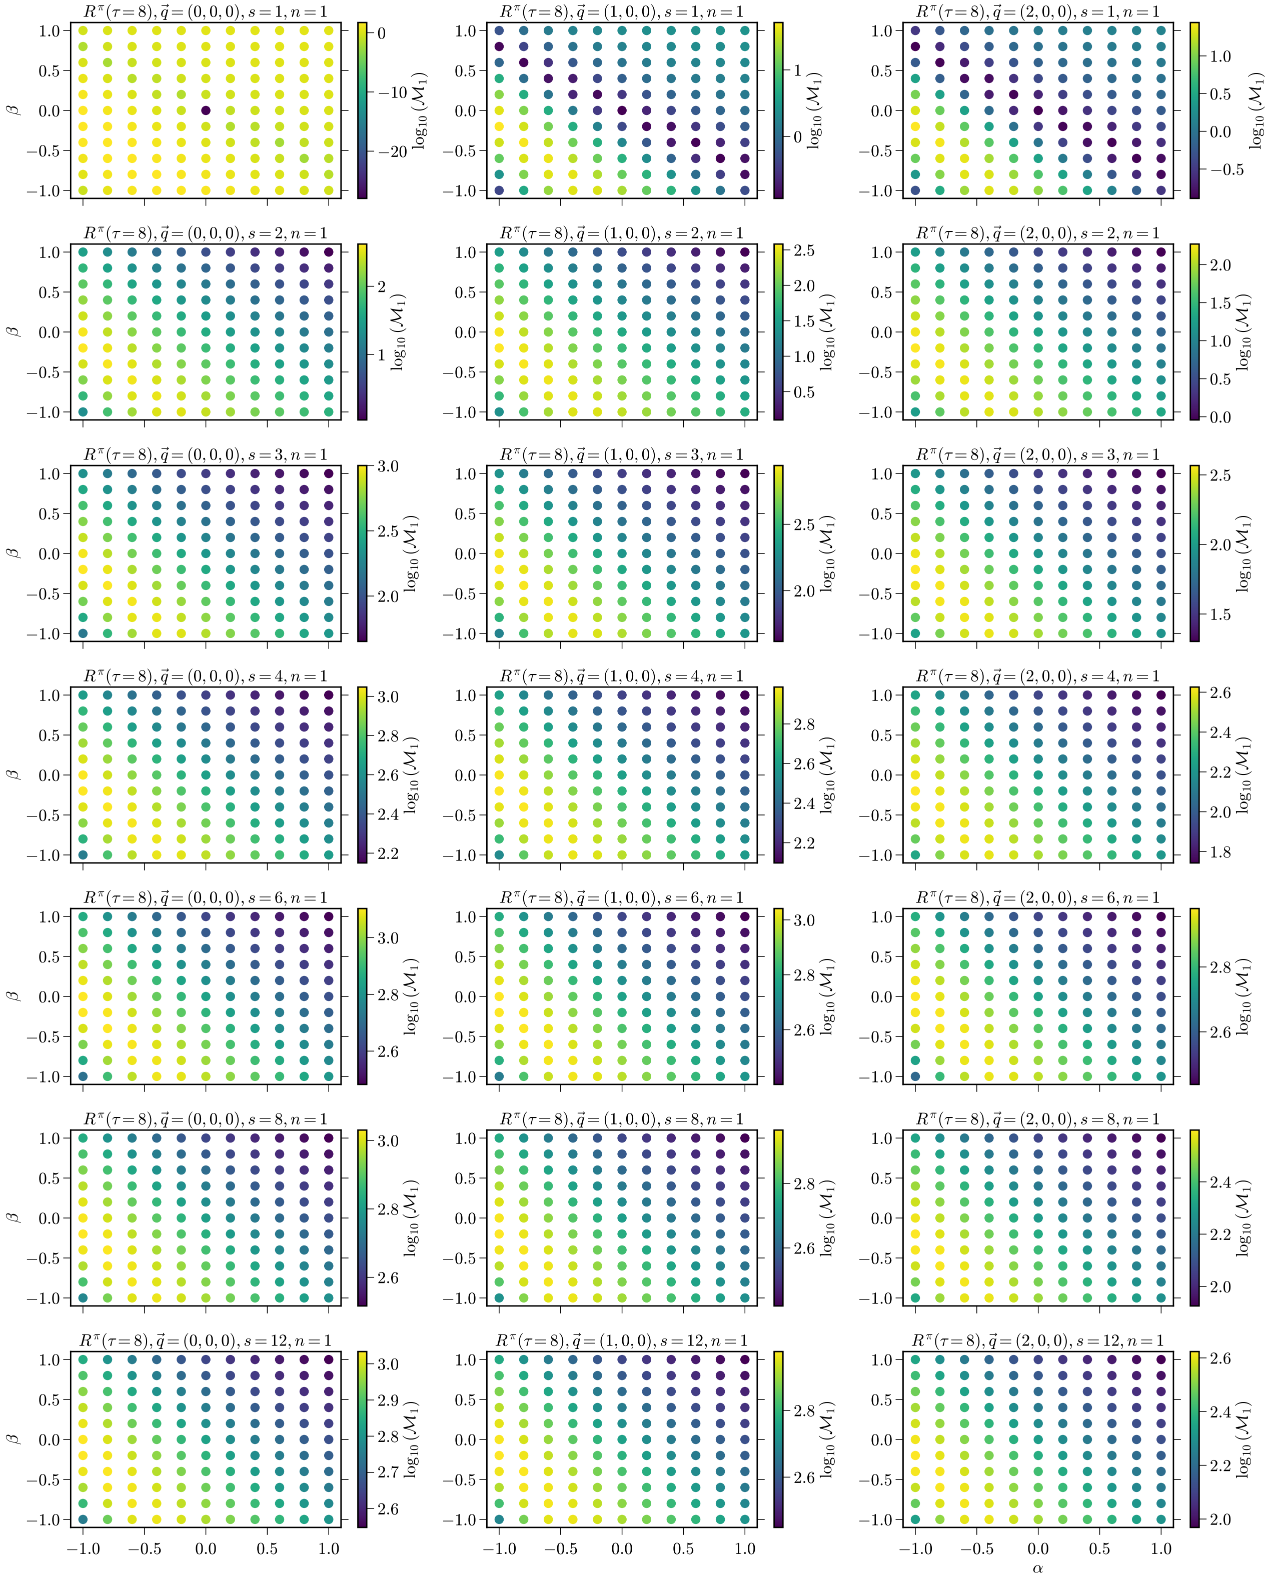

FIG. 25. Metric $\mathcal{M}_1$ (Eq. (25)), for the pion optimized ratio of two-point and three-point functions as a function of $\alpha, \beta$. In this figure, there are $n = 1$ blocking factor, three different values of momentum, and all 7 possible decimation factors.

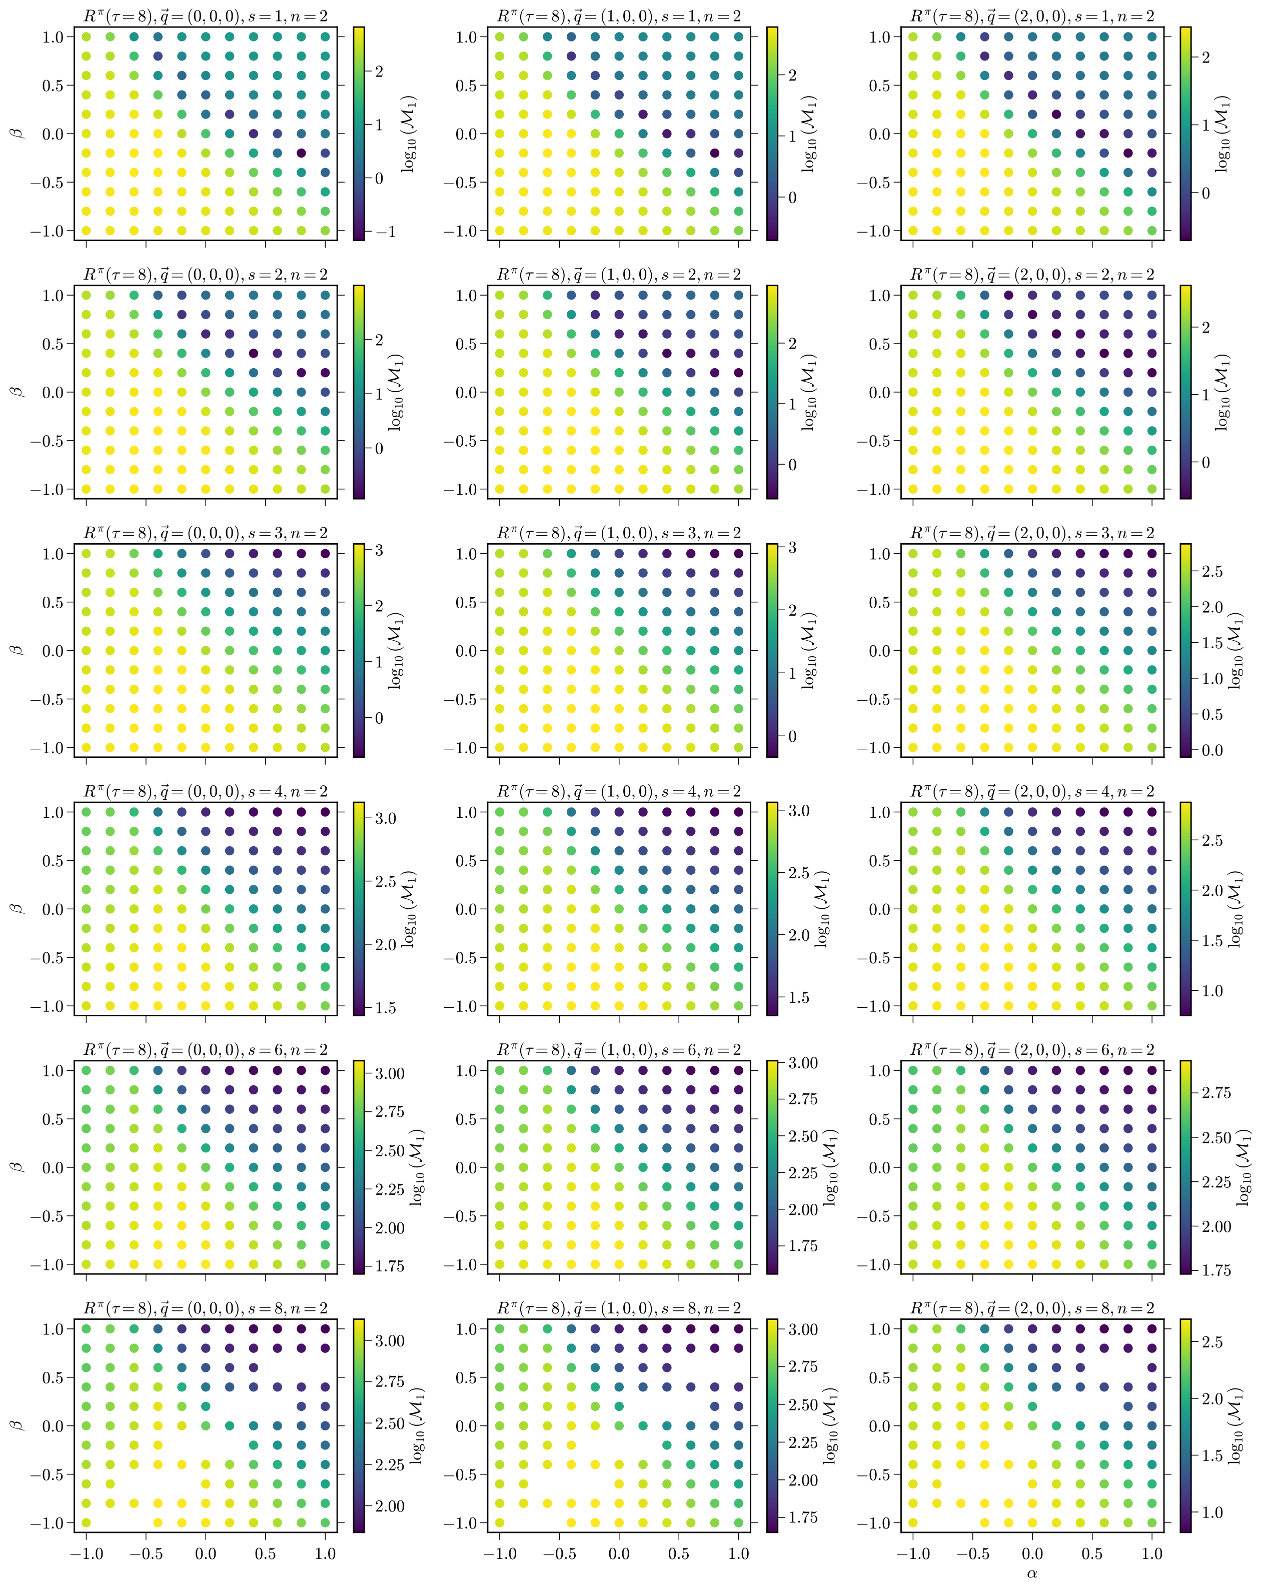

FIG. 26. Metric $\mathcal{M}_1$ (Eq. (25)), for the pion optimized ratio of two-point and three-point functions as a function of $\alpha, \beta$. In this figure, there are $n = 2$ blocking factor, three different values of momentum, and all 7 possible decimation factors.

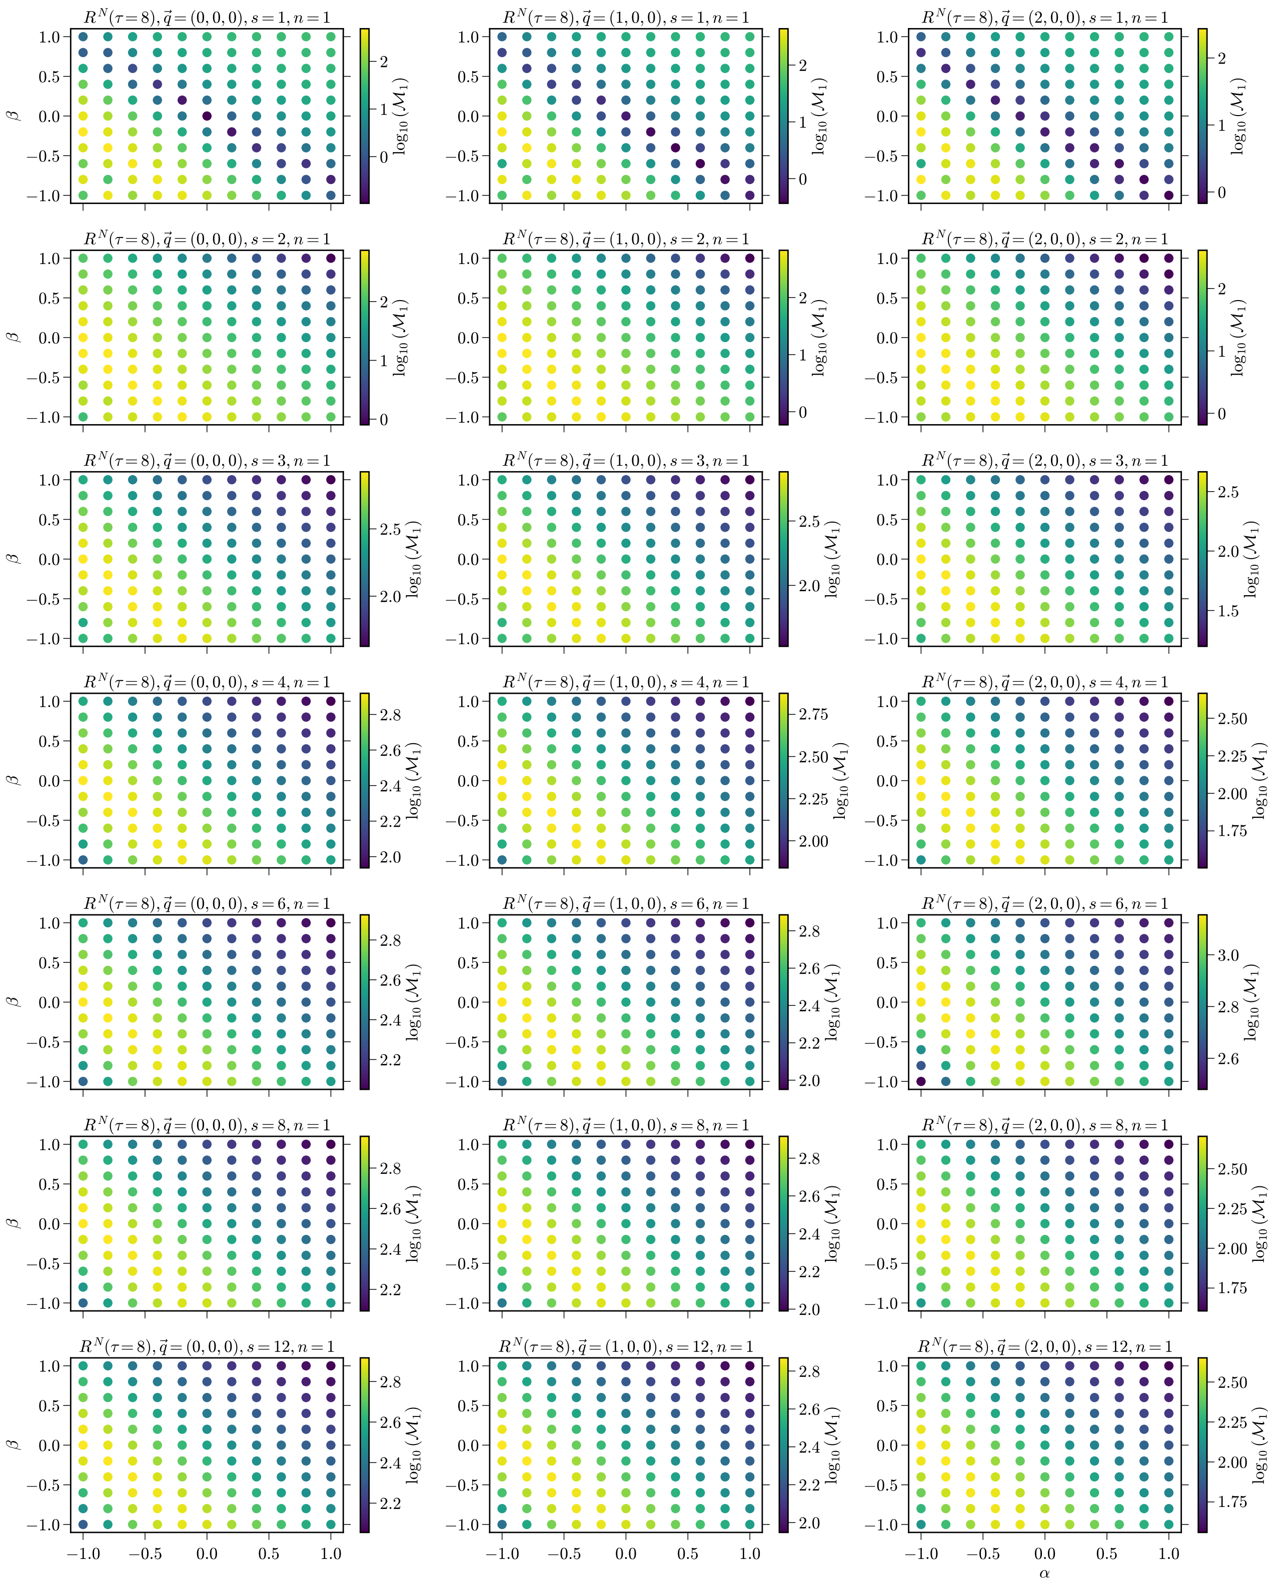


FIG. 27. Metric $\mathcal{M}_1$ (Eq. (25)), for the proton optimized ratio of two-point and three-point functions as a function of $\alpha, \beta$. In this figure, there are $n = 1$ blocking factor, three different values of momentum, and all 7 possible decimation factors.

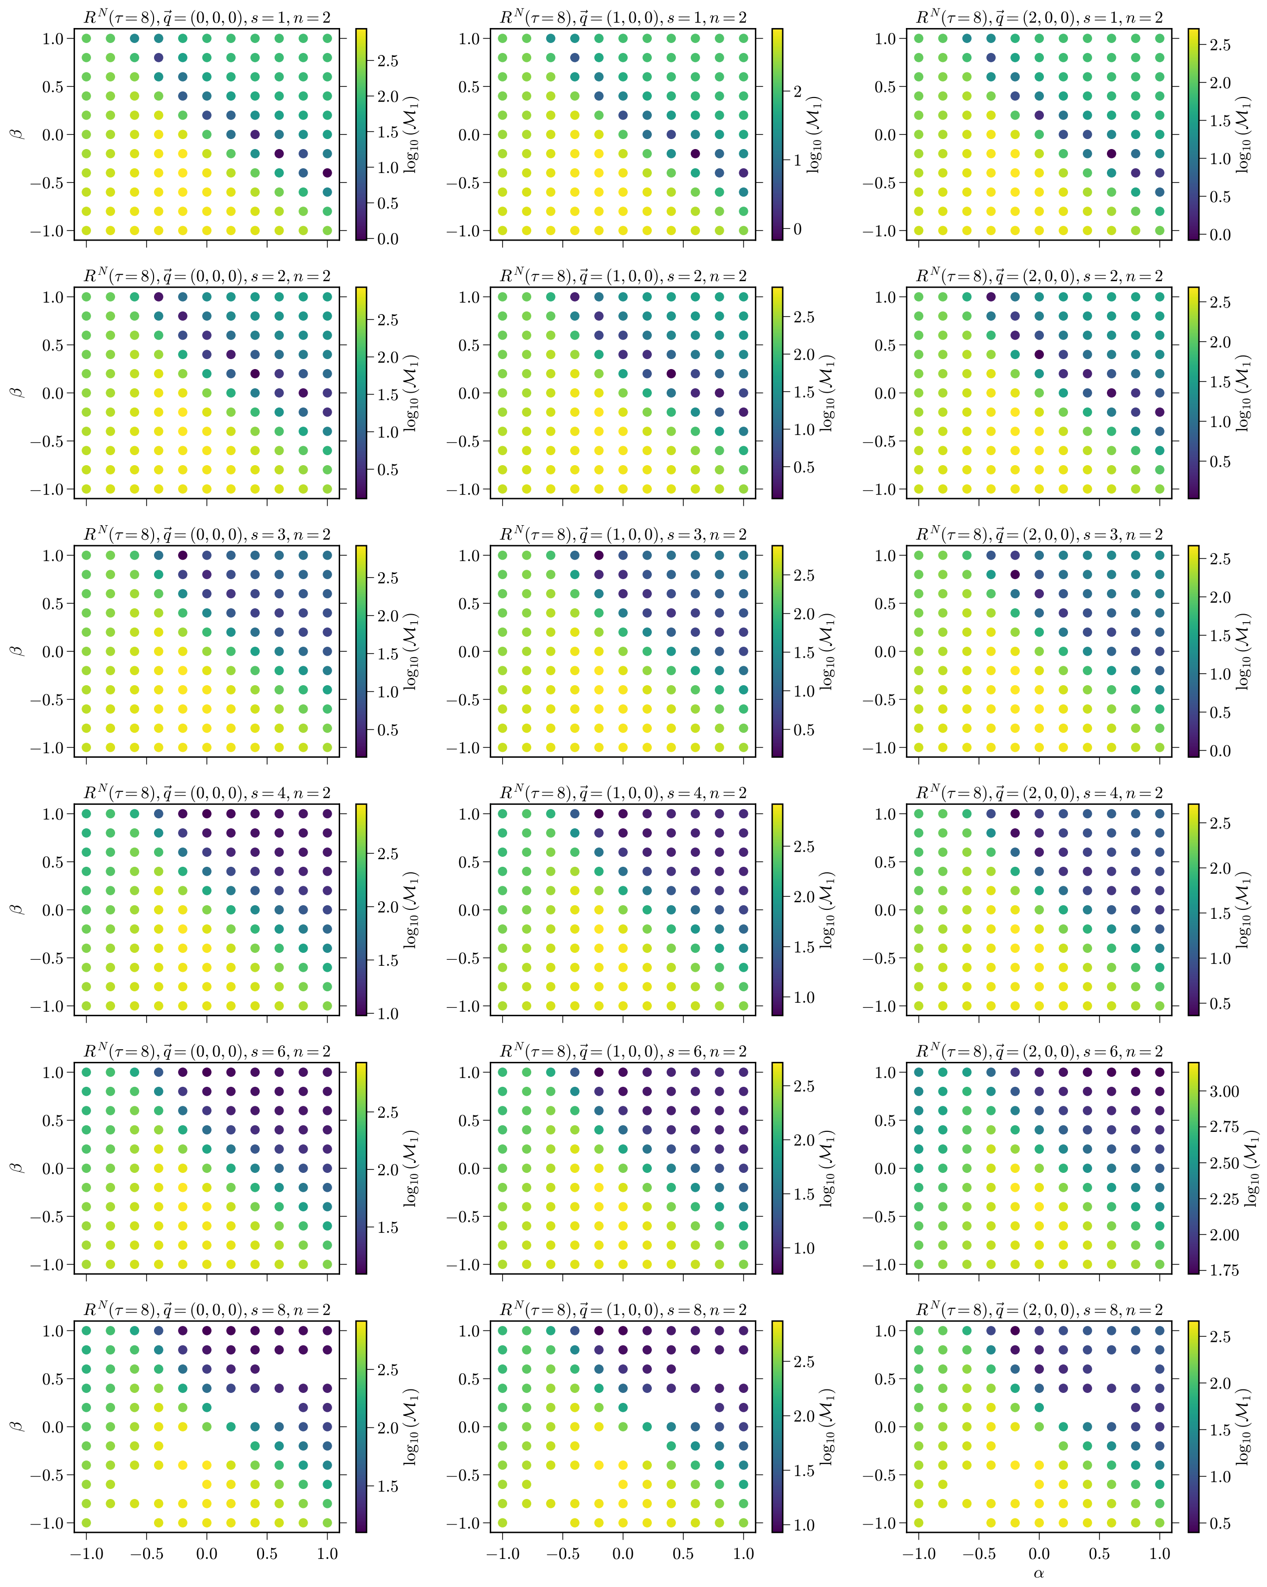


FIG. 28. Metric $\mathcal{M}_1$ (Eq. (25)), for the proton optimized ratio of two-point and three-point functions as a function of $\alpha, \beta$. In this figure, there are $n = 2$ blocking factor, three different values of momentum, and all 7 possible decimation factors.

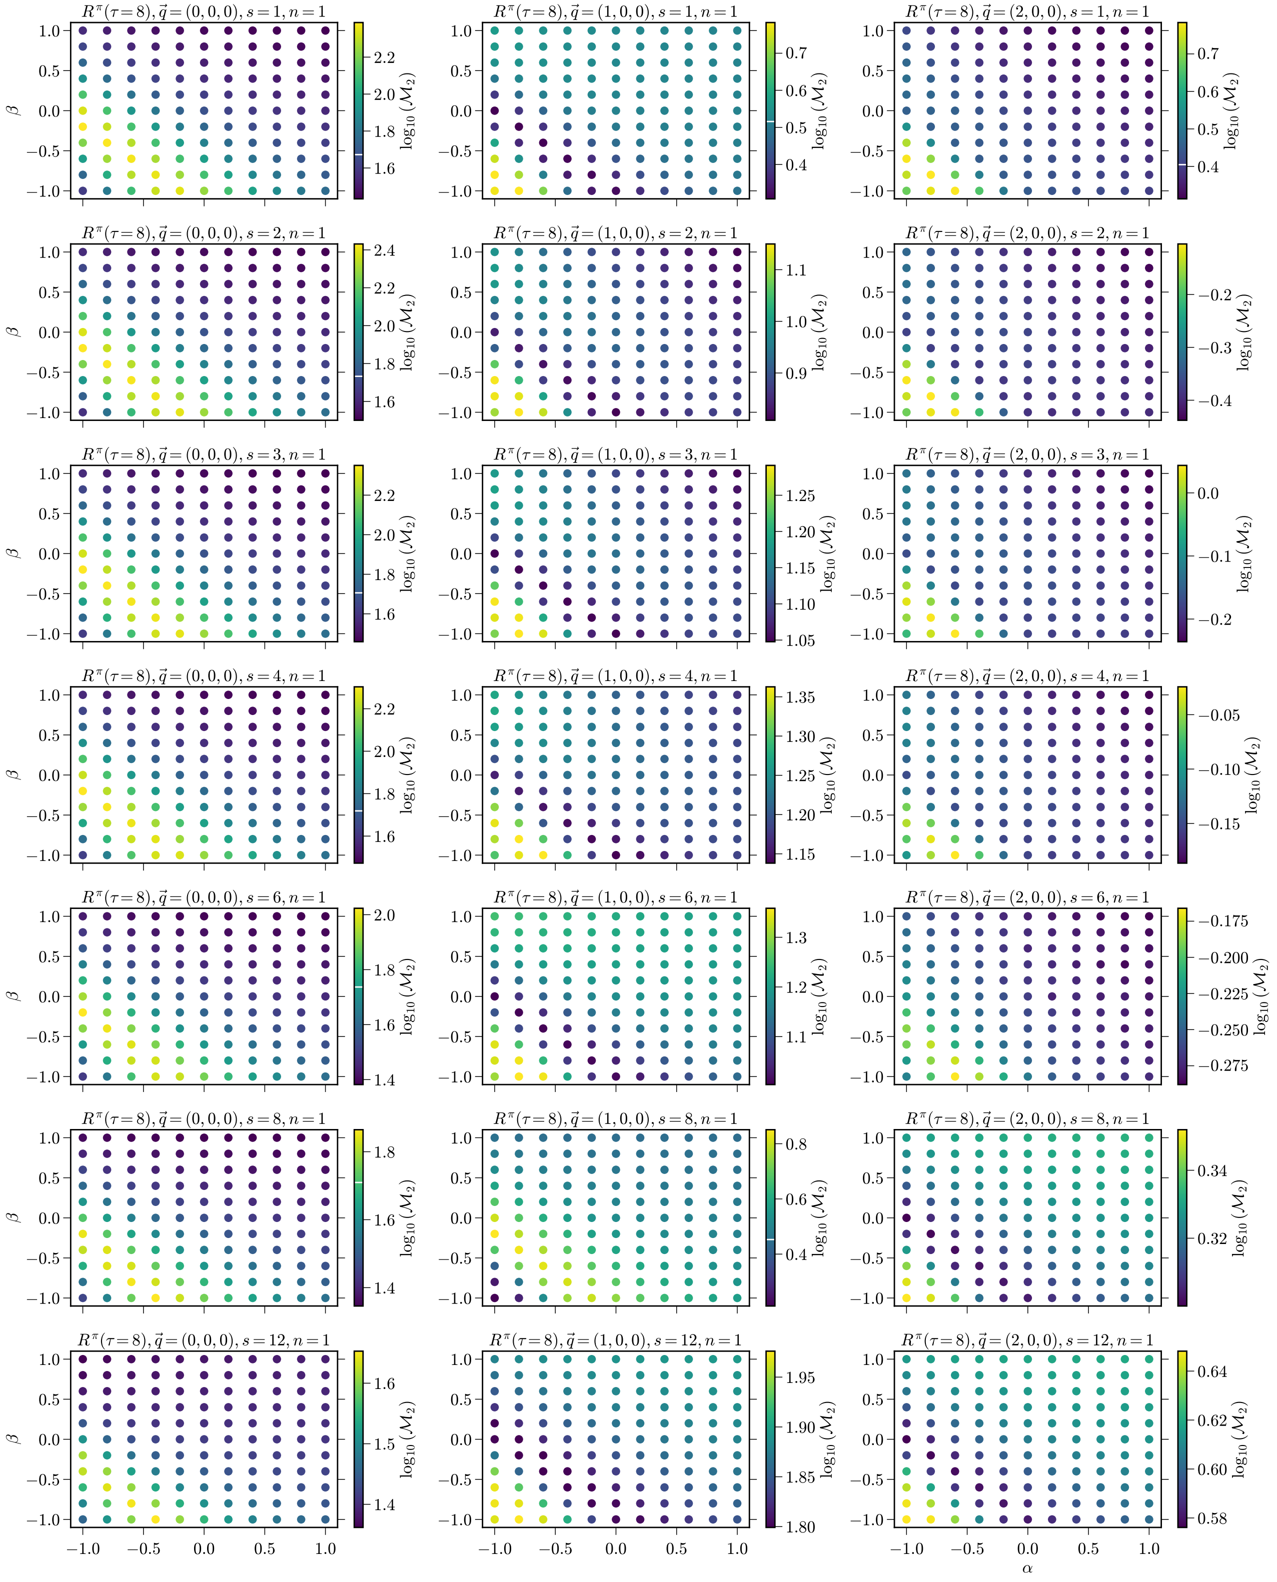

FIG. 29. Metric $\mathcal{M}_2$ (Eq. (26)), for the pion optimized ratio of two-point and three-point functions as a function of $\alpha, \beta$. In this figure, there are $n = 1$ blocking factor, three different values of momentum, and all 7 possible decimation factors.

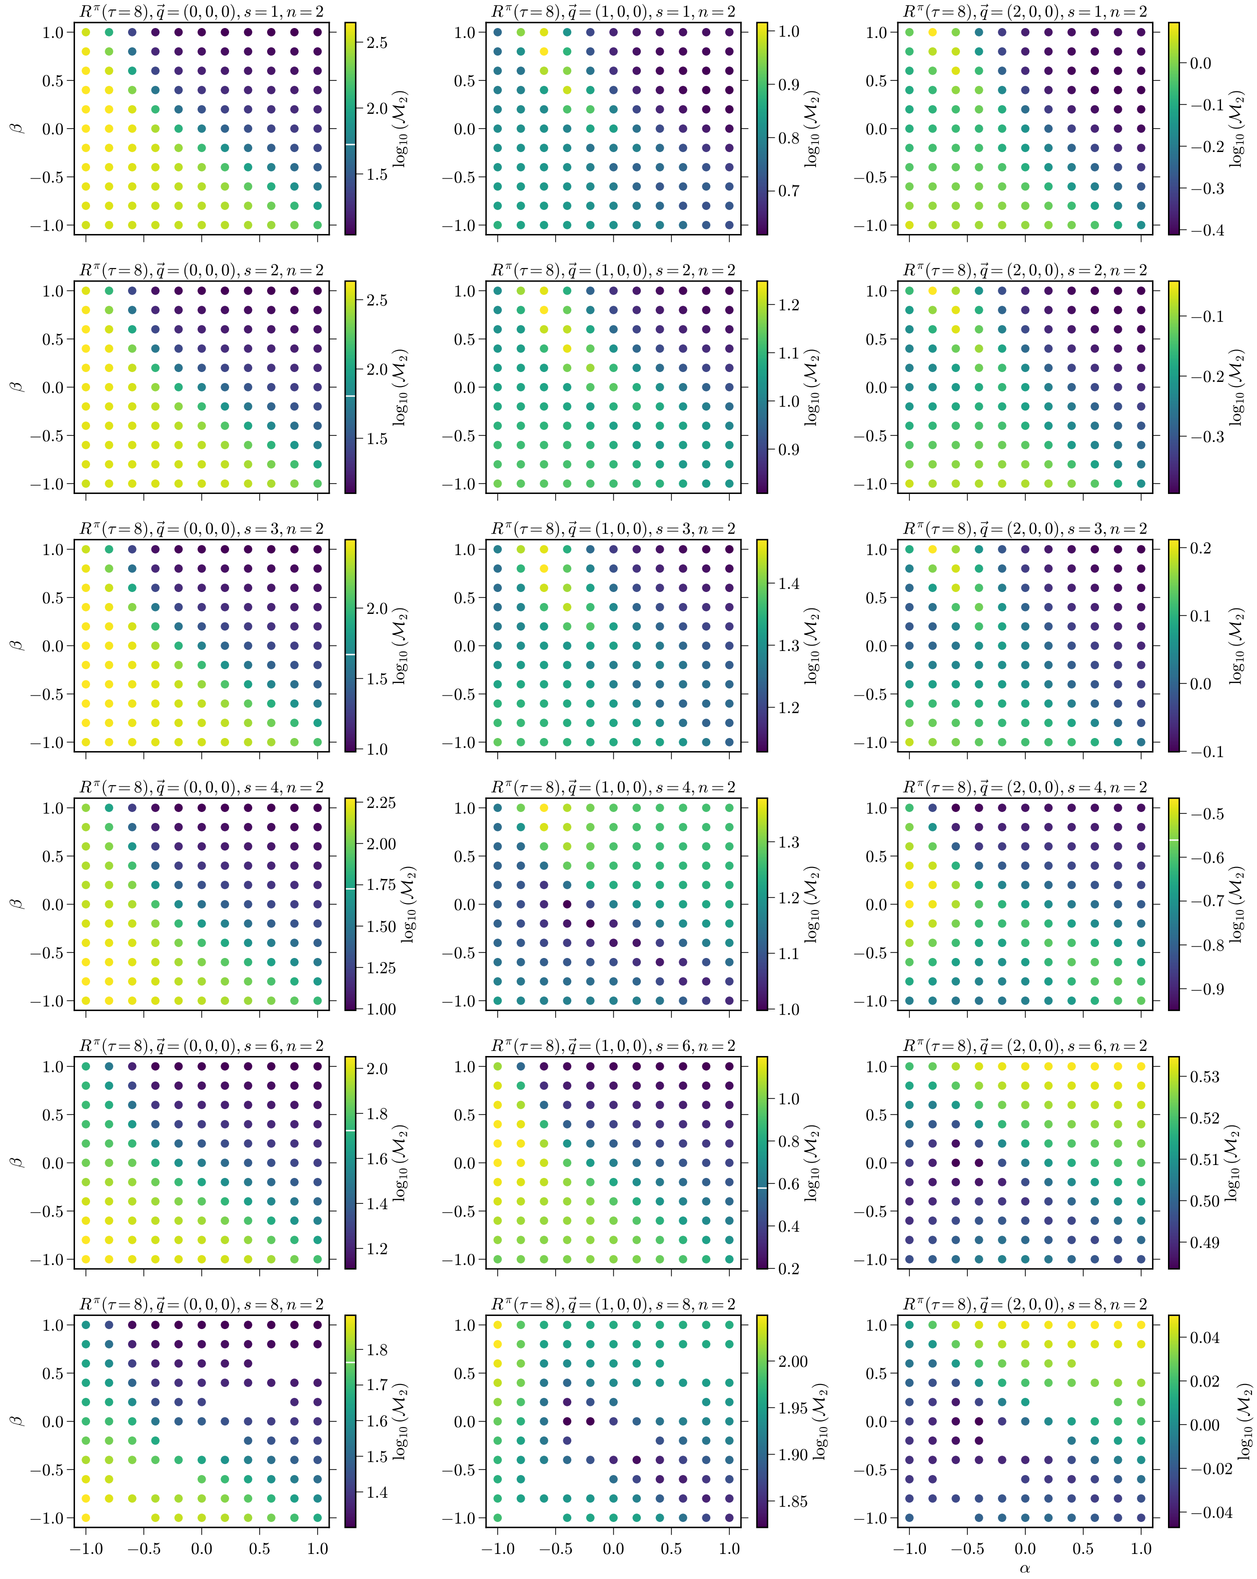


FIG. 30. Metric $\mathcal{M}_2$ (Eq. (26)), for the pion optimized ratio of two-point and three-point functions as a function of $\alpha, \beta$. In this figure, there are $n = 2$ blocking factor, three different values of momentum, and all 7 possible decimation factors.

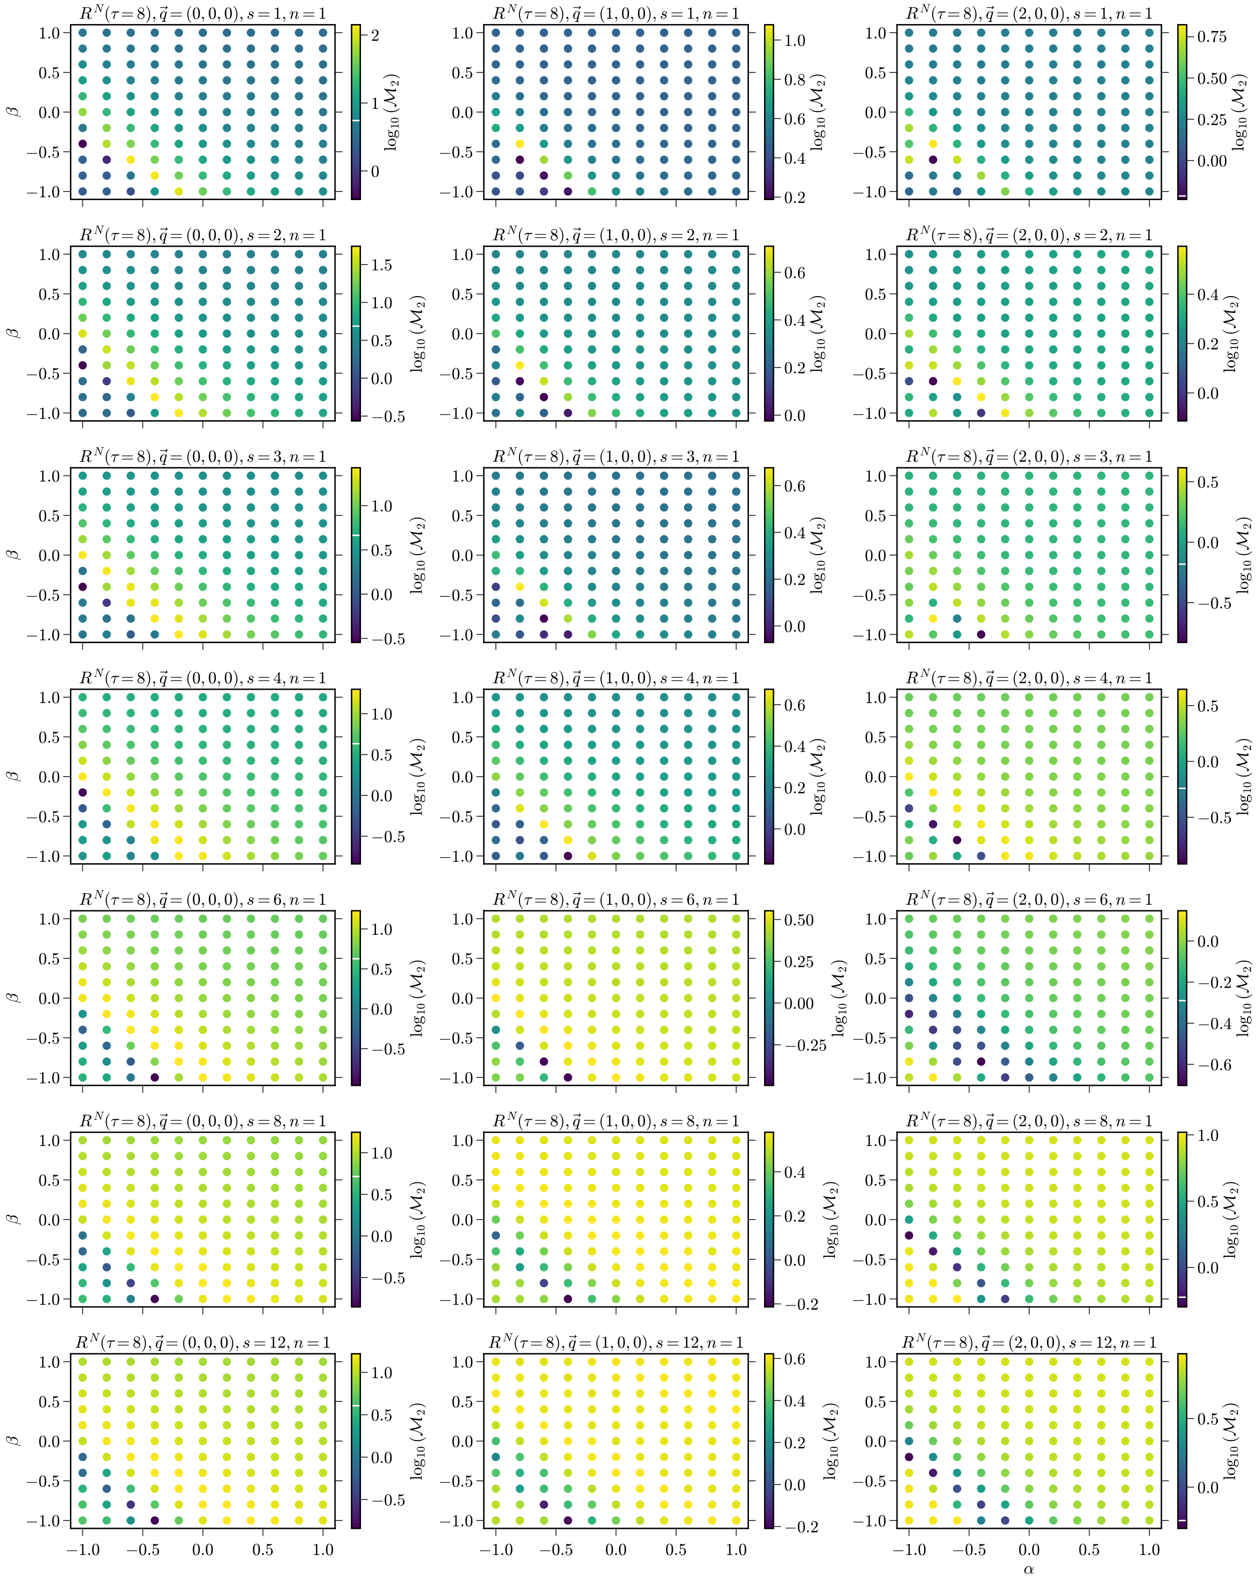

FIG. 31. Metric $\mathcal{M}_2$ (Eq. (26)), for the proton optimized ratio of two-point and three-point functions as a function of $\alpha, \beta$. In this figure, there are $n = 1$ blocking factor, three different values of momentum, and all 7 possible decimation factors.

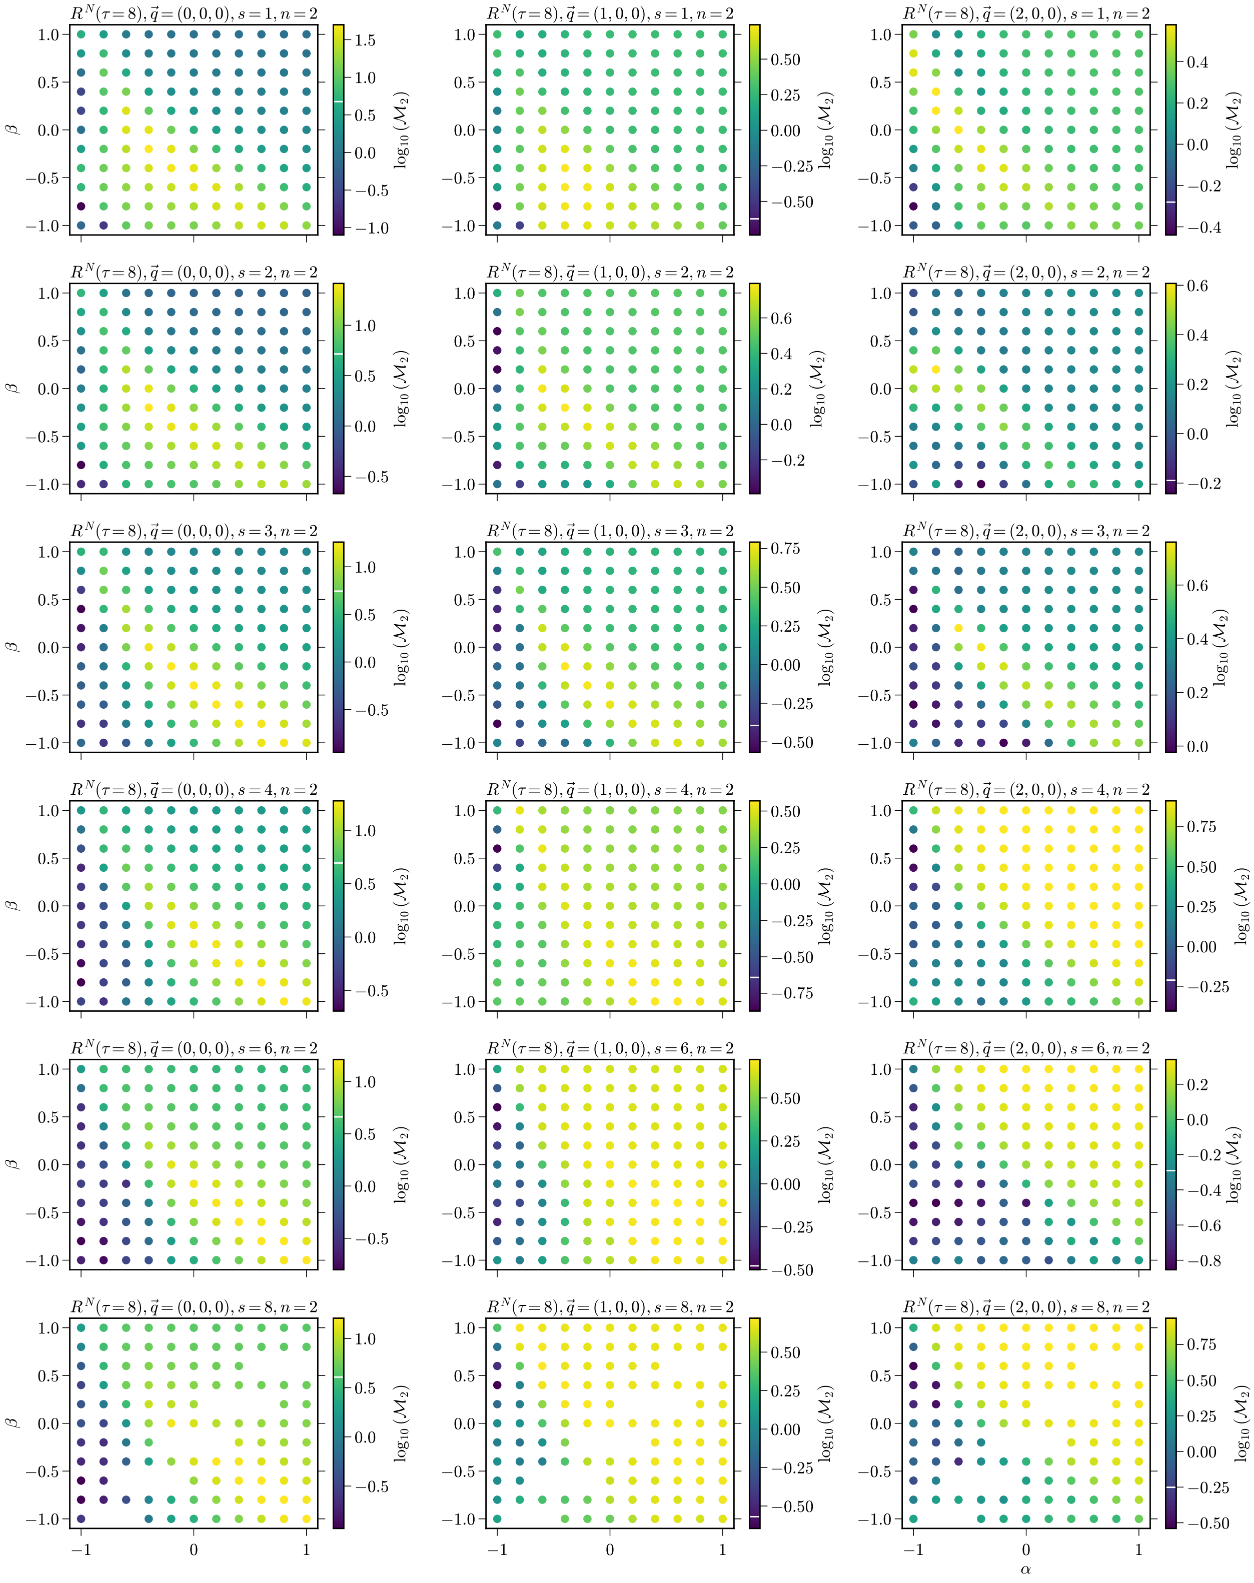


FIG. 32. Metric $\mathcal{M}_2$ (Eq. (26)), for the proton optimized ratio of two-point and three-point functions as a function of $\alpha, \beta$. In this figure, there are $n = 2$ blocking factor, three different values of momentum, and all 7 possible decimation factors.

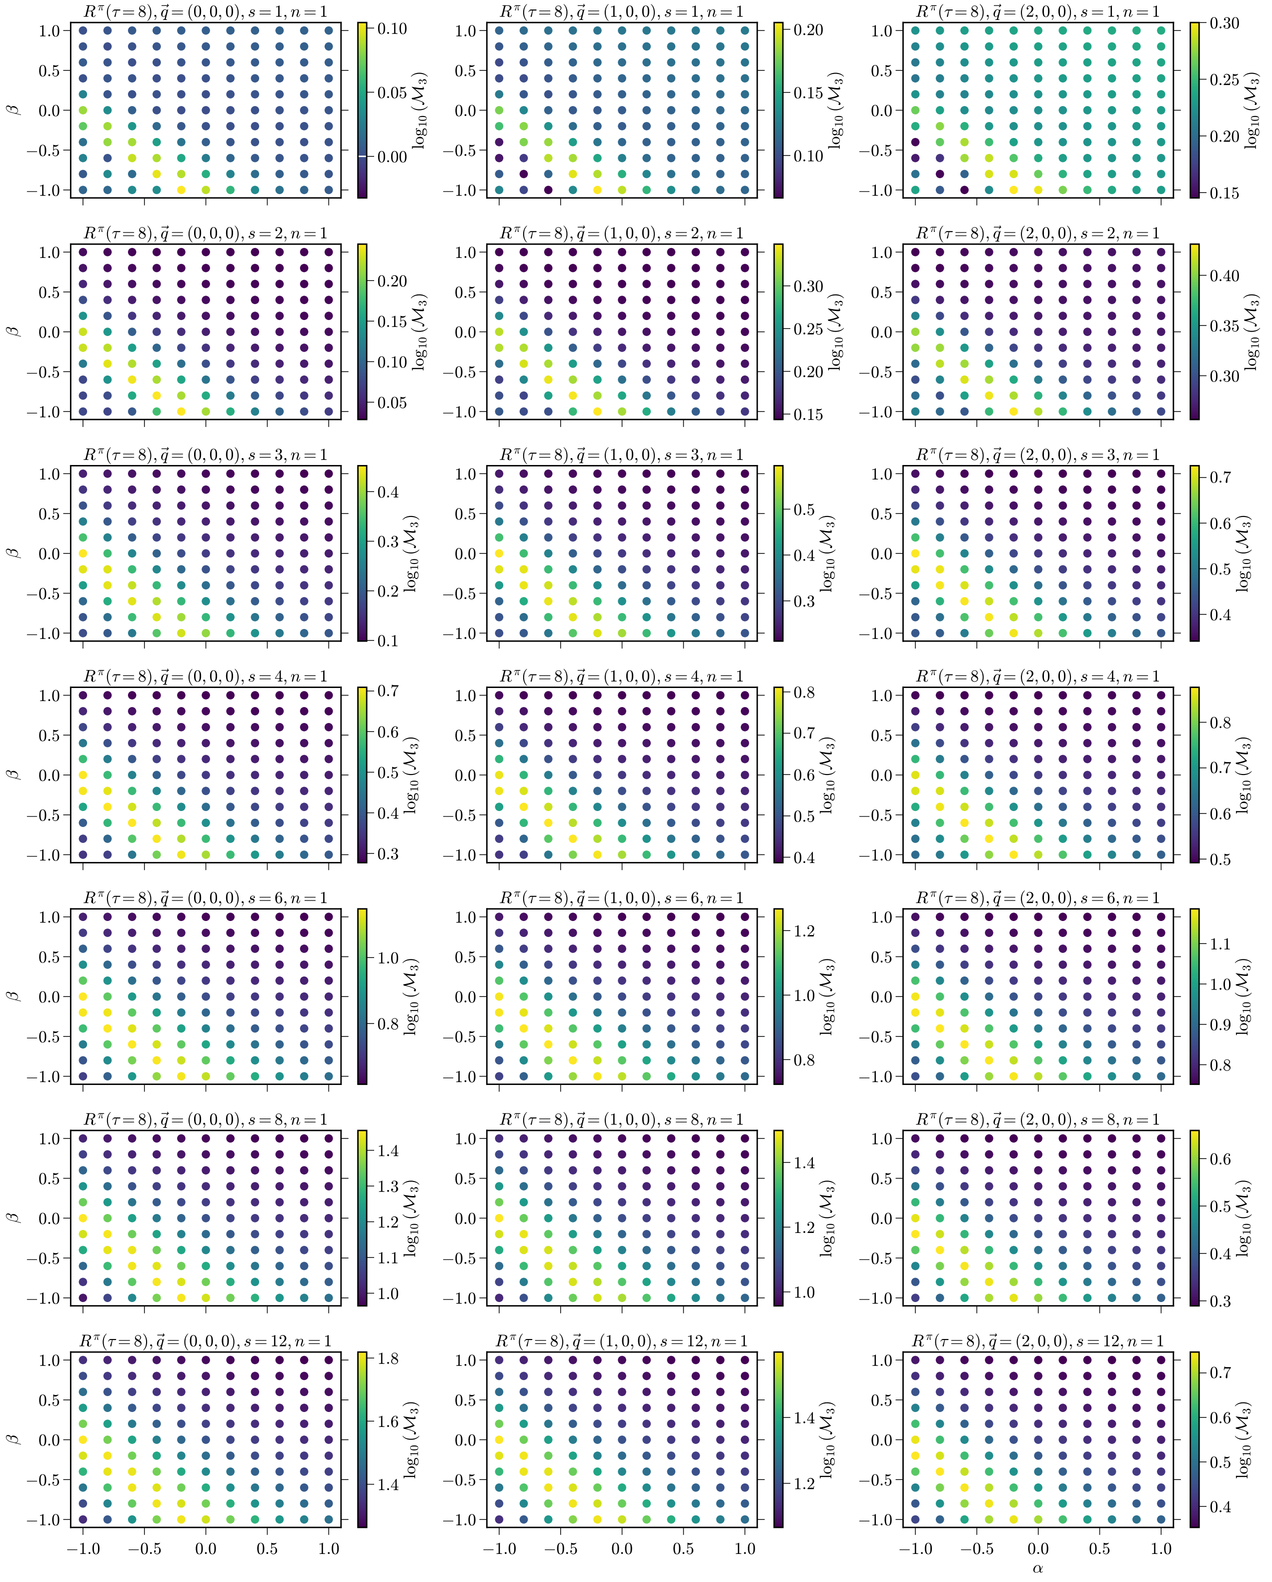


FIG. 33. Metric $\mathcal{M}_3$ (Eq. (27)), for the pion optimized ratio of two-point and three-point functions as a function of $\alpha, \beta$. In this figure, there are $n = 1$ blocking factor, three different values of momentum, and all 7 possible decimation factors.

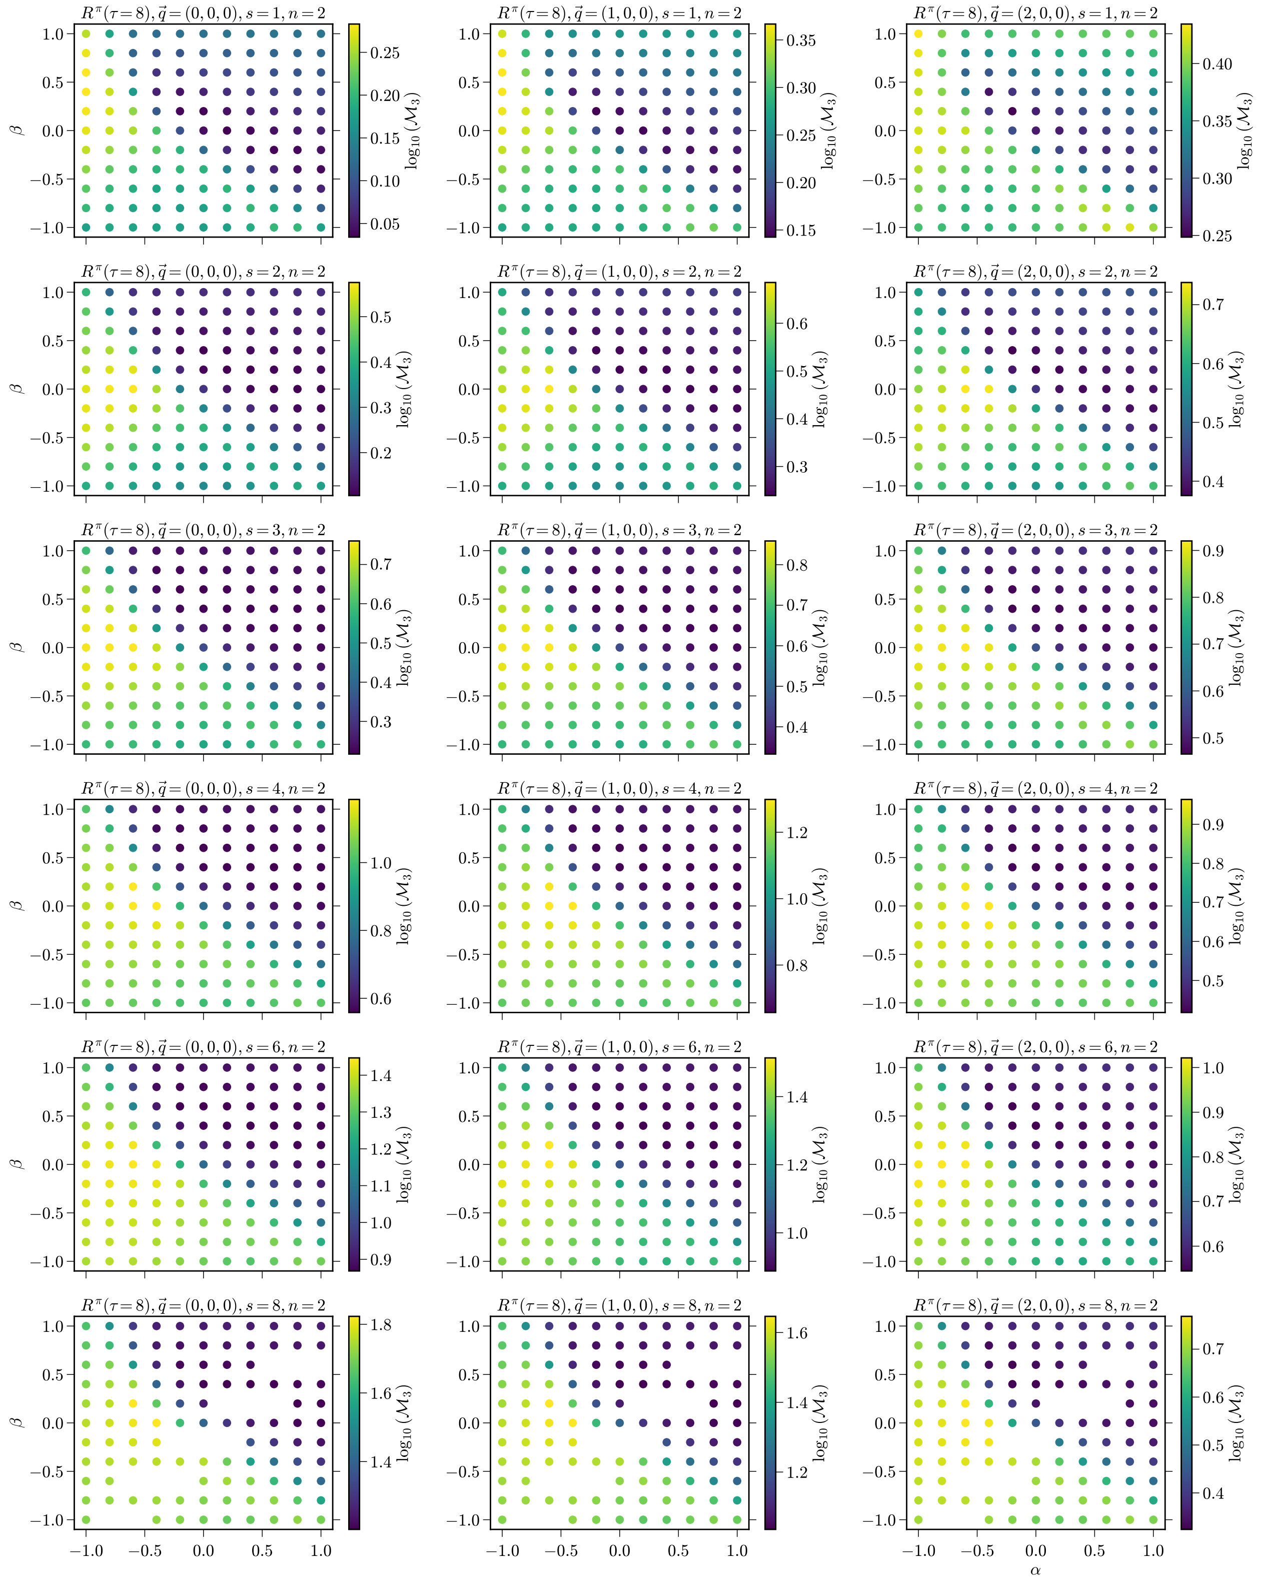

FIG. 34. Metric $\mathcal{M}_3$ (Eq. (27)), for the pion optimized ratio of two-point and three-point functions as a function of $\alpha, \beta$. In this figure, there are $n = 2$ blocking factor, three different values of momentum, and all 7 possible decimation factors.

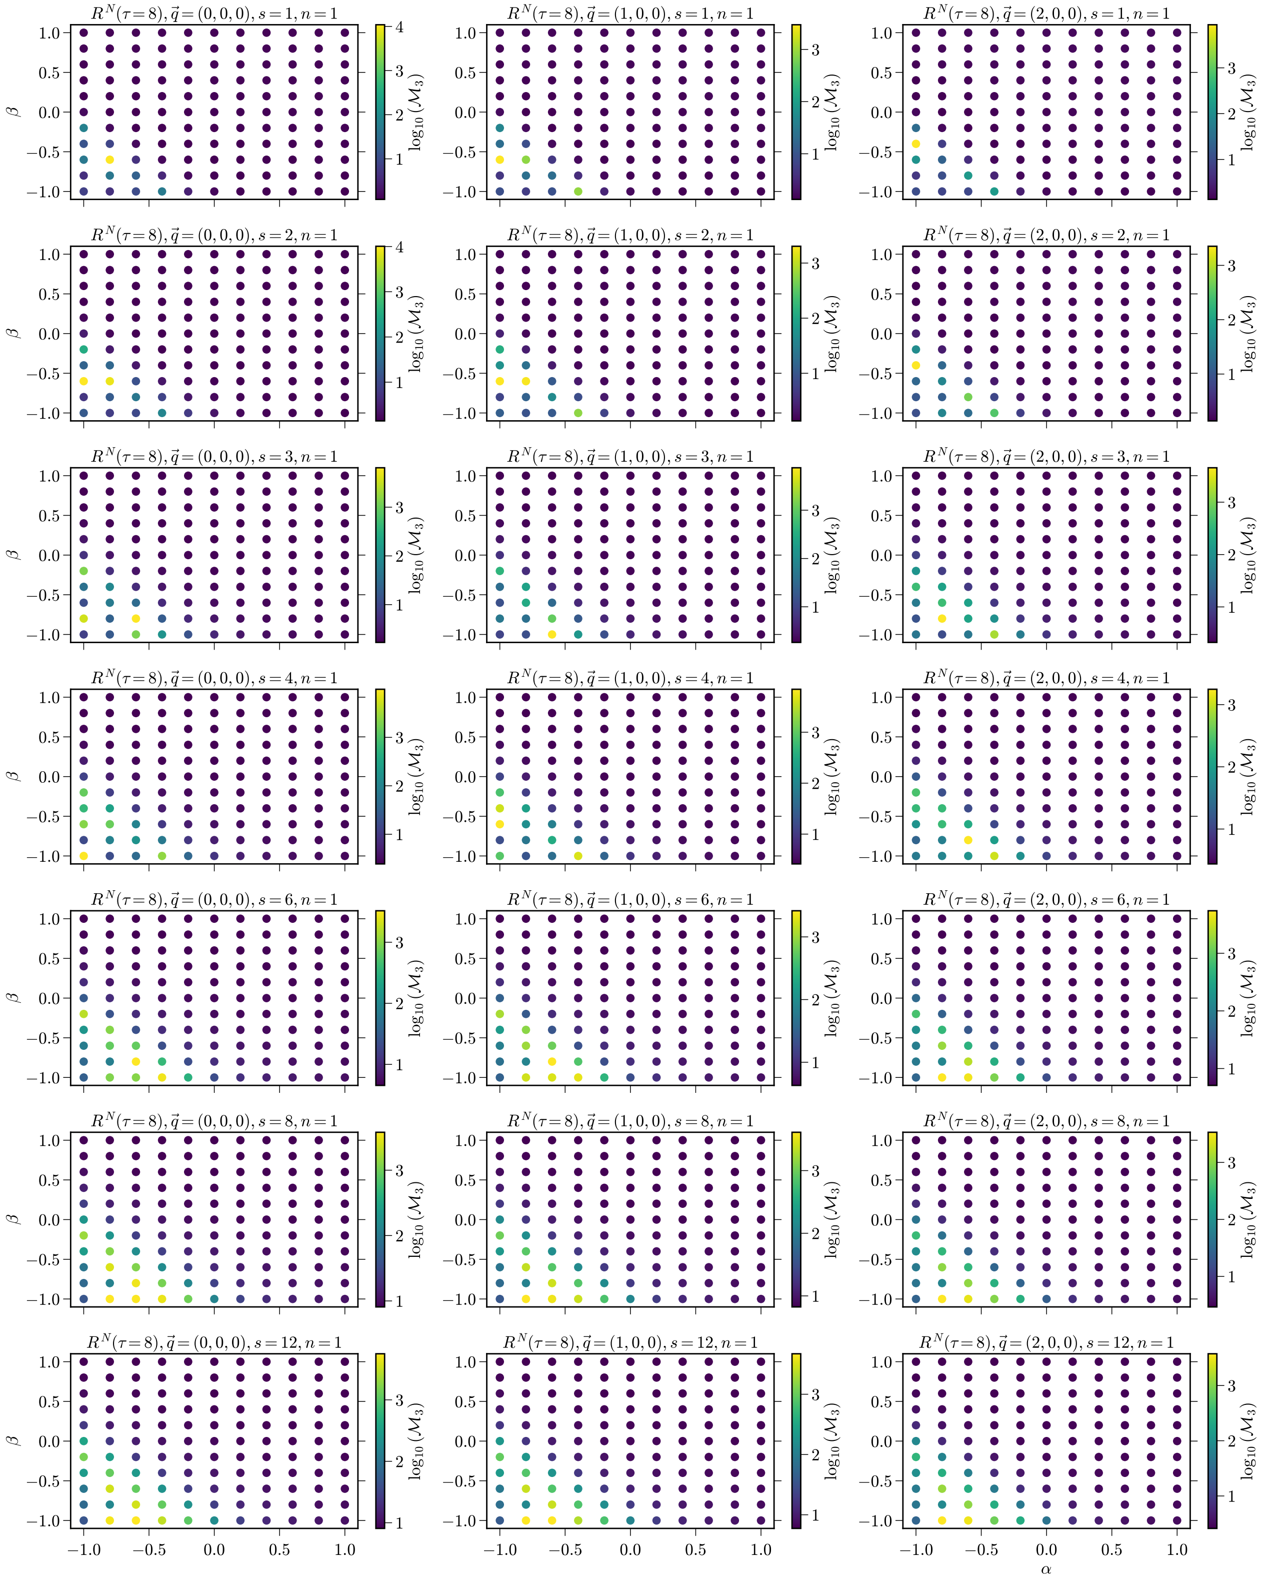


FIG. 35. Metric $\mathcal{M}_3$ (Eq. (27)), for the proton optimized ratio of two-point and three-point functions as a function of $\alpha, \beta$. In this figure, there are $n = 1$ blocking factor, three different values of momentum, and all 7 possible decimation factors.

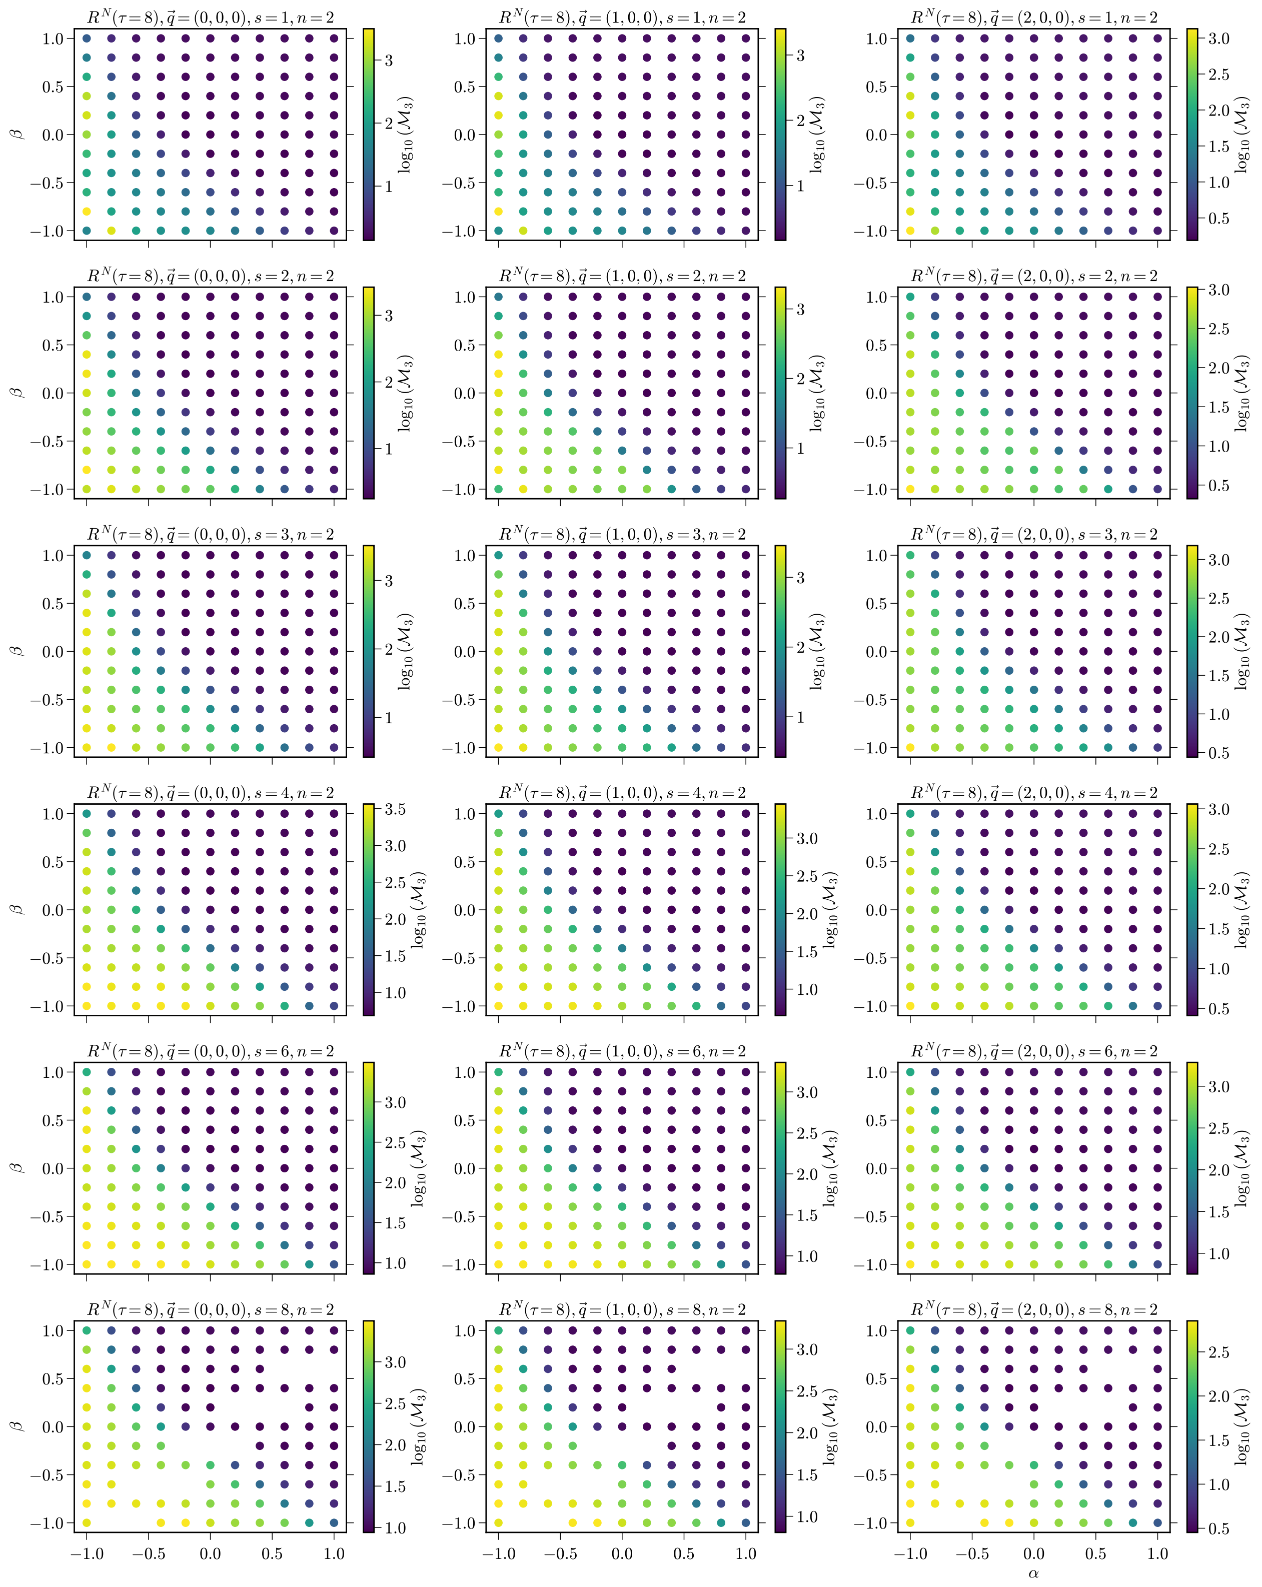

FIG. 36. Metric $\mathcal{M}_3$ (Eq. (27)), for the proton optimized ratio of two-point and three-point functions as a function of $\alpha, \beta$. In this figure, there are $n = 2$ blocking factor, three different values of momentum, and all 7 possible decimation factors.

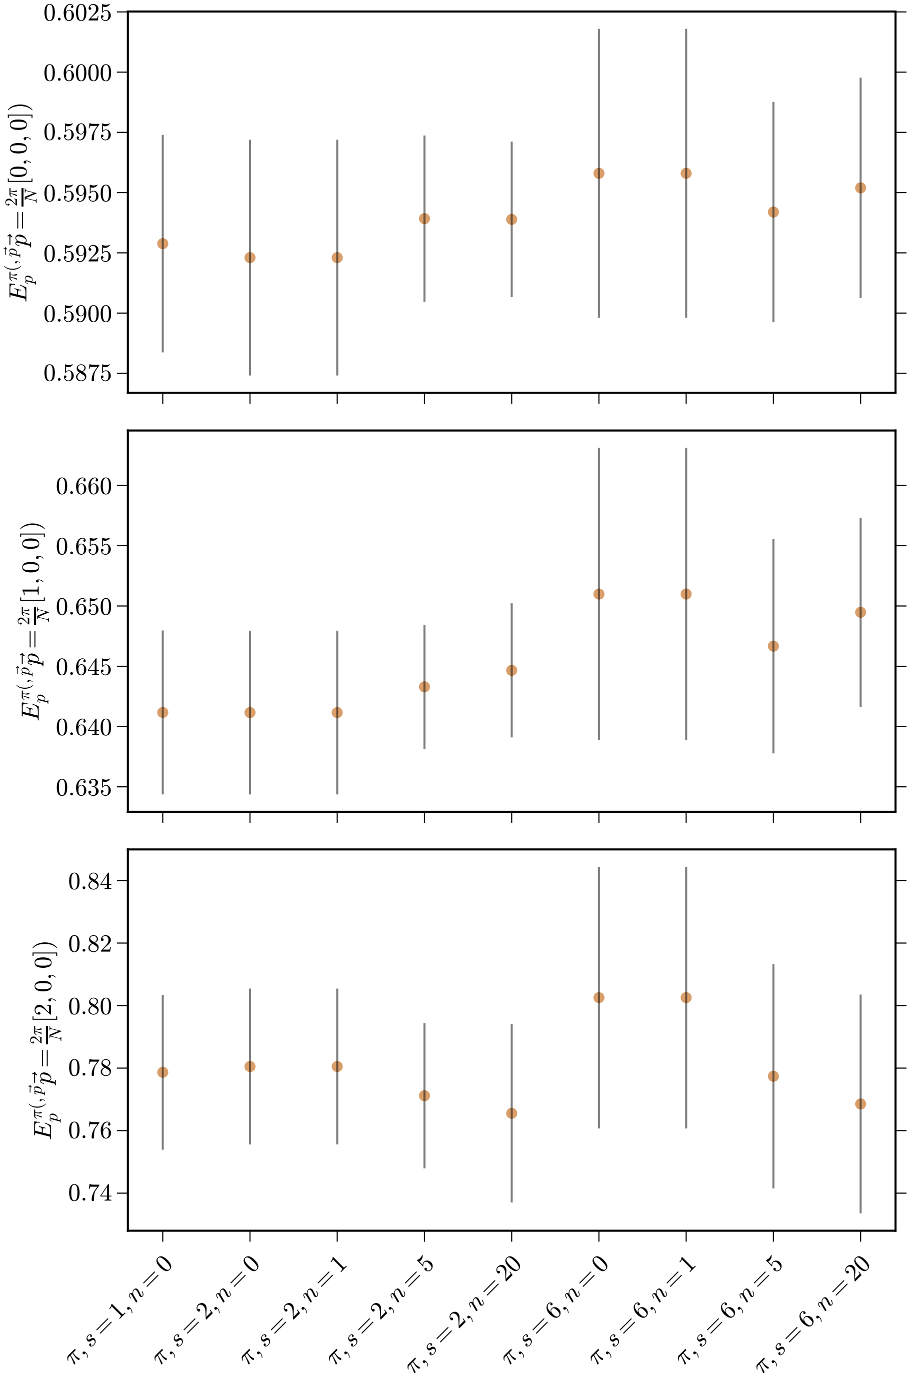


FIG. 37. The best-fit value of the pion effective energy, $E_p^{\pi,\vec{p}}$ (see Sec. IV B). We use $\alpha = \beta = 1$ throughout.

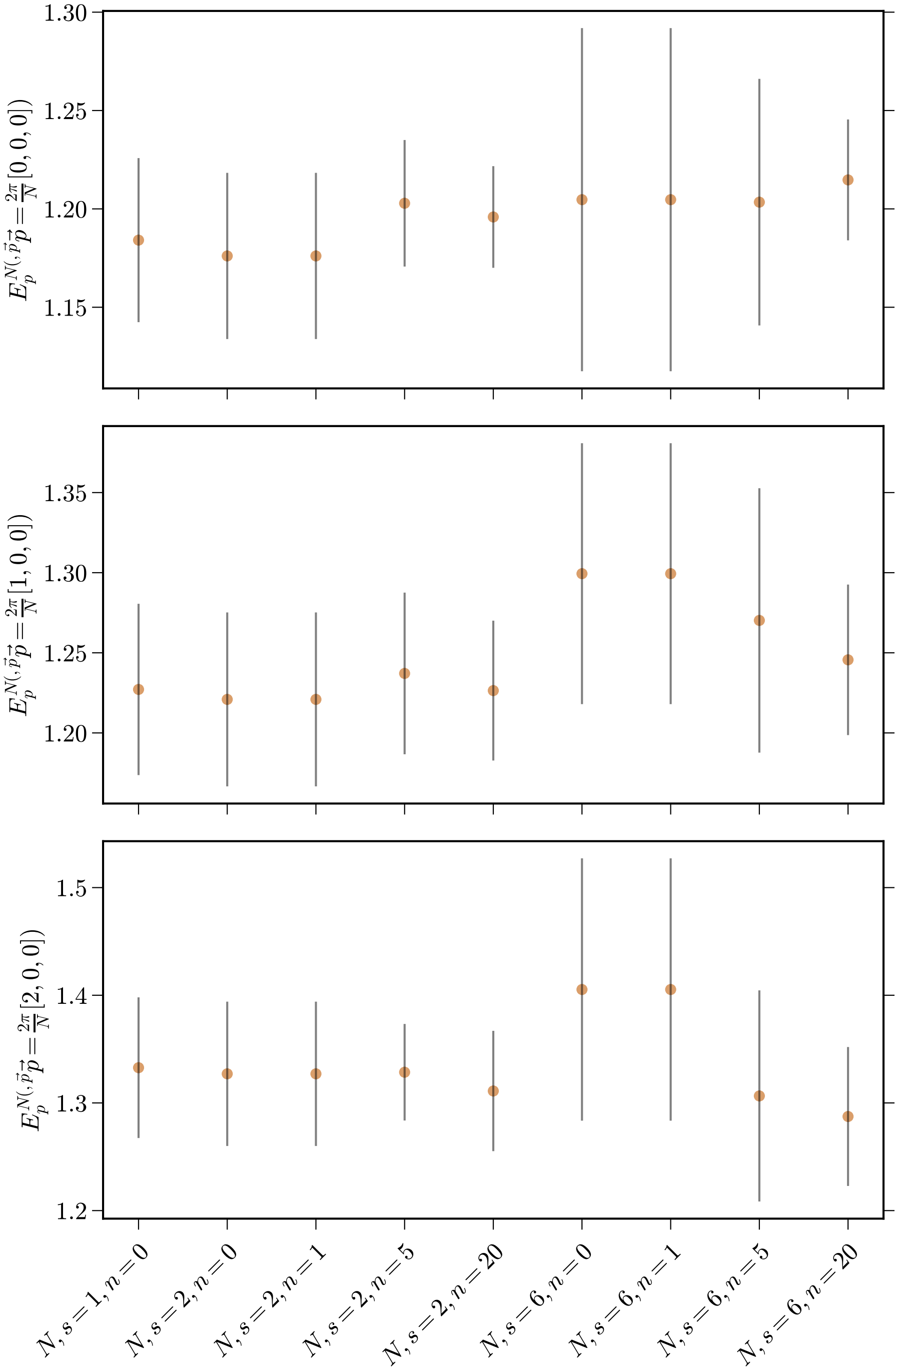


FIG. 38. The best-fit value of the proton effective energy, $E_p^{N,\vec{p}}$ (see Sec. IV B). We use $\alpha = \beta = 1$ throughout.

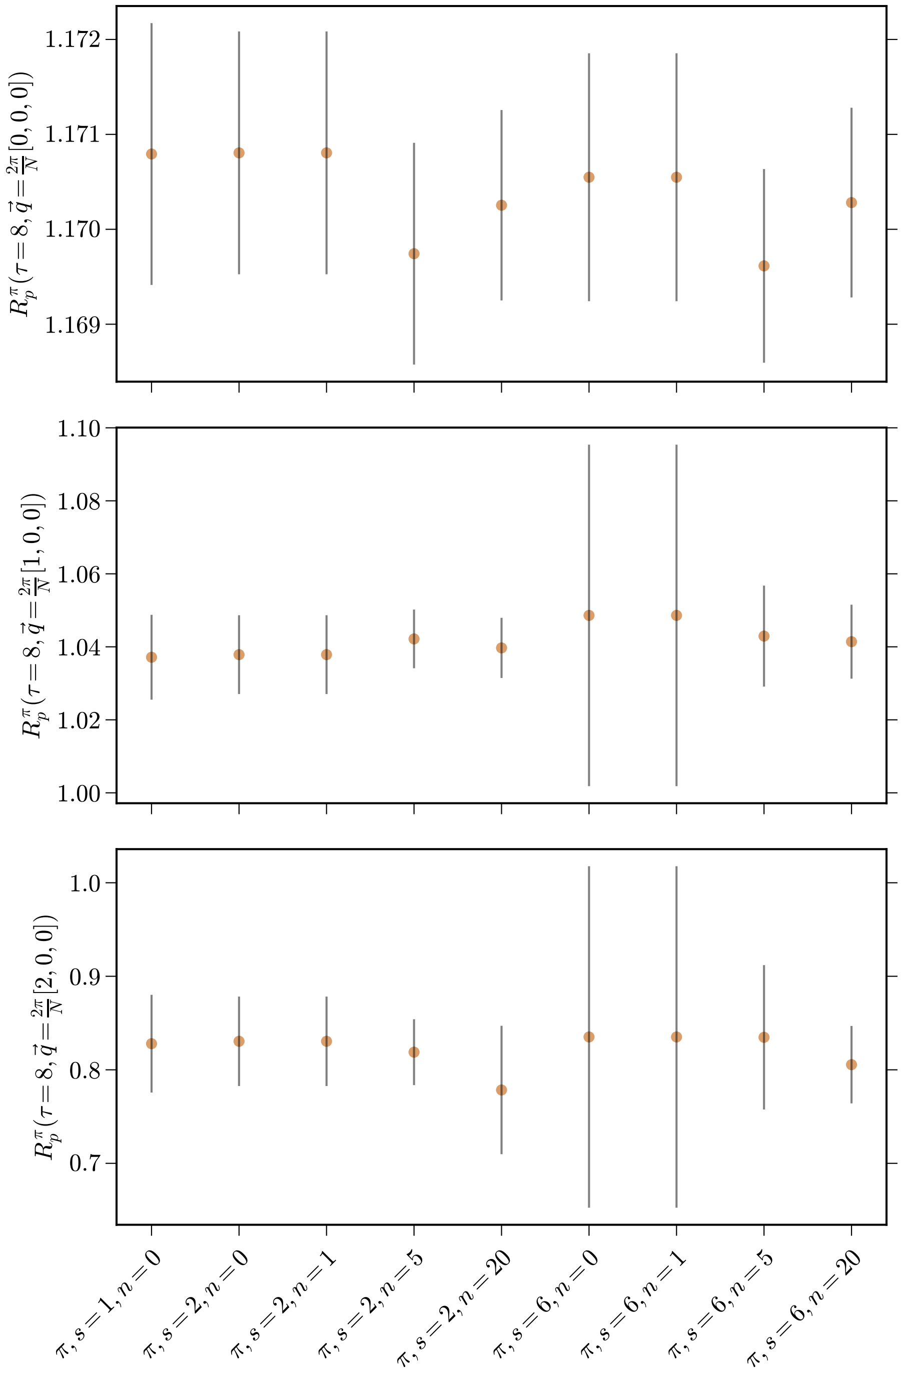


FIG. 39. The best-fit value of the pion improved ratio of three- and two-point functions, $R_p^\pi(\tau,\vec{q})$ (see Sec. IV B). We use $\alpha=\beta=1$ throughout.

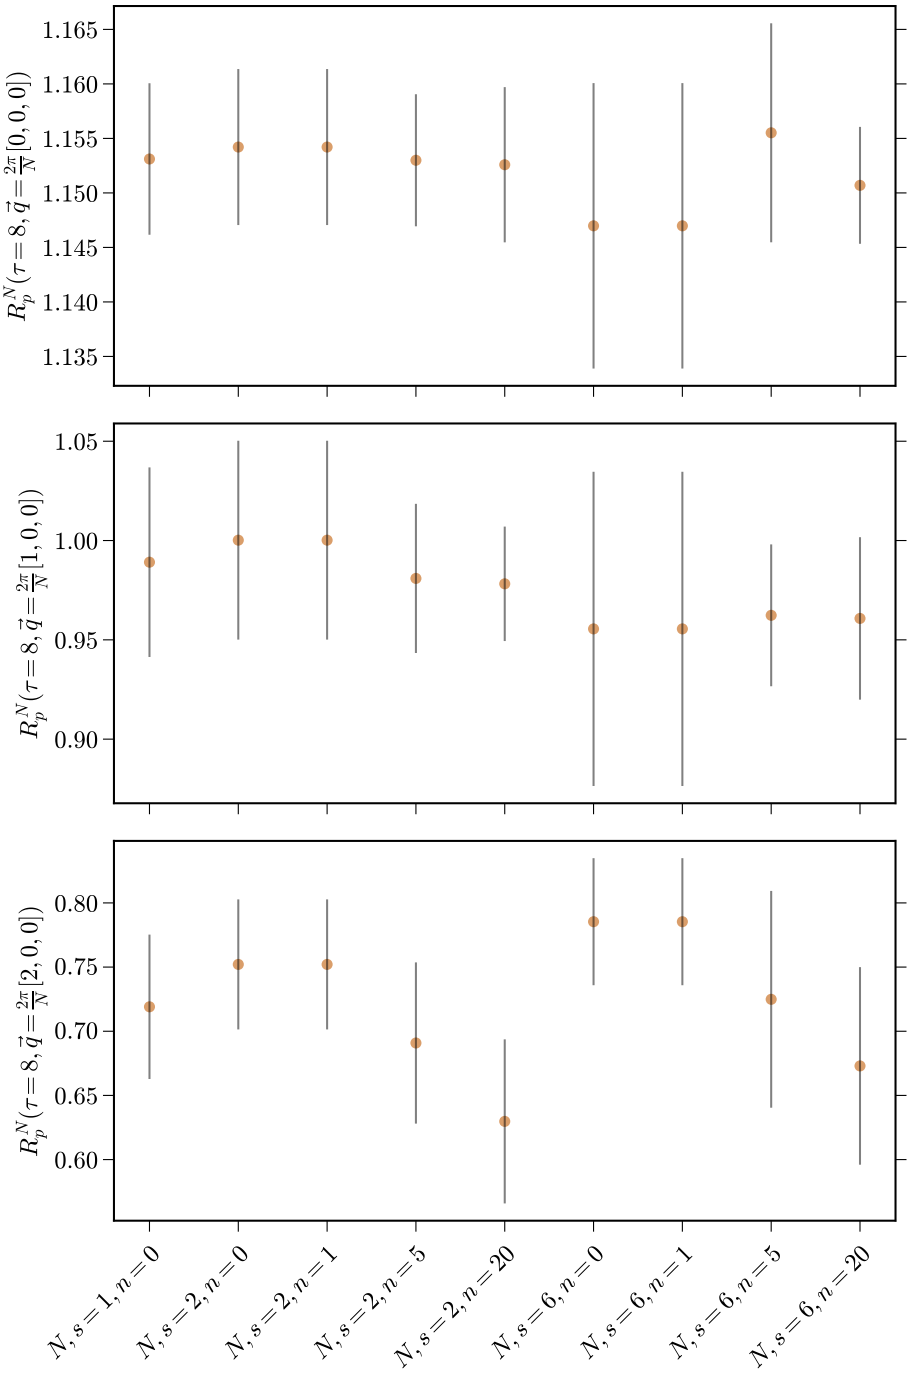


FIG. 40. The best-fit value of the proton improved ratio of three- and two-point functions, $R_p^N(\tau, \vec{q})$ (see Sec. IV B). We use $\alpha = \beta = 1$ throughout.
