# Supplementary material for: Aspects of Propagator Sparsening in Lattice QCD
Source: arXiv:2501.05404 ancillary file (2025-03-28)
Supplement: Supplementary file 2 [file Sparsening_Supplementary_Materials.pdf]

# Aspects of Propagator Sparsening in Lattice QCD: Supplementary Material

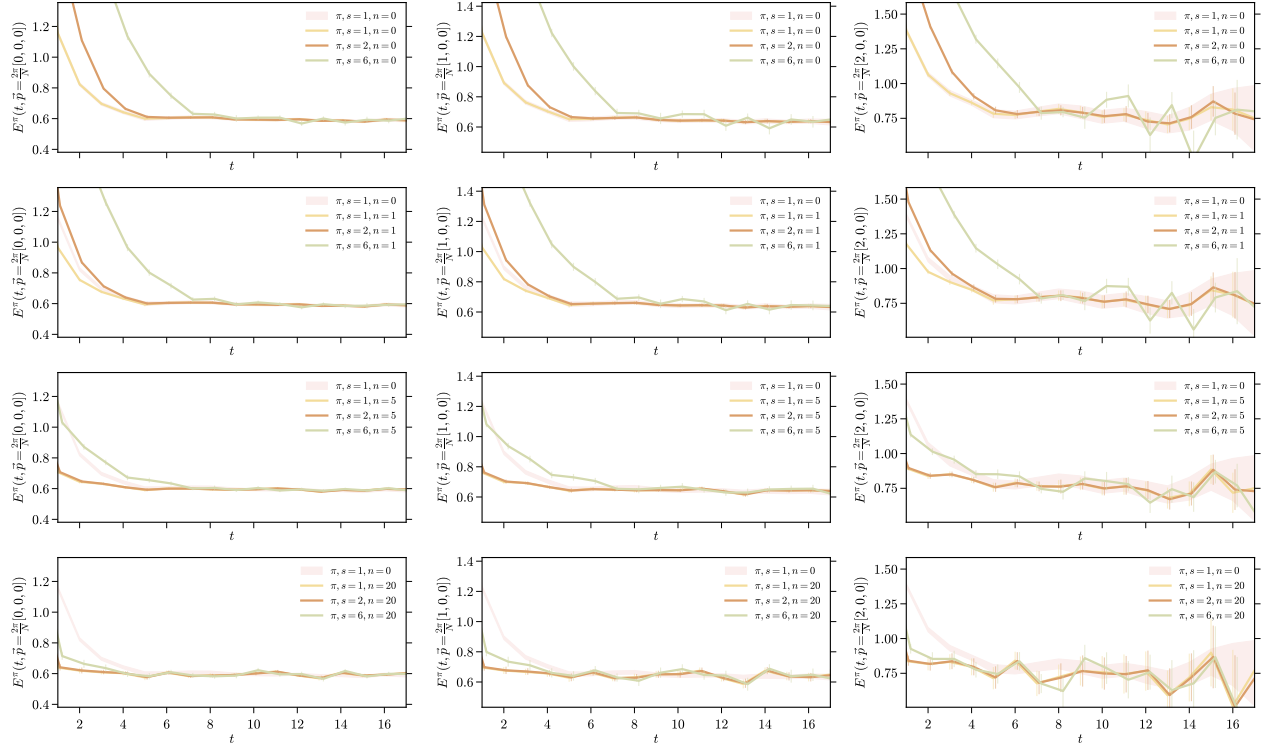

FIG. 1. The pion effective energy as a function of time extent,  $E^\pi(t, \vec{p})$  (Eq. (18)), for three decimation factors ( $s = 1, s = 2, s = 6$ ), three blocking factors ( $n = 1, n = 5, n = 20$ ), three different values of momentum, and  $\alpha = \beta = 1$ . The unsparnsed correlation function with  $s = 1, n = 0$  is shown as a pink shaded-region.

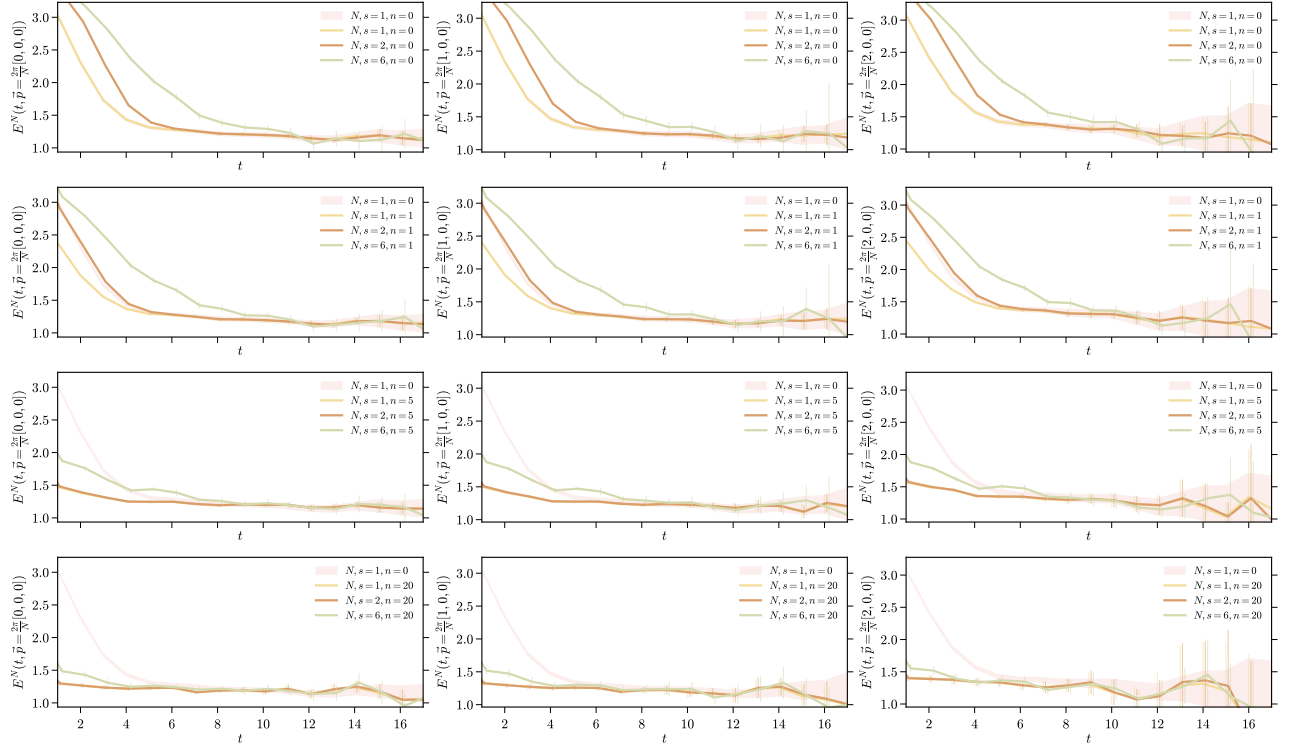

FIG. 2. The proton effective energy as a function of time extent,  $E^N(t, \vec{p})$  (Eq. (18)), for three decimation factors ( $s = 1, s = 2, s = 6$ ), three blocking factors ( $n = 1, n = 5, n = 20$ ), three different values of momentum, and  $\alpha = \beta = 1$ . The unsparsened correlation function with  $s = 1, n = 0$  is shown as a pink shaded-region.

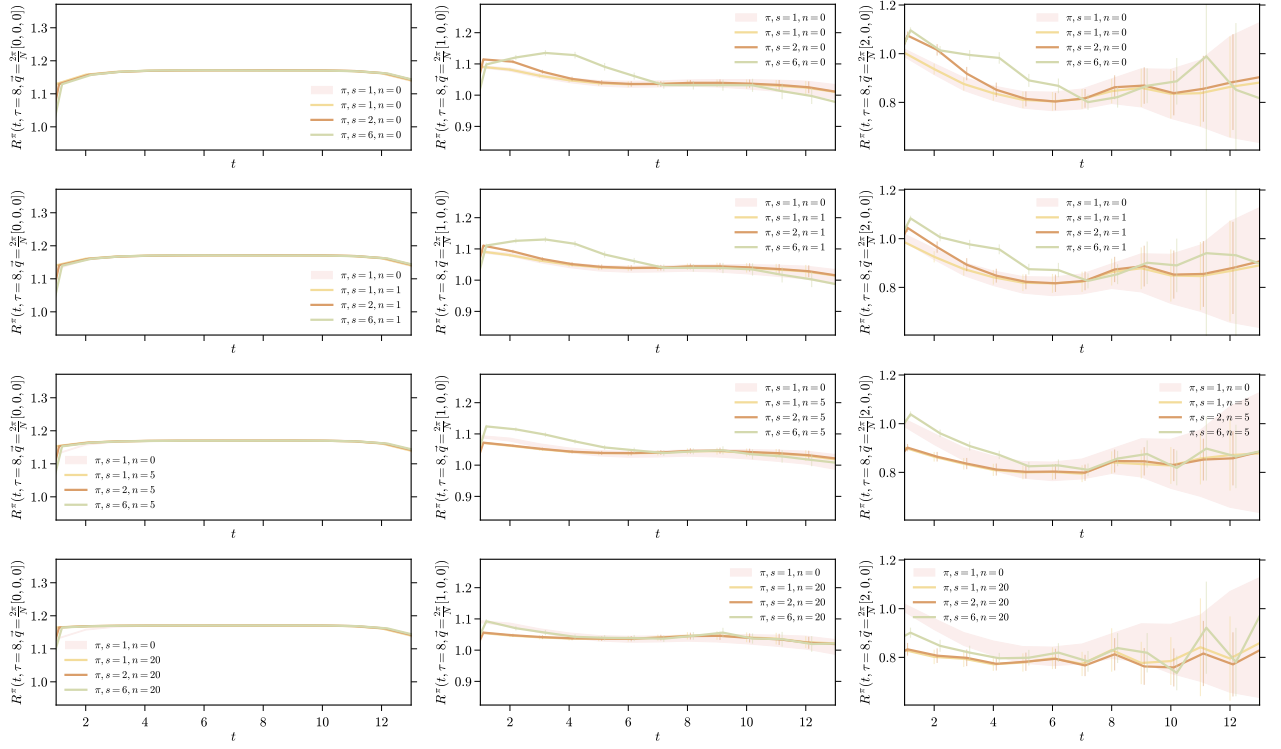

FIG. 3. The pion improved ratio of three- and two-point functions,  $R^\pi(t, \tau=8, \vec{q})$  (Eqs. (30) and (33)), for three decimation factors ( $s=1, s=2, s=6$ ), three blocking factors ( $n=1, n=5, n=20$ ), three different values of momentum, and  $\alpha=\beta=1$ . The unparsened correlation function with  $s=1, n=0$  is shown as a pink shaded-region.

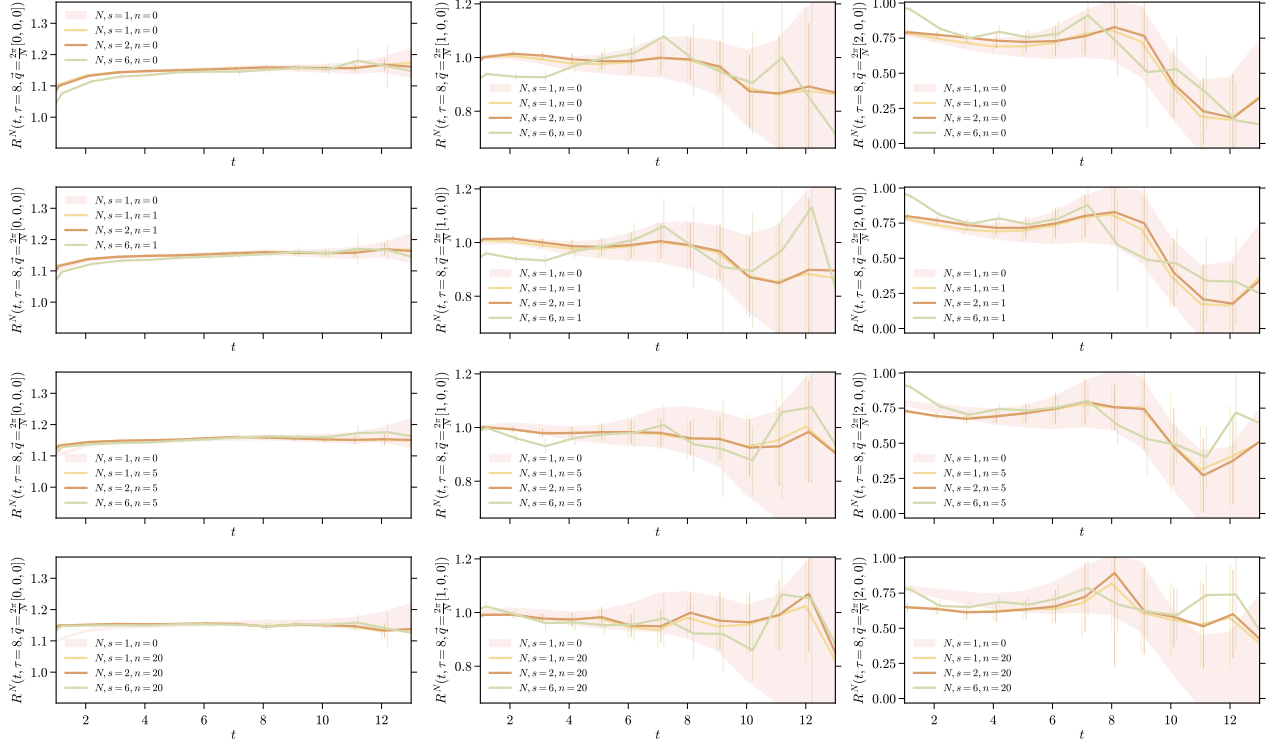

FIG. 4. The proton improved ratio of three- and two-point functions,  $R^N(t, \tau=8, \vec{q})$  (Eqs. (30) and (33)), for three decimation factors ( $s=1, s=2, s=6$ ), three blocking factors ( $n=1, n=5, n=20$ ), three different values of momentum, and  $\alpha=\beta=1$ . The unparsened correlation function with  $s=1, n=0$  is shown as a pink shaded-region.

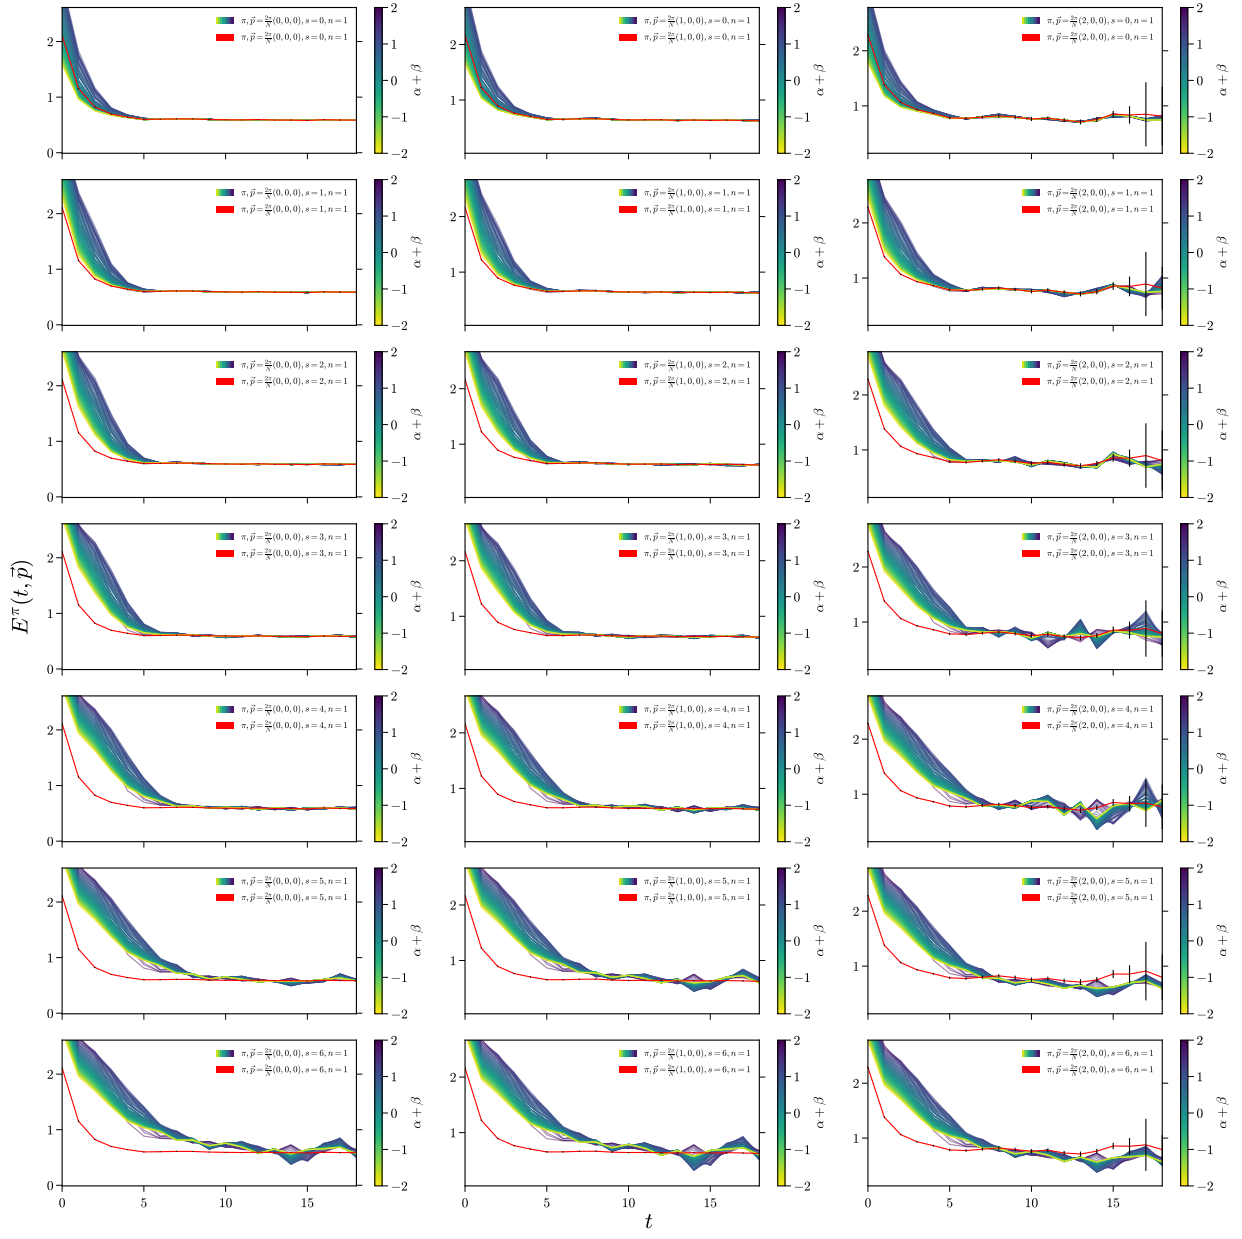

FIG. 5. Effective energy as a function of time,  $E^\pi(t, \vec{p})$  (Eq. (18)), for varying  $\alpha, \beta$  and momentum. The unsparse result is shown in red.

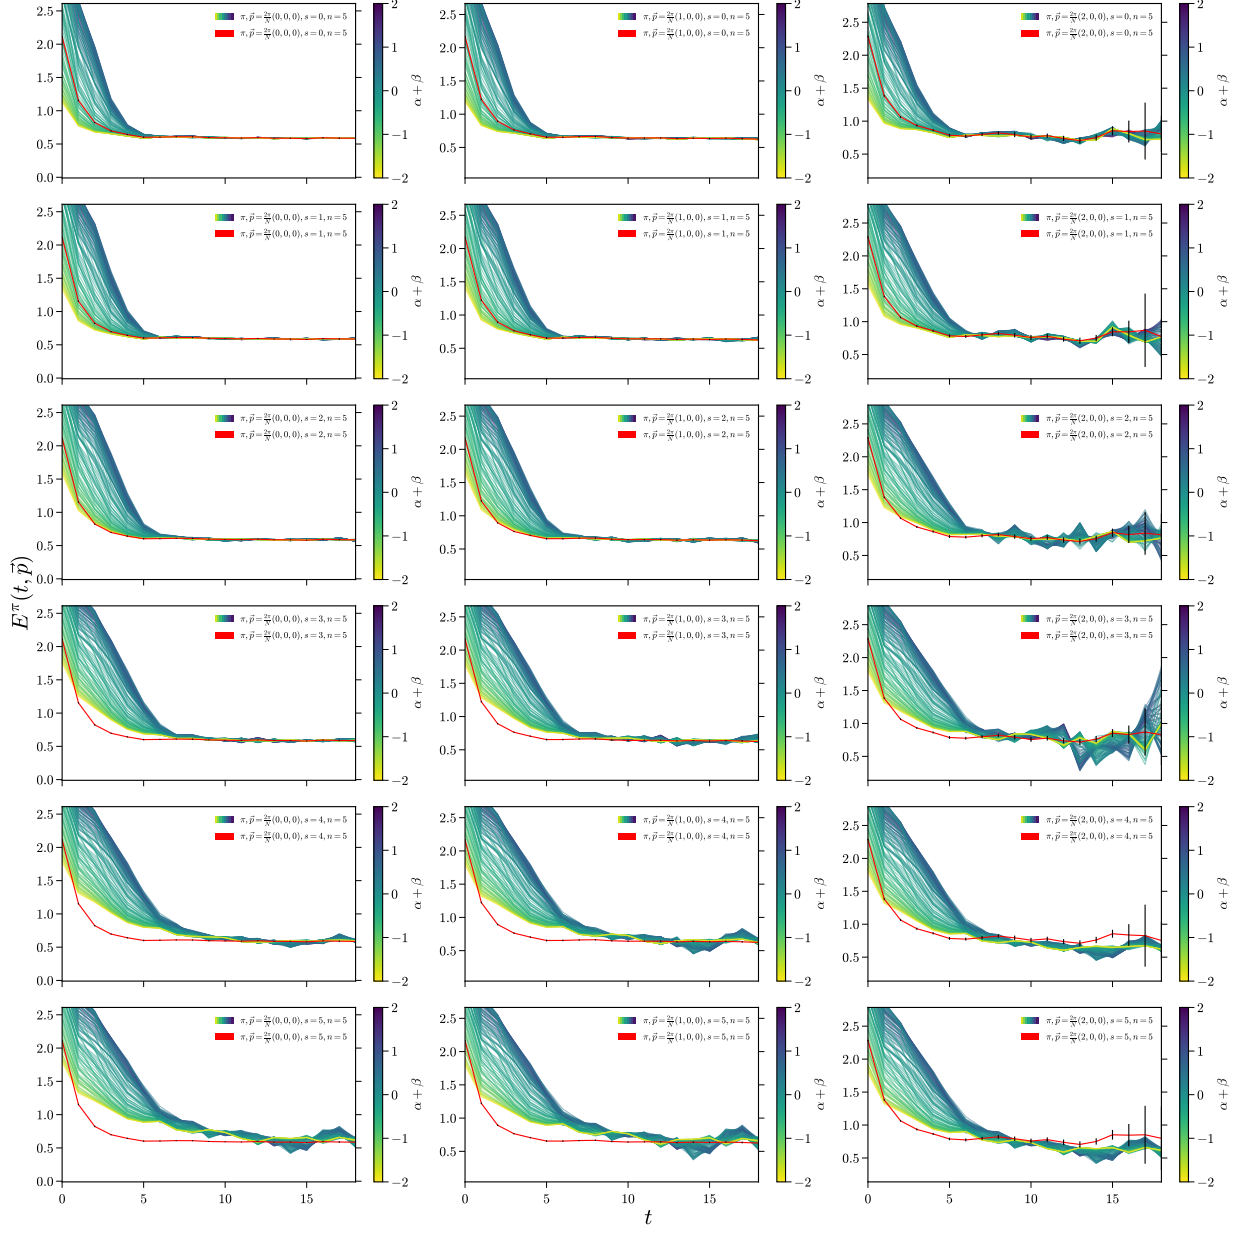

FIG. 6. Effective energy as a function of time,  $E^\pi(t, \vec{p})$  (Eq. (18)), for varying  $\alpha, \beta$  and momentum. The unsparse result is shown in red.

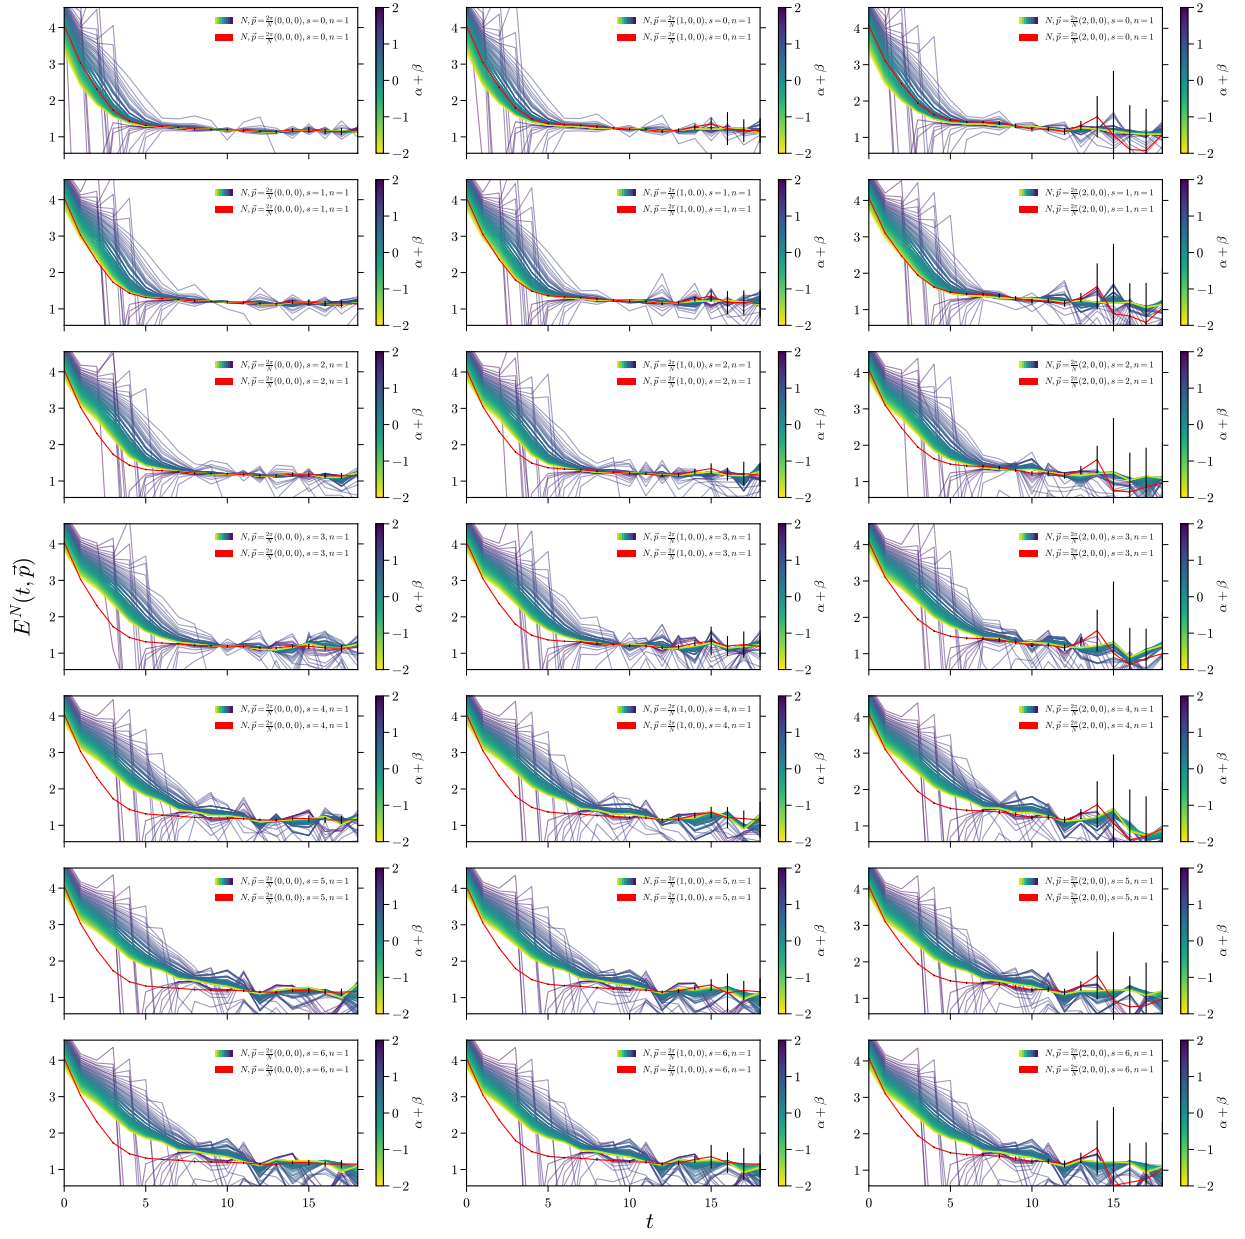

FIG. 7. Effective energy as a function of time,  $E^N(t, \vec{p})$  (Eq. (18)), for varying  $\alpha, \beta$  and momentum. The unparsened result is shown in red.

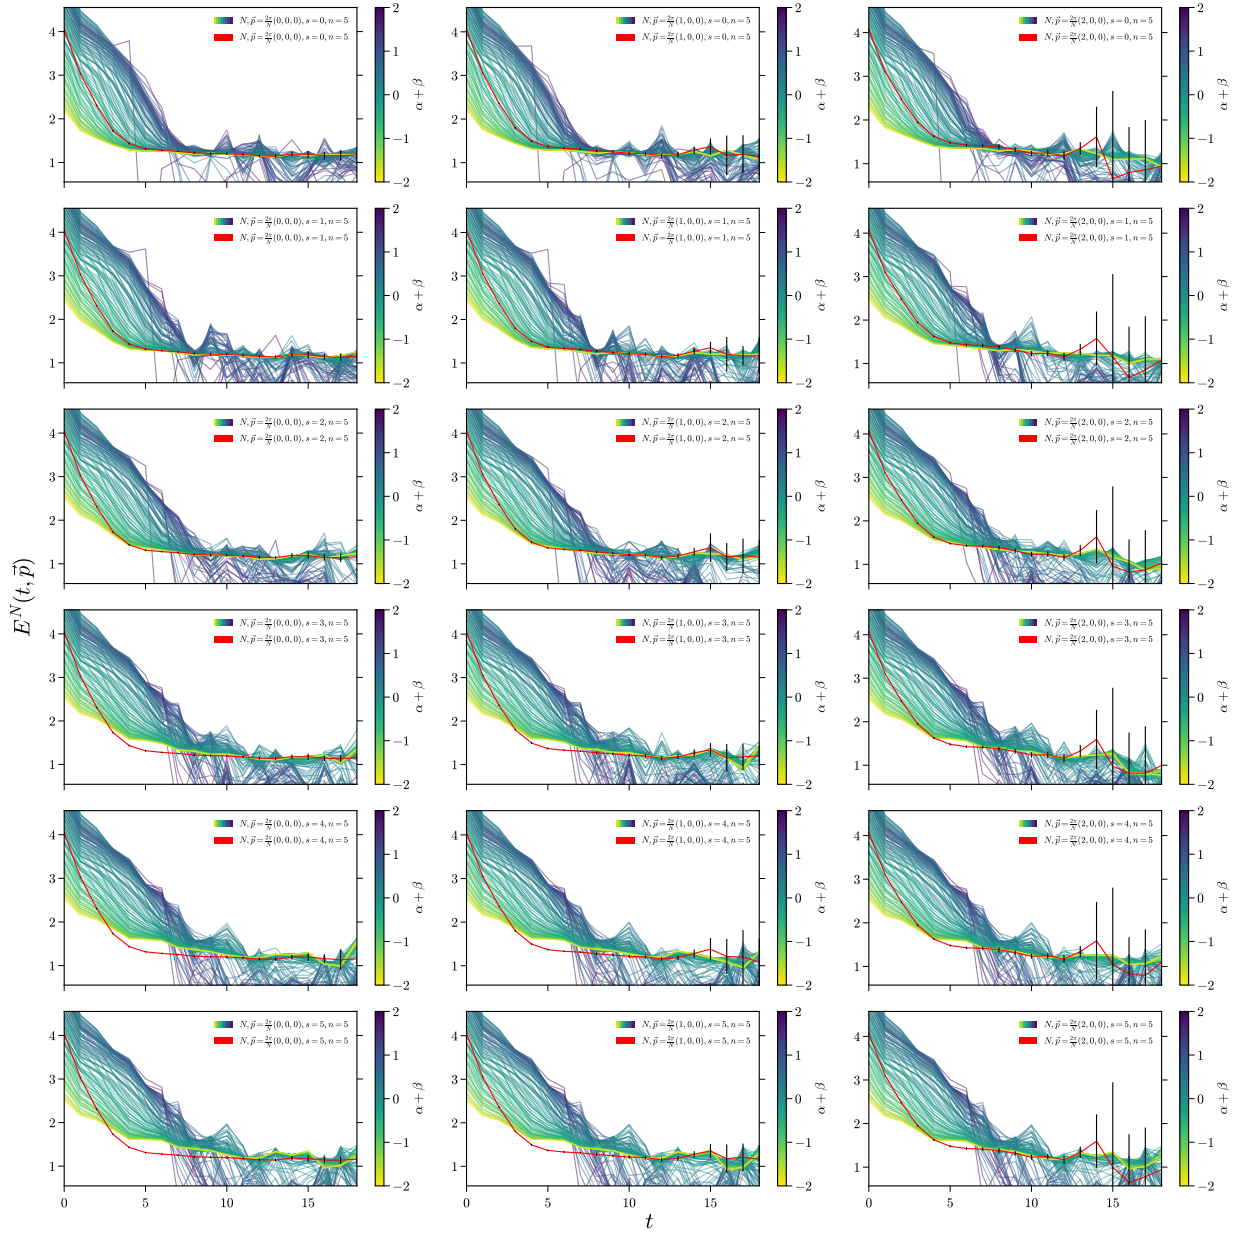

FIG. 8. Effective energy as a function of time,  $E^N(t, \vec{p})$  (Eq. (18)), for varying  $\alpha, \beta$  and momentum. The unparsened result is shown in red.



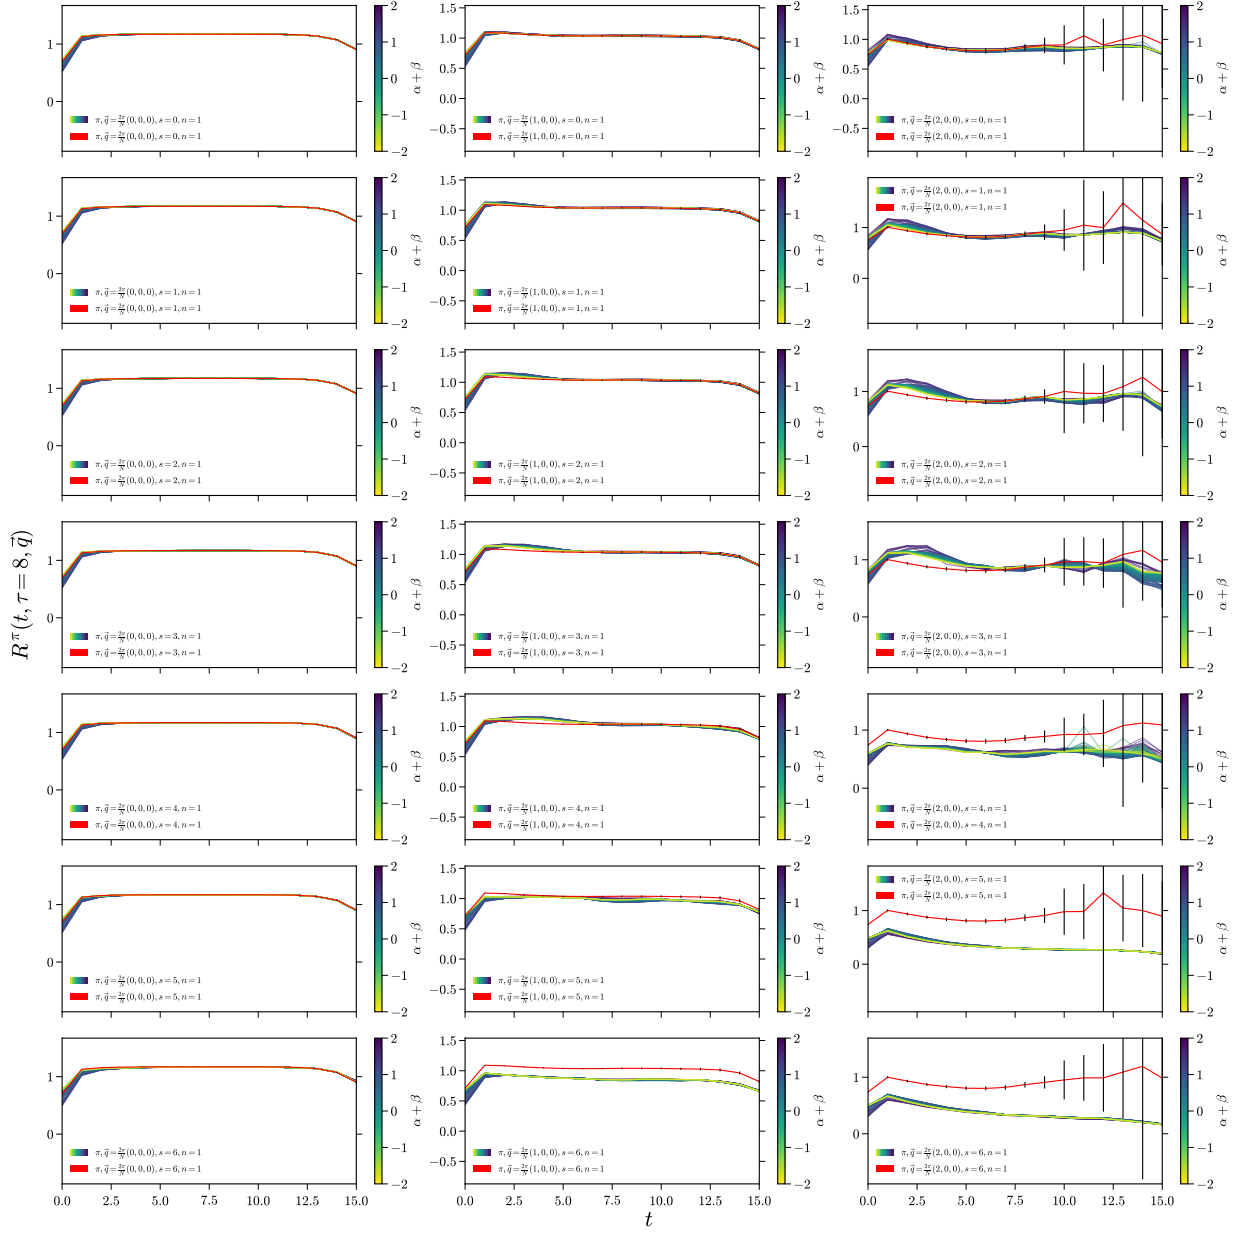

FIG. 9. Improved ratio of three- and two-point functions with  $\tau = 8$ ,  $R^\pi(t, \tau = 8, \vec{q})$  (Eqs. (30) and (33)), for varying  $\alpha, \beta$  and momentum. The unparsened result is shown in red.

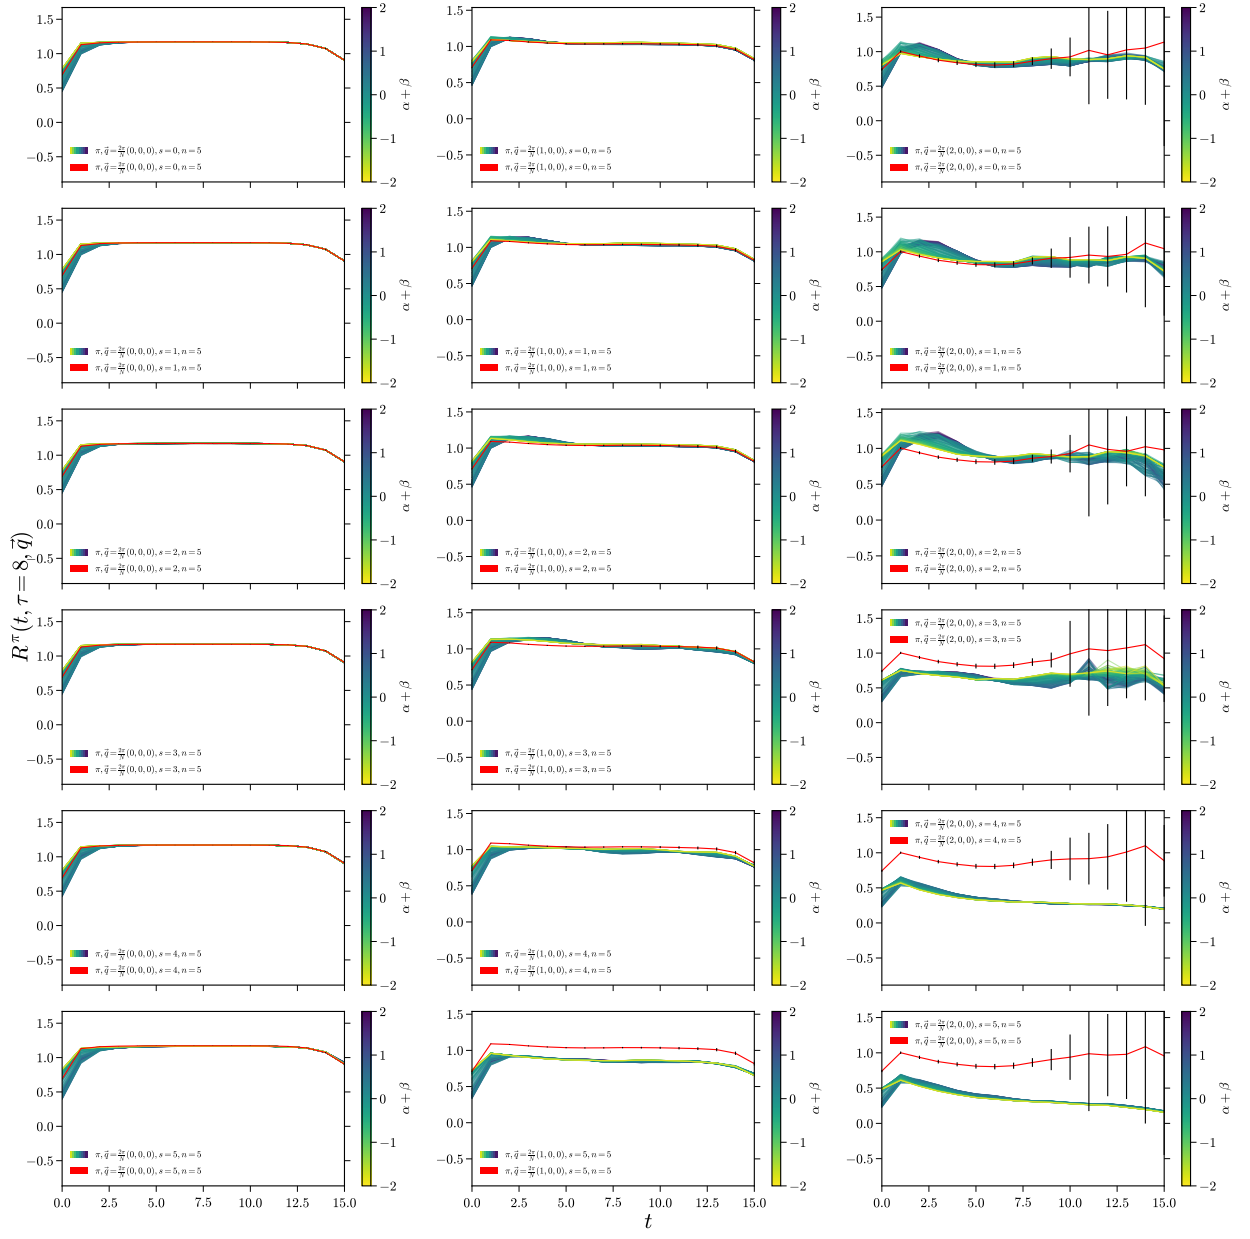

FIG. 10. Improved ratio of three- and two-point functions with  $\tau = 8$ ,  $R^\pi(t, \tau = 8, \vec{q})$  (Eqs. (30) and (33)), for varying  $\alpha, \beta$  and momentum. The unparsened result is shown in red.

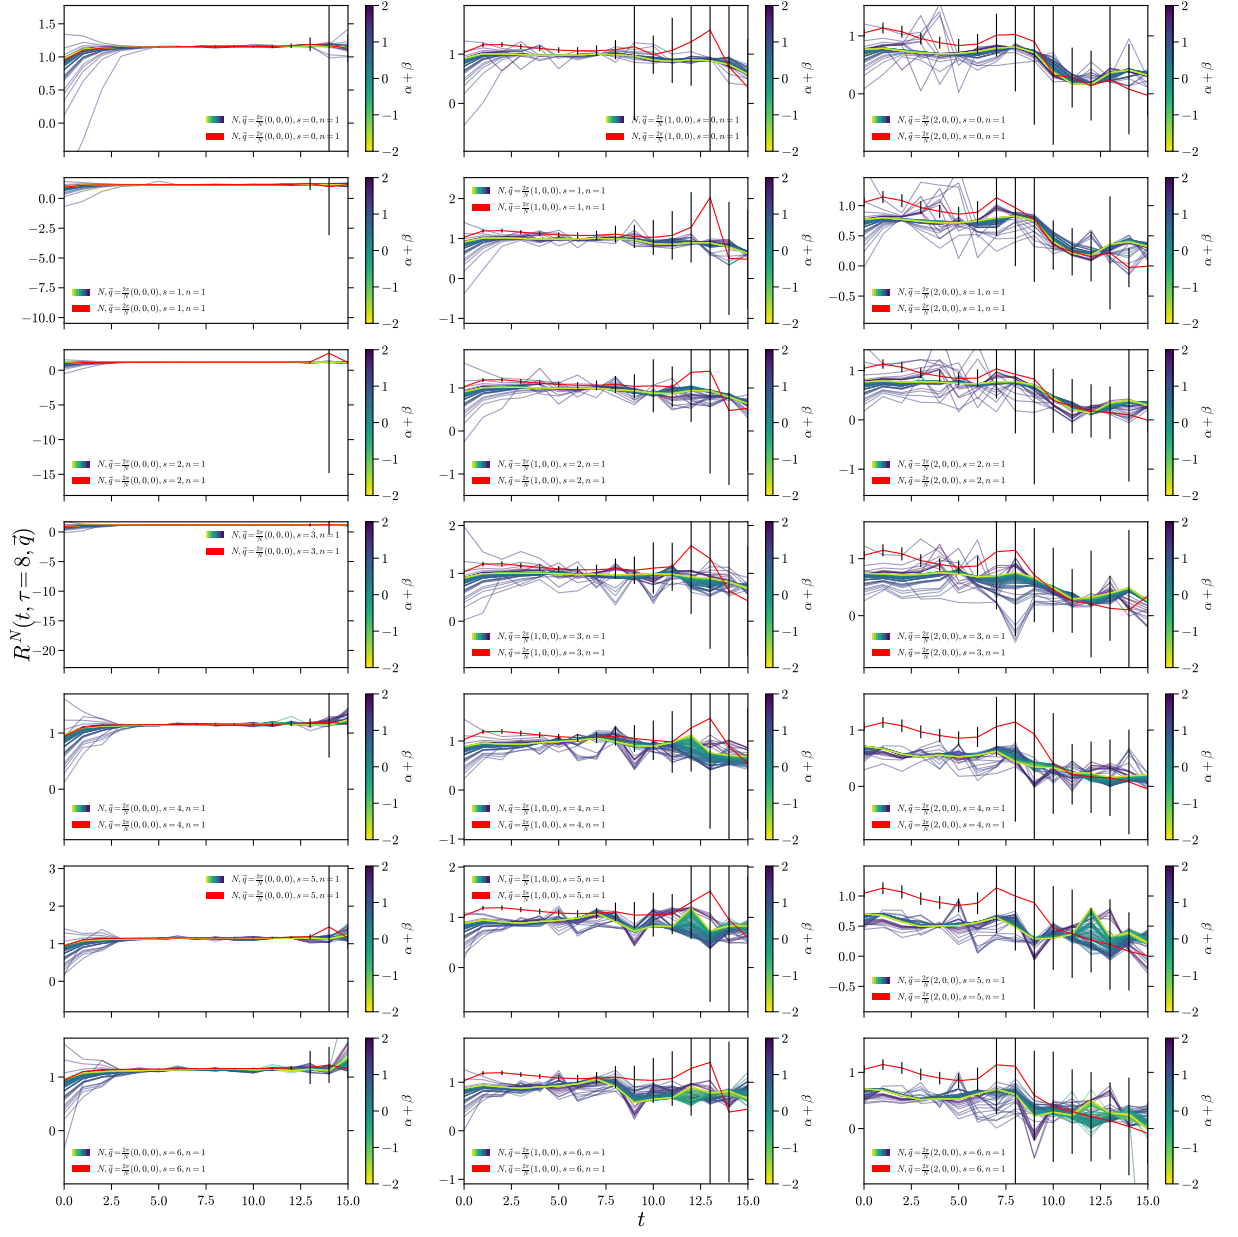

FIG. 11. Improved ratio of three- and two-point functions with  $\tau = 8$ ,  $R^N(t, \tau = 8, \vec{q})$  (Eqs. (30) and (33)), for varying  $\alpha, \beta$  and momentum. The unparsened result is shown in red.

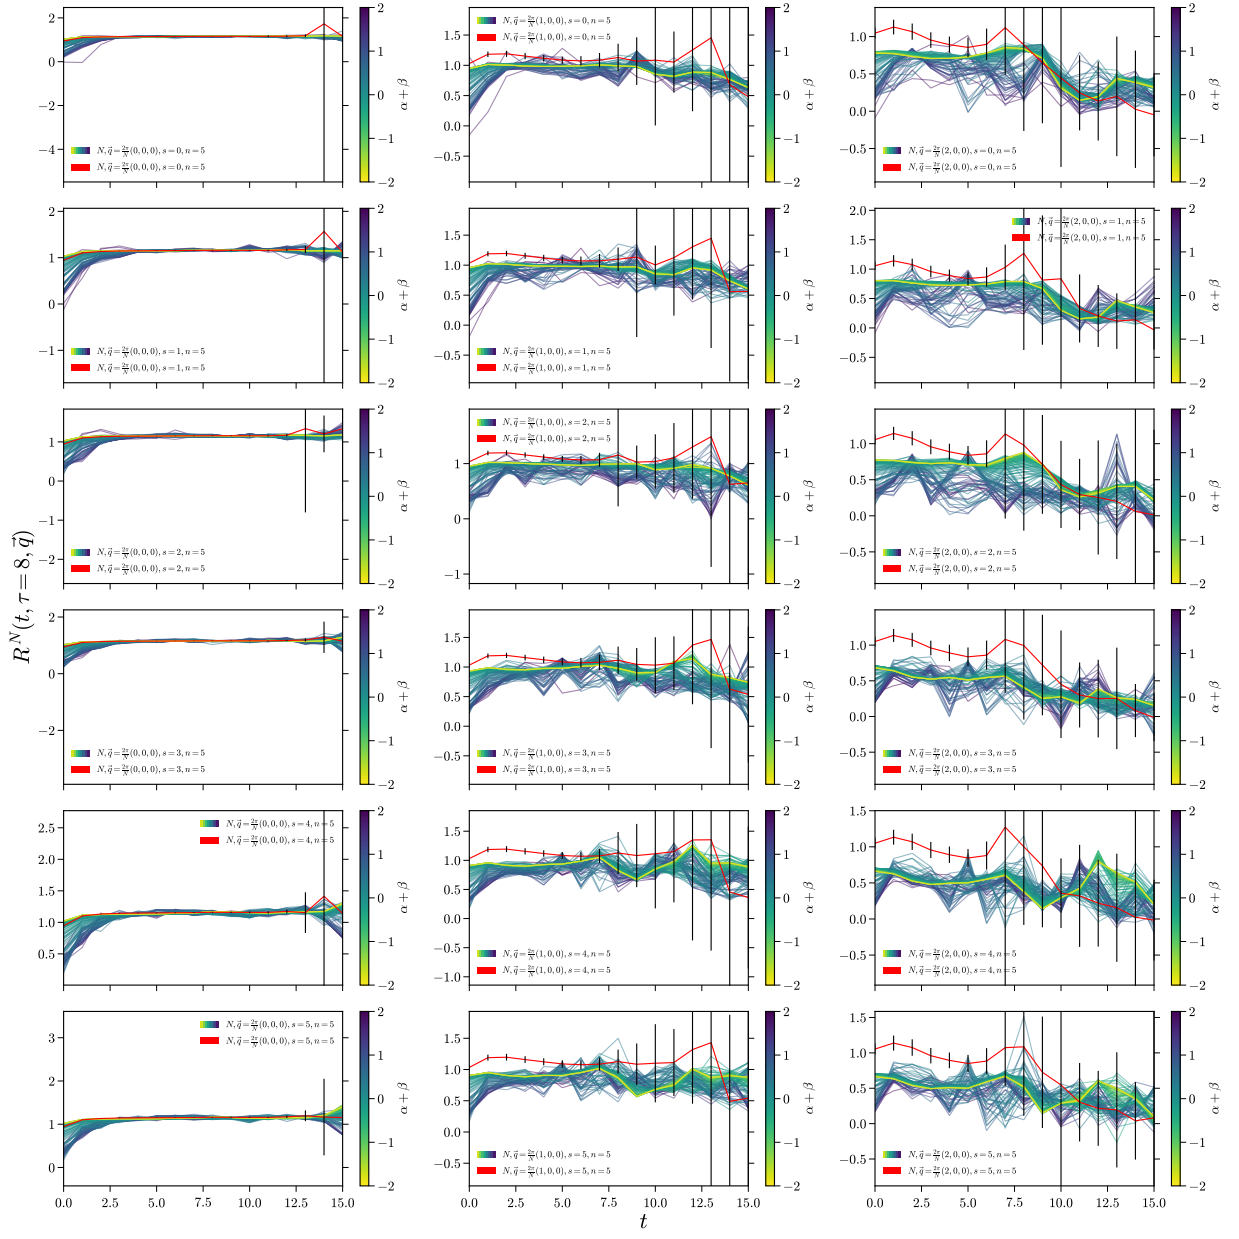

FIG. 12. Improved ratio of three- and two-point functions with  $\tau = 8$ ,  $R^N(t, \tau = 8, \vec{q})$  (Eqs. (30) and (33)), for varying  $\alpha, \beta$  and momentum. The unparsened result is shown in red.

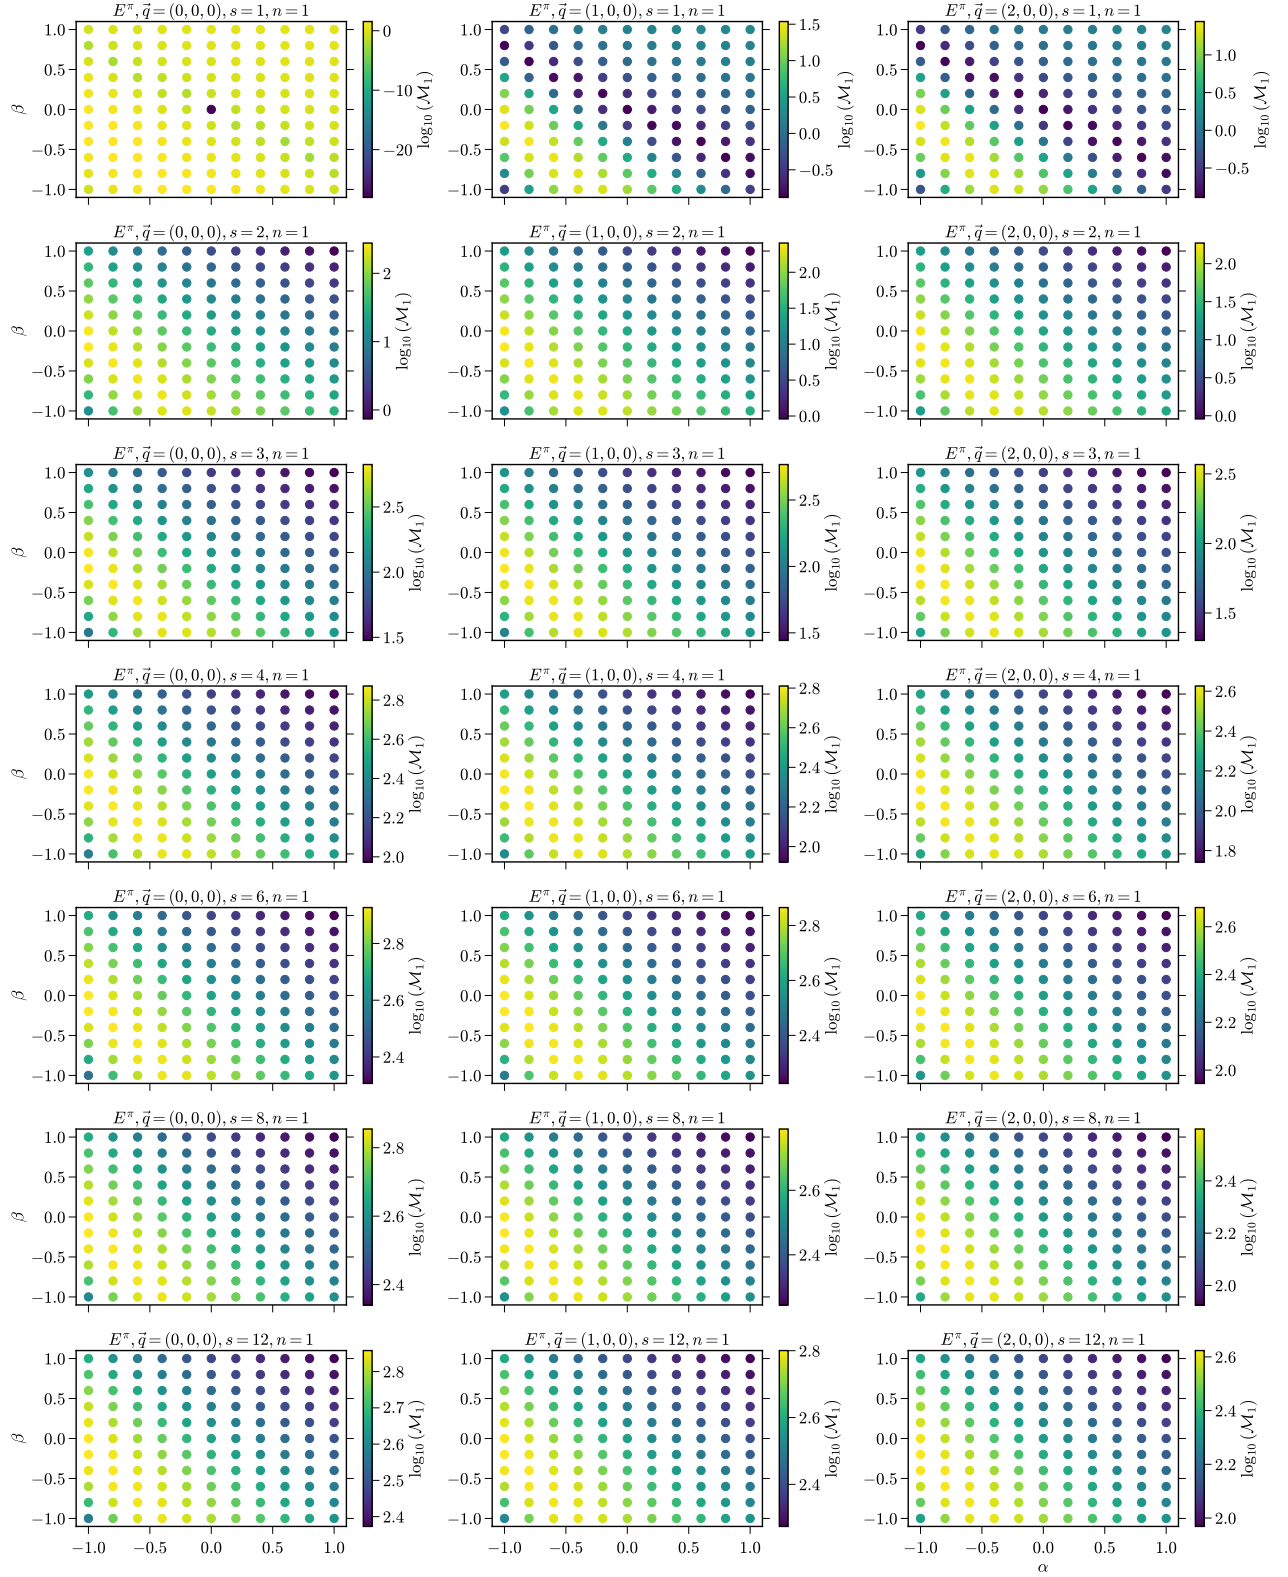

FIG. 13. Metric  $\mathcal{M}_1$  (Eq. (25)), for the pion effective energy as a function of  $\alpha, \beta$ . In this figure, there are  $n = 1$  blocking factor, three different values of momentum, and all 7 possible decimation factors.

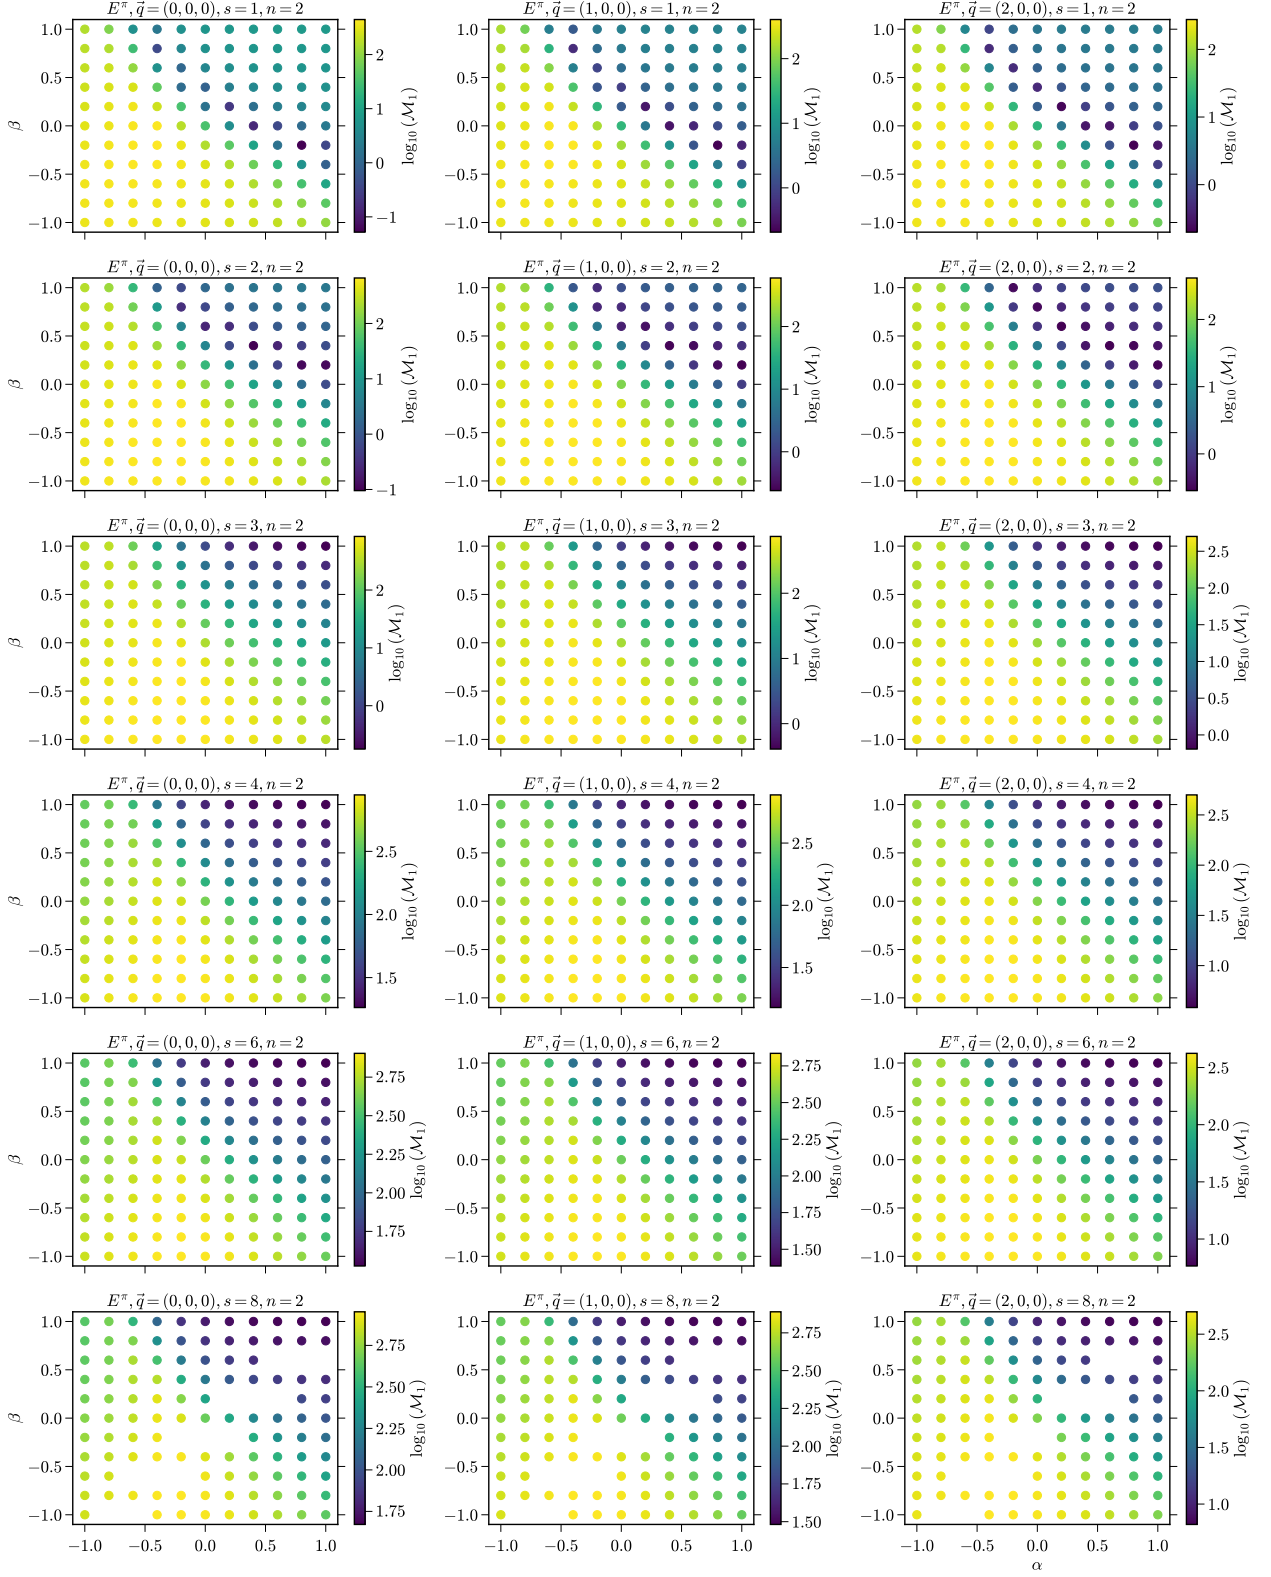

FIG. 14. Metric  $\mathcal{M}_1$  (Eq. (25)), for the pion effective energy as a function of  $\alpha, \beta$ . In this figure, there are  $n = 2$  blocking factor, three different values of momentum, and all 7 possible decimation factors.

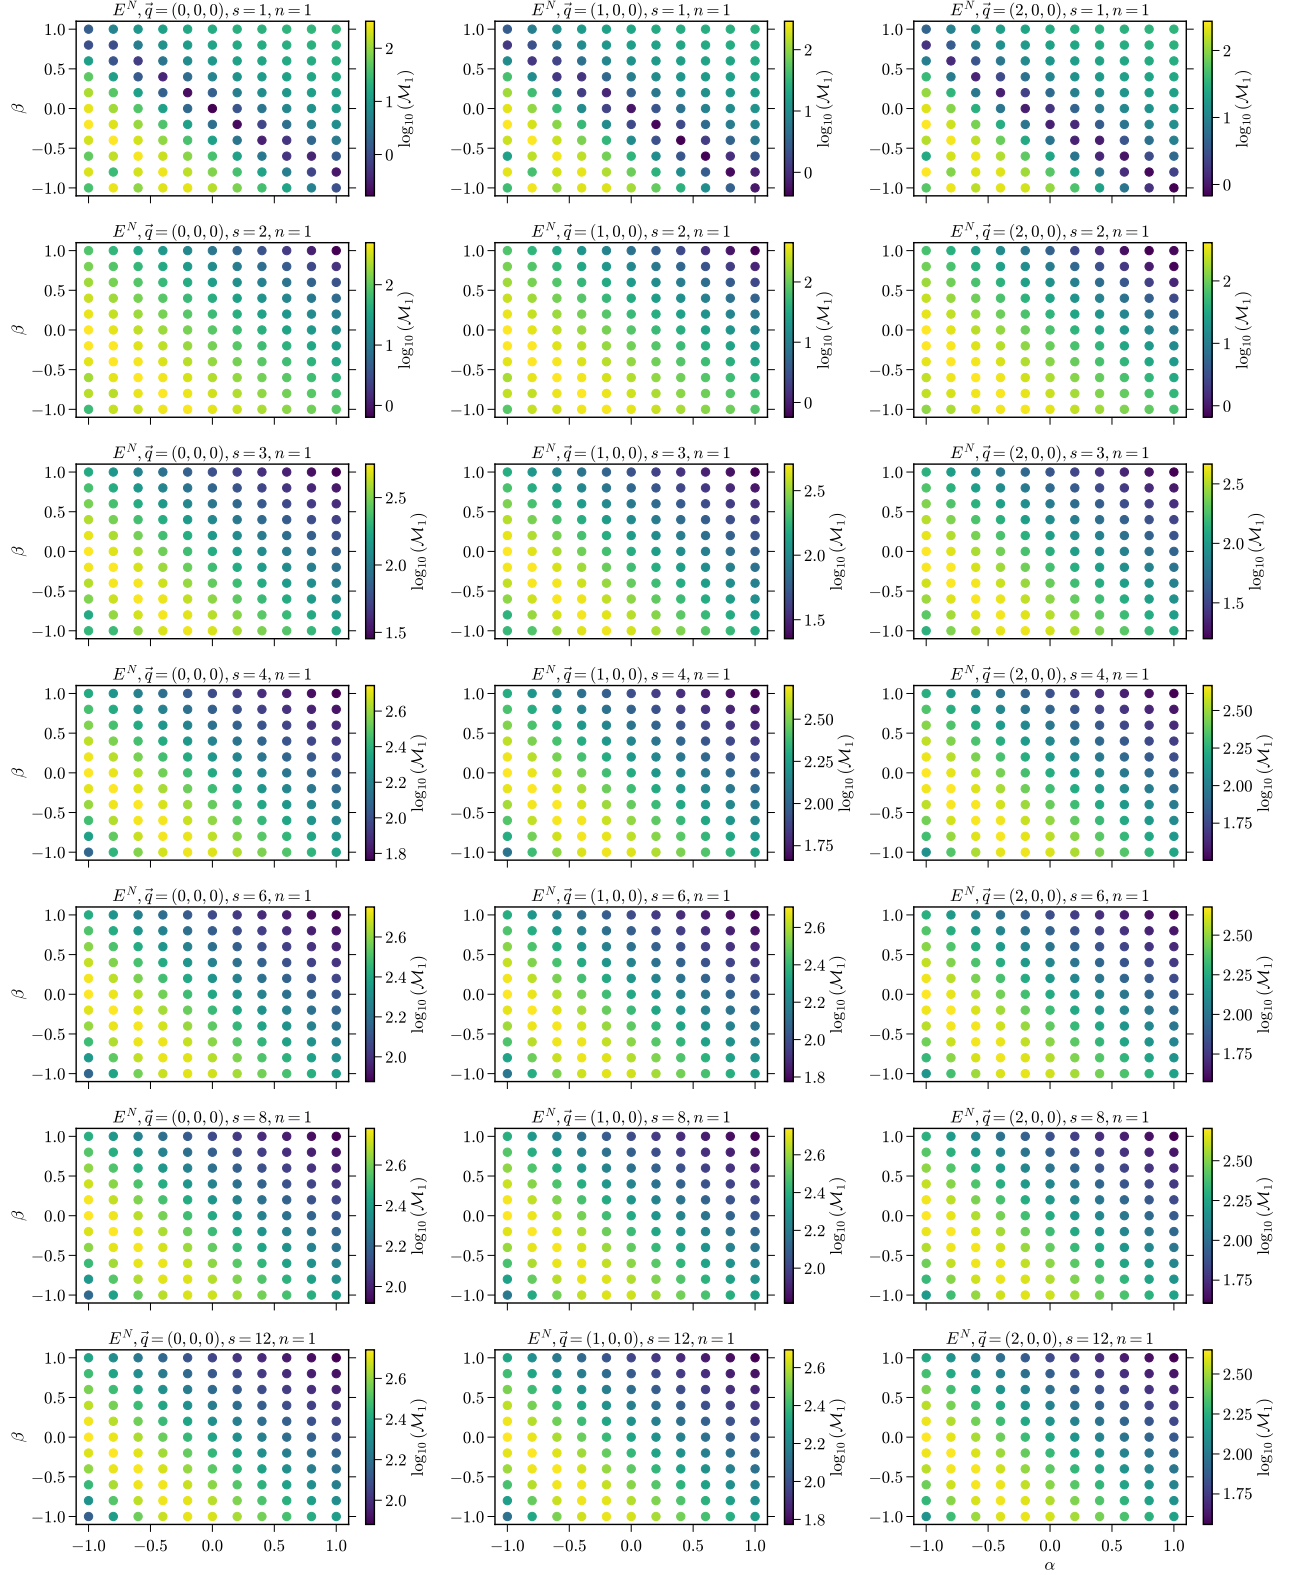

FIG. 15. Metric  $\mathcal{M}_1$  (Eq. (25)), for the proton effective energy as a function of  $\alpha, \beta$ . In this figure, there are  $n = 1$  blocking factor, three different values of momentum, and all 7 possible decimation factors.



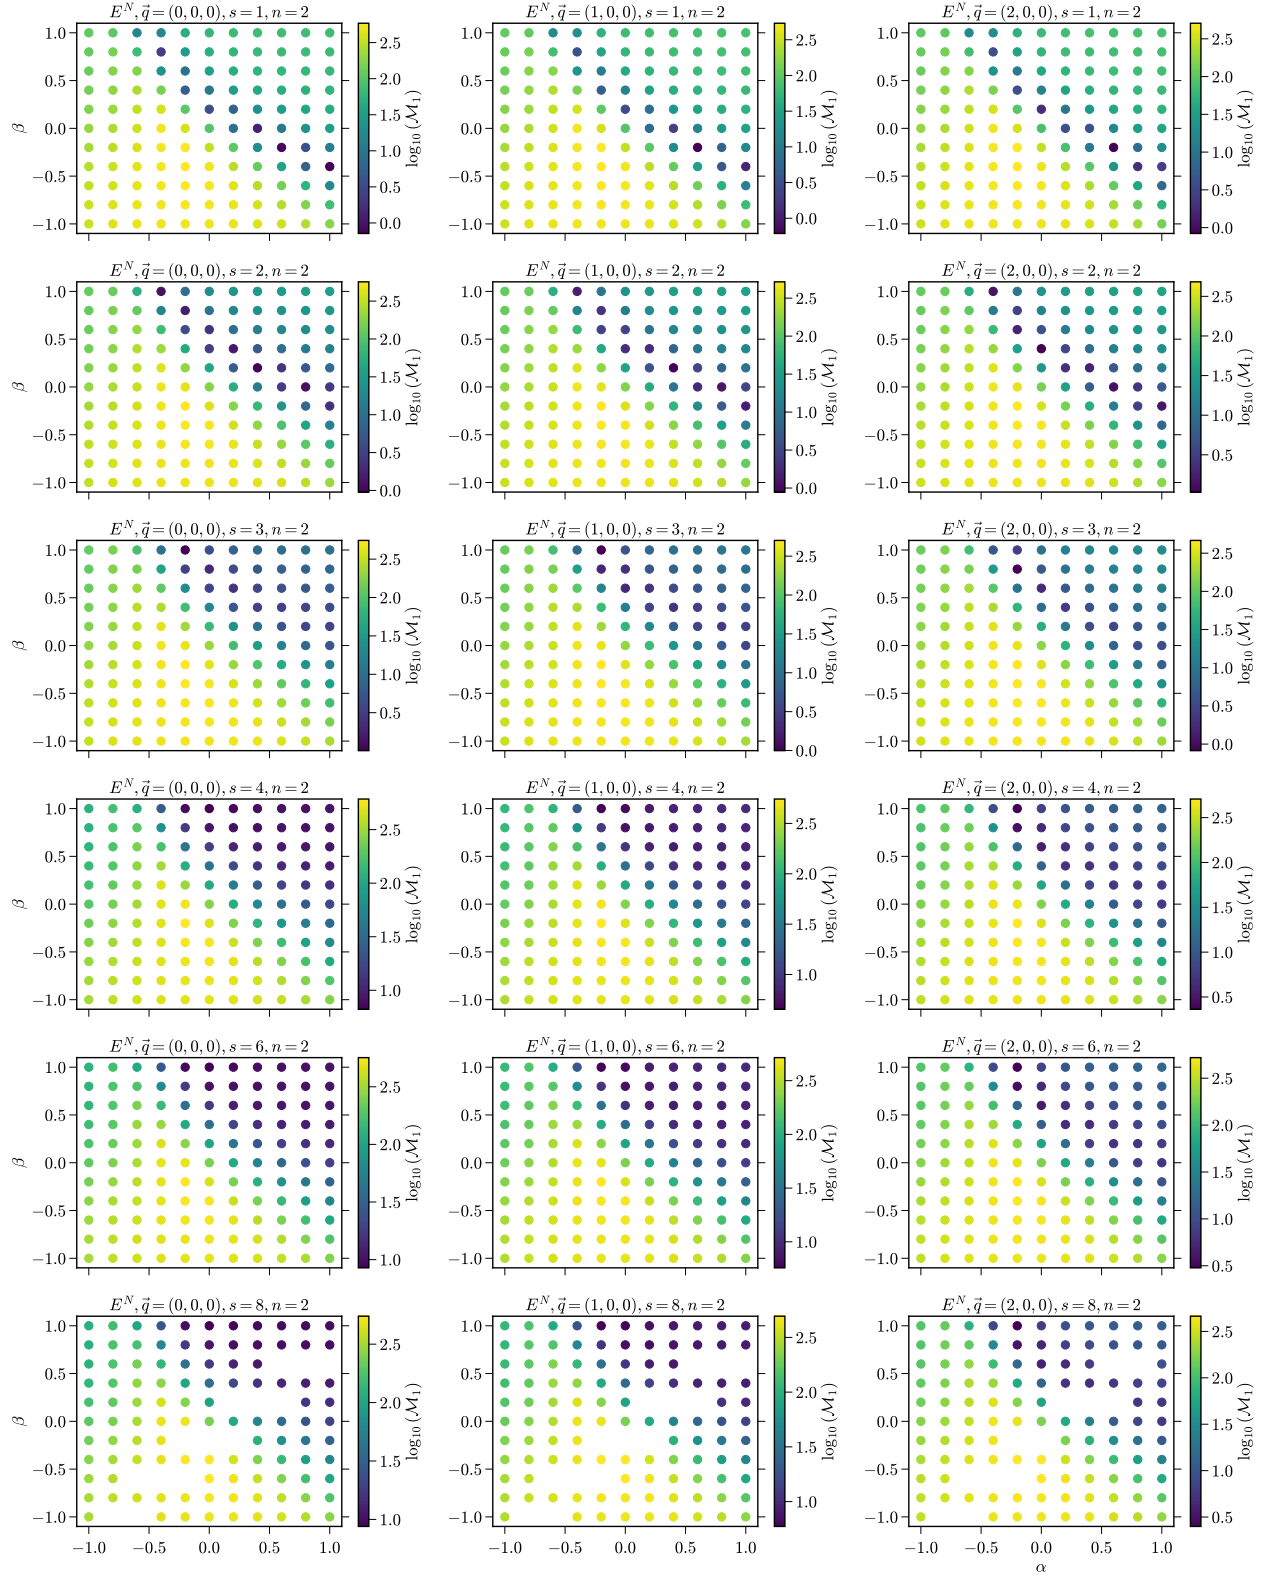

FIG. 16. Metric  $\mathcal{M}_1$  (Eq. (25)), for the proton effective energy as a function of  $\alpha, \beta$ . In this figure, there are  $n = 2$  blocking factor, three different values of momentum, and all 7 possible decimation factors.



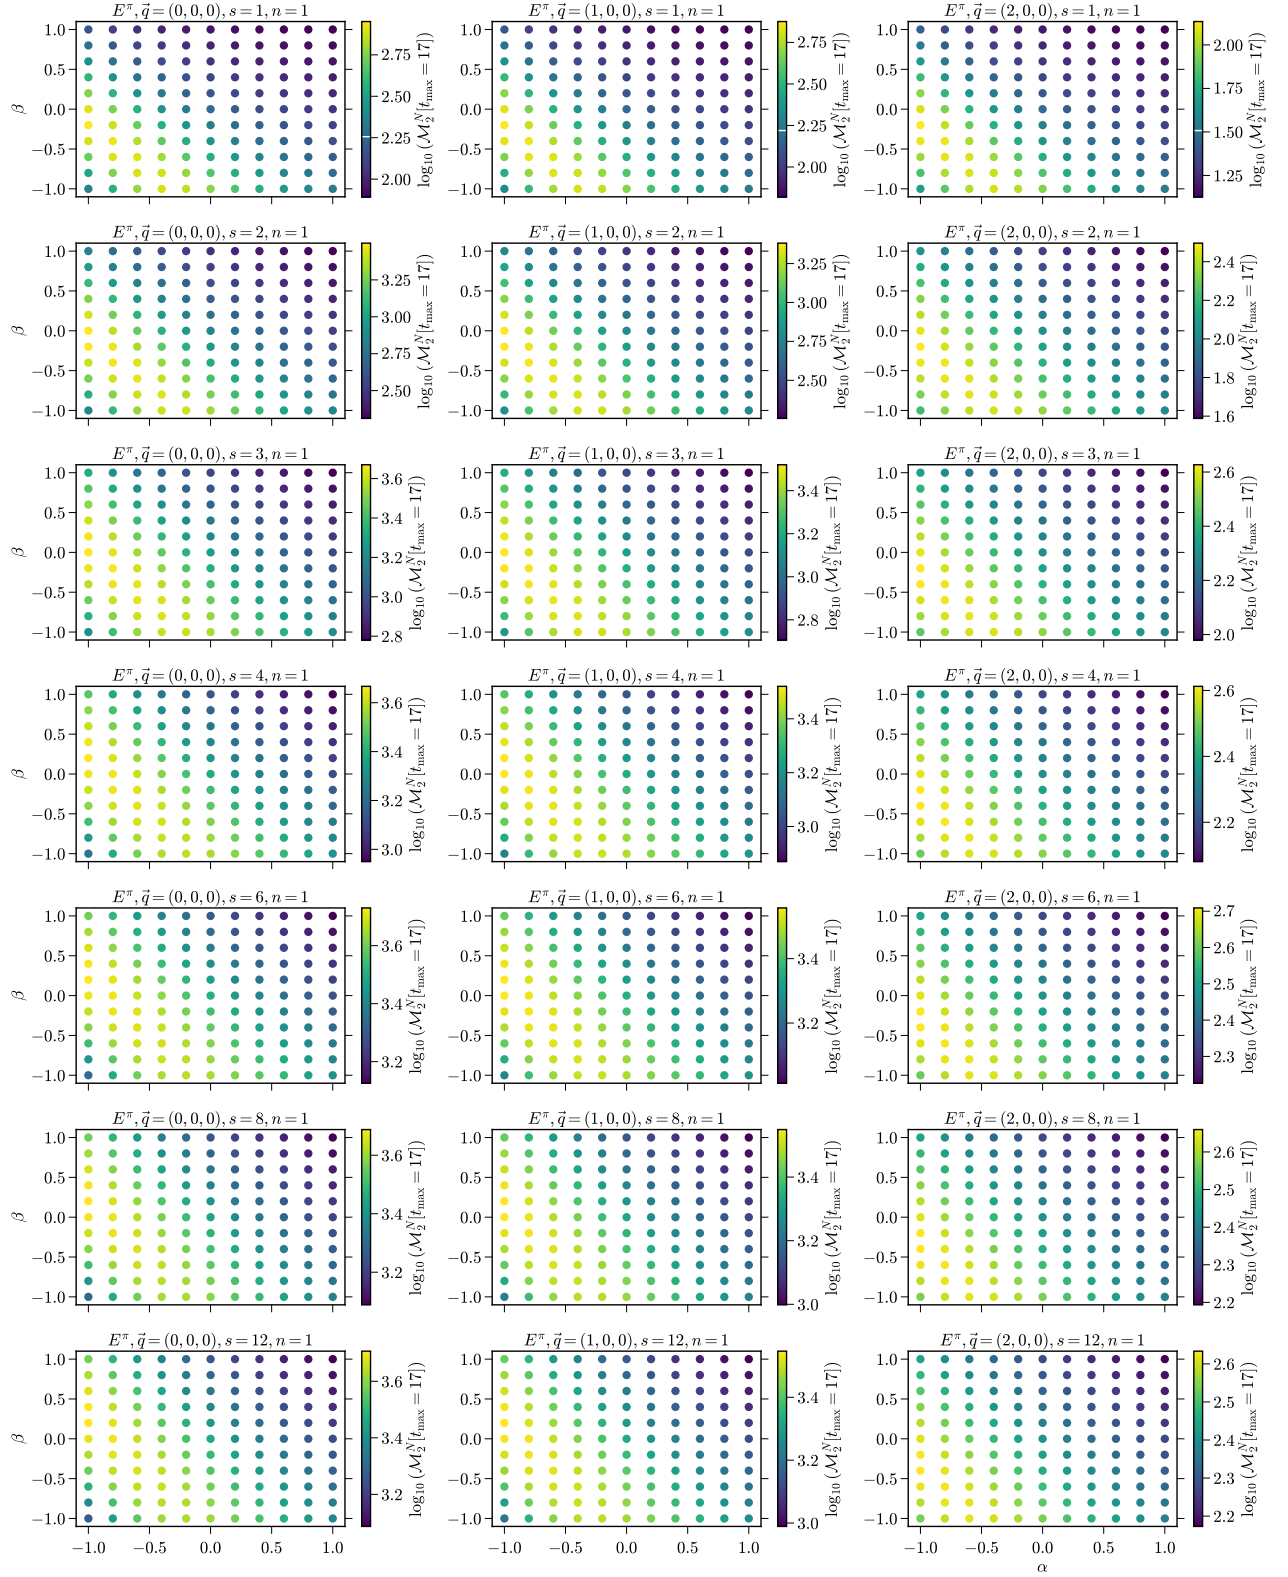

FIG. 17. Metric  $\mathcal{M}_2$  (Eq. (26)), for the pion effective energy as a function of  $\alpha, \beta$ . In this figure, there are  $n = 1$  blocking factor, three different values of momentum, and all 7 possible decimation factors.

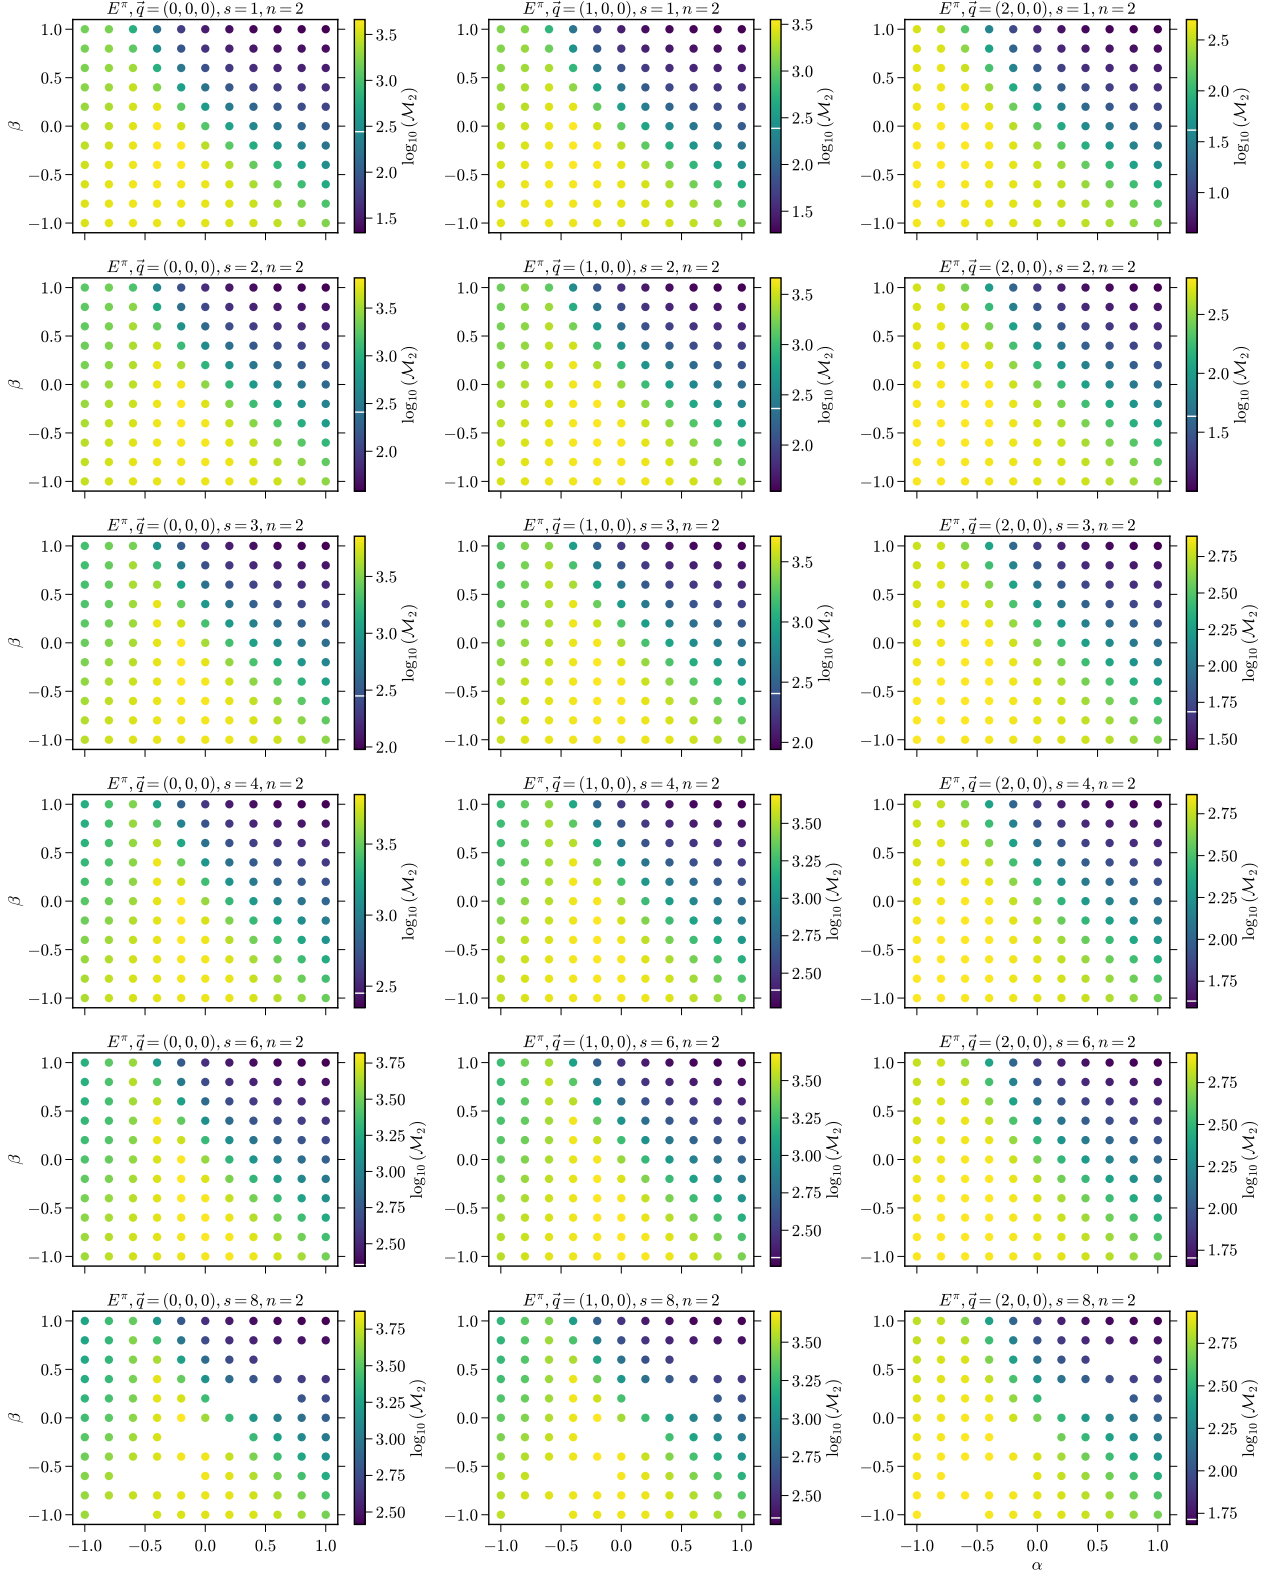

FIG. 18. Metric  $\mathcal{M}_2$  (Eq. (26)), for the pion effective energy as a function of  $\alpha, \beta$ . In this figure, there are  $n = 2$  blocking factor, three different values of momentum, and all 7 possible decimation factors.

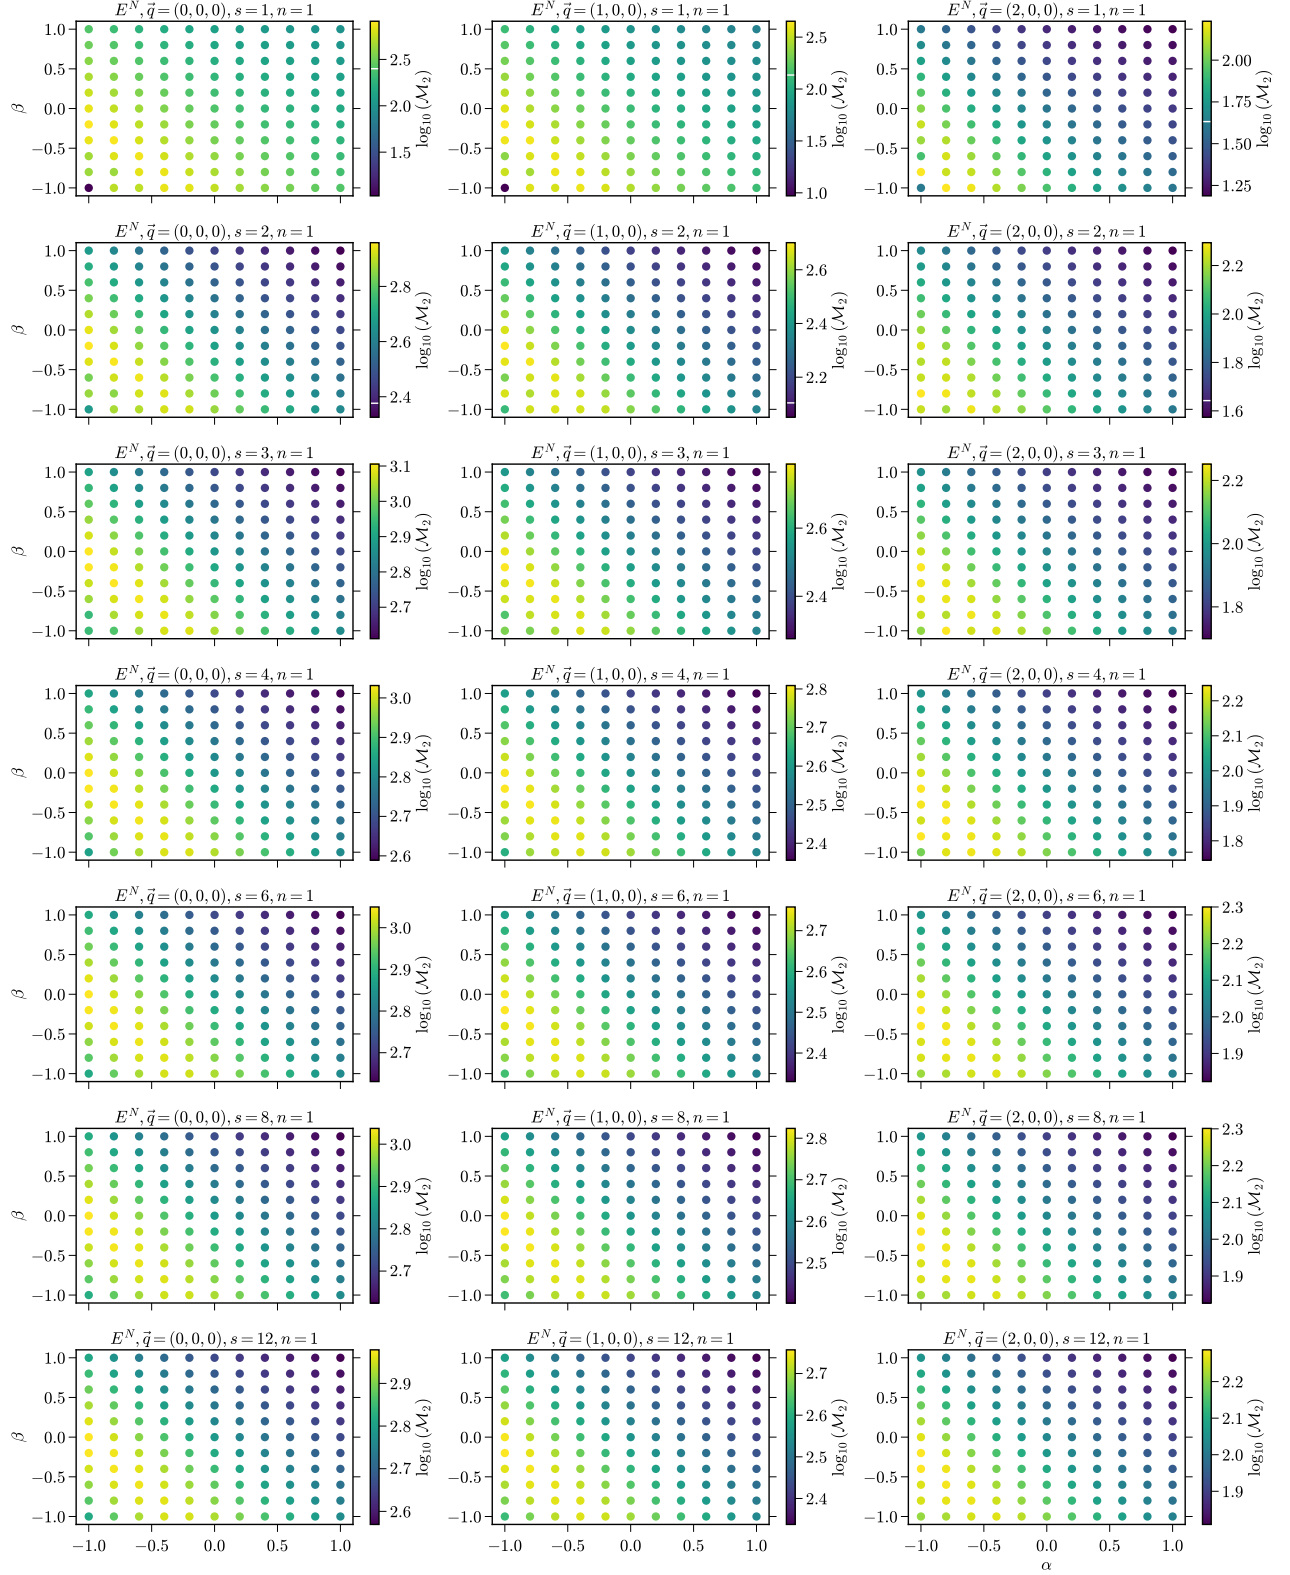

FIG. 19. Metric  $\mathcal{M}_2$  (Eq. (26)), for the proton effective energy as a function of  $\alpha, \beta$ . In this figure, there are  $n = 1$  blocking factor, three different values of momentum, and all 7 possible decimation factors.

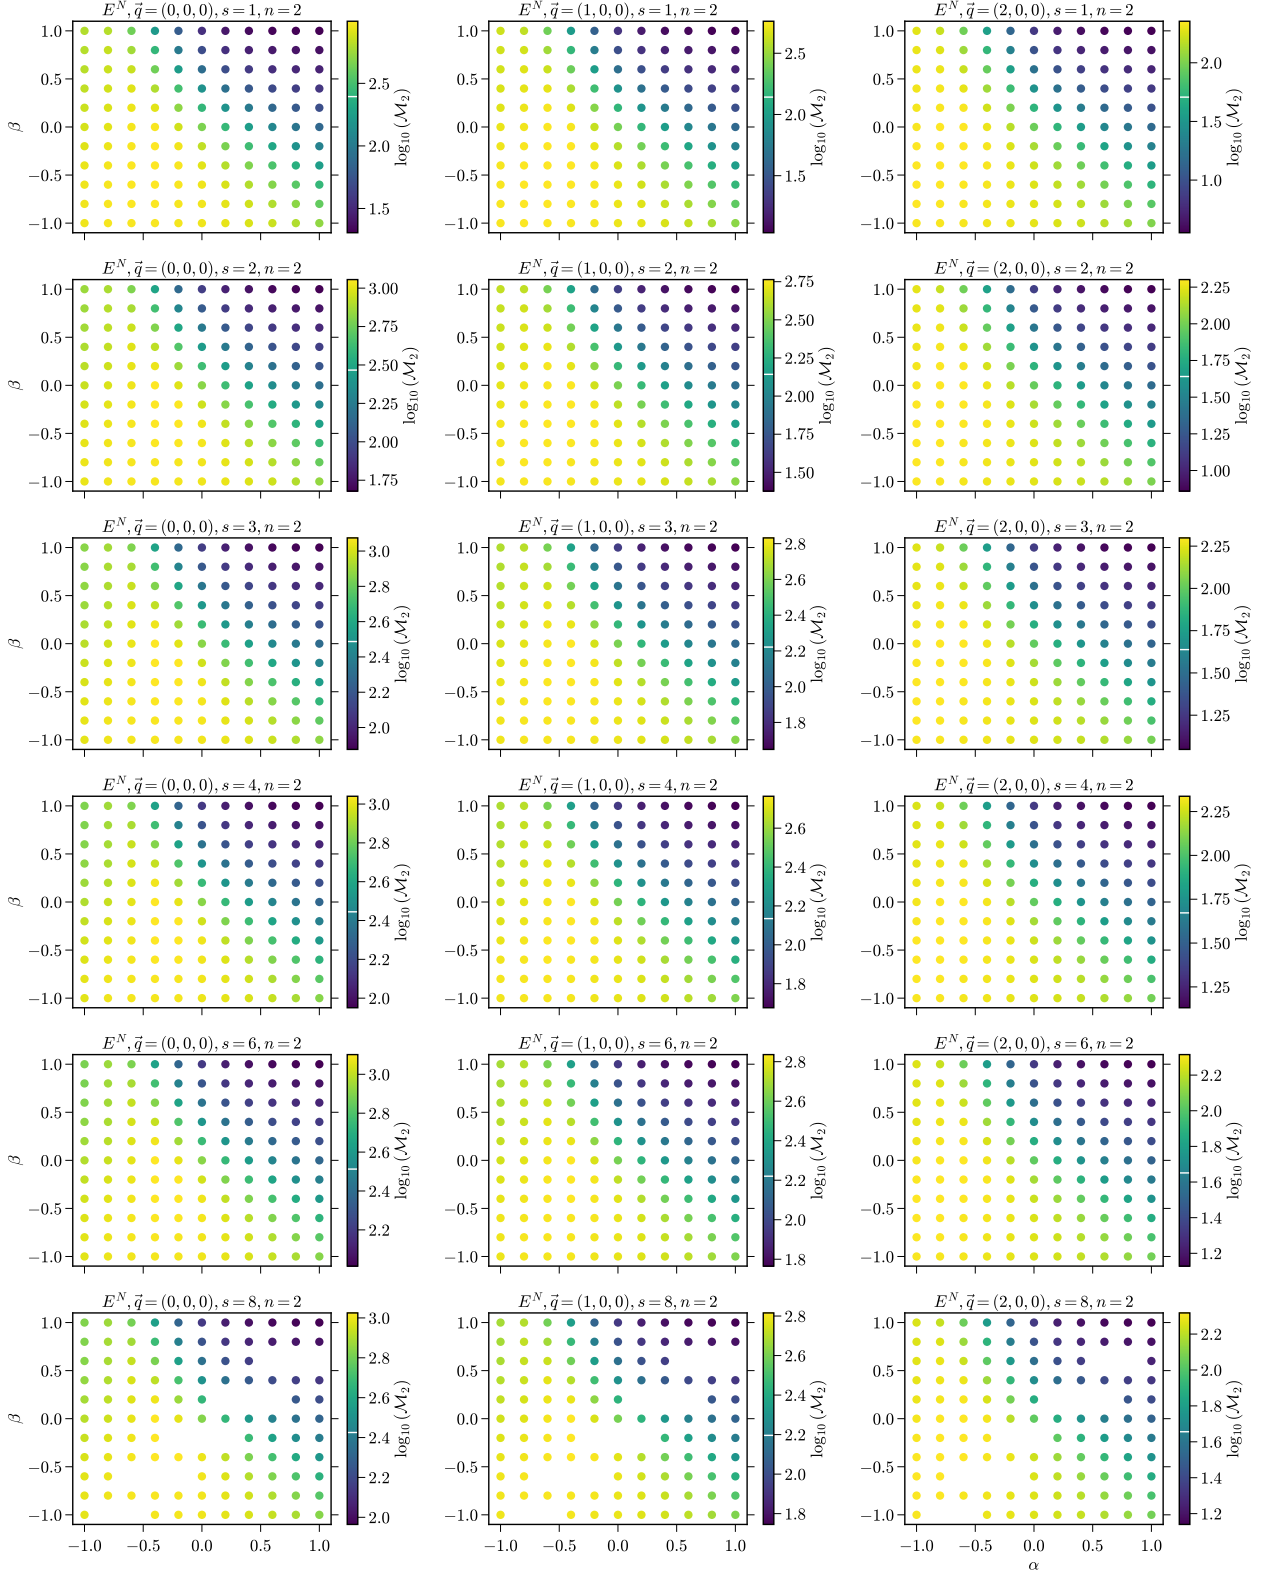

FIG. 20. Metric  $\mathcal{M}_2$  (Eq. (26)), for the proton effective energy as a function of  $\alpha, \beta$ . In this figure, there are  $n = 2$  blocking factor, three different values of momentum, and all 7 possible decimation factors.

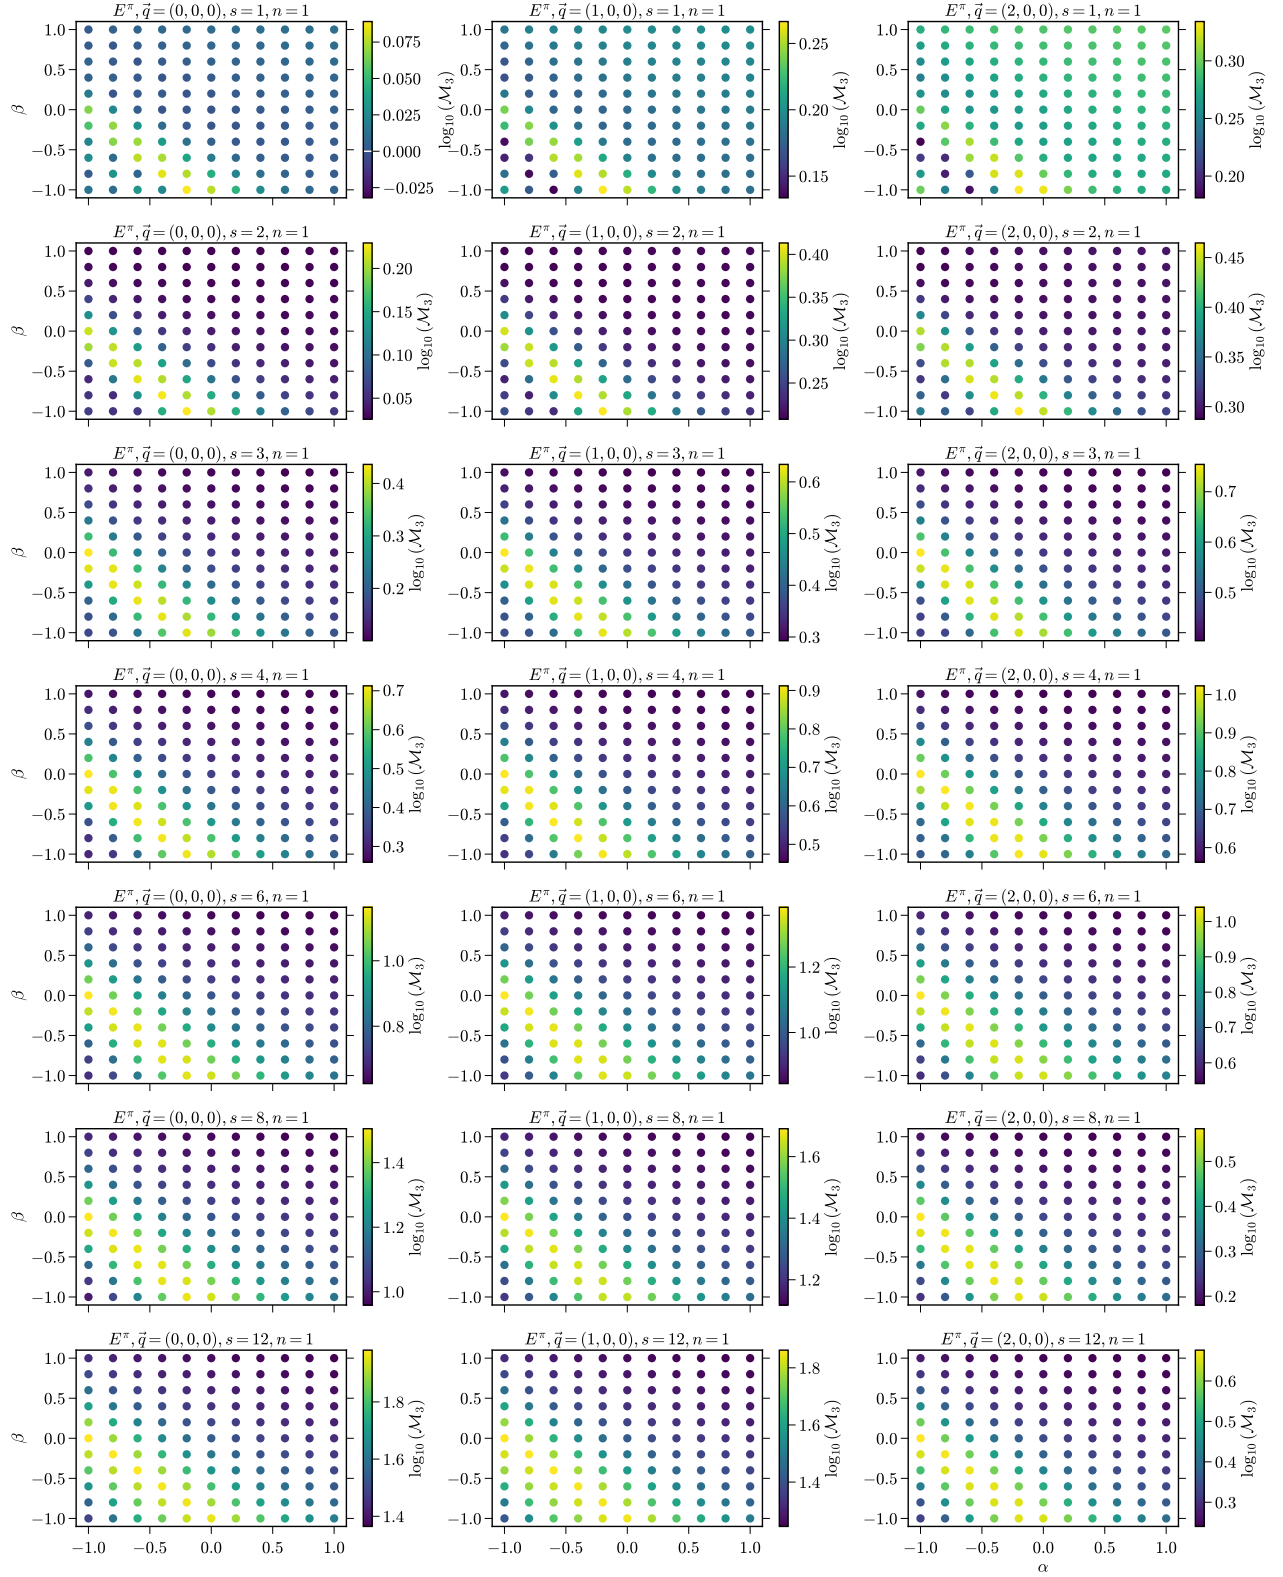

FIG. 21. Metric  $\mathcal{M}_3$  (Eq. (27)), for the pion effective energy as a function of  $\alpha, \beta$ . In this figure, there are  $n = 1$  blocking factor, three different values of momentum, and all 7 possible decimation factors.

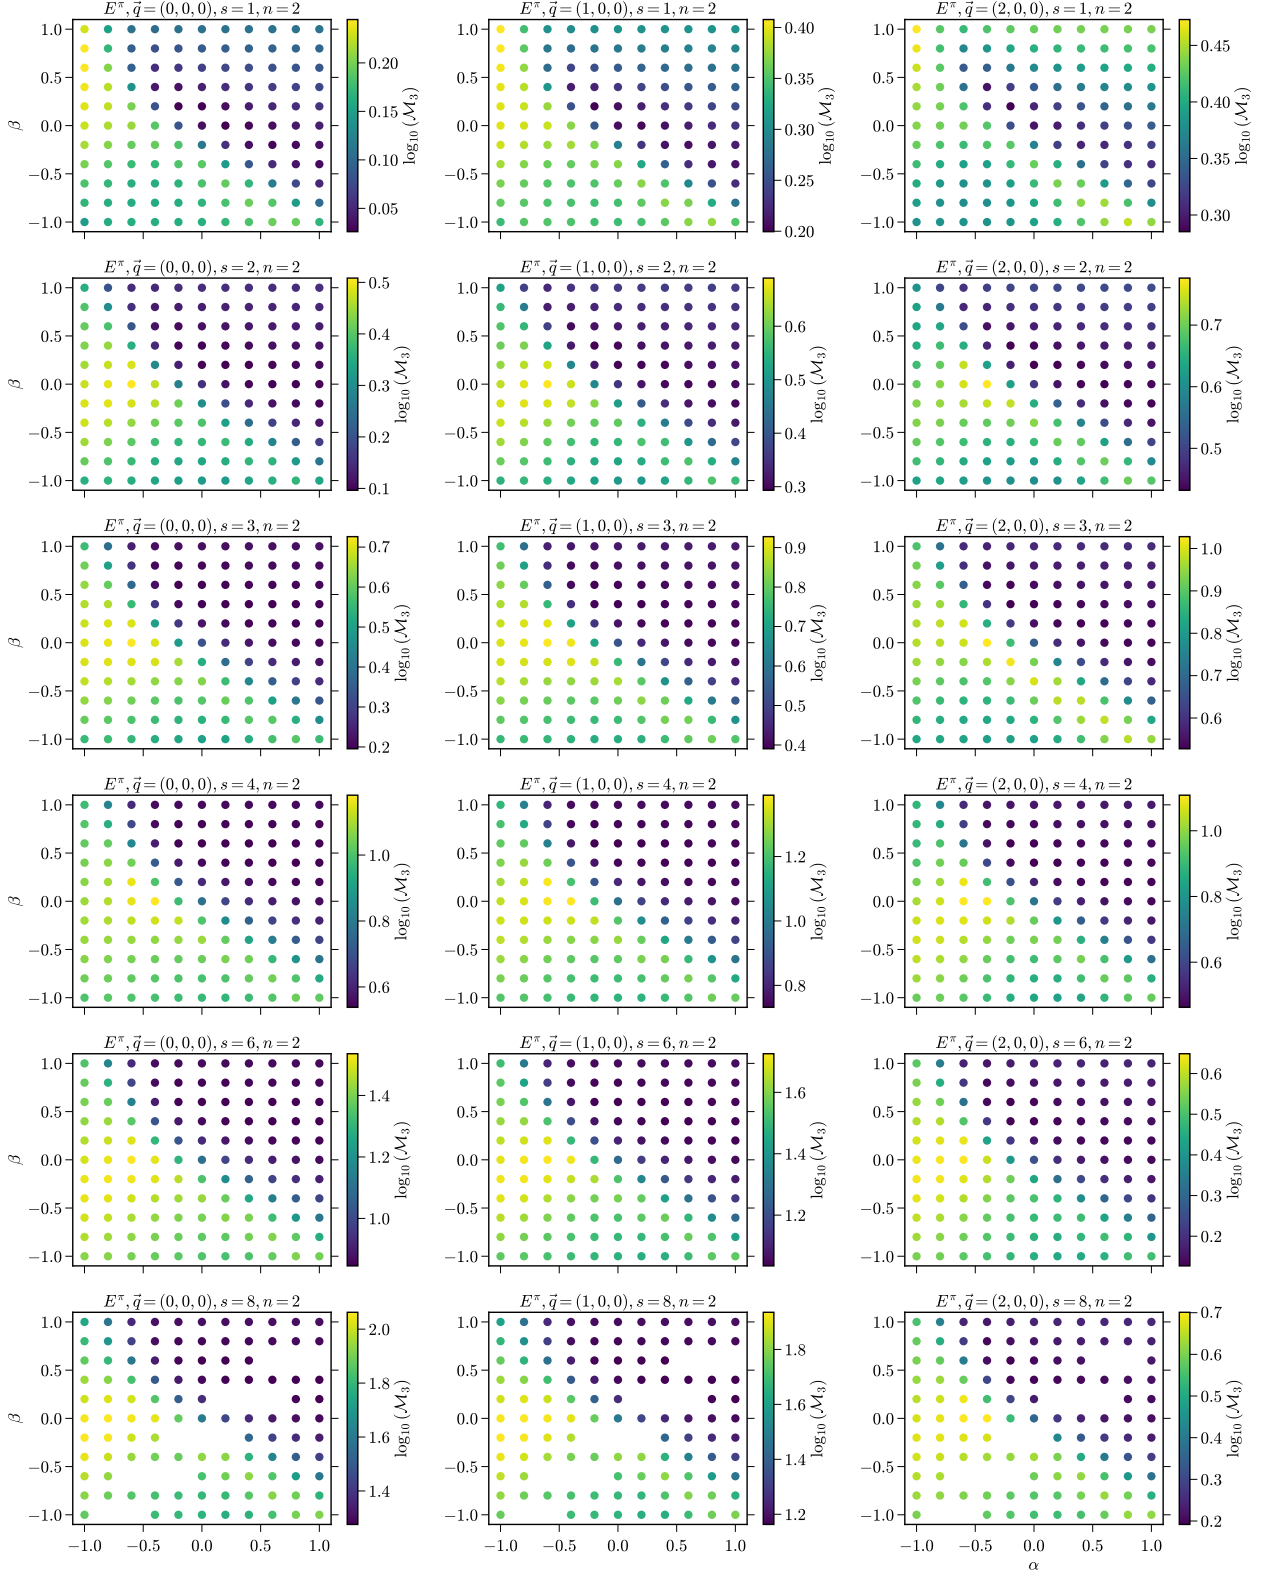

FIG. 22. Metric  $\mathcal{M}_3$  (Eq. (27)), for the pion effective energy as a function of  $\alpha, \beta$ . In this figure, there are  $n = 2$  blocking factor, three different values of momentum, and all 7 possible decimation factors.



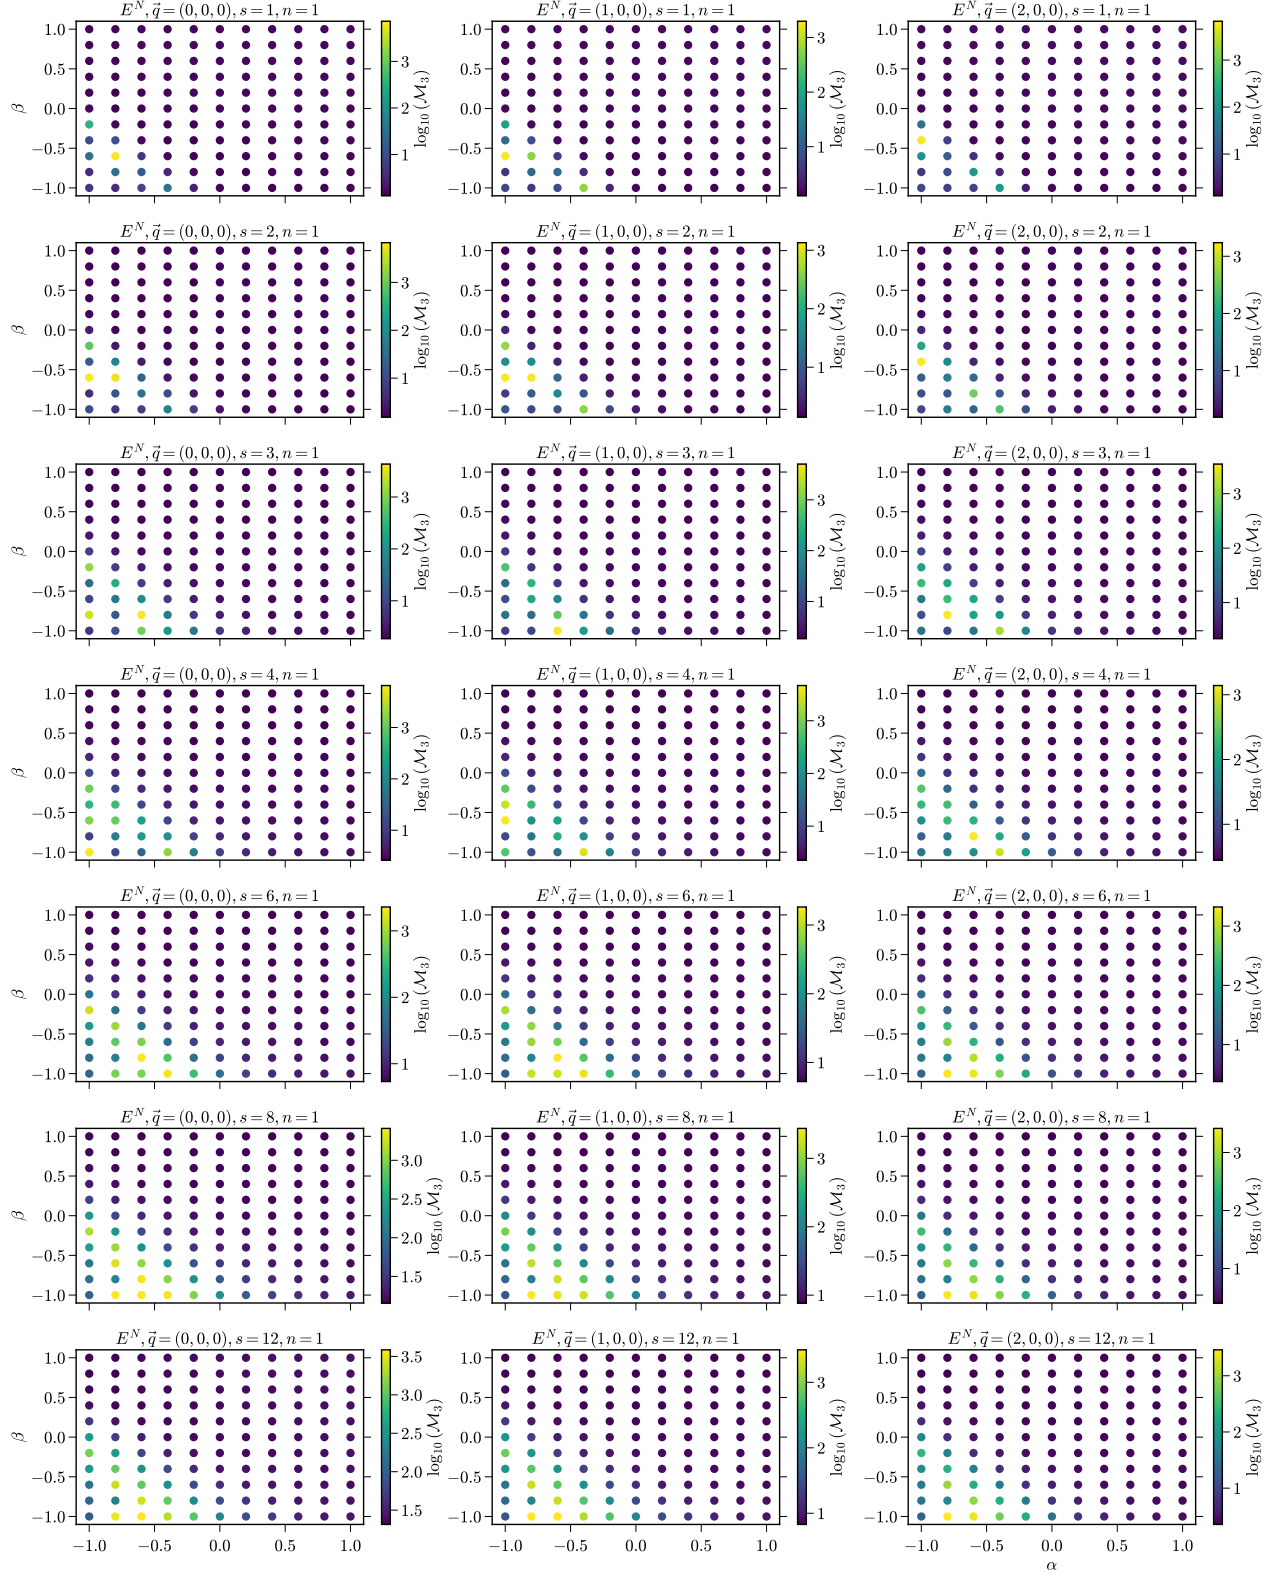

FIG. 23. Metric  $\mathcal{M}_3$  (Eq. (27)), for the proton effective energy as a function of  $\alpha, \beta$ . In this figure, there are  $n = 1$  blocking factor, three different values of momentum, and all 7 possible decimation factors.

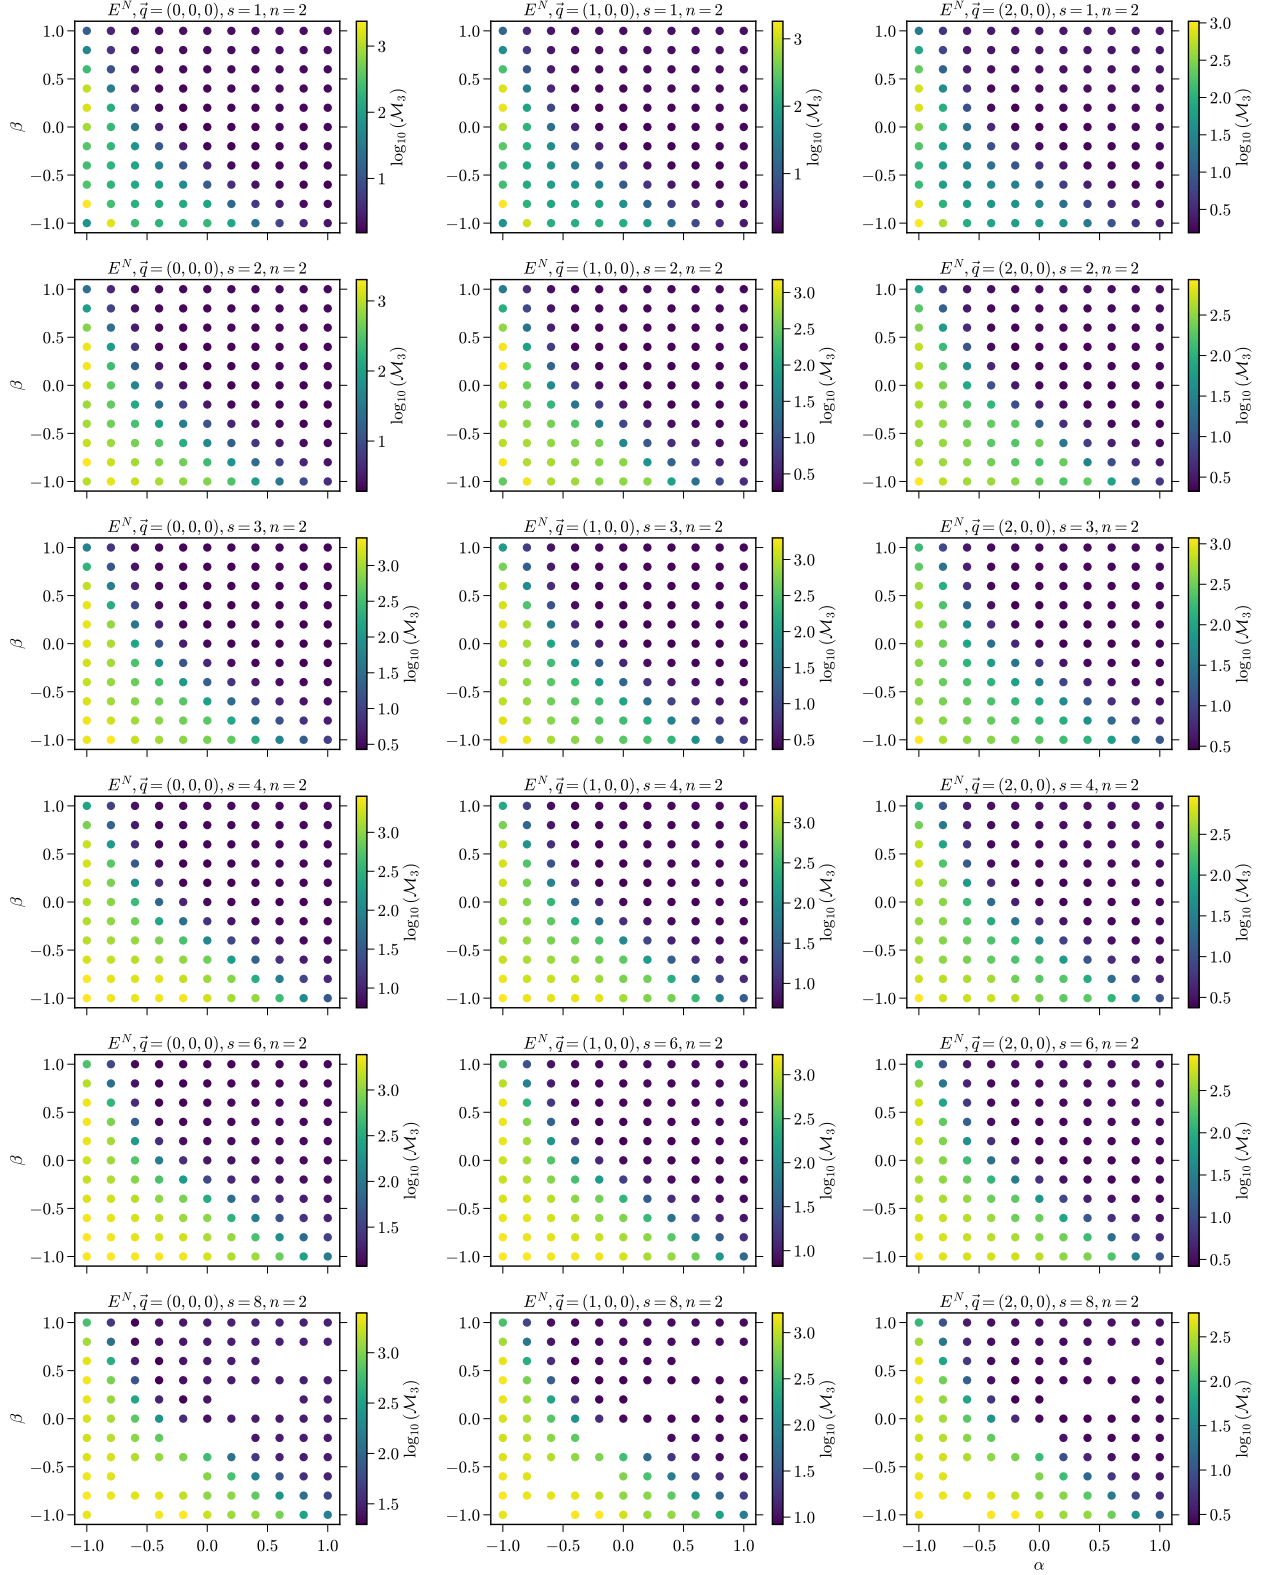

FIG. 24. Metric  $\mathcal{M}_3$  (Eq. (27)), for the proton effective energy as a function of  $\alpha, \beta$ . In this figure, there are  $n = 2$  blocking factor, three different values of momentum, and all 7 possible decimation factors.



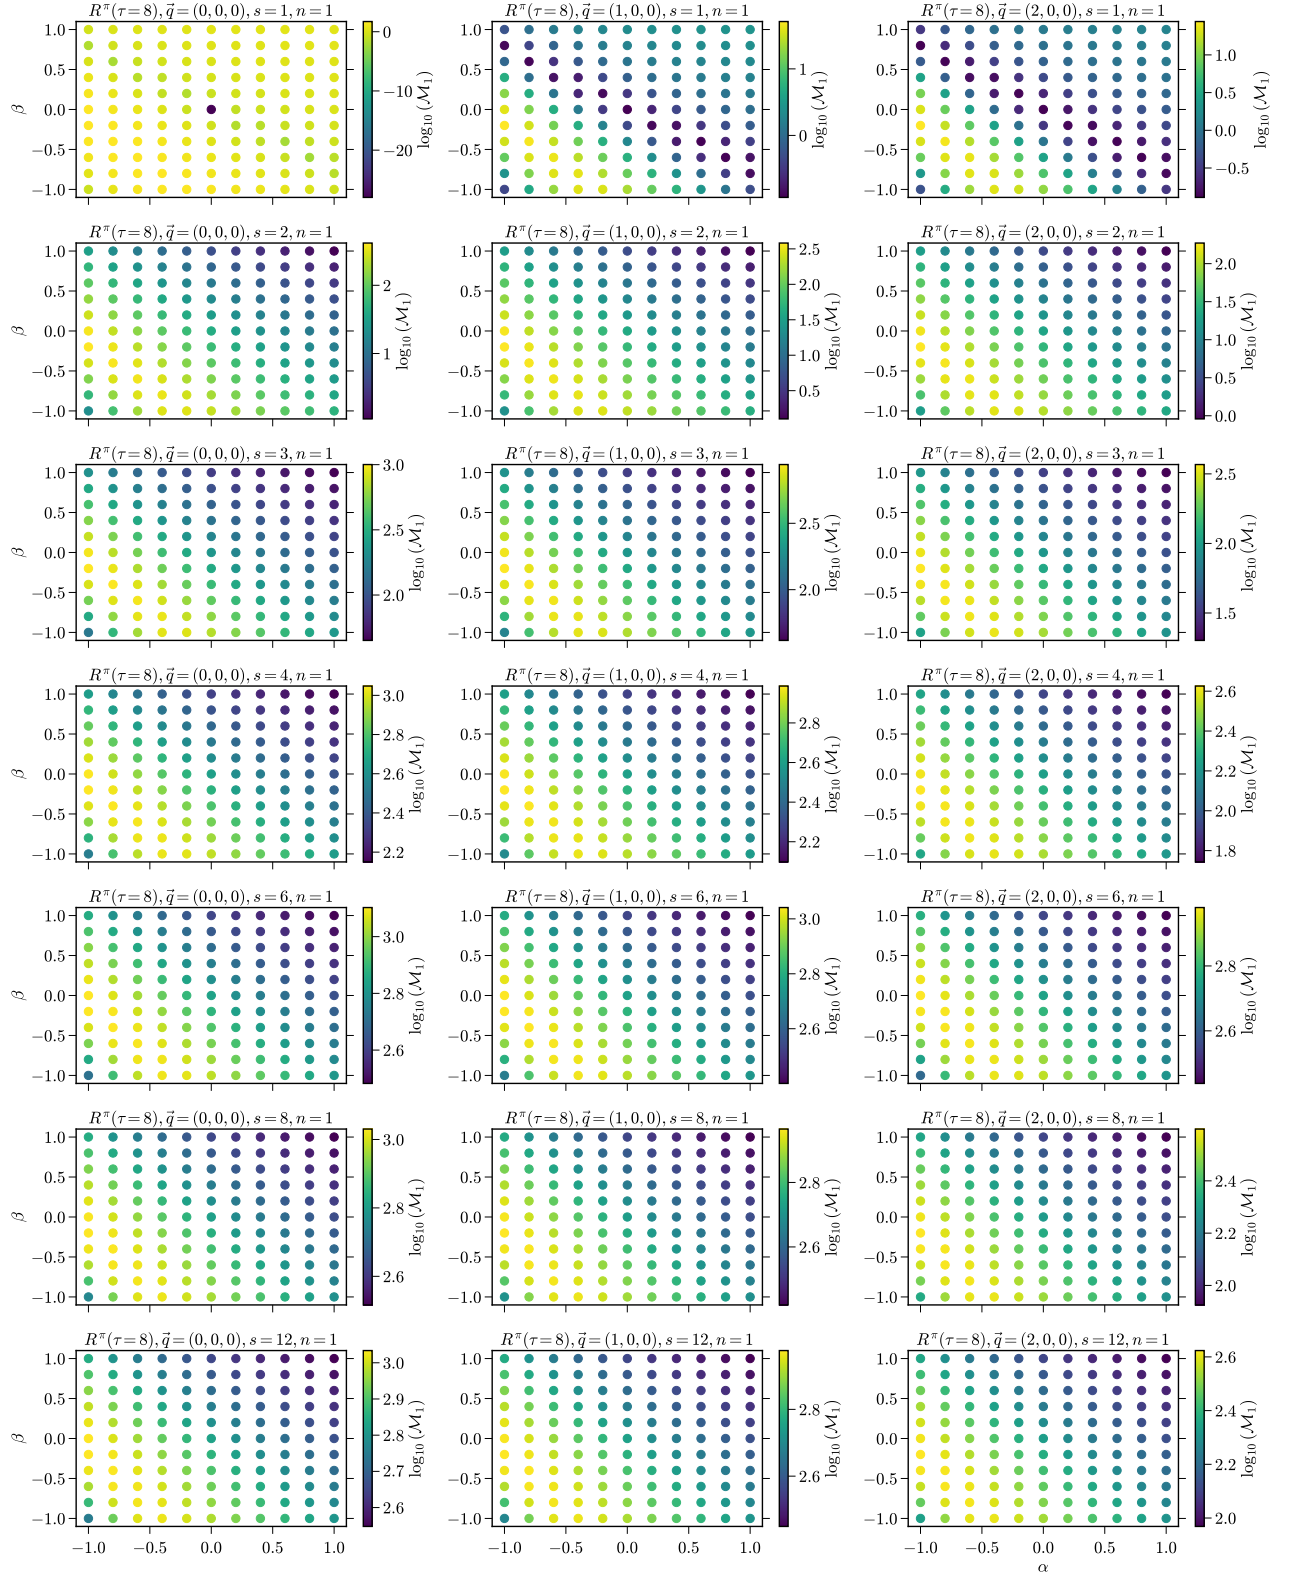

FIG. 25. Metric  $\mathcal{M}_1$  (Eq. (25)), for the pion optimized ratio of two-point and three-point functions as a function of  $\alpha, \beta$ . In this figure, there are  $n = 1$  blocking factor, three different values of momentum, and all 7 possible decimation factors.

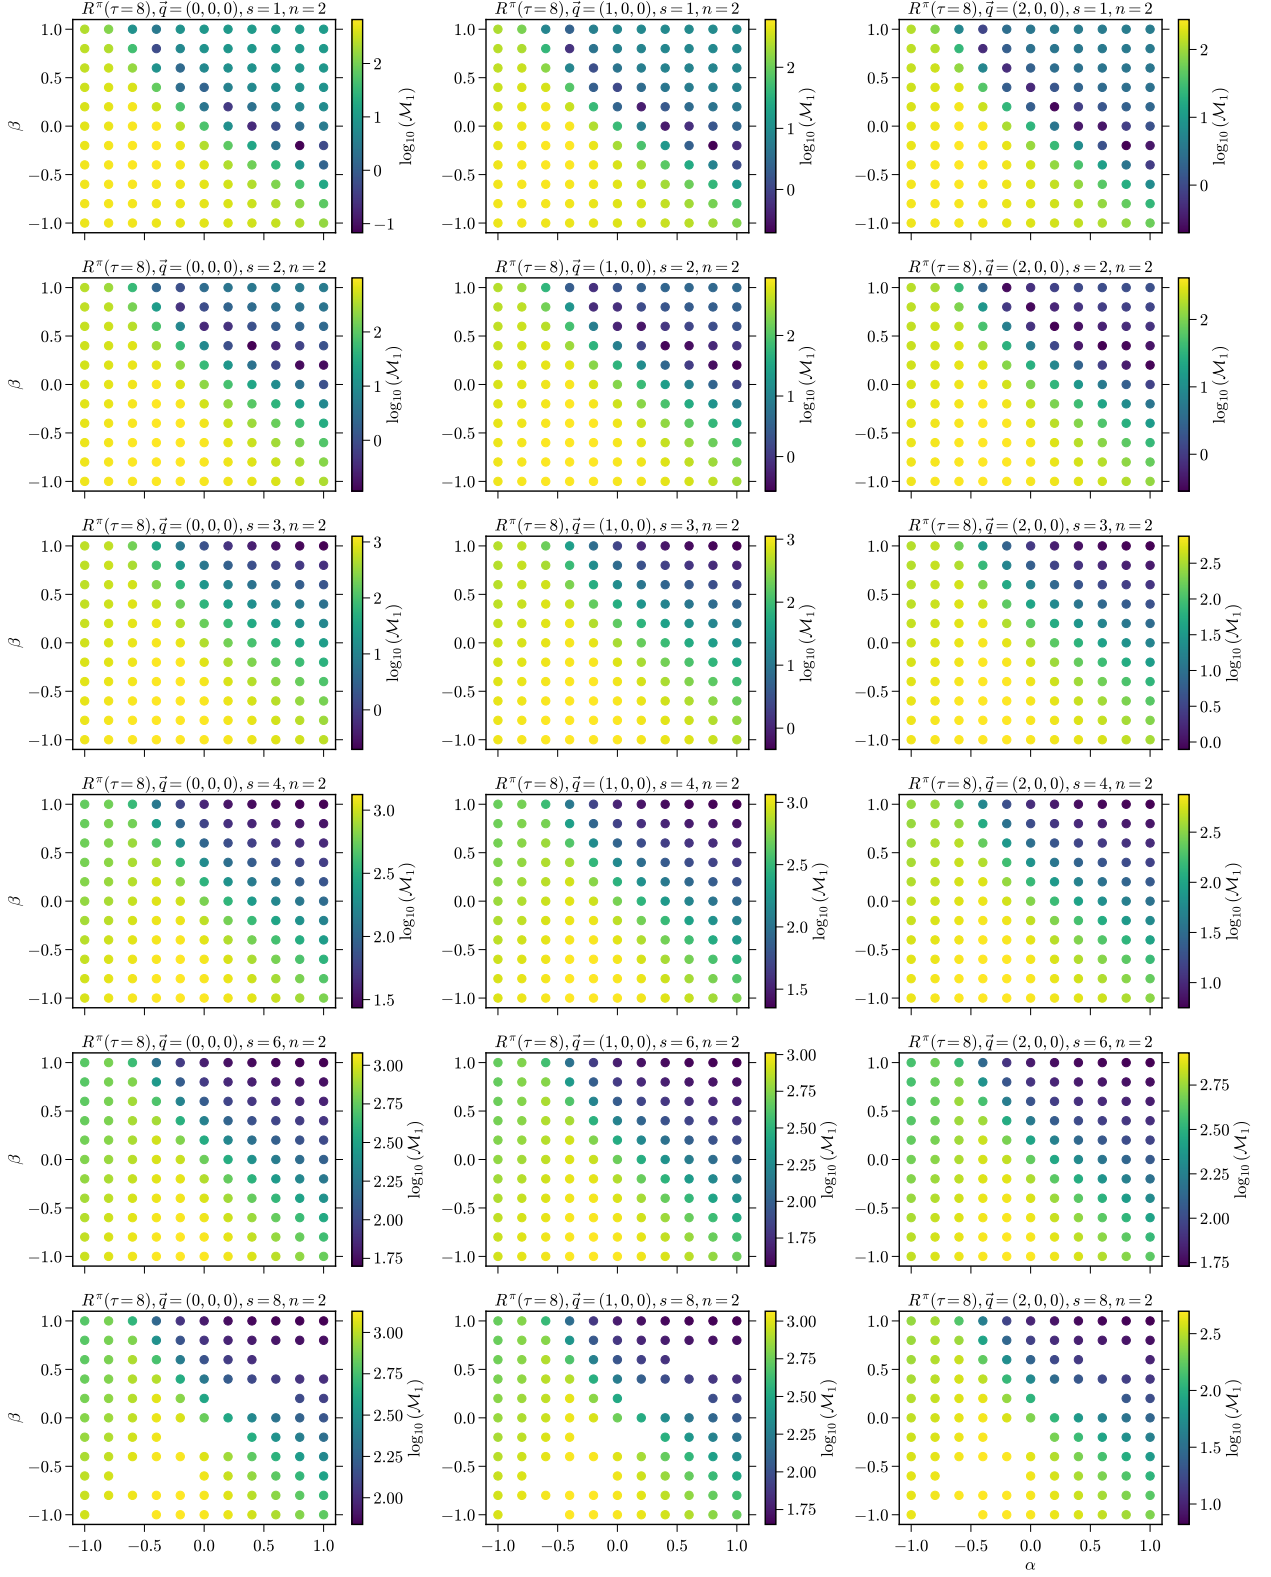

FIG. 26. Metric  $\mathcal{M}_1$  (Eq. (25)), for the pion optimized ratio of two-point and three-point functions as a function of  $\alpha, \beta$ . In this figure, there are  $n = 2$  blocking factor, three different values of momentum, and all 7 possible decimation factors.

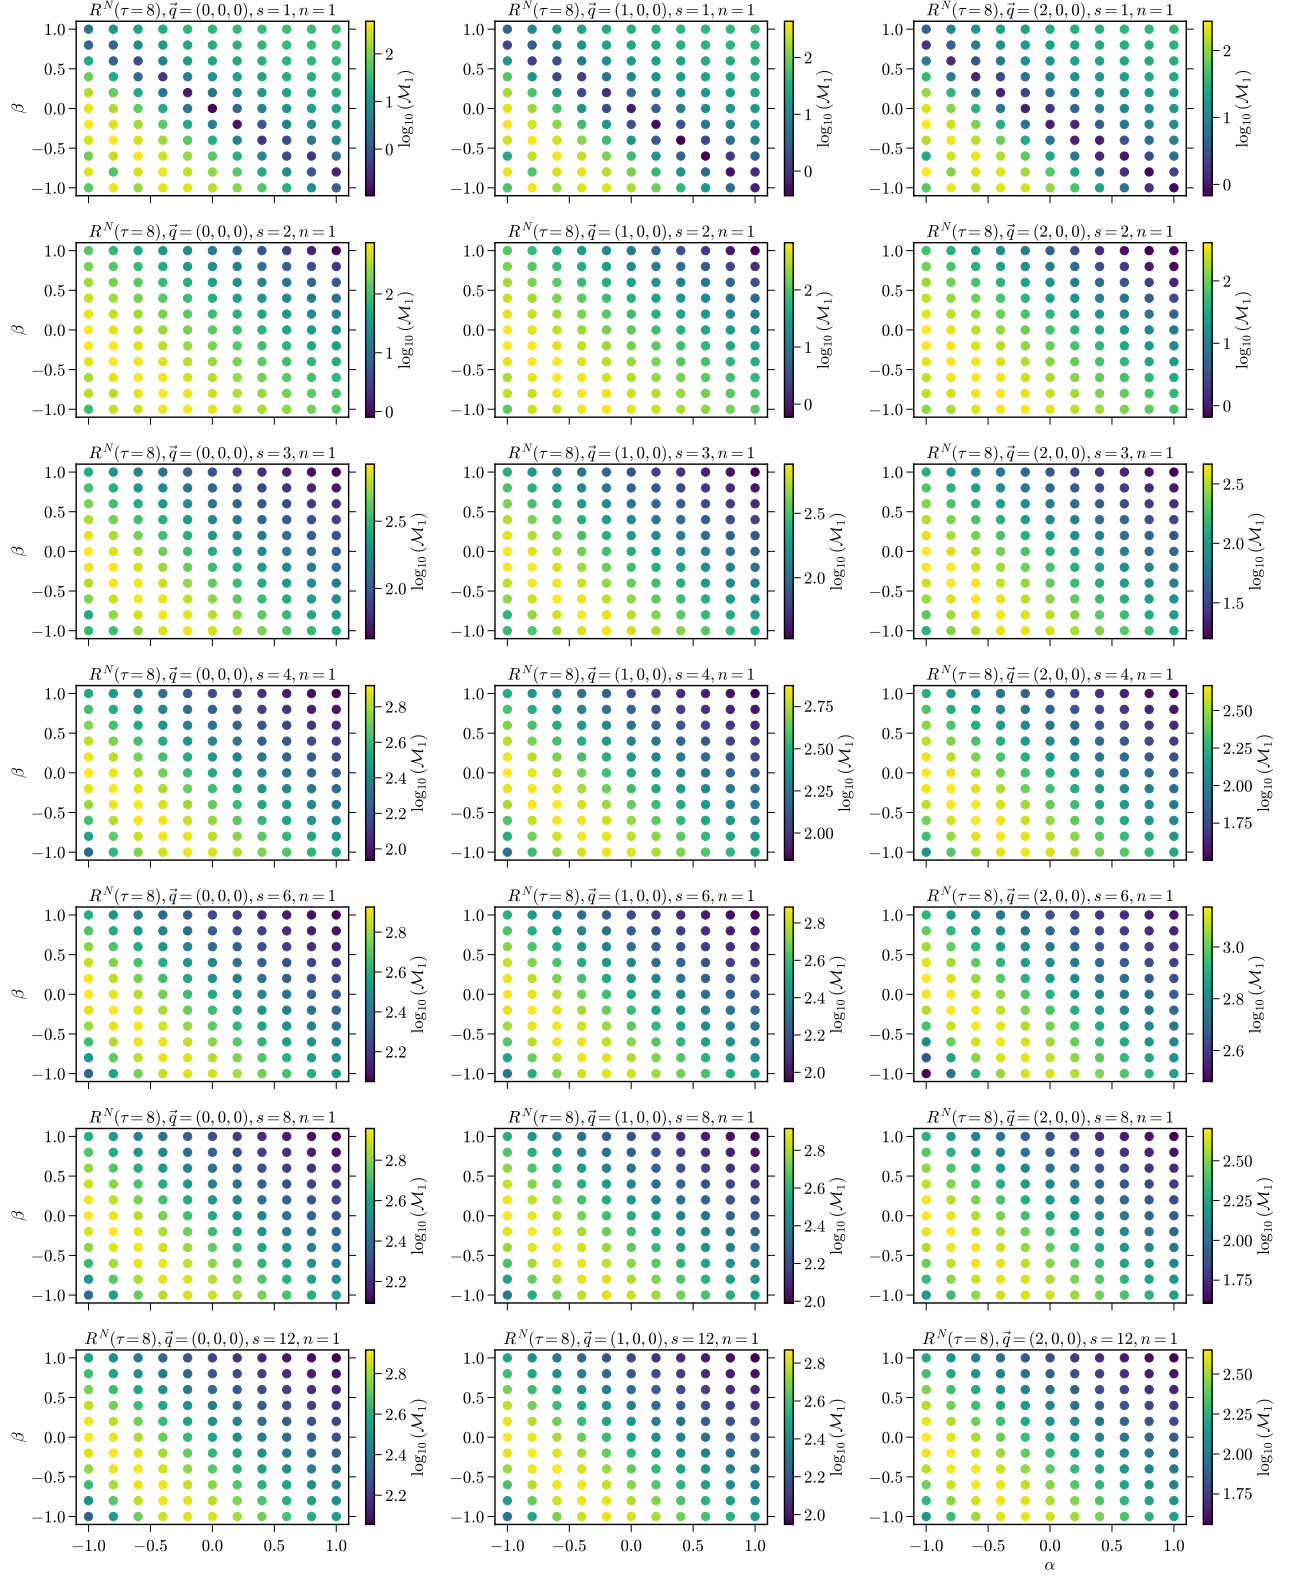

FIG. 27. Metric  $\mathcal{M}_1$  (Eq. (25)), for the proton optimized ratio of two-point and three-point functions as a function of  $\alpha, \beta$ . In this figure, there are  $n = 1$  blocking factor, three different values of momentum, and all 7 possible decimation factors.

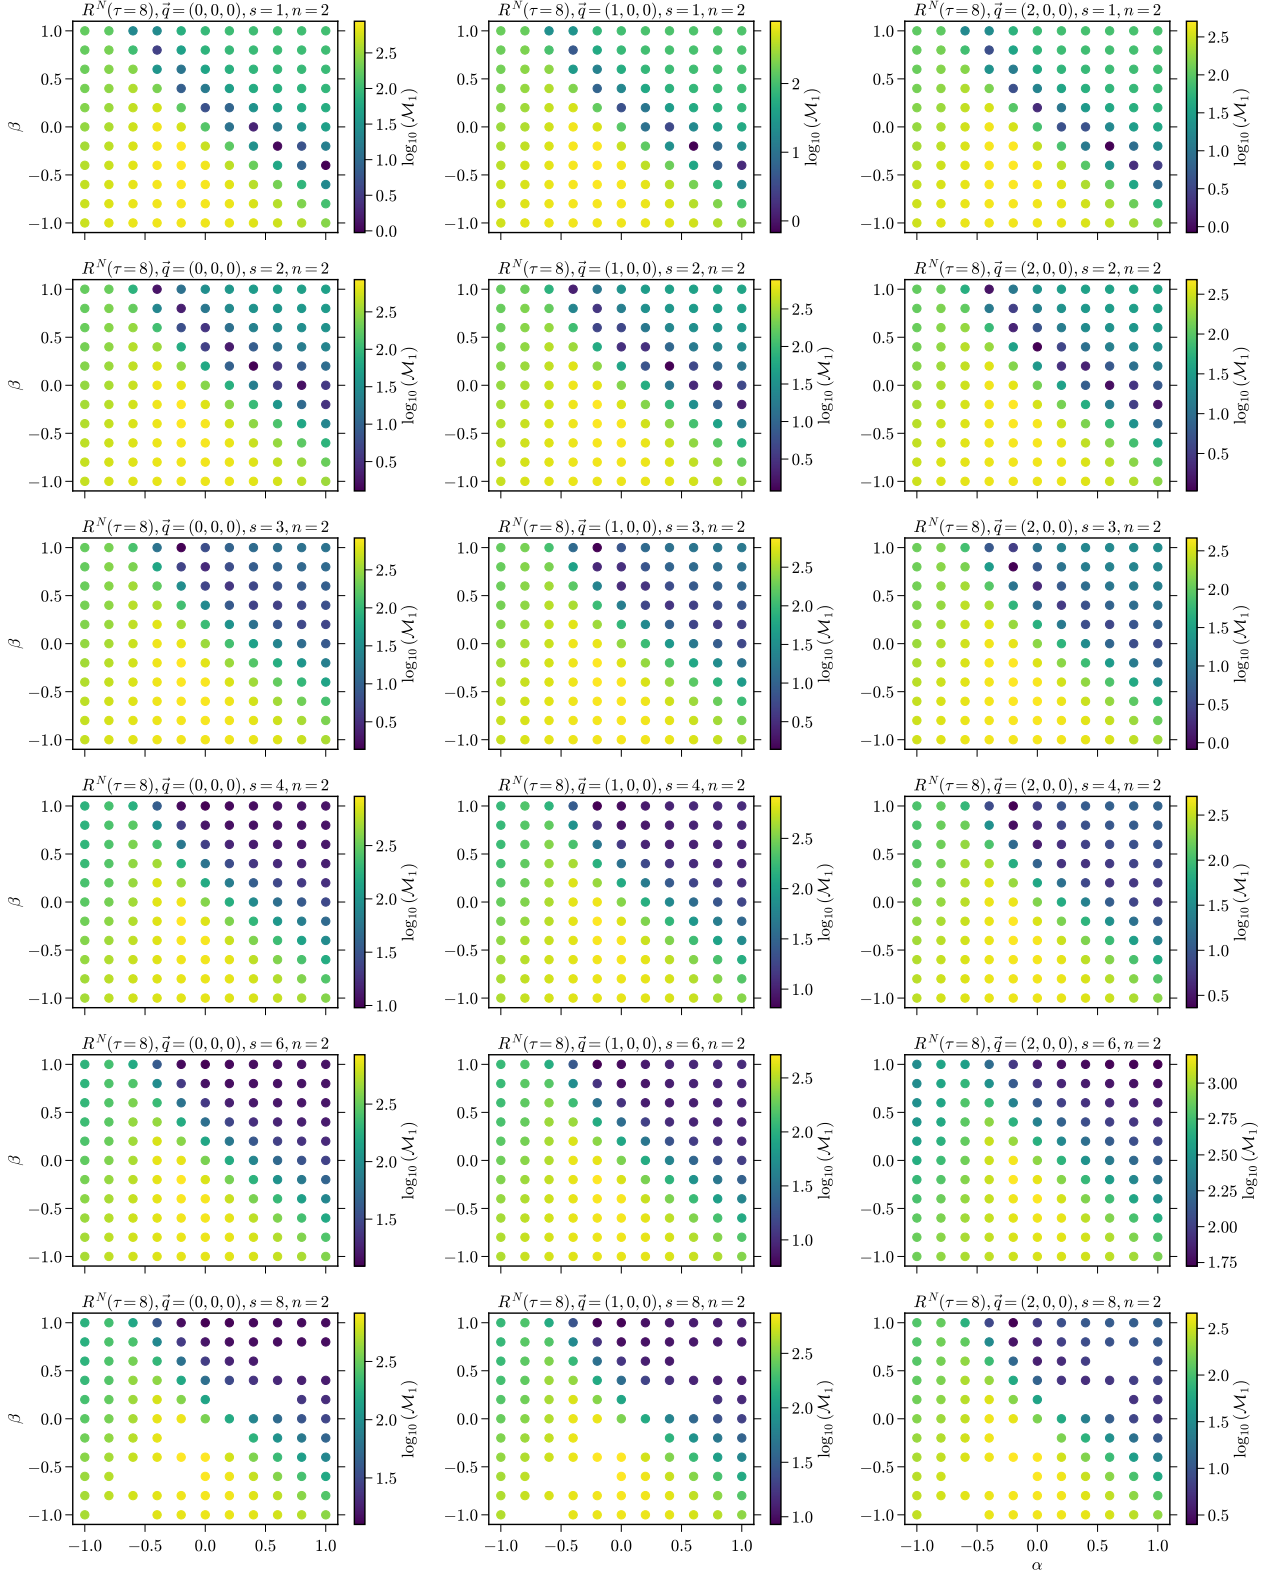

FIG. 28. Metric  $\mathcal{M}_1$  (Eq. (25)), for the proton optimized ratio of two-point and three-point functions as a function of  $\alpha, \beta$ . In this figure, there are  $n = 2$  blocking factor, three different values of momentum, and all 7 possible decimation factors.

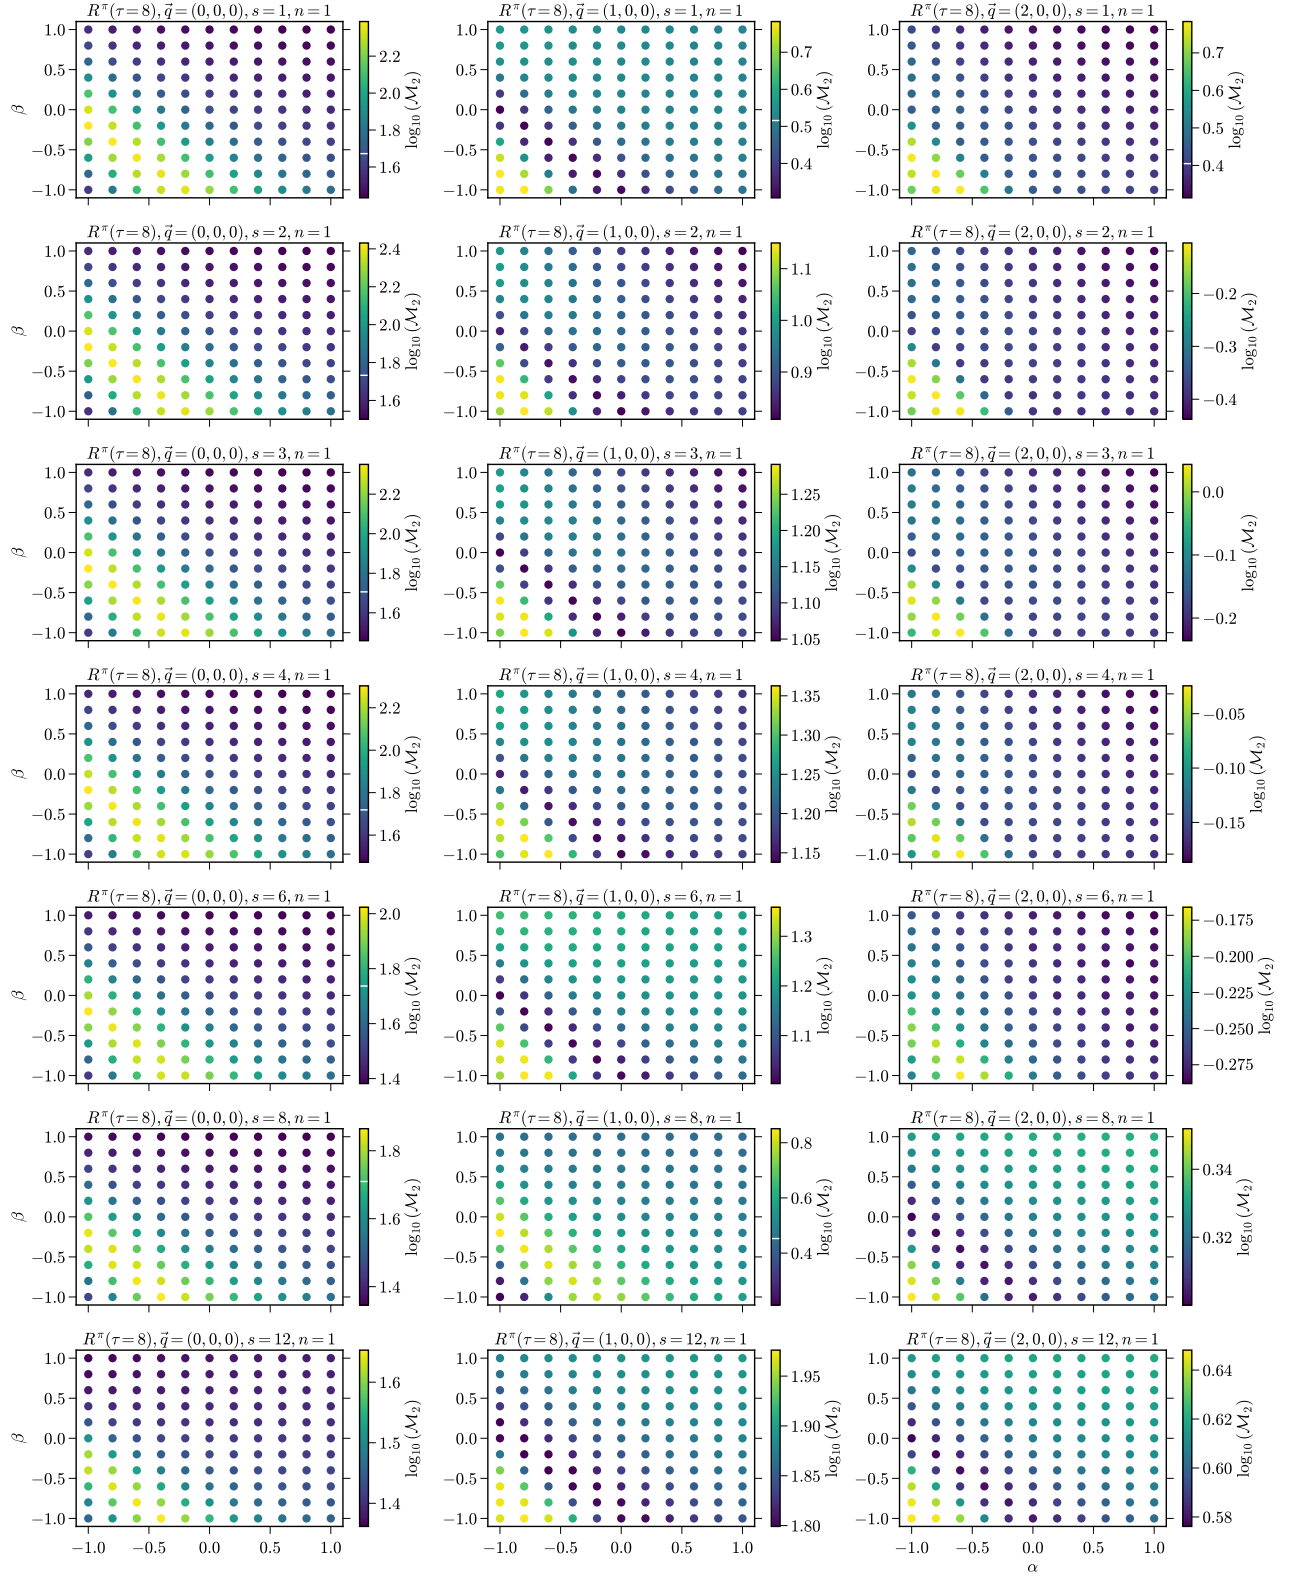

FIG. 29. Metric  $\mathcal{M}_2$  (Eq. (26)), for the pion optimized ratio of two-point and three-point functions as a function of  $\alpha, \beta$ . In this figure, there are  $n = 1$  blocking factor, three different values of momentum, and all 7 possible decimation factors.



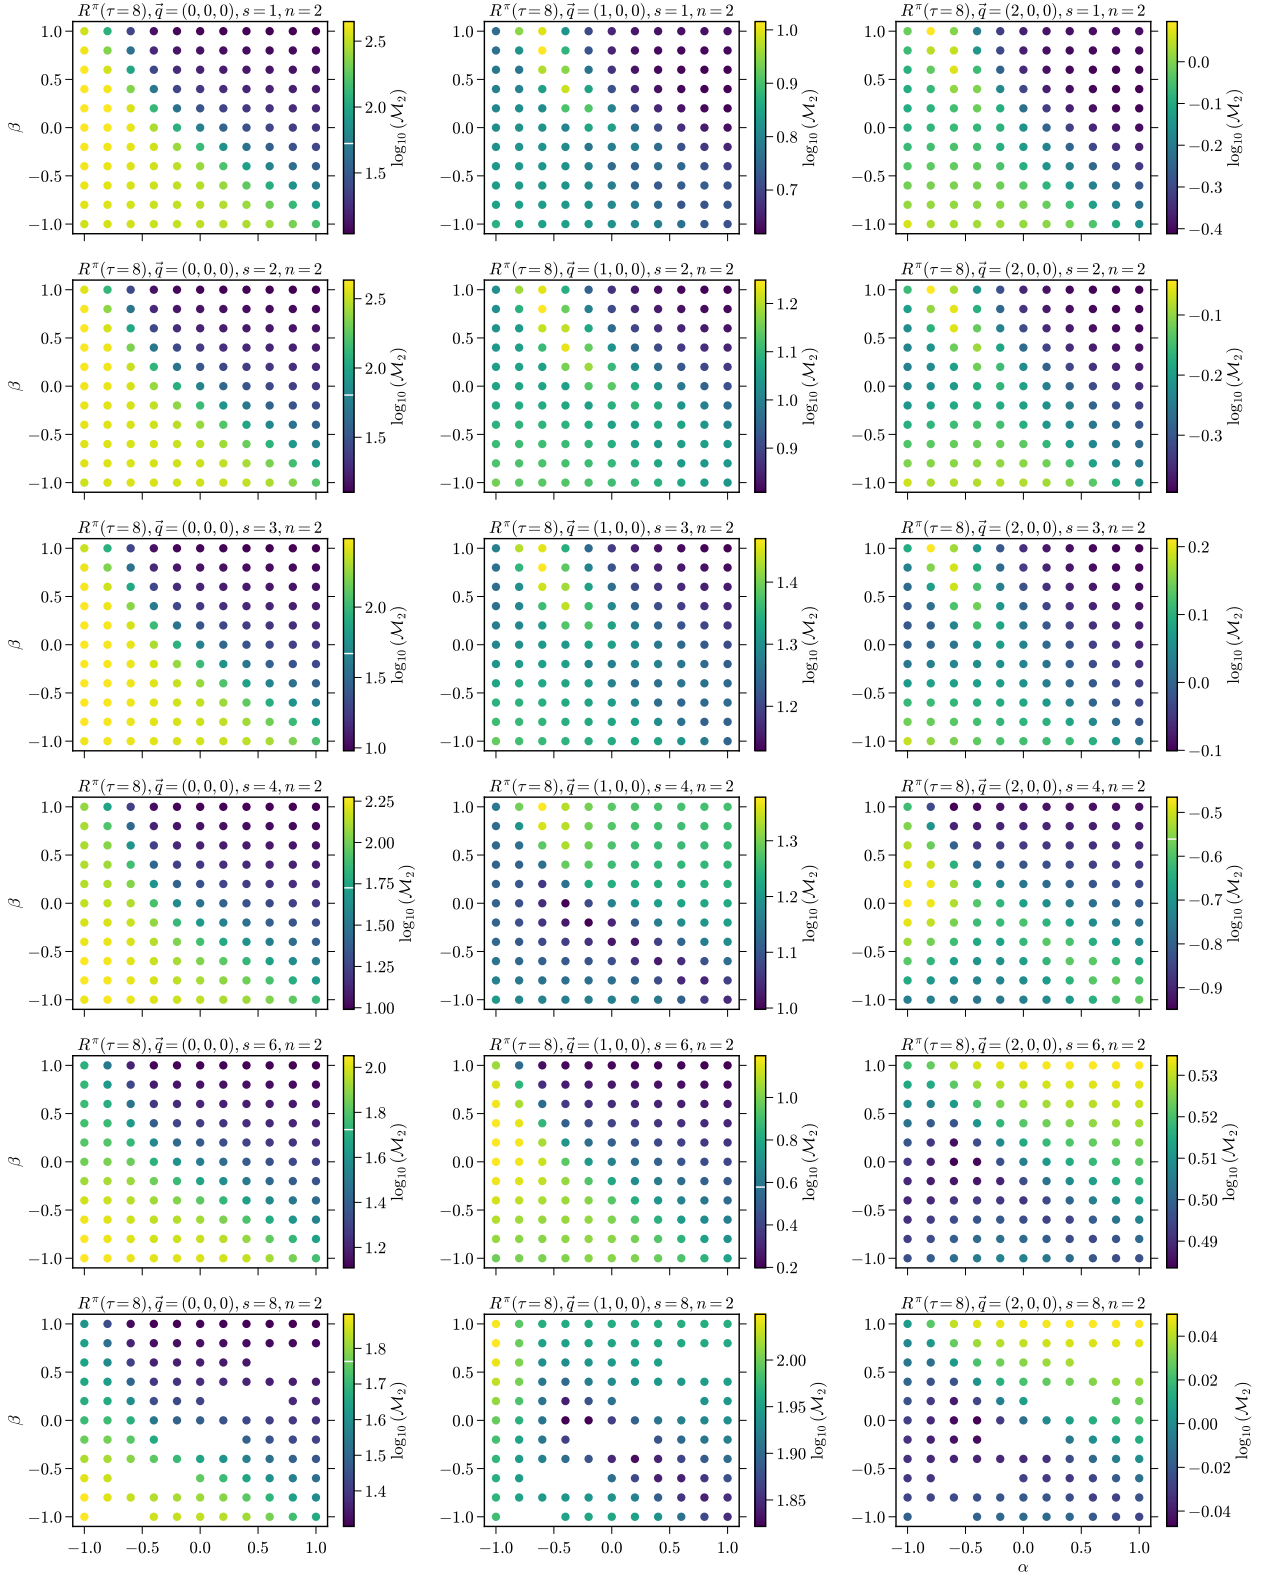

FIG. 30. Metric  $\mathcal{M}_2$  (Eq. (26)), for the pion optimized ratio of two-point and three-point functions as a function of  $\alpha, \beta$ . In this figure, there are  $n = 2$  blocking factor, three different values of momentum, and all 7 possible decimation factors.

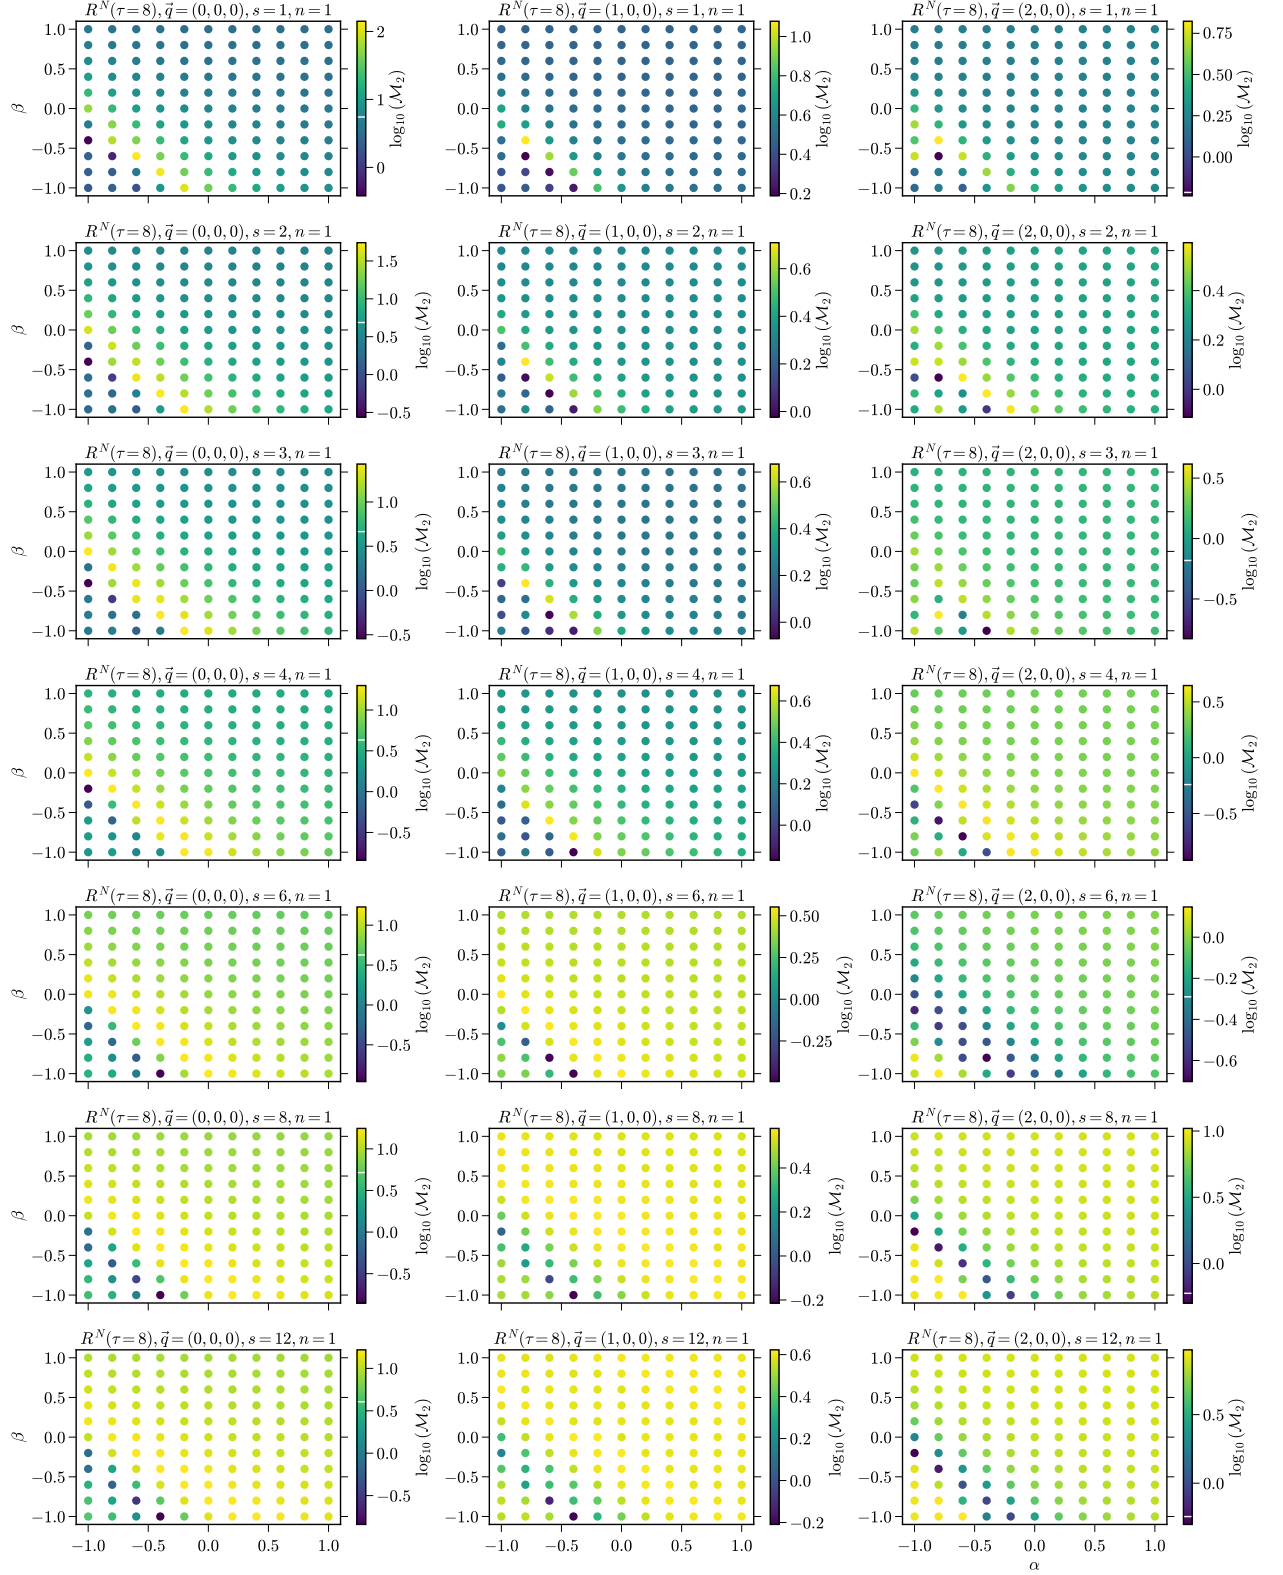

FIG. 31. Metric  $\mathcal{M}_2$  (Eq. (26)), for the proton optimized ratio of two-point and three-point functions as a function of  $\alpha, \beta$ . In this figure, there are  $n = 1$  blocking factor, three different values of momentum, and all 7 possible decimation factors.

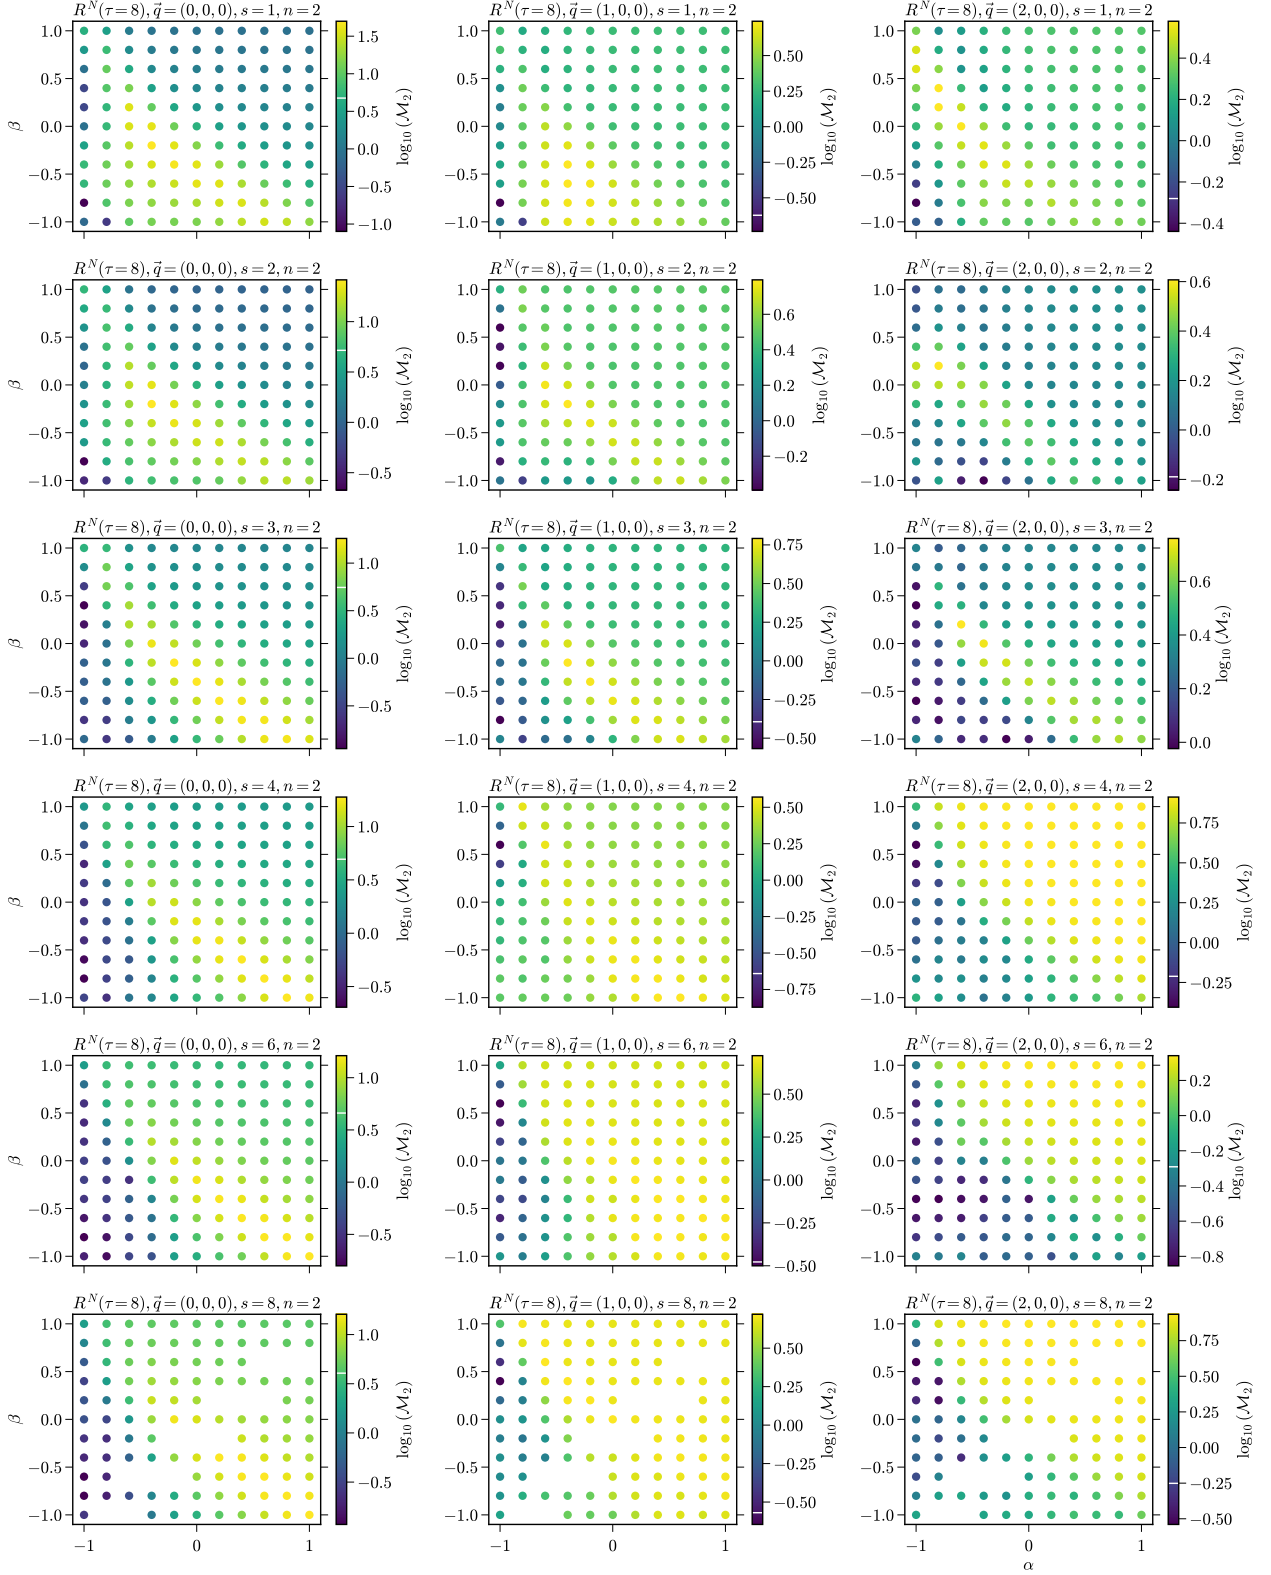

FIG. 32. Metric  $M_2$  (Eq. (26)), for the proton optimized ratio of two-point and three-point functions as a function of  $\alpha, \beta$ . In this figure, there are  $n = 2$  blocking factor, three different values of momentum, and all 7 possible decimation factors.



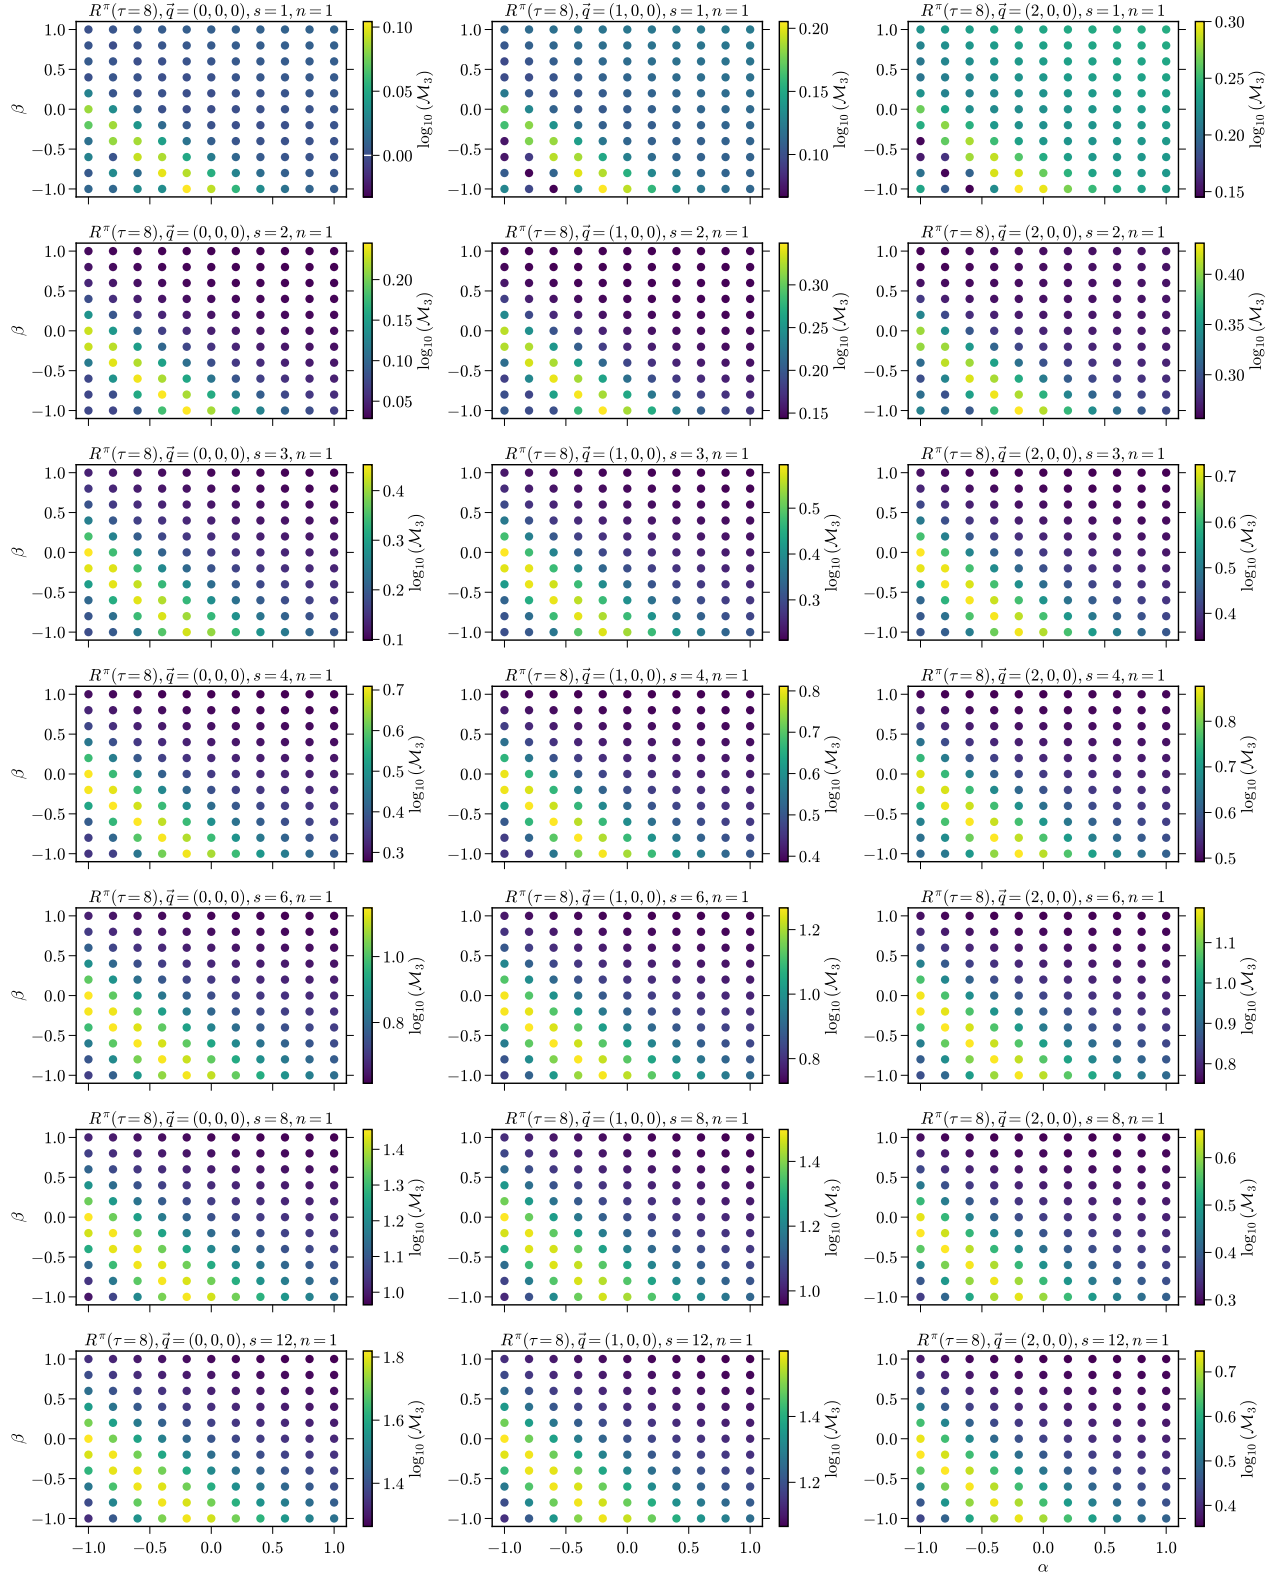

FIG. 33. Metric  $\mathcal{M}_3$  (Eq. (27)), for the pion optimized ratio of two-point and three-point functions as a function of  $\alpha, \beta$ . In this figure, there are  $n = 1$  blocking factor, three different, values of momentum, and all 7 possible decimation factors.

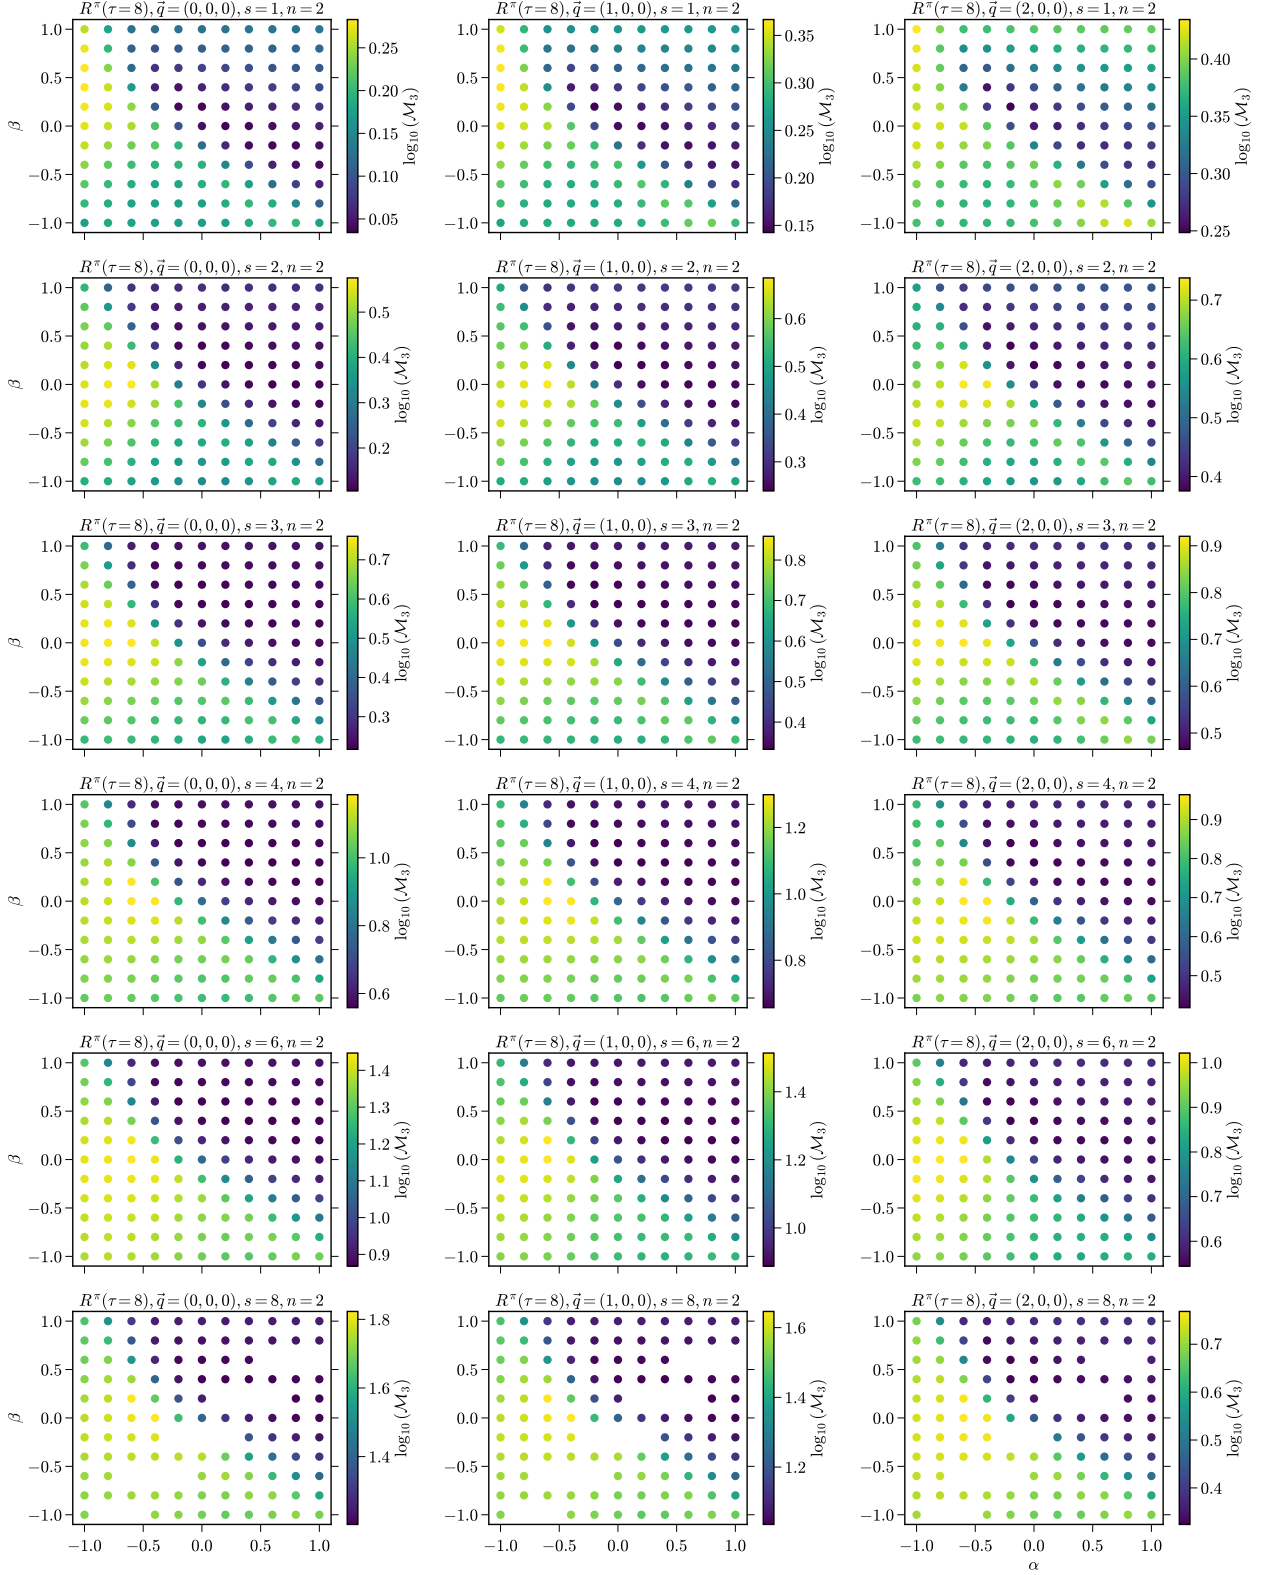

FIG. 34. Metric  $\mathcal{M}_3$  (Eq. (27)), for the pion optimized ratio of two-point and three-point functions as a function of  $\alpha, \beta$ . In this figure, there are  $n = 2$  blocking factor, three different values of momentum, and all 7 possible decimation factors.

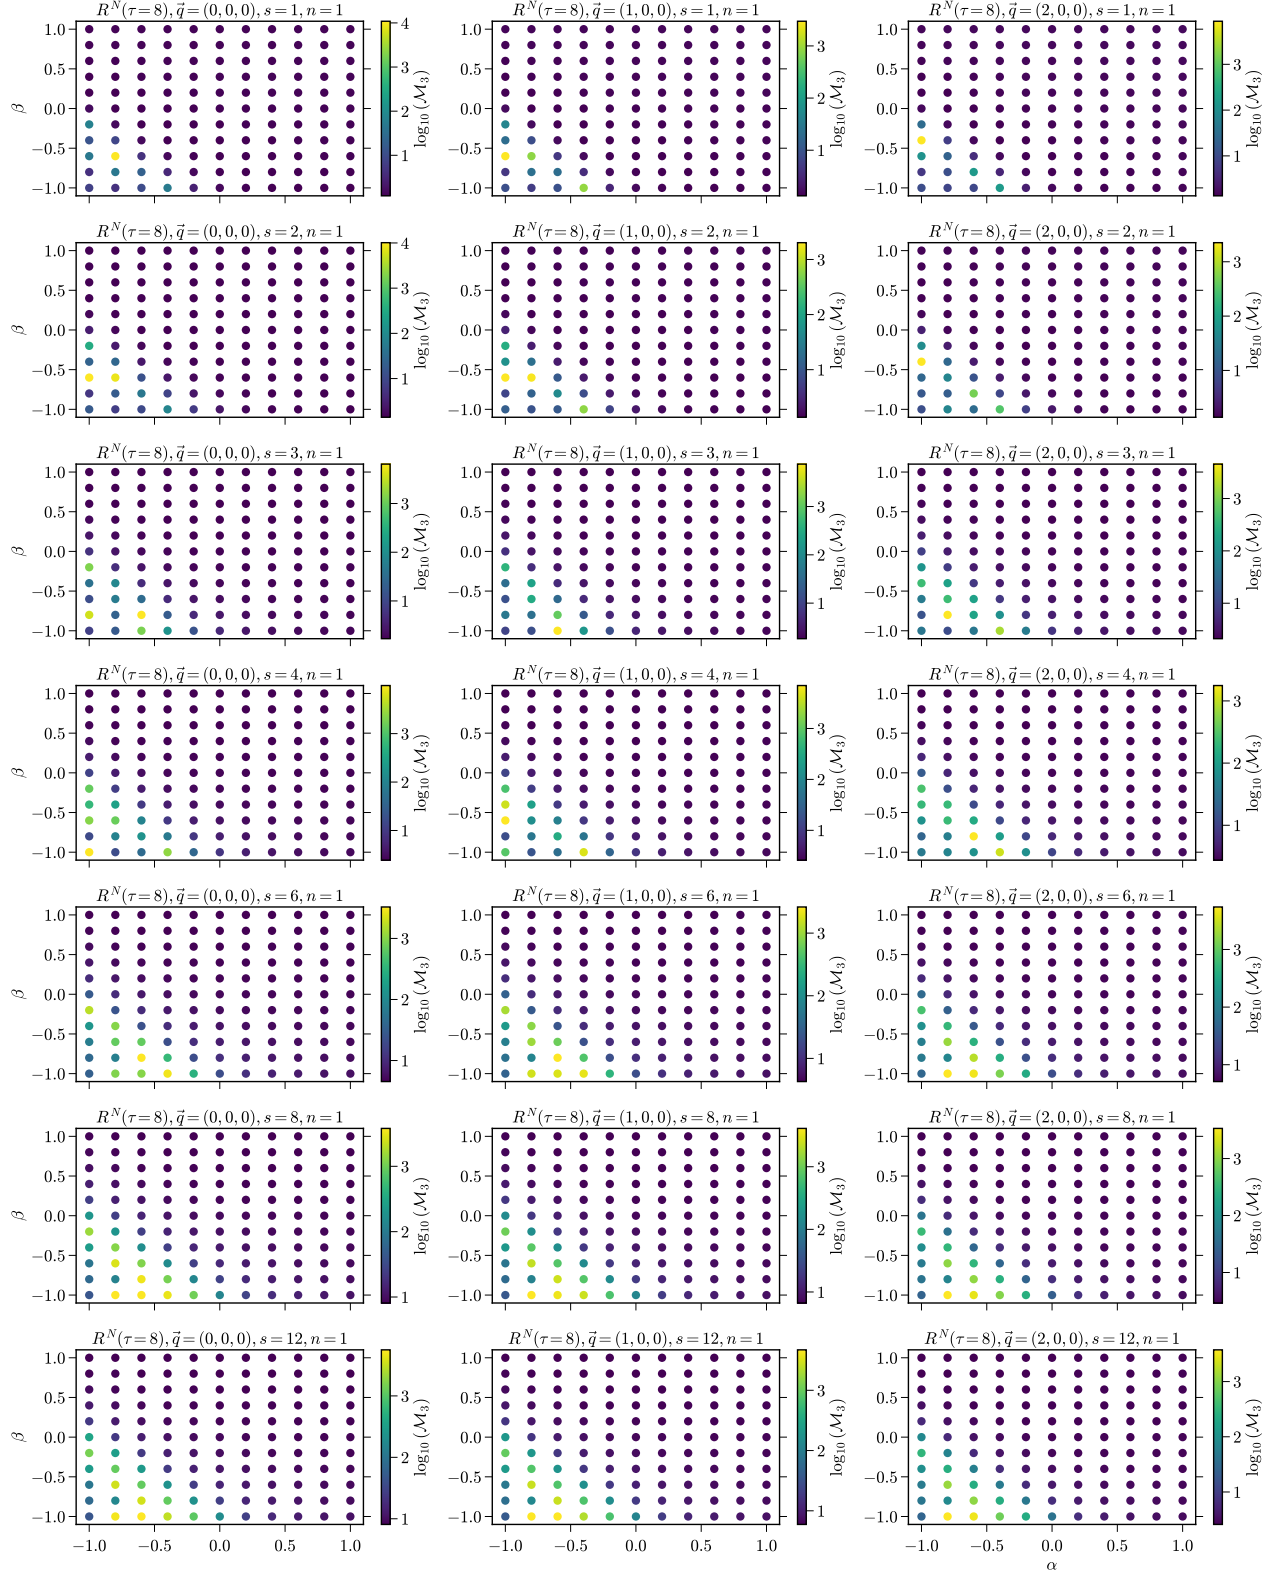

FIG. 35. Metric  $\mathcal{M}_3$  (Eq. (27)), for the proton optimized ratio of two-point and three-point functions as a function of  $\alpha, \beta$ . In this figure, there are  $n = 1$  blocking factor, three different values of momentum, and all 7 possible decimation factors.

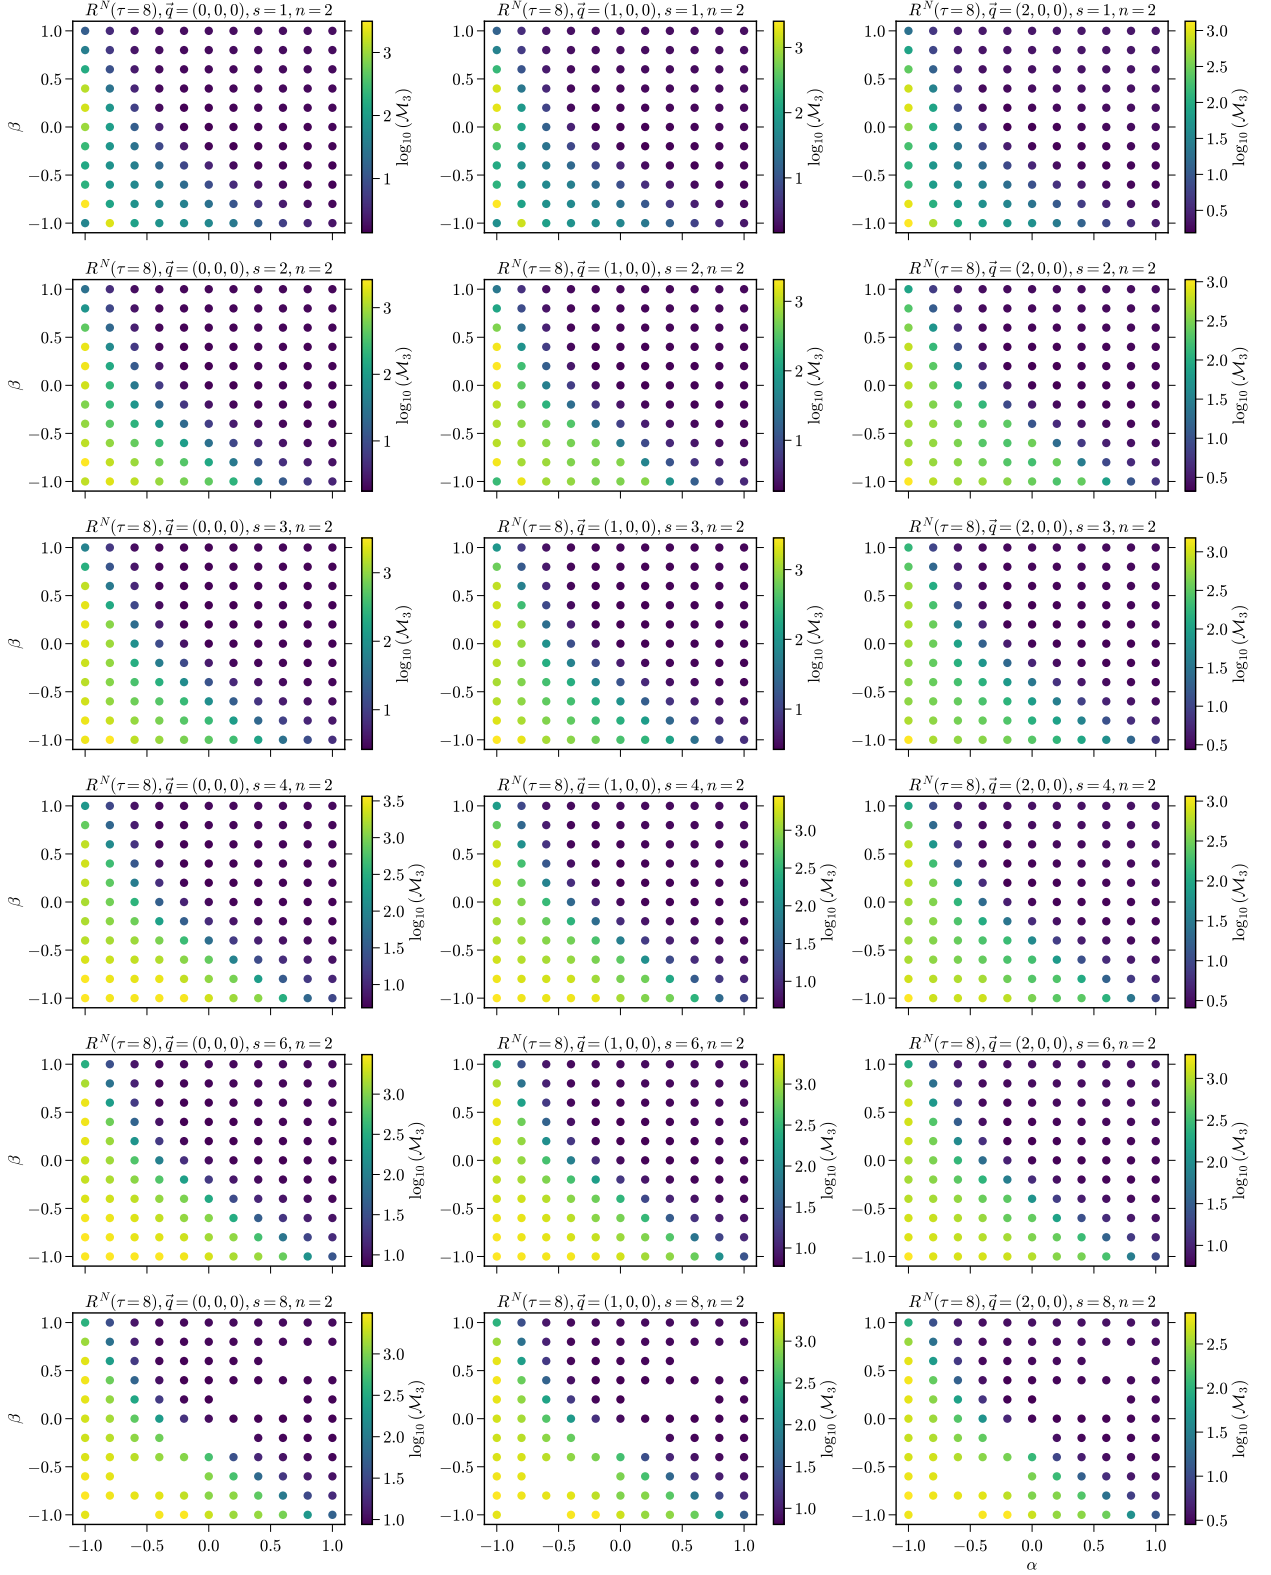

FIG. 36. Metric  $\mathcal{M}_3$  (Eq. (27)), for the proton optimized ratio of two-point and three-point functions as a function of  $\alpha, \beta$ . In this figure, there are  $n = 2$  blocking factor, three different values of momentum, and all 7 possible decimation factors.

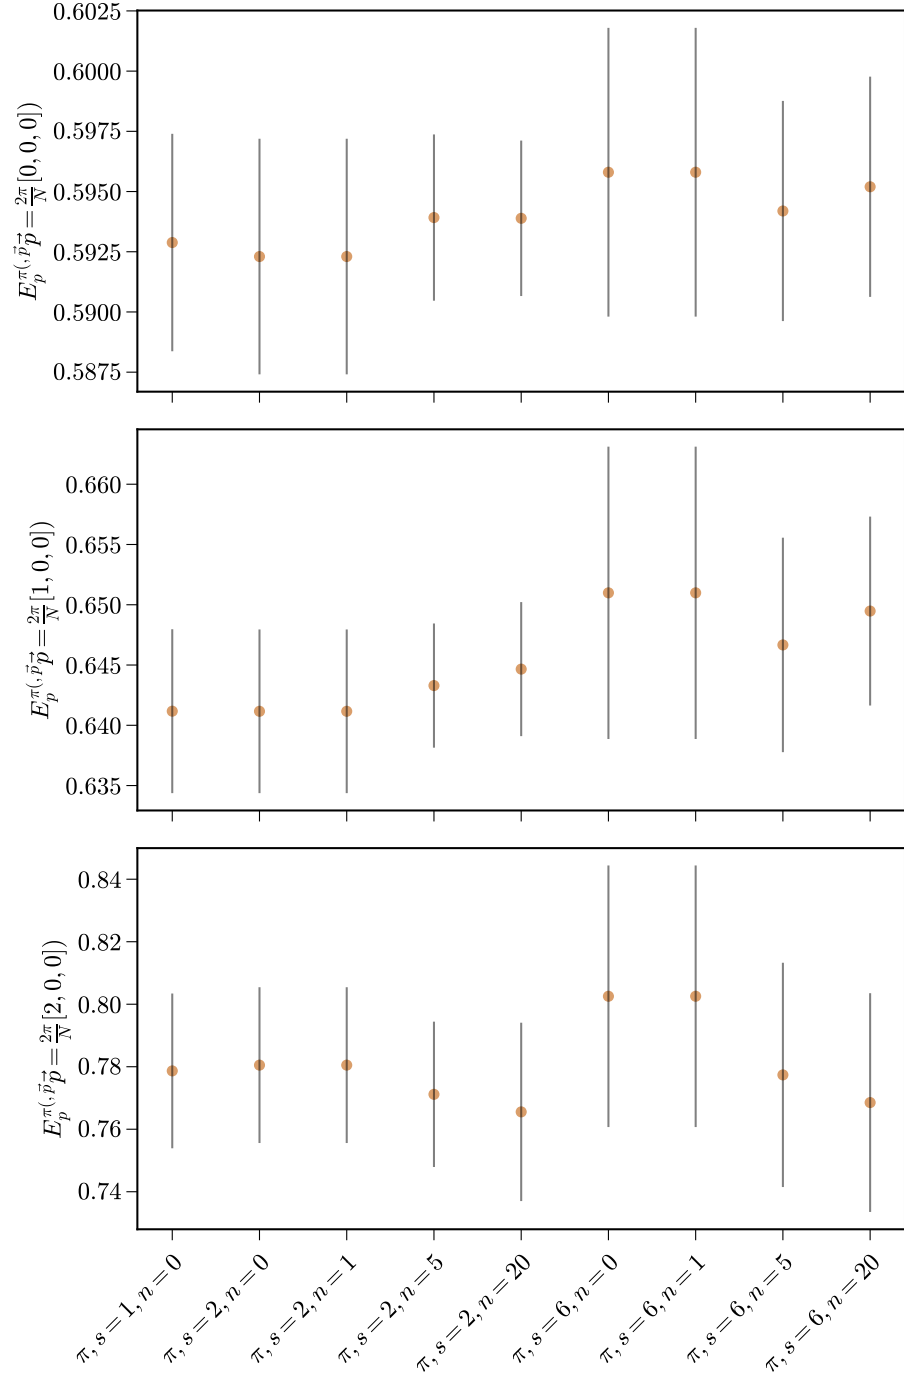

FIG. 37. The best-fit value of the pion effective energy,  $E_p^{\pi, \vec{p}}$  (see Sec. IV B). We use  $\alpha = \beta = 1$  throughout.

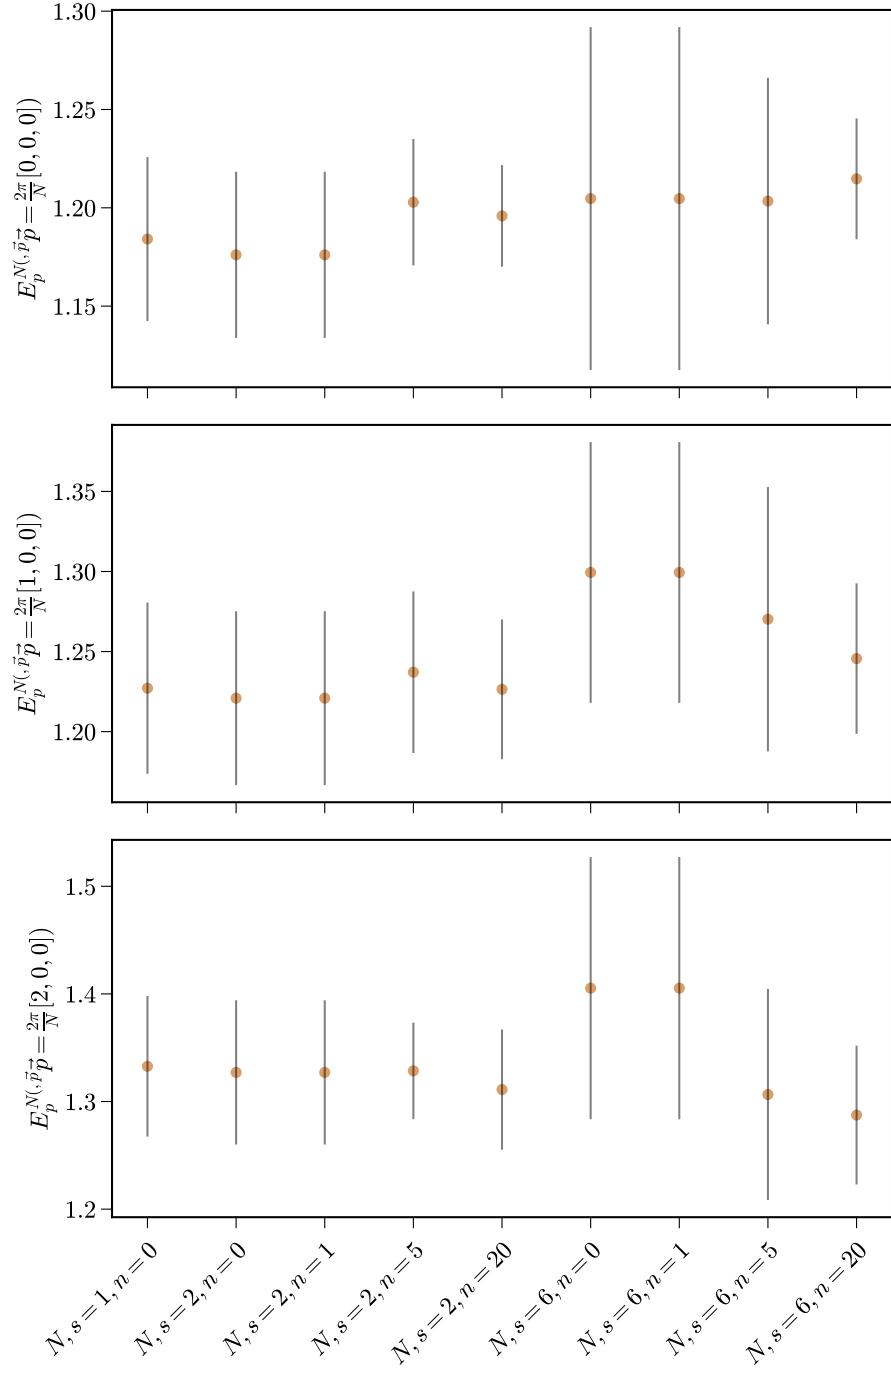

FIG. 38. The best-fit value of the proton effective energy,  $E_p^{N, \vec{p}}$  (see Sec. IV B). We use  $\alpha = \beta = 1$  throughout.

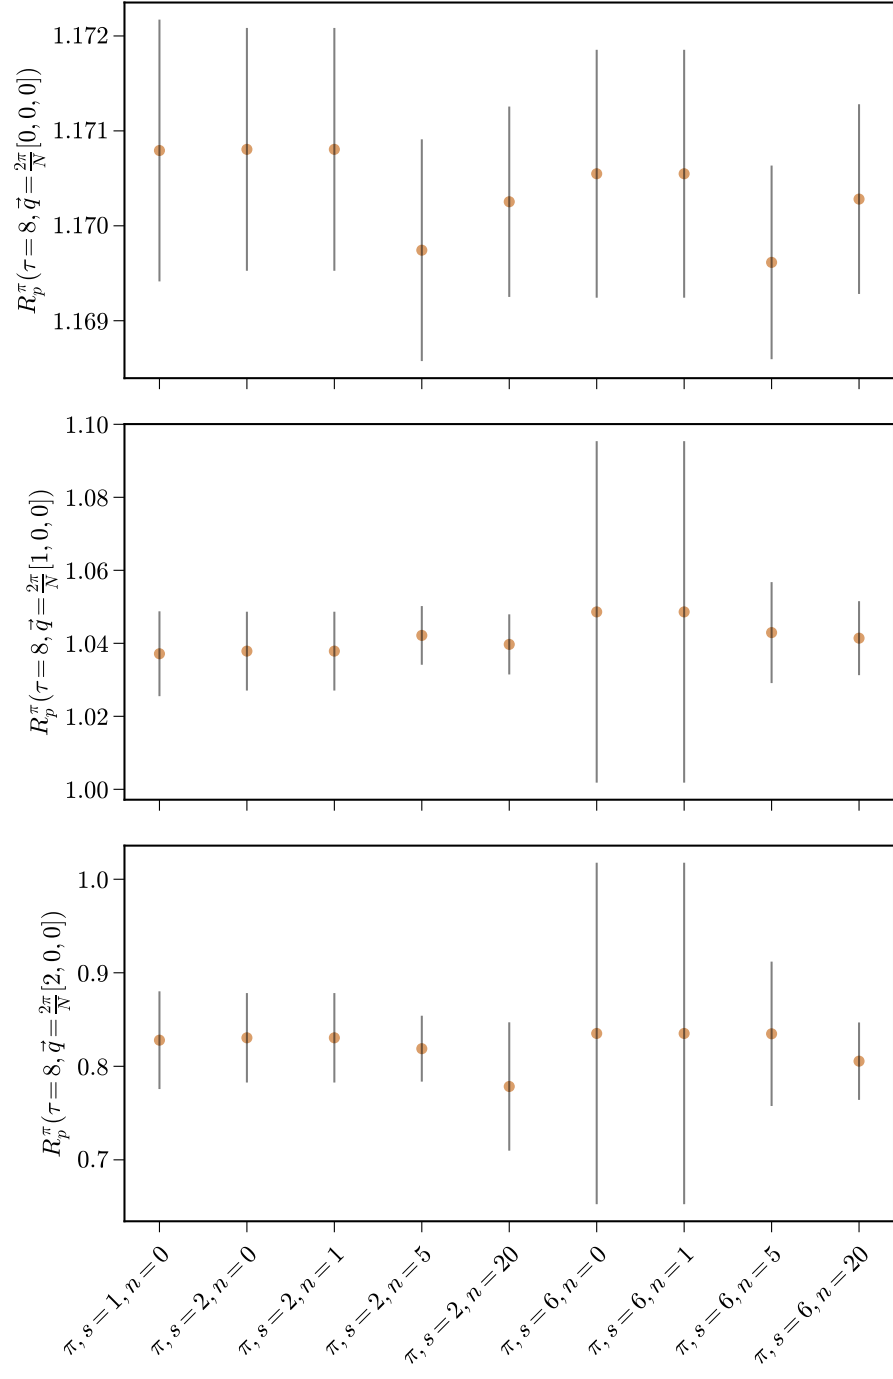

FIG. 39. The best-fit value of the pion improved ratio of three- and two-point functions,  $R_p^\pi(\tau, \vec{q})$  (see Sec. IV B). We use  $\alpha = \beta = 1$  throughout.

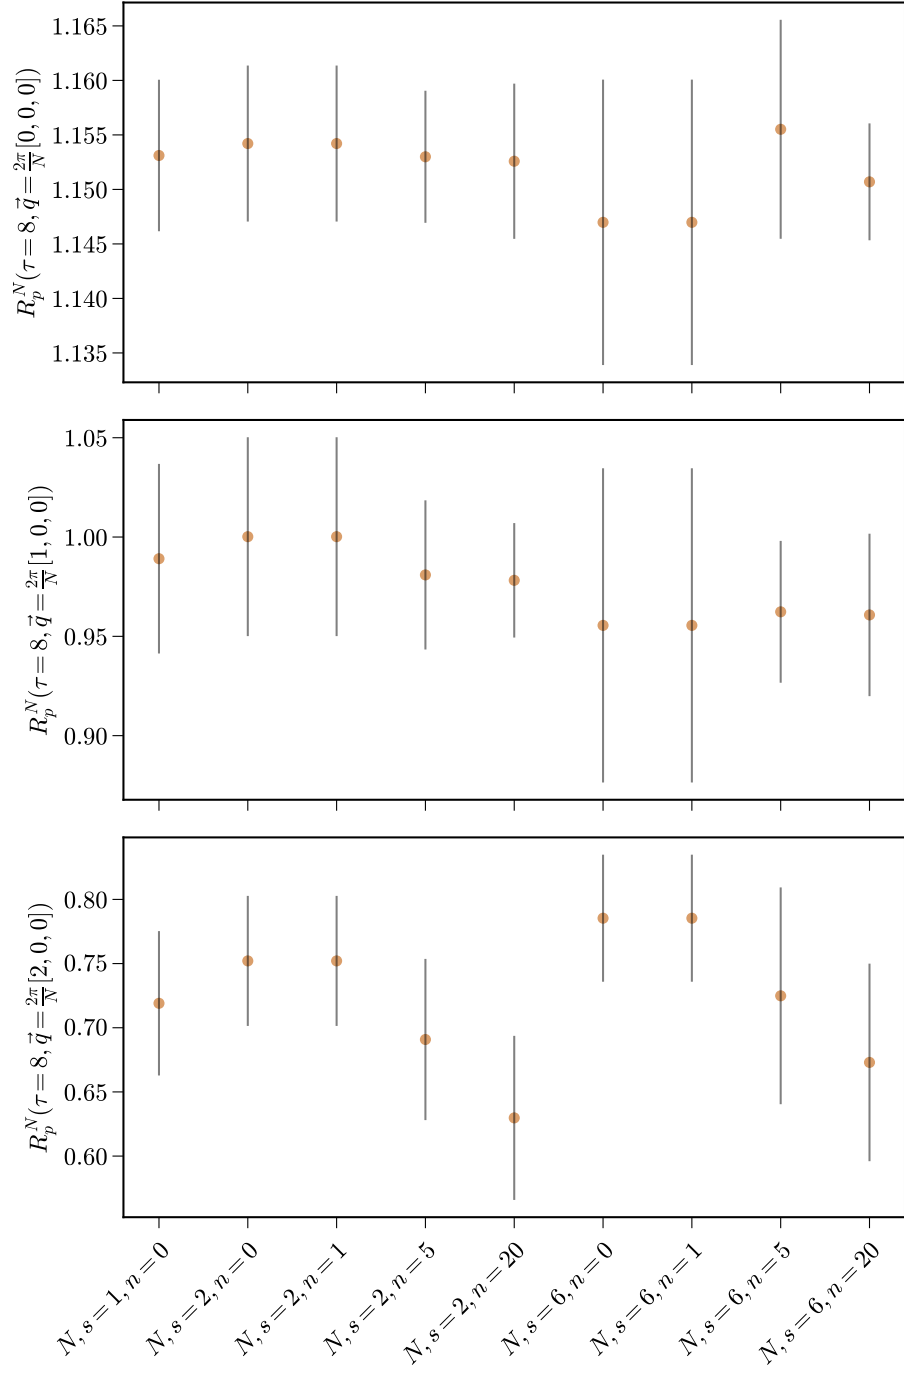

FIG. 40. The best-fit value of the proton improved ratio of three- and two-point functions,  $R_p^N(\tau, \vec{q})$  (see Sec. IV B). We use  $\alpha = \beta = 1$  throughout.
